# Supplementary material for: Realization of Hopf-link structure in phonon spectra: Symmetry guidance and High-throughput investigation
Source: arXiv:2412.01280 ancillary file (2024-12-02)
Supplement: Supplementary file 1 [file Supporting_Information.pdf]

# Supporting Information for "Realization of Hopf-link structure in phonon spectra: Symmetry guidance and High-throughput investigation"

Houhao Wang,[†,‡] Licheng Zhang,[†,‡] Ruixi Pu,[†,‡] Xiangang Wan,[†,‡,¶] and Feng Tang[*,†,‡]

†*National Laboratory of Solid State Microstructures and School of Physics, Nanjing University, Nanjing 210093, China*

‡*Collaborative Innovation Center of Advanced Microstructures, Nanjing University, Nanjing 210093, China*

¶*Jiangsu Physical Science Research Center*

E-mail: fengtang@nju.edu.cn

Section **S1**: Details on first-principles calculation.

Section **S2**: $k \cdot p$ model on the Hopf-link structure in $Ga_5(PS)_3$.

Section **S3**: Seven representative materials with relatively clean phonon Hopf-link structure.

Section **S4**: List of materials with phonon Hopf-link structure.

Section **S5**: Tabulation of space groups possibly hosting phonon Hopf-link structure.

# S1. Details on first-principles calculation

In our work, for each investigated material, we utilize the optimized lattice constants and the force constants stored in Phonon Database at Kyoto University,[1] which are derived from the finite displacement method using the Vienna Ab initio Simulation Package (VASP).[2,3] The calculation of irreducible representations (irreps) of phonons within high-symmetry lines (HSLs) of each material is based on our homemade program written in Python, which is based on the phonon eigenstates output by PHONOPY package.[4] Identifying nodal loops and nodal chains lying in high-symmetry planes (HSPLs) in the Brillouin zone (BZ) involves setting a threshold for the energy gap between a pair of branches to 0.01 THz and using a $100 \times 100$ $K$-points mesh in 2D momentum planes. The phonon tight-binding Hamiltonian is generated from the computed force constants using the PHONOPYTB tool.[5,6] This tool is used to calculate surface states via the iterative Green's function approach[7] and to compute the Berry phase.

## S2. $k \cdot p$ model on the Hopf-link structure in $Ga_5(PS)_3$

*Brief summary.*—To further validate the predicted Hopf-link structure in $Ga_5(PS)_3$ mentioned in the main text, we use the constructed $k \cdot p$ model to fit the first-principles phonon spectra and to sketch the nodal loops based on the concrete $k \cdot p$ model. We first list the $k \cdot p$ models near the BCs indicated by the dashed yellow circle, which include $\mathrm{G}_i$ $(i = 1, 2, 3)$ mentioned in the main text.

The $k \cdot p$ model for $\mathrm{G}_1$ reads

$$H_{\mathrm{G}_1} = \begin{pmatrix} q_z(R_1 + R_4) & q_x(R_2 - \mathrm{i}R_3) \\ q_x(R_2 + \mathrm{i}R_3) & q_z(R_1 - R_4) \end{pmatrix} \tag{S1}$$

where $q_{x,y,z}$ are the momentum components measured from the band crossings (BCs) (in units of $\frac{1}{\text{Å}}$) in the HSL and $R_1$, $R_2$, $R_3$ and $R_4$ are all real-valued parameters.

The $k \cdot p$ model for $\mathrm{G}_2$ reads

$$H_{\mathrm{G}_2} = \begin{pmatrix} q_z(R_1 + R_4) & q_y(R_2 - \mathrm{i}R_3) \\ q_y(R_2 + \mathrm{i}R_3) & q_z(R_1 - R_4) \end{pmatrix} \tag{S2}$$

For above BCs within a nodal loop, the nodal structure solution of $k \cdot p$ model precisely gives the tangent of the nodal loop at the BC. For example, $q_y = 0, q_z = 0$ is the nodal structure solution of Eq. S2, namely, the corresponding nodal line is along $x$ direction (vertical to HSL G). So the nodal loop must lie in HSPL $k_y = 0$.

For $\mathrm{G}_3$, the $k \cdot p$ model reads

$$H_{\mathrm{G}_3} = \begin{pmatrix} H_{11} & H_{12} \\ H_{21} & H_{22} \end{pmatrix} \tag{S3}$$

The explicit forms of $H_{ij}$ read

$$
\begin{aligned}
H_{11} =& q_z(R_1 + R_7 + q_z(R_2 + R_8)) \\
& + q_y^2(R_3 + R_9) + q_x^2(R_4 + R_{10}), \\
H_{12} =& q_x \cdot q_y(R_5 - \mathrm{i}R_6), \\
H_{21} =& q_x \cdot q_y(R_5 + \mathrm{i}R_6), \\
H_{22} =& q_z(R_1 - R_7 + q_z(R_2 - R_8)) \\
& + q_y^2(R_3 - R_9) + q_x^2(R_4 - R_{10}).
\end{aligned}
$$

Eq. S3 has two nodal structure solutions in the forms of curve equation. The first solution, $q_x = 0, R_9 \cdot q_y^2 + R_8 \cdot \left(q_z + \frac{R_7}{2R_8}\right)^2 = R_8 \cdot \left(\frac{R_7}{2R_8}\right)^2$, implies a nodal loop within HSPL $k_x = \frac{1}{2}$. The second solution, $q_y = 0, R_{10} \cdot q_x^2 + R_8 \cdot \left(q_z + \frac{R_7}{2R_8}\right)^2 = R_8 \cdot \left(\frac{R_7}{2R_8}\right)^2$, implies a nodal loop within HSPL $k_y = 0$. So the $k \cdot p$ model for $G_3$ indicates that a nodal loop within $k_x = \frac{1}{2}$ and a nodal loop within $k_y = 0$ touch at the BC in HSL G to compose nodal chain structure.

Table S1: The fitted model parameters, $R_i$ for the $k \cdot p$ models around the BCs $G_1$, $G_2$ and $G_3$. The units of these parameters are in THz. Note that there is freedom in choosing $R_2$ and $R_3$ for the former two BCs, as well as in choosing $R_5$ and $R_6$ for the last BC. This freedom can be restricted by including higher-order $k \cdot p$ terms.

| $k \cdot p$ model | $R_1$ | $R_2^2 + R_3^2$ | $R_4$ |
|---|---|---|---|
| $H_{G_1}$ | 0.840123 | 8.41 | 0.203818 |
| $H_{G_2}$ | 0.380772 | 0.403360 | −1.371847 |
| | $R_1$ | $R_2$ | $R_3$ |
| | −0.0315 | −0.045123 | −0.557407 |
| $H_{G_3}$ | $R_4$ | $R_5^2 + R_6^2$ | $R_7$ |
| | −20.817893 | 4.407191 | −0.884446 |
| | $R_8$ | $R_9$ | $R_{10}$ |
| | 1.357454 | −0.377451 | 3.739920 |

These $k \cdot p$ model parameters of BCs are detailed in Table S1. As shown in Figure S1 (a-f), we compare the 3D dispersion near the identified BCs with nodal loop trajectory near

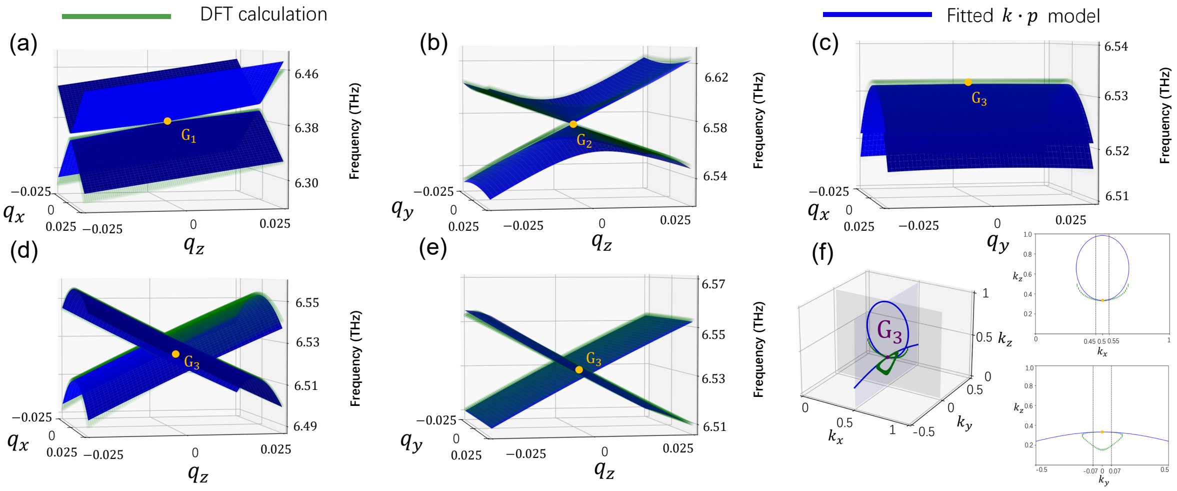


Figure S1: (a-f) Comparison of the 3D dispersion near BCs of Hopf-link structure in $Ga_5(PS)_3$ using fitted $k \cdot p$ model and first-principles calculations. The real-valued parameters of $k \cdot p$ model for BCs are detailed in Table S1. (a-b) The 3D dispersion centered at $G_1$ on $q_{xz}$ plane and $G_2$ on $q_{yz}$ plane, respectively. (c-e) The 3D dispersion centered at $G_3$ on $q_{xy}$, $q_{xz}$ and $q_{yz}$ planes, respectively. (f) Comparison of the nodal loop trajectory near $G_3$ using fitted $k \cdot p$ model in Eq. S3 and using first-principles calculation in 3D BZ. The two nodal loop trajectories that compose the nodal chain in $k_x = \frac{1}{2}$ and $k_y = 0$ from first-principles results correspond to a hyperbola and an ellipse nodal structure solution near $G_3$ obtained by the $k \cdot p$ model, respectively. The first solution of the $k \cdot p$ model, $q_x = 0, R_9 \cdot q_y^2 + R_8 \cdot \left(q_z + \frac{R_7}{2R_8}\right)^2 = R_8 \cdot \left(\frac{R_7}{2R_8}\right)^2$, is a hyperbola in $k_x = \frac{1}{2}$, which fits very well in the interval $k_y \in [-0.07, 0.07]$. The second solution of the $k \cdot p$ model, $q_y = 0, R_{10} \cdot q_x^2 + R_8 \cdot \left(q_z + \frac{R_7}{2R_8}\right)^2 = R_8 \cdot \left(\frac{R_7}{2R_8}\right)^2$, is an ellipse in $k_y = 0$, which fits very well in the interval $k_x \in [0.45, 0.55]$.

BC $G_3$ using fitted $k \cdot p$ model (shown in blue) and first-principles calculation (shown in green). We find that the 3D dispersion near BCs $G_2$ obtained from the $k \cdot p$ model and from first-principles results, fits very well within the interval of $|\Delta q| \leq 0.025$. For BCs $G_1$ and $G_3$, the deviation becomes slightly larger as $\Delta q$ increases. Next, we consider nodal loop trajectory near $G_3$. For BC $G_3$ within nodal chain, we substitute the parameters from Table S1 into two nodal structure solutions of Eq S3. As shown in Figure S1 (f), we find two nodal loop trajectory to compose the nodal chain in $k_x = \frac{1}{2}$ and $k_y = 0$ from first-principles results correspond to a hyperbola and an ellipse nodal structure solution near $G_3$ obtained from the $k \cdot p$ model, respectively. In addition, the nodal loop trajectory near $G_3$ in the interval $k_y \in [-0.07, 0.07]$ in $k_x = \frac{1}{2}$ and $k_x \in [0.45, 0.55]$ in $k_y = 0$, obtained from the $k \cdot p$ model,

fits very well with first-principles results. It is worth mentioning that the predicted nodal structures based on CRs are further confirmed by our effective $k \cdot p$ model, which could be used in future studies to investigate the effects of external fields on the behavior of these BCs and the associated nodal loops.

# S3. Seven representative materials with relatively clean phonon Hopf-link structure

*Brief summary.*—For the other seven representative materials with relatively clean Hopf-link structures mentioned in the main text, this section provides the necessary data, including irreps of the BCs within HSLs, the elucidation of the Hopf-link structure, and the character tables of the little groups of HSLs.

## A. Calculation results of materials

We list specified information of these Hopf-link materials in Table S2. For each material in Table S2, we give calculation results, including Hopf-link type, Space group (SG) and chemical formula, the HSL for diagnosing Hopf-link structure, the equations of two HSPLs for containing Hopf-link structure, branches of bands, the coordinates, frequencies and irreps of BCs. The naming convention and the coordinates of HSLs follow those on the Bilbao server.[8]

## B. Hopf-link structure of materials

For each material, we show crystal structure, phonon spectrum, phonon dispersion along the HSL and Hopf-link structure in the BZ.

Table S2: The information of representative materials with relatively clean Hopf-link structure. The first column provides the categories of Hopf-link structures. The second column lists the corresponding SGs. The materials are given in the third column. The fourth, fifth, and sixth columns contain the positions of HSLs and two HSPLs. The seventh column contains the branches of bands. The eighth, ninth, and tenth columns contain the coordinates, frequencies, and irreps of BCs.

| TYPE | SG | Formula | HSL | HSPL1 | HSPL2 | Branches | Band Crossings | Frequency (THz) | Irrep |
|---|---|---|---|---|---|---|---|---|---|
| I | 33 | $LiCaS_2$ | LD $(0,0,w)$ | $k_x=0$ | $k_y=0$ | 8th-9th | $LD_1$ (0, 0, 0.160) | 3.30 | $1\oplus4$ |
| | | | | | | | $LD_2$ (0, 0, 0.282) | 3.06 | $1\oplus3$ |
| | | | | | | | $LD_3$ (0, 0, 0.409) | 2.90 | $2\oplus3$ |
| I | 33 | $LiInSe_2$ | LD $(0,0,w)$ | $k_x=0$ | $k_y=0$ | 8th-9th | $LD_1$ (0, 0, 0.225) | 1.71 | $1\oplus4$ |
| | | | | | | | $LD_2$ (0, 0, 0.377) | 1.61 | $1\oplus3$ |
| | | | | | | | $LD_3$ (0, 0, 0.434) | 1.57 | $2\oplus3$ |
| I | 41 | $Ca_2Al_2Si(HO_4)_2$ | SM $(0,0,w)$ | $k_x=0$ | $k_y=0$ | 48th-49th | $SM_1$ (0, 0, 0.304) | 7.62 | $2\oplus3$ |
| | | | | | | | $SM_2$ (0, 0, 0.540) | 7.82 | $2\oplus4$ |
| | | | | | | | $SM_3$ (0, 0, 0.826) | 7.46 | $1\oplus4$ |
| I | 60 | $Ca_7GeN_6$ | SM $(u, 0, 0)$ | $k_y=0$ | $k_z=0$ | 132th-133th | $SM_1$ (0.068, 0, 0) | 11.75 | $\{1\}\oplus\{4\}$ |
| | | | | | | | $SM_2$ (0.116, 0, 0) | 11.76 | $\{1\}\oplus\{3\}$ |
| | | | | | | | $SM_3$ (0.398, 0, 0) | 11.68 | $\{2\}\oplus\{3\}$ |
| I | 61 | $Al(HO)_3$ | SM $(u, 0, 0)$ | $k_y=0$ | $k_z=0$ | 124th-125th | $SM_1$ (0.113, 0, 0) | 30.28 | $\{1\}\oplus\{4\}$ |
| | | | | | | | $SM_2$ (0.252, 0, 0) | 30.36 | $\{2\}\oplus\{4\}$ |
| | | | | | | | $SM_3$ (0.284, 0, 0) | 30.38 | $\{1\}\oplus\{4\}$ |
| I | 70 | $NaNd(GaS_2)_4$ | SM $(u, 0, 0)$ | $k_y=0$ | $k_z=0$ | 54th-55th | $SM_1$ (0.074, 0, 0) | 3.78 | $\{1\}\oplus\{4\}$ |
| | | | | | | | $SM_2$ (0.384, 0, 0) | 3.70 | $\{1\}\oplus\{3\}$ |
| | | | | | | | $SM_3$ (0.880, 0, 0) | 3.71 | $\{1\}\oplus\{4\}$ |
| II | 26 | $RbTh_3F_{13}$ | H $(0,\frac{1}{2},w)$ | $k_x=0$ | $k_y=\frac{1}{2}$ | 87th-88th<br>88th-89th | $H_1$ (0, 0.5, 0.100) | 10.57 | $1\oplus3$ |
| | | | | | | | $H_2$ (0, 0.5, 0.152) | 10.65 | $1\oplus4$ |
| | | | | | | | $H_3$ (0, 0.5, 0.253) | 10.59 | $3\oplus4$ |

## (1). $LiCaS_2$

$LiCaS_2$[9] in SG 33 has 3 BCs, named $LD_1$, $LD_2$, and $LD_3$ in HSL LD $(0,0,w)$, respectively. The coordinates, frequencies, and irreps of these BCs are listed in Table S2. According to the nodal loop location corresponding to BCs listed in Table S13, $LD_1$, $LD_2$, and $LD_3$ must lie in a nodal loop within $k_x = 0$, $k_y = 0$, and $k_z = 0$, respectively. As shown in Figure S2 (e), the blue nodal loop within HSPL $k_x = 0$ from both $LD_1$ and $LD_3$ is nested with the yellow nodal loop from $LD_2$ within HSPL $k_y = 0$ to compose the type-I loop-loop structure.

## (2). $LiInSe_2$

$LiInSe_2$[10] in SG 33 has 3 BCs, named by $LD_1$, $LD_2$ and $LD_3$ in HSL LD $(0,0,w)$, respectively. The coordinates, frequencies and irreps of these BCs are listed in Table S2. According to the nodal loop location corresponding to BCs listed in Table S13, $LD_1$, $LD_2$ and $LD_3$ must lie in a nodal loop within $k_x = 0$, $k_y = 0$ and $k_x = 0$, respectively. As shown in Figure S3 (e),

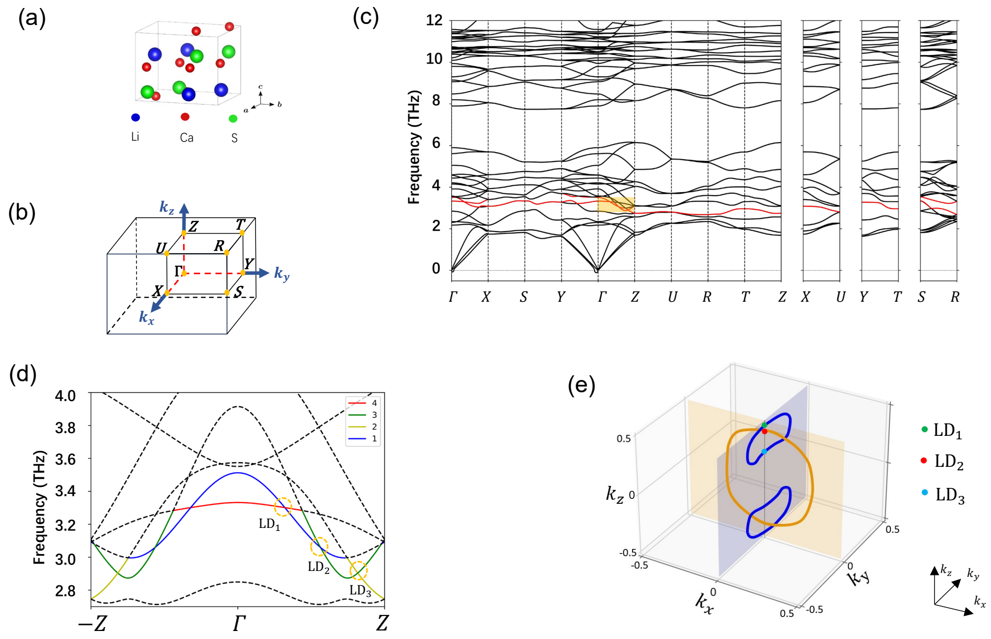

Figure S2: The Hopf-link phonon of $LiCaS_2$ (SG 33). (a) The crystal structure of $LiCaS_2$. (b) The bulk BZ of SG 33. (c) The phonon spectrum between 0.0 and 12.0 THz. (d) The phonon dispersion between 2.8 and 4.0 THz along the $-Z-\Gamma-Z$ path in the BZ. (e) The loop-loop structure in the BZ.

the blue nodal loop within HSPL $k_x = 0$ from both $LD_1$ and $LD_3$ is nested with the yellow nodal loop from $LD_2$ within HSPL $k_y = 0$ to compose the type-I loop-loop structure.

**(3).** $Ca_2Al_2Si(HO_4)_2$

$Ca_2Al_2Si(HO_4)_2$ in SG 41 has 3 BCs, named by $SM_1$, $SM_2$ and $SM_3$ in HSL SM $(0, 0, w)$, respectively. The coordinates, frequencies and irreps of these BCs are listed in Table S2. According to the nodal loop location corresponding to BCs listed in Table S13, $SM_1$, $SM_2$ and $SM_3$ must lie in a nodal loop within $k_y = 0$, $k_x = 0$ and $k_y = 0$, respectively. As shown in Figure S4 (e), the blue nodal loop within HSPL $k_y = 0$ from both $SM_1$ and $SM_3$ is nested with the yellow nodal loop from $SM_2$ within HSPL $k_x = 0$ to compose the type-I loop-loop structure.

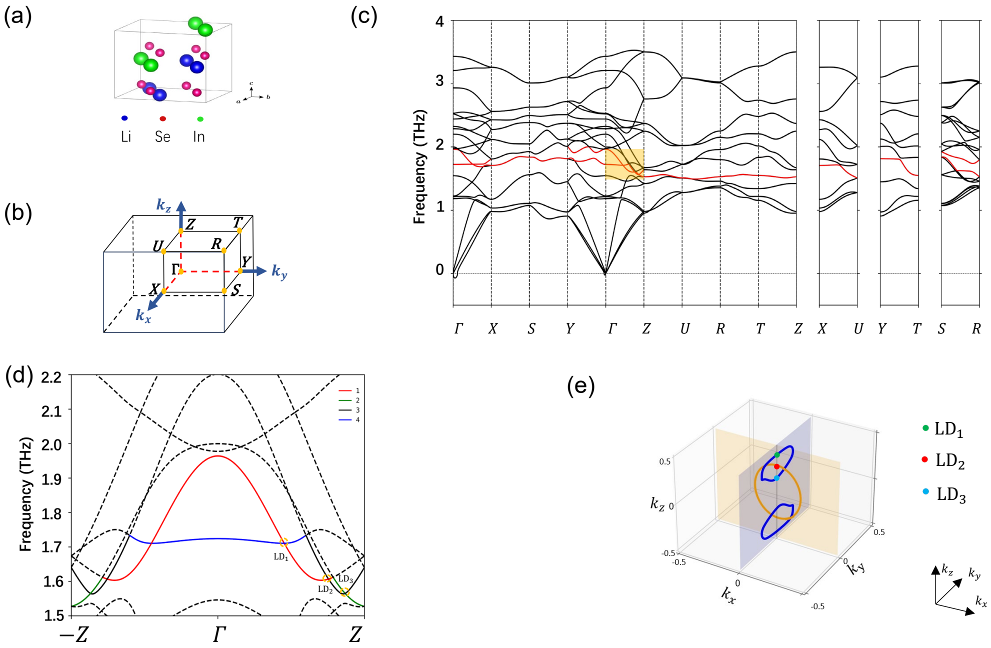

Figure S3: The Hopf-link phonon of $LiInSe_2$ (SG 33). (a) The crystal structure of $LiInSe_2$. (b) The bulk BZ of SG 33. (c) The phonon spectrum between 0.0 and 4.0 THz. (d) The phonon dispersion between 1.5 and 2.2 THz along the $-Z-\Gamma-Z$ path in the BZ. (e) The loop-loop structure in the BZ.

### (4). $Ca_7GeN_6$

$Ca_7GeN_6$[11] in SG 60 has 3 BCs, named by $SM_1$, $SM_2$ and $SM_3$ in HSL SM $(u, 0, 0)$, respectively. The coordinates, frequencies and irreps of these BCs are listed in Table S2. According to the nodal loop location corresponding to BCs listed in Table S13, $SM_1$, $SM_2$ and $SM_3$ must lie in a nodal loop within $k_y = 0$, $k_z = 0$ and $k_y = 0$, respectively. As shown in Figure S5(e), the blue nodal loop within HSPL $k_y = 0$ from both $SM_1$ and $SM_3$ is nested with the yellow nodal loop from $SM_2$ within HSPL $k_z = 0$ to compose the type-I loop-loop structure.

### (5). $Al(HO)_3$

$Al(HO)_3$ in SG 61 has 3 BCs, named by $SM_1$, $SM_2$ and $SM_3$ in HSL SM $(u, 0, 0)$, respectively. The coordinates, frequencies and irreps of these BCs are listed in Table S2. According to the nodal loop location corresponding to BCs listed in Table S13, $SM_1$, $SM_2$ and $SM_3$ must lie in a nodal loop within $k_y = 0$, $k_z = 0$ and $k_y = 0$, respectively. As is shown in Figure

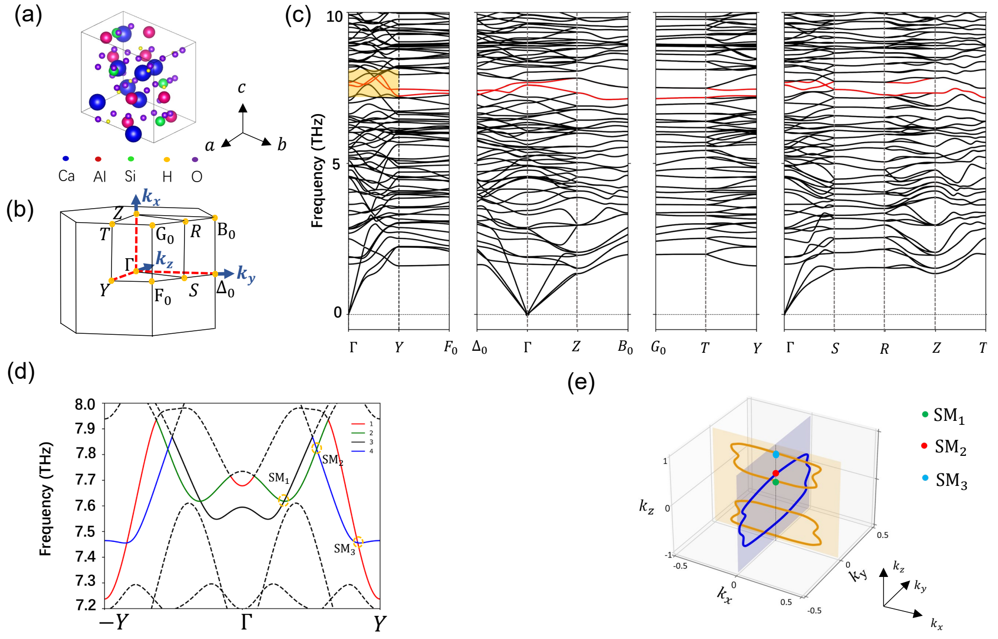


Figure S4: The Hopf-link phonon of $Ca_2Al_2Si(HO_4)_2$ (SG 41). (a) The crystal structure of $Ca_2Al_2Si(HO_4)_2$. (b) The bulk BZ of SG 41. (c) The phonon spectrum between 0.0 and 10.0 THz. (d) The phonon dispersion between 7.2 and 8.0 THz along the $-Y - \Gamma - Y$ path in the BZ. (e) The loop-loop structure in the BZ.

S6(e), the blue nodal loop within HSPL $k_y = 0$ from both $SM_1$ and $SM_3$ is nested with the yellow nodal loop from $SM_2$ within HSPL $k_z = 0$ to compose the type-I loop-loop structure.

### (6). $NaNd(GaS_2)_4$

$NaNd(GaS_2)_4$[12] in SG 70 has 3 BCs, named by $SM_1$, $SM_2$ and $SM_3$ in HSL SM $(u, 0, 0)$, respectively. The coordinates, frequencies and irreps of these BCs are listed in Table S2. According to the nodal loop location corresponding to BCs listed in Table S13, $SM_1$, $SM_2$ and $SM_3$ must lie in a nodal loop within $k_y = 0$, $k_z = 0$ and $k_y = 0$, respectively. As shown in Figure S7(e), the blue nodal loop within HSPL $k_y = 0$ from both $SM_1$ and $SM_3$ is nested with the yellow nodal loop from $SM_2$ within HSPL $k_z = 0$ to compose the type-I loop-loop structure.

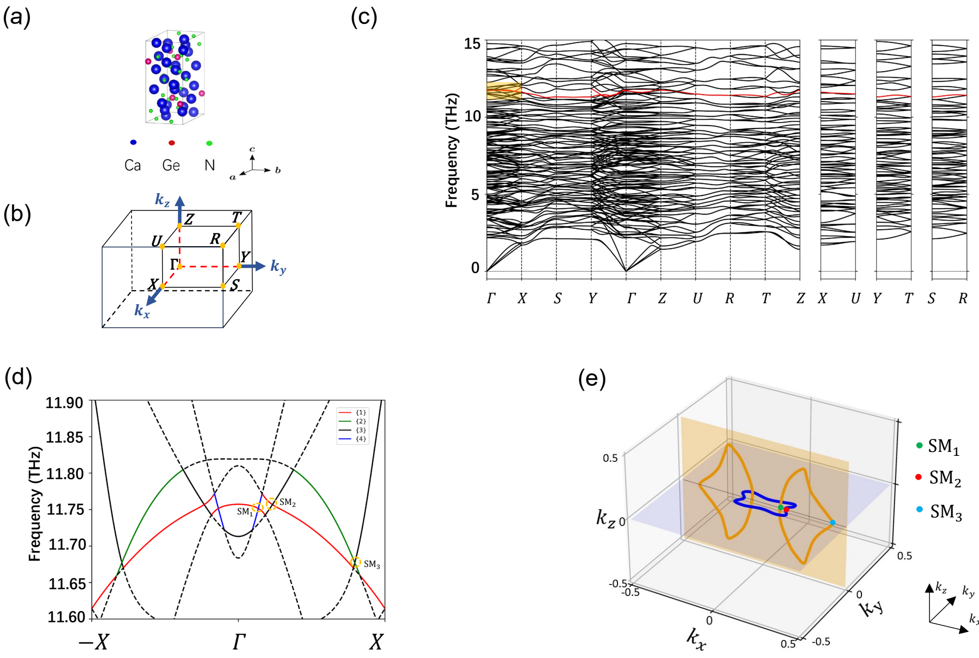


Figure S5: The Hopf-link phonon of $Ga_7GeN_6$ (SG 60). (a) The crystal structure of $Ga_7GeN_6$. (b) The bulk BZ of SG 60. (c) The phonon spectrum between 0.0 and 15.0 THz. (d) The phonon dispersion between 11.6 and 11.9 THz along the $-X - \Gamma - X$ path in the BZ. (e) The loop-loop structure in the BZ.

## (7). $RbTh_3F_{13}$

$RbTh_3F_{13}$[13] in SG 26 has 3 BCs, named by $H_1$, $H_2$ and $H_3$ in HSL H $(0, \frac{1}{2}, w)$, respectively. The coordinates, frequencies and irreps of these BCs are listed in Table S2. According to the nodal loop location and nodal chain location corresponding to BCs listed in Table S14, $H_1$ and $H_2$ must lie in a nodal loop within $k_x = 0$ and $k_y = \frac{1}{2}$,respectively, while $H_3$ is a touching point of two nodal loops within $k_x = 0$ and $k_y = \frac{1}{2}$, forming a nodal chain structure. As shown in Figure S8(e), $H_1$ lies in the nodal loop (blue) within HSPL $k_x = 0$ and $H_3$ lies in the nodal chain. $H_2$ lies in the nodal loop (yellow) within HSPL $k_y = \frac{1}{2}$ which is nested with the nodal loop (blue) within HSPL $k_x = 0$ to compose the type-II loop-chain structure.

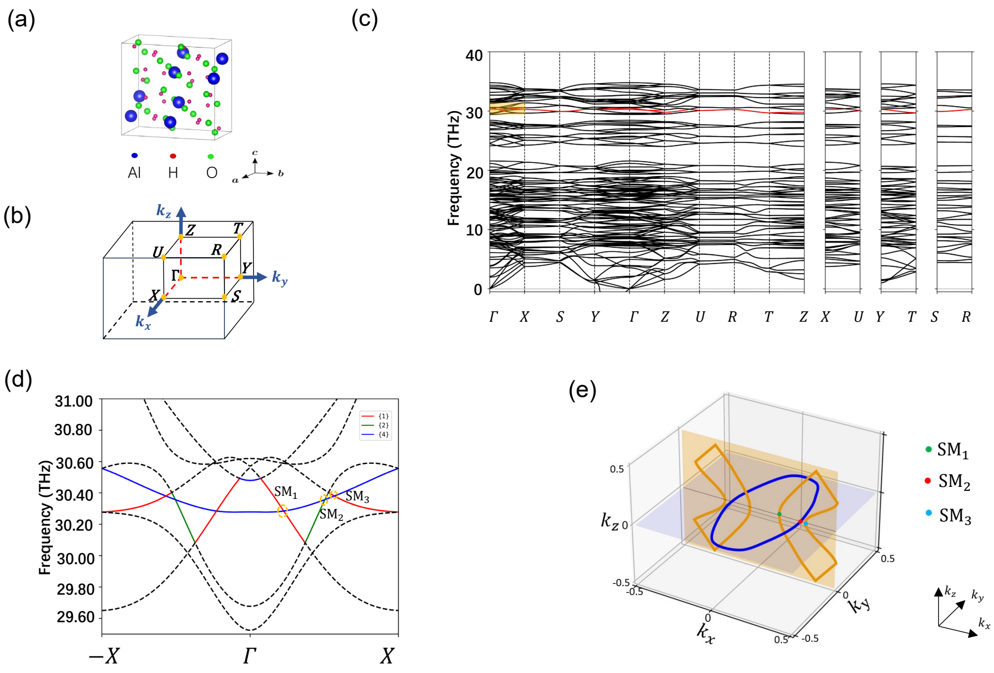

Figure S6: The Hopf-link phonon of $Al(HO)_3$ (SG 61). (a) The crystal structure of $Al(HO)_3$. (b) The bulk BZ of SG 61. (c) The phonon dispersion between 0.0 and 40.0 THz. (d) The phonon dispersion between 29.6 and 31.0 THz along the $-X-\Gamma-X$ path in the BZ. (e) The loop-loop structure in the BZ.

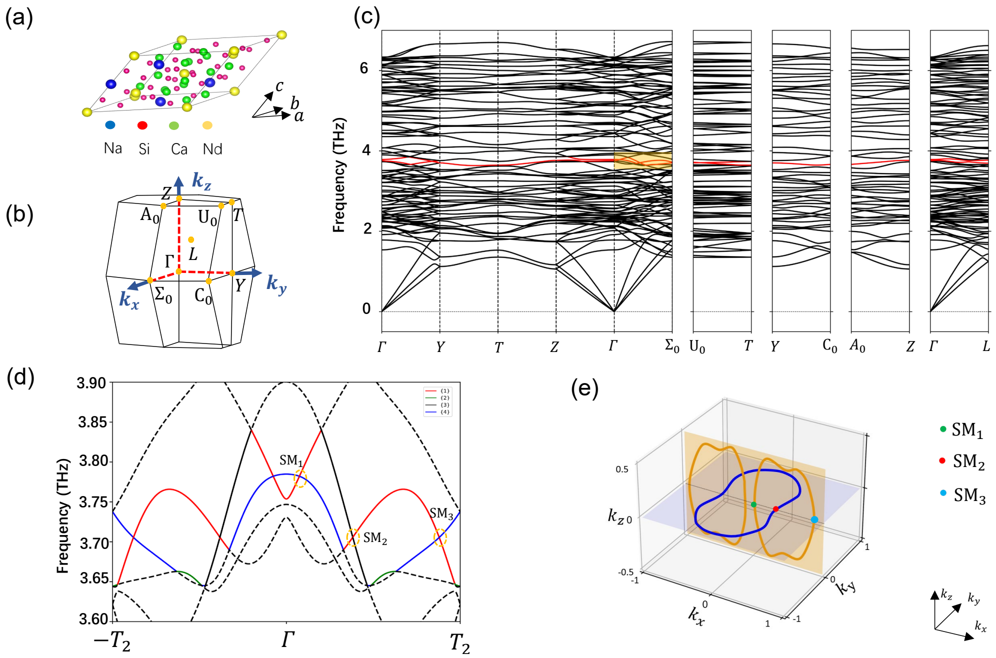

Figure S7: The Hopf-link phonon of $NaNd(GaS_2)_4$ (SG 70). (a) The crystal structure of $NaNd(GaS_2)_4$. (b) The bulk BZ of SG 70. (c) The phonon spectrum between 0.0 and 7.0 THz. (d) The phonon dispersion between 3.6 and 3.9 THz along the $-T_2-\Gamma-T_2$ path in the BZ. The convention coordinate of $T_2$ is $(1,0,0)$. (e) The loop-loop structure in the BZ.

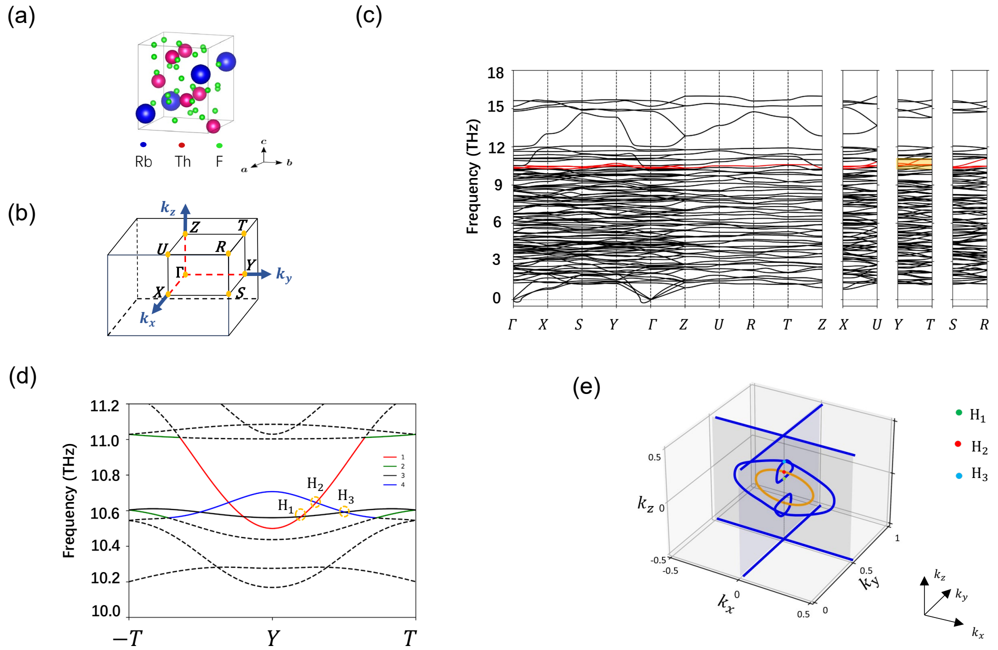


Figure S8: The Hopf-link phonon of $RbTh_3F_{13}$ (SG 26). (a) The crystal structure of $RbTh_3F_{13}$. (b) The bulk BZ of SG 26. (c) The phonon spectrum between 0.0 and 18.0 THz. (d) The phonon dispersion between 10.0 and 11.2 THz along the $-T-Y-T$ path in the BZ. (e) The loop-chain structure in the BZ.

## C. The character tables of little groups of HSLs

We list the character tables of little groups of HSLs in SGs corresponding to eight Hopf-link materials mentioned in the main text. Taking the character tables of HSL G $(\frac{1}{2}, 0, w)$ in SG 25 from Table S3 as an example, the first column contains matrix presentations of four operations of the little groups of HSL G, which consist of two parts: a rotation part represented by a three-dimensional matrix and a translation part represented by a three-dimensional column vector. The second to fifth columns contain four irreps, labeled as 1, 2, 3, and 4 respectively, and the characters of the little groups corresponding to these irreps.

Table S3: Matrices of the representations of the little group of HSL G $(\frac{1}{2}, 0, w)$ in SG 25.

| Matrix presentation | 1 | 2 | 3 | 4 |
|---|---|---|---|---|
| $\begin{pmatrix} 1 & 0 & 0 & 0.0 \\ 0 & 1 & 0 & 0.0 \\ 0 & 0 & 1 & 0.0 \end{pmatrix}$ | 1 | 1 | 1 | 1 |
| $\begin{pmatrix} -1 & 0 & 0 & 0.0 \\ 0 & -1 & 0 & 0.0 \\ 0 & 0 & 1 & 0.0 \end{pmatrix}$ | 1 | 1 | $-1$ | $-1$ |
| $\begin{pmatrix} 1 & 0 & 0 & 0.0 \\ 0 & -1 & 0 & 0.0 \\ 0 & 0 & 1 & 0.0 \end{pmatrix}$ | 1 | $-1$ | 1 | $-1$ |
| $\begin{pmatrix} -1 & 0 & 0 & 0.0 \\ 0 & 1 & 0 & 0.0 \\ 0 & 0 & 1 & 0.0 \end{pmatrix}$ | 1 | $-1$ | $-1$ | 1 |

Table S4: Matrices of the representations of the little group of HSL H $(0, \frac{1}{2}, w)$ in SG 26.

| Matrix presentation | 1 | 2 | 3 | 4 |
|---|---|---|---|---|
| $\begin{pmatrix} 1 & 0 & 0 & 0.0 \\ 0 & 1 & 0 & 0.0 \\ 0 & 0 & 1 & 0.0 \end{pmatrix}$ | 1 | 1 | 1 | 1 |
| $\begin{pmatrix} -1 & 0 & 0 & 0.0 \\ 0 & -1 & 0 & 0.0 \\ 0 & 0 & 1 & 0.5 \end{pmatrix}$ | −1 | −1 | 1 | 1 |
| $\begin{pmatrix} 1 & 0 & 0 & 0.0 \\ 0 & -1 & 0 & 0.0 \\ 0 & 0 & 1 & 0.5 \end{pmatrix}$ | −1 | 1 | −1 | 1 |
| $\begin{pmatrix} -1 & 0 & 0 & 0.0 \\ 0 & 1 & 0 & 0.0 \\ 0 & 0 & 1 & 0.0 \end{pmatrix}$ | 1 | −1 | −1 | 1 |

Table S5: Matrices of the representations of the little group of of HSL LD $(0, 0, w)$ in SG 33.

| Matrix presentation | 1 | 2 | 3 | 4 |
|---|---|---|---|---|
| $\begin{pmatrix} 1 & 0 & 0 & 0.0 \\ 0 & 1 & 0 & 0.0 \\ 0 & 0 & 1 & 0.0 \end{pmatrix}$ | 1 | 1 | 1 | 1 |
| $\begin{pmatrix} -1 & 0 & 0 & -1.0 \\ 0 & -1 & 0 & 0.0 \\ 0 & 0 & 1 & 0.5 \end{pmatrix}$ | −1 | −1 | 1 | 1 |
| $\begin{pmatrix} -1 & 0 & 0 & -0.5 \\ 0 & 1 & 0 & -0.5 \\ 0 & 0 & 1 & 0.5 \end{pmatrix}$ | −1 | 1 | −1 | 1 |
| $\begin{pmatrix} 1 & 0 & 0 & -0.5 \\ 0 & -1 & 0 & 0.5 \\ 0 & 0 & 1 & 0.0 \end{pmatrix}$ | 1 | −1 | −1 | 1 |

Table S6: Matrices of the representations of the little group of HSL SM $(0, 0, w)$ in SG 41.

| Matrix presentation | 1 | 2 | 3 | 4 |
|---|---|---|---|---|
| $\begin{pmatrix} 1 & 0 & 0 & 0.0 \\ 0 & 1 & 0 & 0.0 \\ 0 & 0 & 1 & 0.0 \end{pmatrix}$ | 1 | 1 | 1 | 1 |
| $\begin{pmatrix} -1 & 0 & 0 & 0.0 \\ 0 & 0 & 1 & 0.0 \\ 0 & 1 & 0 & 0.0 \end{pmatrix}$ | 1 | 1 | $-1$ | $-1$ |
| $\begin{pmatrix} 1 & 0 & 0 & 0.5 \\ 0 & 0 & 1 & 0.5 \\ 0 & 1 & 0 & -0.5 \end{pmatrix}$ | 1 | $-1$ | 1 | $-1$ |
| $\begin{pmatrix} -1 & 0 & 0 & -0.5 \\ 0 & 1 & 0 & -0.5 \\ 0 & 0 & 1 & 0.5 \end{pmatrix}$ | 1 | $-1$ | $-1$ | 1 |

Table S7: Matrices of the representations of the little group of HSL SM $(u, 0, 0)$ in SG 60.

| Matrix presentation | {1} | {2} | {3} | {4} |
|---|---|---|---|---|
| $\begin{pmatrix} 1 & 0 & 0 & 0.0 \\ 0 & 1 & 0 & 0.0 \\ 0 & 0 & 1 & 0.0 \end{pmatrix}$ | 1 | 1 | 1 | 1 |
| $\begin{pmatrix} 1 & 0 & 0 & -0.5 \\ 0 & -1 & 0 & -0.5 \\ 0 & 0 & -1 & 0.0 \end{pmatrix}$ | $-1$ | $-1$ | 1 | 1 |
| $\begin{pmatrix} 1 & 0 & 0 & 0.0 \\ 0 & -1 & 0 & 0.0 \\ 0 & 0 & 1 & -0.5 \end{pmatrix}$ | 1 | $-1$ | 1 | $-1$ |
| $\begin{pmatrix} 1 & 0 & 0 & 0.5 \\ 0 & 1 & 0 & -0.5 \\ 0 & 0 & -1 & 0.5 \end{pmatrix}$ | $-1$ | 1 | 1 | $-1$ |

Table S8: Matrices of the representations of the little group of HSL SM $(u, 0, 0)$ in SG 61.

| Matrix presentation | {1} | {2} | {3} | {4} |
|---|---|---|---|---|
| $\begin{pmatrix} 1 & 0 & 0 & 0.0 \\ 0 & 1 & 0 & 0.0 \\ 0 & 0 & 1 & 0.0 \end{pmatrix}$ | 1 | 1 | 1 | 1 |
| $\begin{pmatrix} 1 & 0 & 0 & -0.5 \\ 0 & -1 & 0 & 0.5 \\ 0 & 0 & -1 & 0.0 \end{pmatrix}$ | −1 | −1 | 1 | 1 |
| $\begin{pmatrix} 1 & 0 & 0 & 0.0 \\ 0 & -1 & 0 & 0.5 \\ 0 & 0 & 1 & 0.5 \end{pmatrix}$ | 1 | −1 | 1 | −1 |
| $\begin{pmatrix} 1 & 0 & 0 & 0.5 \\ 0 & 1 & 0 & 0.0 \\ 0 & 0 & -1 & 0.5 \end{pmatrix}$ | −1 | 1 | 1 | −1 |

Table S9: Matrices of the representations of the little group of HSL SM $(u, 0, 0)$ in SG 70.

| Matrix presentation | {1} | {2} | {3} | {4} |
|---|---|---|---|---|
| $\begin{pmatrix} 1 & 0 & 0 & 0.0 \\ 0 & 1 & 0 & 0.0 \\ 0 & 0 & 1 & 0.0 \end{pmatrix}$ | 1 | 1 | 1 | 1 |
| $\begin{pmatrix} -1 & -1 & -1 & 0.0 \\ 0 & 0 & 1 & 0.0 \\ 0 & 1 & 0 & 0.0 \end{pmatrix}$ | 1 | 1 | −1 | −1 |
| $\begin{pmatrix} 0 & 0 & -1 & 0.25 \\ 1 & 1 & 1 & -0.75 \\ -1 & 0 & 0 & 0.25 \end{pmatrix}$ | −1 | 1 | −1 | 1 |
| $\begin{pmatrix} 0 & -1 & 0 & 0.25 \\ -1 & 0 & 0 & 0.25 \\ 1 & 1 & 1 & -0.75 \end{pmatrix}$ | −1 | 1 | 1 | −1 |

# S4. List of materials with phonon Hopf-link structure

*Brief summary.*—In this section, we first introduce our strategy for searching for Type-I/II loop-loop, Type-I/II loop-chain, Type-I/II inter-chain, and intra-chain structures by identifying BCs in HSLs, respectively. Then we provide detailed information on all candidate materials identified through our search, including the types of Hopf-link structures, SGs, material IDs from the online database of the Materials Project,[14] chemical formulas, HSLs, and branches of bands.

*The strategy for loop-loop structure.*–A loop-loop structure requires identifying BCs that lie within the loops of neighboring HSPLs. The HSPLs that accommodate the two loops are distinct while ensuring that the loops are nested within each other. The locations of the nested nodal loops and their corresponding irreps of BCs are listed in Table S13.

The screening of the Type-I loop-loop structure is divided into three steps: first, we extract the BCs from the bands (band indices: $n$ and $n+1$), as indicated by BC1; second, we ensure that the irreps of BC1 correspond exclusively to the irreps listed in Table S13; third, we check whether the loops are nested within each other in the BZ.

The screening of the Type-II loop-loop structure is divided into three steps: first, extract BCs from bands (band indices: $n$, $n+1$), indicated by BC1, and extract BCs from bands (band indices: $n+1$, $n+2$), indicated by BC2; second, ensure that all irreps of BC1 and BC2 correspond exclusively to the irreps listed in Table S13; third, check whether the loops are nested with each other in the BZ.

Based on the above strategy, we find 92 materials with loop-loop structures (either of type-I or of type-II) shown in Table S10.

Table S10: List of materials with loop-loop structure in phonon spectra. For each material, they are characterized by the type of Hopf-link structure, SG, the material ID from the online database of Materials Project,[14] chemical formula, the HSL and branches of bands.

| Type | SG | Material ID | Formula | HSL | Branches |
|---|---|---|---|---|---|
| I | 29 | mp-554856 | $Na_2Si_2O_5$ | LD | 31-32 |
| I | 31 | mp-18073 | $K_7TaAs_4$ | LD | 28-29 |
| I | 32 | mp-669414 | $HfPbO_3$ | LD | 58-59 |
| I | 33 | mp-3647 | $LiGaS_2$ | LD | 8-9 |
| I | 33 | mp-20310 | $LiInSe_2$ | LD | 8-9 |
| I | 33 | mp-559689 | $LiAlSiO_4$ | LD | 10-11 |
| I | 38 | mp-27376 | $Rb_6Si_{10}O_{23}$ | SM | 66-67 |
| I | 41 | mp-686748 | $Ca_2Al_2Si(HO_4)_2$ | SM | 48-49 |
| I | 51 | mp-600038 | $SiO_2$ | DT | 30-31 |
| I | 53 | mp-28741 | $CuSe_3Br$ | DT | 22-23 |
| I | 57 | mp-17913 | $Tb_2SiSeO_4$ | DT | 30-31 |
| I | 57 | mp-18466 | $Nd_2SiSeO_4$ | G | 30-31 |
| I | 57 | mp-18610 | $Sm_2SiSeO_4$ | G | 30-31 |
| I | 58 | mp-541568 | $Sr_2Li_3NbN_4$ | LD | 66-67 |
| I | 60 | mp-570555 | $Ca_7GeN_6$ | SM | 132-133 |
| I | 61 | mp-626605 | $Al(HO)_3$ | SM | 124-125 |
| I | 62 | mp-1477 | $BaSi_2$ | DT | 4-5 |
| I | 62 | mp-1875 | $TeF_6$ | LD | 80-81 |
| I | 62 | mp-2632 | $TlF_3$ | SM | 30-31 |
| I | 62 | mp-2879 | $SrSnO_3$ | SM | 30-31 |
| I | 62 | mp-2955 | $NaMgF_3$ | DT | 36-37 |
| I | 62 | mp-3196 | $NdGaO_3$ | SM | 52-53 |

to be continued

| Type | SG | Material ID | Formula | HSL | Branches |
|---|---|---|---|---|---|
| I | 62 | mp-3378 | $SrHfO_3$ | SM | 22-23 |
| I | 62 | mp-4438 | $CaSnO_3$ | SM | 54-55 |
| I | 62 | mp-4535 | $PrGaO_3$ | SM | 52-53 |
| I | 62 | mp-5126 | $ZnSO_4$ | LD | 22-23 |
| I | 62 | mp-5616 | $Sr_2P_2O_7$ | LD | 40-41 |
| I | 62 | mp-5837 | $LaGaO_3$ | SM | 54-55 |
| I | 62 | mp-5900 | $Ba_2ZrF_8$ | DT | 20-21 |
| I | 62 | mp-6493 | $CaMgSiO_4$ | LD | 36-37 |
| I | 62 | mp-9625 | $LiMgPO_4$ | DT | 38-39 |
| I | 62 | mp-16927 | $TbNaGeO_4$ | LD | 58-59 |
| I | 62 | mp-17054 | $Cs_3TaS_4$ | DT | 18-19 |
| I | 62 | mp-17975 | $KSrPO_4$ | SM | 34-35 |
| I | 62 | mp-17989 | $K_3PS_4$ | SM | 34-35 |
| I | 62 | mp-18101 | $K_2Cd_3S_4$ | LD | 24-25 |
| I | 62 | mp-18327 | $Ba_2Tl_2O_5$ | SM | 82-83 |
| I | 62 | mp-18334 | $NaHoGeO_4$ | LD | 58-59 |
| I | 62 | mp-18629 | $NaTmGeO_4$ | LD | 32-33 |
| I | 62 | mp-20489 | $SrPbO_3$ | DT | 48-49 |
| I | 62 | mp-23622 | $Sm_3Si_2ClO_8$ | SM | 54-55 |
| I | 62 | mp-24446 | $LiH_2SO_4$ | SM | 6-7 |
| I | 62 | mp-28091 | $In_2(TeO_3)_3$ | SM | 54-55 |
| I | 62 | mp-29883 | $Rb_3PbCl_5$ | SM | 102-103 |
| I | 62 | mp-505089 | $TbLi_4F_8$ | DT | 130-131 |
| I | 62 | mp-558490 | $Tb_3Se_2ClO_8$ | SM | 6-7 |
| I | 62 | mp-558938 | $Zn_4SiTePbO_{10}$ | SM | 8-9 |

to be continued

| Type | SG | Material ID | Formula | HSL | Branches |
|---|---|---|---|---|---|
| I | 62 | mp-697981 | $Cd_3H_2CSeO_8$ | SM | 30-31 |
| I | 62 | mp-755165 | $YScO_3$ | LD | 40-41 |
| I | 62 | mp-756166 | $LaHoO_3$ | SM | 30-31 |
| I | 62 | mp-756290 | $TbGaO_3$ | SM | 30-31 |
| I | 62 | mp-756979 | $Rb_3ClO$ | SM | 6-7 |
| I | 62 | mp-771005 | $LuTa_3O_9$ | SM | 42-43 |
| I | 62 | mp-771957 | $Ta_2PbO_6$ | LD | 56-57 |
| I | 62 | mp-773011 | $Dy_2Ge_2O_7$ | SM | 70-71 |
| I | 64 | mp-17951 | $Cs_4Zn_3F_{10}$ | DT | 40-41 |
| I | 65 | mp-560998 | $SiO_2$ | B | 155-156 |
| I | 67 | mp-7310 | $ZrPbF_6$ | SM | 17-18 |
| I | 70 | mp-14515 | $NaNd(GaS_2)_4$ | SM | 54-55 |
| I | 128 | mp-610738 | $Zr(InBr_3)_2$ | DT | 14-15 |
| I | 131 | mp-639480 | $SiO_2$ | U | 42-43 |
| I | 135 | mp-30959 | LiHS | SM | 42-43 |
| I | 136 | mp-6491 | $Na_2ZnP_2O_7$ | DT | 8-9 |
| I | 136 | mp-698032 | $Na_3H_7Ru$ | SM | 30-31 |
| I | 185 | mp-556647 | $Ba_5Re_3ClO_{15}$ | U | 22-23 |
| I | 190 | mp-557407 | $K_3NaUC_3O_{11}$ | LD | 25-26 |
| II | 29 | mp-559138 | $Ba_2Zn(BO_3)_2$ | G | 131-133 |
| II | 33 | mp-554529 | $Ba_2TiO_4$ | LD | 147-149; 148-150 |
| II | 39 | mp-532443 | $Li_5V_5Cl_{16}$ | A | 38-40 |
| II | 44 | mp-638070 | $LiB_{13}C_2$ | LD | 88-90 |
| II | 46 | mp-633099 | $Sb_2Pb_2O_7$ | LD | 22-24; 43-45 |
| II | 51 | mp-639463 | $SiO_2$ | H | 37-39 |

to be continued

| Type | SG | Material ID | Formula | HSL | Branches |
|---|---|---|---|---|---|
| II | 53 | mp-556631 | $KZrSnF_7$ | C | 97-99 |
| II | 57 | mp-3311 | $SrUO_4$ | SM | 41-43 |
| II | 57 | mp-16903 | $SrSbF_5$ | SM | 73-75 |
| II | 57 | mp-17834 | $La_2SiSeO_4$ | SM | 51-53 |
| II | 57 | mp-759925 | $Zn_2Hg_2H_2Se_2O_{11}$ | SM | 114-116 |
| II | 58 | mp-541568 | $Sr_2Li_3NbN_4$ | DT | 60-62 |
| II | 61 | mp-10368 | CoPSe | SM | 68-70 |
| II | 61 | mp-556216 | $HIO_3$ | SM | 107-109 |
| II | 61 | mp-561533 | SbOF | SM | 91-93 |
| II | 62 | mp-778924 | $ZnSeO_4$ | LD | 7-9 |
| II | 63 | mp-18619 | $Na_2Ge_2Se_5$ | SM | 16-18 |
| II | 63 | mp-754073 | $Lu_2TiO_5$ | DT | 14-16 |
| II | 63 | mp-973391 | $LiSiB_6$ | DT | 87-89 |
| II | 67 | mp-760489 | $PH_6NO_2$ | B | 13-15 |
| II | 74 | mp-4103 | $Sr_2Sb_2O_7$ | DT | 30-32 |
| II | 74 | mp-23768 | $AlZnH_4O_2F_5$ | DT | 30-32 |
| II | 74 | mp-39511 | $LiCaTa_2O_6F$ | SM | 1-3 |
| II | 74 | mp-655591 | $LiB1_3C_2$ | LD | 87-89 |
| II | 188 | mp-540631 | $KTa(GeO_3)_3$ | SM | 34-36 |
| II | 188 | mp-546032 | $RbTa(GeO_3)_3$ | SM | 34-36 |

*The strategy for loop-chain structure.*—A loop-chain structure requires identifying two types of BCs: one lies in a loop and the other in a chain, while ensuring the loop is nested with the chain. The locations of the nested nodal loops and nodal chains, and their corresponding irreps of BCs are listed in Table S14.

The screening of the Type-I loop-chain structure is divided into three steps: first, extract BCs from bands (band indices: $n$, $n+1$), indicated by BC1; second, ensure that the irreps of BC1 correspond to the irreps listed in Table S14; third, check whether loops and chains are nested with each other in the BZ.

The screening of the Type-II loop-chain structure is divided into three steps: first, extract BCs from bands (band indices: $n$, $n+1$), indicated by BC1, and extract BCs from bands (band indices: $n+1$, $n+2$), indicated by BC2; second, ensure that BC1 (or BC2) corresponds exclusively to irreps associated with one loop or more loops (Table S14), while ensuring that BC2 (or BC1) contains irreps associated with one chain or more chains (Table S14); third, check whether the loops and chains are nested within each other in the BZ.

Based on above strategy, we find 20 materials with loop-chain structure (either of type-I or of type-II) shown in Table S11.

Table S11: List of materials with loop-chain structure in phonon spectra. For each material, they are characterized by the type of Hopf-link structure, SG, the material ID from the online database of Materials Project,[14] chemical formula, the HSL and branches of bands.

| Type | SG | Material ID | Formula | HSL | Branches |
|---|---|---|---|---|---|
| I | 33 | mp-558105 | $LiB_6O_9F$ | LD | 26-27 |
| I | 62 | mp-10233 | $Ca_2BN_2F$ | SM | 44-45 |
| I | 62 | mp-10837 | $Na_2MgInF_7$ | DT | 28-29 |
| I | 62 | mp-18332 | $Lu_2ZnS_4$ | LD | 16-17 |
| I | 62 | mp-755138 | $NdInO_3$ | LD | 12-13 |
| I | 62 | mp-756205 | $ScBiO_3$ | SM | 18-19 |

to be continued

| Type | SG | Material ID | Formula | HSL | Branches |
|---|---|---|---|---|---|
| I | 63 | mp-15684 | $K_2CuAs$ | SM | 6-7 |
| I | 127 | mp-9656 | $BaY_2PdO_5$ | DT | 6-7 |
| II | 25 | mp-676038 | $Ga_5(PS)_3$ | G | 14-16 |
| II | 26 | mp-555463 | $RbTh_3F_{13}$ | H | 87-89 |
| II | 26 | mp-555976 | $Na_2TiSiO_5$ | Q | 18-20 |
| II | 31 | mp-13725 | $Li_3PO_4$ | LD | 38-40 |
| II | 31 | mp-769365 | $ZnSeO_4$ | H | 21-23 |
| II | 33 | mp-230 | $SbO_2$ | LD | 16-18 |
| II | 33 | mp-2254 | $Al_2O_3$ | LD | 86-88 |
| II | 36 | mp-510293 | $Pb_3SeO_5$ | H | 20-22 |
| II | 58 | mp-531265 | $Ca_3(BN_2)_2$ | SM | 158-160 |
| II | 62 | mp-2632 | $TlF_3$ | LD | 32-34 |
| II | 62 | mp-3792 | $YAlO_3$ | SM | 10-12 |
| II | 71 | mp-504806 | $K_2Li_{14}Pb_3O_{14}$ | DT | 9-11 |

*The strategy for inter-chain structure.*—An inter-chain structure requires that the existence of two or more chains that are nested together. The locations of the nodal chains and their corresponding irreps of BCs are listed in Table S15.

The screening of the Type-I inter-chain structure is divided into three steps: first, extract BCs from bands (band indices: $n$, $n+1$), indicated by BC1; second, ensure that irreps of BC1 include at least two irreps listed in Table S15, check whether chains are nested with each other in the BZ.

The screening of the Type-II inter-chain structure is divided into three steps: first, extract BCs from bands (band indices: $n$, $n+1$), indicated by BC1, and BCs from bands (band indices: $n+1$, $n+2$), indicated by BC2; second, ensure that both irreps of BC1 and irreps of BC2 include at least one irrep listed in Table S15; third, check whether chains are nested with each other in the BZ.

Based on the above strategy, we find 2 materials with inter-chain structure shown in Table S12.

Table S12: List of materials with inter-chain structure in phonon spectra. For each material, they are characterized by the type of Hopf-link structure, SG, the material ID from the online database of Materials Project,[14] chemical formula, the HSL and branches of bands.

| Type | SG | Material ID | Formula | HSL | Branches |
|---|---|---|---|---|---|
| II | 52 | mp-27522 | $K_2Zr_2O_5$ | LD | 24-26 |
| II | 59 | mp-561356 | $Cs_2UP_2O_9$ | LD | 30-32 |

*The strategy for intra-chain structure.*—An inter-chain structure is a nested configuration formed by a single chain due to time-reversal symmetry and the periodicity of the BZ. The locations of the nodal chains and their corresponding irreps of BCs are listed in Table S16.

The screening of the intra-chain structure is divided into three steps: first, extract BCs from bands (band indices: $n$, $n+1$), indicated by BC1; second, ensure that irrep of BC1 correspond exclusively to one irrep listed in Table S16, third, check whether the chain is a nested configuration in the BZ.

Based on the above strategy, we did not find intra-chain structures in pristine crystalline materials.

# S5. Tabulation of space groups possibly hosting phonon Hopf-link structure

In this section, we list tabulation of space groups possibly hosting four kinds of phonon Hopf-link structures, respectively.

The naming convention and the coordinates of HSLs follow those on the Bilbao server.[8] A nodal loop lies within a HSPL, for which we provide the normal vector of the HSPL. A nodal chain lies within multiple HSPLs, for which we provide the normal vectors of all HSPLs. Taking HSL G $(\frac{1}{2}, 0, w)$ in SG 25 as an example, the location of the nodal loop is $(-1, 0, 0)$ or $(0, -1, 0)$, which means the nodal loop lies within the HSPL $k_x = \frac{1}{2}$ or the HSPL $k_y = 0$. The location of the nodal chain is $(0, -1, 0)$, $(-1, 0, 0)$, which means the nodal chain lies within the two HSPLs $k_y = 0$ and $k_x = \frac{1}{2}$.

*The tabulation for loop-loop structure.*—In Table S13, The first column lists the corresponding SGs, with a total of 109. The second column lists the conventional coordinates of HSLs for diagnosing loop-loop structures. The third and fifth columns list the locations of two nested nodal loops (referred to as nodal loop 1 and nodal loop 2), respectively. The fourth and sixth columns show the irreps of the BCs in the HSL, which can imply nodal loop 1 and nodal loop 2, respectively.

*The tabulation for loop-chain structure.*—In Table S14, the first column lists the corresponding SGs, with a total of 109. The second column lists the HSLs for diagnosing the loop-chain structure. The third and fifth columns list the locations of the nested nodal chain and nodal loop, respectively. The fourth and sixth columns show the irreps of the BCs in the HSL, which can imply the nodal chain and the nodal loop, respectively.

*The tabulation for inter-chain structure.*—In Table S15, the first column lists the corresponding SGs, with a total of 141. The second column lists the HSLs for diagnosing the inter-chain structure. The third column lists the location of the nodal chain. The fourth column shows the irreps of the BCs in the HSL, which can imply the nodal chain.

*The tabulation for intra-chain structure.*—In Table S16, the first column lists the corresponding SGs, with a total of 109. The second column lists the HSLs for diagnosing the inter-chain structure. The third column lists the location of the nodal chain. The fourth column shows the irreps of the BCs in the HSL, which can imply the nodal chain.

Table S13: Loop-loop structure

| SG | HSL | Location of nodal loop 1 | Irreps of BC | Location of nodal loop 2 | Irreps of BC |
|---|---|---|---|---|---|
| 25 | $G(\frac{1}{2},\ 0,\ w)$ | $(-1,\ 0,\ 0)$ | 1⊕3 or 2⊕4 | $(0,\ -1,\ 0)$ | 1⊕4 or 2⊕3 |
| 25 | $H(0,\ \frac{1}{2},\ w)$ | $(-1,\ 0,\ 0)$ | 1⊕3 or 2⊕4 | $(0,\ -1,\ 0)$ | 1⊕4 or 2⊕3 |
| 25 | $LD(0,\ 0,\ w)$ | $(-1,\ 0,\ 0)$ | 1⊕3 or 2⊕4 | $(0,\ -1,\ 0)$ | 1⊕4 or 2⊕3 |
| 25 | $Q(\frac{1}{2},\ \frac{1}{2},\ w)$ | $(-1,\ 0,\ 0)$ | 1⊕3 or 2⊕4 | $(0,\ -1,\ 0)$ | 1⊕4 or 2⊕3 |
| 26 | $G(\frac{1}{2},\ 0,\ w)$ | $(-1,\ 0,\ 0)$ | 1⊕3 or 2⊕4 | $(0,\ -1,\ 0)$ | 1⊕4 or 2⊕3 |
| 26 | $H(0,\ \frac{1}{2},\ w)$ | $(-1,\ 0,\ 0)$ | 1⊕3 or 2⊕4 | $(0,\ -1,\ 0)$ | 1⊕4 or 2⊕3 |
| 26 | $LD(0,\ 0,\ w)$ | $(-1,\ 0,\ 0)$ | 1⊕3 or 2⊕4 | $(0,\ -1,\ 0)$ | 1⊕4 or 2⊕3 |
| 26 | $Q(\frac{1}{2},\ \frac{1}{2},\ w)$ | $(-1,\ 0,\ 0)$ | 1⊕3 or 2⊕4 | $(0,\ -1,\ 0)$ | 1⊕4 or 2⊕3 |
| 27 | $G(\frac{1}{2},\ 0,\ w)$ | $(-1,\ 0,\ 0)$ | 1⊕3 or 2⊕4 | $(0,\ -1,\ 0)$ | 1⊕4 or 2⊕3 |
| 27 | $H(0,\ \frac{1}{2},\ w)$ | $(-1,\ 0,\ 0)$ | 1⊕3 or 2⊕4 | $(0,\ -1,\ 0)$ | 1⊕4 or 2⊕3 |
| 27 | $LD(0,\ 0,\ w)$ | $(-1,\ 0,\ 0)$ | 1⊕3 or 2⊕4 | $(0,\ -1,\ 0)$ | 1⊕4 or 2⊕3 |
| 27 | $Q(\frac{1}{2},\ \frac{1}{2},\ w)$ | $(-1,\ 0,\ 0)$ | 1⊕3 or 2⊕4 | $(0,\ -1,\ 0)$ | 1⊕4 or 2⊕3 |
| 28 | $H(0,\ \frac{1}{2},\ w)$ | $(0,\ 1,\ 0)$ | 1⊕3 or 2⊕4 | $(-1,\ 0,\ 0)$ | 1⊕4 or 2⊕3 |
| 28 | $LD(0,\ 0,\ w)$ | $(0,\ 1,\ 0)$ | 1⊕3 or 2⊕4 | $(-1,\ 0,\ 0)$ | 1⊕4 or 2⊕3 |
| 29 | $H(0,\ \frac{1}{2},\ w)$ | $(0,\ 1,\ 0)$ | 1⊕3 or 2⊕4 | $(-1,\ 0,\ 0)$ | 1⊕4 or 2⊕3 |
| 29 | $LD(0,\ 0,\ w)$ | $(0,\ 1,\ 0)$ | 1⊕3 or 2⊕4 | $(-1,\ 0,\ 0)$ | 1⊕4 or 2⊕3 |
| 30 | $G(\frac{1}{2},\ 0,\ w)$ | $(-1,\ 0,\ 0)$ | 1⊕3 or 2⊕4 | $(0,\ -1,\ 0)$ | 1⊕4 or 2⊕3 |
| 30 | $LD(0,\ 0,\ w)$ | $(-1,\ 0,\ 0)$ | 1⊕3 or 2⊕4 | $(0,\ -1,\ 0)$ | 1⊕4 or 2⊕3 |
| 31 | $H(0,\ \frac{1}{2},\ w)$ | $(0,\ 1,\ 0)$ | 1⊕3 or 2⊕4 | $(-1,\ 0,\ 0)$ | 1⊕4 or 2⊕3 |
| 31 | $LD(0,\ 0,\ w)$ | $(0,\ 1,\ 0)$ | 1⊕3 or 2⊕4 | $(-1,\ 0,\ 0)$ | 1⊕4 or 2⊕3 |
| 32 | $LD(0,\ 0,\ w)$ | $(-1,\ 0,\ 0)$ | 1⊕3 or 2⊕4 | $(0,\ -1,\ 0)$ | 1⊕4 or 2⊕3 |
| 32 | $Q(\frac{1}{2},\ \frac{1}{2},\ w)$ | $(-1,\ 0,\ 0)$ | 1⊕2 or 3⊕4 | $(0,\ -1,\ 0)$ | 1⊕4 or 2⊕3 |
| 33 | $LD(0,\ 0,\ w)$ | $(0,\ 1,\ 0)$ | 1⊕3 or 2⊕4 | $(-1,\ 0,\ 0)$ | 1⊕4 or 2⊕3 |
| 33 | $Q(\frac{1}{2},\ \frac{1}{2},\ w)$ | $(0,\ 1,\ 0)$ | 1⊕2 or 3⊕4 | $(-1,\ 0,\ 0)$ | 1⊕4 or 2⊕3 |
| 34 | $LD(0,\ 0,\ w)$ | $(-1,\ 0,\ 0)$ | 1⊕3 or 2⊕4 | $(0,\ -1,\ 0)$ | 1⊕4 or 2⊕3 |
| 34 | $Q(\frac{1}{2},\ \frac{1}{2},\ w)$ | $(-1,\ 0,\ 0)$ | 1⊕2 or 3⊕4 | $(0,\ -1,\ 0)$ | 1⊕4 or 2⊕3 |
| 35 | $H(1,\ 0,\ w)$ | $(-1,\ 0,\ 0)$ | 1⊕3 or 2⊕4 | $(0,\ -1,\ 0)$ | 1⊕4 or 2⊕3 |
| 35 | $LD(0,\ 0,\ w)$ | $(-1,\ 0,\ 0)$ | 1⊕3 or 2⊕4 | $(0,\ -1,\ 0)$ | 1⊕4 or 2⊕3 |
| 36 | $H(1,\ 0,\ w)$ | $(0,\ 1,\ 0)$ | 1⊕3 or 2⊕4 | $(-1,\ 0,\ 0)$ | 1⊕4 or 2⊕3 |
| 36 | $LD(0,\ 0,\ w)$ | $(0,\ 1,\ 0)$ | 1⊕3 or 2⊕4 | $(-1,\ 0,\ 0)$ | 1⊕4 or 2⊕3 |
| 37 | $H(1,\ 0,\ w)$ | $(-1,\ 0,\ 0)$ | 1⊕3 or 2⊕4 | $(0,\ -1,\ 0)$ | 1⊕4 or 2⊕3 |
| 37 | $LD(0,\ 0,\ w)$ | $(-1,\ 0,\ 0)$ | 1⊕3 or 2⊕4 | $(0,\ -1,\ 0)$ | 1⊕4 or 2⊕3 |
| 38 | $A(\frac{1}{2},\ 0,\ w)$ | $(1,\ 0,\ 0)$ | 1⊕3 or 2⊕4 | $(0,\ -1,\ 0)$ | 1⊕4 or 2⊕3 |
| 38 | $SM(0,\ 0,\ w)$ | $(1,\ 0,\ 0)$ | 1⊕3 or 2⊕4 | $(0,\ -1,\ 0)$ | 1⊕4 or 2⊕3 |
| 39 | $A(\frac{1}{2},\ 0,\ w)$ | $(1,\ 0,\ 0)$ | 1⊕3 or 2⊕4 | $(0,\ -1,\ 0)$ | 1⊕4 or 2⊕3 |
| 39 | $SM(0,\ 0,\ w)$ | $(1,\ 0,\ 0)$ | 1⊕3 or 2⊕4 | $(0,\ -1,\ 0)$ | 1⊕4 or 2⊕3 |
| 40 | $SM(0,\ 0,\ w)$ | $(1,\ 0,\ 0)$ | 1⊕3 or 2⊕4 | $(0,\ -1,\ 0)$ | 1⊕4 or 2⊕3 |
| 41 | $SM(0,\ 0,\ w)$ | $(1,\ 0,\ 0)$ | 1⊕3 or 2⊕4 | $(0,\ -1,\ 0)$ | 1⊕4 or 2⊕3 |
| 42 | $H(0,\ 1,\ w)$ | $(1,\ 0,\ 0)$ | 1⊕3 or 2⊕4 | $(0,\ 1,\ 0)$ | 1⊕4 or 2⊕3 |
| 42 | $LD(0,\ 0,\ w)$ | $(1,\ 0,\ 0)$ | 1⊕3 or 2⊕4 | $(0,\ 1,\ 0)$ | 1⊕4 or 2⊕3 |
| 43 | $LD(0,\ 0,\ w)$ | $(1,\ 0,\ 0)$ | 1⊕3 or 2⊕4 | $(0,\ 1,\ 0)$ | 1⊕4 or 2⊕3 |

| SG | HSL | Location of nodal loop 1 | Irreps of BC | Location of nodal loop 2 | Irreps of BC |
|---|---|---|---|---|---|
| 44 | LD$(0,\ 0,\ w)$ | $(1,\ 0,\ 0)$ | 1⊕3 or 2⊕4 | $(0,\ -1,\ 0)$ | 1⊕4 or 2⊕3 |
| 45 | LD$(0,\ 0,\ w)$ | $(1,\ 0,\ 0)$ | 1⊕3 or 2⊕4 | $(0,\ -1,\ 0)$ | 1⊕4 or 2⊕3 |
| 46 | LD$(0,\ 0,\ w)$ | $(0,\ -1,\ 0)$ | 1⊕3 or 2⊕4 | $(-1,\ 0,\ 0)$ | 1⊕4 or 2⊕3 |
| 47 | A$\left(u,\ 0,\ \frac{1}{2}\right)$ | $(0,\ -1,\ 0)$ | {1}⊕{3} or {2}⊕{4} | $(0,\ 0,\ 1)$ | {1}⊕{4} or {2}⊕{3} |
| 47 | B$\left(0,\ v,\ \frac{1}{2}\right)$ | $(0,\ 0,\ 1)$ | {1}⊕{3} or {2}⊕{4} | $(-1,\ 0,\ 0)$ | {1}⊕{4} or {2}⊕{3} |
| 47 | C$\left(u,\ \frac{1}{2},\ 0\right)$ | $(0,\ -1,\ 0)$ | {1}⊕{3} or {2}⊕{4} | $(0,\ 0,\ 1)$ | {1}⊕{4} or {2}⊕{3} |
| 47 | D$\left(\frac{1}{2},\ v,\ 0\right)$ | $(0,\ 0,\ 1)$ | {1}⊕{3} or {2}⊕{4} | $(-1,\ 0,\ 0)$ | {1}⊕{4} or {2}⊕{3} |
| 47 | DT$(0,\ v,\ 0)$ | $(0,\ 0,\ 1)$ | {1}⊕{3} or {2}⊕{4} | $(-1,\ 0,\ 0)$ | {1}⊕{4} or {2}⊕{3} |
| 47 | E$\left(u,\ \frac{1}{2},\ \frac{1}{2}\right)$ | $(0,\ -1,\ 0)$ | {1}⊕{3} or {2}⊕{4} | $(0,\ 0,\ 1)$ | {1}⊕{4} or {2}⊕{3} |
| 47 | G$\left(\frac{1}{2},\ 0,\ w\right)$ | $(-1,\ 0,\ 0)$ | {1}⊕{3} or {2}⊕{4} | $(0,\ -1,\ 0)$ | {1}⊕{4} or {2}⊕{3} |
| 47 | H$\left(0,\ \frac{1}{2},\ w\right)$ | $(-1,\ 0,\ 0)$ | {1}⊕{3} or {2}⊕{4} | $(0,\ -1,\ 0)$ | {1}⊕{4} or {2}⊕{3} |
| 47 | LD$(0,\ 0,\ w)$ | $(-1,\ 0,\ 0)$ | {1}⊕{3} or {2}⊕{4} | $(0,\ -1,\ 0)$ | {1}⊕{4} or {2}⊕{3} |
| 47 | P$\left(\frac{1}{2},\ v,\ \frac{1}{2}\right)$ | $(0,\ 0,\ 1)$ | {1}⊕{3} or {2}⊕{4} | $(-1,\ 0,\ 0)$ | {1}⊕{4} or {2}⊕{3} |
| 47 | Q$\left(\frac{1}{2},\ \frac{1}{2},\ w\right)$ | $(-1,\ 0,\ 0)$ | {1}⊕{3} or {2}⊕{4} | $(0,\ -1,\ 0)$ | {1}⊕{4} or {2}⊕{3} |
| 47 | SM$(u,\ 0,\ 0)$ | $(0,\ -1,\ 0)$ | {1}⊕{3} or {2}⊕{4} | $(0,\ 0,\ 1)$ | {1}⊕{4} or {2}⊕{3} |
| 48 | DT$(0,\ v,\ 0)$ | $(0,\ 0,\ 1)$ | {1}⊕{3} or {2}⊕{4} | $(-1,\ 0,\ 0)$ | {1}⊕{4} or {2}⊕{3} |
| 48 | E$\left(u,\ \frac{1}{2},\ \frac{1}{2}\right)$ | $(0,\ -1,\ 0)$ | {1}⊕{3} or {2}⊕{4} | $(0,\ 0,\ 1)$ | {1}⊕{4} or {2}⊕{3} |
| 48 | LD$(0,\ 0,\ w)$ | $(-1,\ 0,\ 0)$ | {1}⊕{3} or {2}⊕{4} | $(0,\ -1,\ 0)$ | {1}⊕{4} or {2}⊕{3} |
| 48 | P$\left(\frac{1}{2},\ v,\ \frac{1}{2}\right)$ | $(-1,\ 0,\ 0)$ | {1}⊕{3} or {2}⊕{4} | $(0,\ 0,\ 1)$ | {1}⊕{4} or {2}⊕{3} |
| 48 | Q$\left(\frac{1}{2},\ \frac{1}{2},\ w\right)$ | $(0,\ -1,\ 0)$ | {1}⊕{3} or {2}⊕{4} | $(-1,\ 0,\ 0)$ | {1}⊕{4} or {2}⊕{3} |
| 48 | SM$(u,\ 0,\ 0)$ | $(0,\ 0,\ 1)$ | {1}⊕{3} or {2}⊕{4} | $(0,\ -1,\ 0)$ | {1}⊕{4} or {2}⊕{3} |
| 49 | C$\left(u,\ \frac{1}{2},\ 0\right)$ | $(0,\ -1,\ 0)$ | {1}⊕{3} or {2}⊕{4} | $(0,\ 0,\ 1)$ | {1}⊕{4} or {2}⊕{3} |
| 49 | D$\left(\frac{1}{2},\ v,\ 0\right)$ | $(0,\ 0,\ 1)$ | {1}⊕{3} or {2}⊕{4} | $(-1,\ 0,\ 0)$ | {1}⊕{4} or {2}⊕{3} |
| 49 | DT$(0,\ v,\ 0)$ | $(0,\ 0,\ 1)$ | {1}⊕{3} or {2}⊕{4} | $(-1,\ 0,\ 0)$ | {1}⊕{4} or {2}⊕{3} |
| 49 | G$\left(\frac{1}{2},\ 0,\ w\right)$ | $(-1,\ 0,\ 0)$ | {1}⊕{3} or {2}⊕{4} | $(0,\ -1,\ 0)$ | {1}⊕{4} or {2}⊕{3} |
| 49 | H$\left(0,\ \frac{1}{2},\ w\right)$ | $(-1,\ 0,\ 0)$ | {1}⊕{3} or {2}⊕{4} | $(0,\ -1,\ 0)$ | {1}⊕{4} or {2}⊕{3} |
| 49 | LD$(0,\ 0,\ w)$ | $(-1,\ 0,\ 0)$ | {1}⊕{3} or {2}⊕{4} | $(0,\ -1,\ 0)$ | {1}⊕{4} or {2}⊕{3} |
| 49 | Q$\left(\frac{1}{2},\ \frac{1}{2},\ w\right)$ | $(-1,\ 0,\ 0)$ | {1}⊕{3} or {2}⊕{4} | $(0,\ -1,\ 0)$ | {1}⊕{4} or {2}⊕{3} |
| 49 | SM$(u,\ 0,\ 0)$ | $(0,\ -1,\ 0)$ | {1}⊕{3} or {2}⊕{4} | $(0,\ 0,\ 1)$ | {1}⊕{4} or {2}⊕{3} |
| 50 | A$\left(u,\ 0,\ \frac{1}{2}\right)$ | $(0,\ -1,\ 0)$ | {1}⊕{3} or {2}⊕{4} | $(0,\ 0,\ 1)$ | {1}⊕{4} or {2}⊕{3} |
| 50 | B$\left(0,\ v,\ \frac{1}{2}\right)$ | $(0,\ 0,\ 1)$ | {1}⊕{3} or {2}⊕{4} | $(-1,\ 0,\ 0)$ | {1}⊕{4} or {2}⊕{3} |
| 50 | DT$(0,\ v,\ 0)$ | $(0,\ 0,\ 1)$ | {1}⊕{3} or {2}⊕{4} | $(-1,\ 0,\ 0)$ | {1}⊕{4} or {2}⊕{3} |
| 50 | LD$(0,\ 0,\ w)$ | $(-1,\ 0,\ 0)$ | {1}⊕{3} or {2}⊕{4} | $(0,\ -1,\ 0)$ | {1}⊕{4} or {2}⊕{3} |
| 50 | Q$\left(\frac{1}{2},\ \frac{1}{2},\ w\right)$ | $(-1,\ 0,\ 0)$ | {1}⊕{3} or {2}⊕{4} | $(0,\ -1,\ 0)$ | {1}⊕{4} or {2}⊕{3} |
| 50 | SM$(u,\ 0,\ 0)$ | $(0,\ -1,\ 0)$ | {1}⊕{3} or {2}⊕{4} | $(0,\ 0,\ 1)$ | {1}⊕{4} or {2}⊕{3} |
| 51 | A$\left(u,\ 0,\ \frac{1}{2}\right)$ | $(0,\ 0,\ -1)$ | {1}⊕{3} or {2}⊕{4} | $(0,\ -1,\ 0)$ | {1}⊕{4} or {2}⊕{3} |
| 51 | B$\left(0,\ v,\ \frac{1}{2}\right)$ | $(-1,\ 0,\ 0)$ | {1}⊕{3} or {2}⊕{4} | $(0,\ 0,\ -1)$ | {1}⊕{4} or {2}⊕{3} |
| 51 | C$\left(u,\ \frac{1}{2},\ 0\right)$ | $(0,\ 0,\ -1)$ | {1}⊕{3} or {2}⊕{4} | $(0,\ -1,\ 0)$ | {1}⊕{4} or {2}⊕{3} |
| 51 | DT$(0,\ v,\ 0)$ | $(-1,\ 0,\ 0)$ | {1}⊕{3} or {2}⊕{4} | $(0,\ 0,\ -1)$ | {1}⊕{4} or {2}⊕{3} |
| 51 | E$\left(u,\ \frac{1}{2},\ \frac{1}{2}\right)$ | $(0,\ 0,\ -1)$ | {1}⊕{3} or {2}⊕{4} | $(0,\ -1,\ 0)$ | {1}⊕{4} or {2}⊕{3} |
| 51 | H$\left(0,\ \frac{1}{2},\ w\right)$ | $(0,\ -1,\ 0)$ | {1}⊕{3} or {2}⊕{4} | $(-1,\ 0,\ 0)$ | {1}⊕{4} or {2}⊕{3} |

| SG | HSL | Location of nodal loop 1 | Irreps of BC | Location of nodal loop 2 | Irreps of BC |
|---|---|---|---|---|---|
| 51 | LD$(0,\ 0,\ w)$ | $(0,\ -1,\ 0)$ | {1}⊕{3} or {2}⊕{4} | $(-1,\ 0,\ 0)$ | {1}⊕{4} or {2}⊕{3} |
| 51 | SM$(u,\ 0,\ 0)$ | $(0,\ 0,\ -1)$ | {1}⊕{3} or {2}⊕{4} | $(0,\ -1,\ 0)$ | {1}⊕{4} or {2}⊕{3} |
| 52 | DT$(0,\ v,\ 0)$ | $(-1,\ 0,\ 0)$ | {1}⊕{3} or {2}⊕{4} | $(0,\ 0,\ 1)$ | {1}⊕{4} or {2}⊕{3} |
| 52 | LD$(0,\ 0,\ w)$ | $(0,\ 1,\ 0)$ | {1}⊕{3} or {2}⊕{4} | $(-1,\ 0,\ 0)$ | {1}⊕{4} or {2}⊕{3} |
| 52 | P$\left(\frac{1}{2},\ v,\ \frac{1}{2}\right)$ | $(-1,\ 0,\ 0)$ | {1}⊕{3} or {2}⊕{4} | $(0,\ 0,\ 1)$ | {1}⊕{4} or {2}⊕{3} |
| 52 | SM$(u,\ 0,\ 0)$ | $(0,\ 0,\ 1)$ | {1}⊕{3} or {2}⊕{4} | $(0,\ 1,\ 0)$ | {1}⊕{4} or {2}⊕{3} |
| 53 | C$\left(u,\ \frac{1}{2},\ 0\right)$ | $(0,\ 0,\ 1)$ | {1}⊕{3} or {2}⊕{4} | $(0,\ 1,\ 0)$ | {1}⊕{4} or {2}⊕{3} |
| 53 | DT$(0,\ v,\ 0)$ | $(-1,\ 0,\ 0)$ | {1}⊕{3} or {2}⊕{4} | $(0,\ 0,\ 1)$ | {1}⊕{4} or {2}⊕{3} |
| 53 | H$\left(0,\ \frac{1}{2},\ w\right)$ | $(0,\ 1,\ 0)$ | {1}⊕{3} or {2}⊕{4} | $(-1,\ 0,\ 0)$ | {1}⊕{4} or {2}⊕{3} |
| 53 | LD$(0,\ 0,\ w)$ | $(0,\ 1,\ 0)$ | {1}⊕{3} or {2}⊕{4} | $(-1,\ 0,\ 0)$ | {1}⊕{4} or {2}⊕{3} |
| 53 | SM$(u,\ 0,\ 0)$ | $(0,\ 0,\ 1)$ | {1}⊕{3} or {2}⊕{4} | $(0,\ 1,\ 0)$ | {1}⊕{4} or {2}⊕{3} |
| 54 | C$\left(u,\ \frac{1}{2},\ 0\right)$ | $(0,\ 0,\ -1)$ | {1}⊕{3} or {2}⊕{4} | $(0,\ -1,\ 0)$ | {1}⊕{4} or {2}⊕{3} |
| 54 | DT$(0,\ v,\ 0)$ | $(-1,\ 0,\ 0)$ | {1}⊕{3} or {2}⊕{4} | $(0,\ 0,\ -1)$ | {1}⊕{4} or {2}⊕{3} |
| 54 | H$\left(0,\ \frac{1}{2},\ w\right)$ | $(0,\ -1,\ 0)$ | {1}⊕{3} or {2}⊕{4} | $(-1,\ 0,\ 0)$ | {1}⊕{4} or {2}⊕{3} |
| 54 | LD$(0,\ 0,\ w)$ | $(0,\ -1,\ 0)$ | {1}⊕{3} or {2}⊕{4} | $(-1,\ 0,\ 0)$ | {1}⊕{4} or {2}⊕{3} |
| 54 | SM$(u,\ 0,\ 0)$ | $(0,\ 0,\ -1)$ | {1}⊕{3} or {2}⊕{4} | $(0,\ -1,\ 0)$ | {1}⊕{4} or {2}⊕{3} |
| 55 | A$\left(u,\ 0,\ \frac{1}{2}\right)$ | $(0,\ -1,\ 0)$ | {1}⊕{3} or {2}⊕{4} | $(0,\ 0,\ 1)$ | {1}⊕{4} or {2}⊕{3} |
| 55 | B$\left(0,\ v,\ \frac{1}{2}\right)$ | $(0,\ 0,\ 1)$ | {1}⊕{3} or {2}⊕{4} | $(-1,\ 0,\ 0)$ | {1}⊕{4} or {2}⊕{3} |
| 55 | DT$(0,\ v,\ 0)$ | $(0,\ 0,\ 1)$ | {1}⊕{3} or {2}⊕{4} | $(-1,\ 0,\ 0)$ | {1}⊕{4} or {2}⊕{3} |
| 55 | LD$(0,\ 0,\ w)$ | $(-1,\ 0,\ 0)$ | {1}⊕{3} or {2}⊕{4} | $(0,\ -1,\ 0)$ | {1}⊕{4} or {2}⊕{3} |
| 55 | SM$(u,\ 0,\ 0)$ | $(0,\ -1,\ 0)$ | {1}⊕{3} or {2}⊕{4} | $(0,\ 0,\ 1)$ | {1}⊕{4} or {2}⊕{3} |
| 56 | DT$(0,\ v,\ 0)$ | $(0,\ 0,\ 1)$ | {1}⊕{3} or {2}⊕{4} | $(-1,\ 0,\ 0)$ | {1}⊕{4} or {2}⊕{3} |
| 56 | LD$(0,\ 0,\ w)$ | $(-1,\ 0,\ 0)$ | {1}⊕{3} or {2}⊕{4} | $(0,\ -1,\ 0)$ | {1}⊕{4} or {2}⊕{3} |
| 56 | SM$(u,\ 0,\ 0)$ | $(0,\ -1,\ 0)$ | {1}⊕{3} or {2}⊕{4} | $(0,\ 0,\ 1)$ | {1}⊕{4} or {2}⊕{3} |
| 57 | D$\left(\frac{1}{2},\ v,\ 0\right)$ | $(0,\ 0,\ -1)$ | {1}⊕{3} or {2}⊕{4} | $(1,\ 0,\ 0)$ | {1}⊕{4} or {2}⊕{3} |
| 57 | DT$(0,\ v,\ 0)$ | $(0,\ 0,\ -1)$ | {1}⊕{3} or {2}⊕{4} | $(1,\ 0,\ 0)$ | {1}⊕{4} or {2}⊕{3} |
| 57 | G$\left(\frac{1}{2},\ 0,\ w\right)$ | $(1,\ 0,\ 0)$ | {1}⊕{3} or {2}⊕{4} | $(0,\ -1,\ 0)$ | {1}⊕{4} or {2}⊕{3} |
| 57 | LD$(0,\ 0,\ w)$ | $(1,\ 0,\ 0)$ | {1}⊕{3} or {2}⊕{4} | $(0,\ -1,\ 0)$ | {1}⊕{4} or {2}⊕{3} |
| 57 | SM$(u,\ 0,\ 0)$ | $(0,\ -1,\ 0)$ | {1}⊕{3} or {2}⊕{4} | $(0,\ 0,\ -1)$ | {1}⊕{4} or {2}⊕{3} |
| 58 | DT$(0,\ v,\ 0)$ | $(0,\ 0,\ 1)$ | {1}⊕{3} or {2}⊕{4} | $(-1,\ 0,\ 0)$ | {1}⊕{4} or {2}⊕{3} |
| 58 | LD$(0,\ 0,\ w)$ | $(-1,\ 0,\ 0)$ | {1}⊕{3} or {2}⊕{4} | $(0,\ -1,\ 0)$ | {1}⊕{4} or {2}⊕{3} |
| 58 | SM$(u,\ 0,\ 0)$ | $(0,\ -1,\ 0)$ | {1}⊕{3} or {2}⊕{4} | $(0,\ 0,\ 1)$ | {1}⊕{4} or {2}⊕{3} |
| 59 | A$\left(u,\ 0,\ \frac{1}{2}\right)$ | $(0,\ -1,\ 0)$ | {1}⊕{3} or {2}⊕{4} | $(0,\ 0,\ 1)$ | {1}⊕{4} or {2}⊕{3} |
| 59 | B$\left(0,\ v,\ \frac{1}{2}\right)$ | $(0,\ 0,\ 1)$ | {1}⊕{3} or {2}⊕{4} | $(-1,\ 0,\ 0)$ | {1}⊕{4} or {2}⊕{3} |
| 59 | DT$(0,\ v,\ 0)$ | $(0,\ 0,\ 1)$ | {1}⊕{3} or {2}⊕{4} | $(-1,\ 0,\ 0)$ | {1}⊕{4} or {2}⊕{3} |
| 59 | LD$(0,\ 0,\ w)$ | $(-1,\ 0,\ 0)$ | {1}⊕{3} or {2}⊕{4} | $(0,\ -1,\ 0)$ | {1}⊕{4} or {2}⊕{3} |
| 59 | SM$(u,\ 0,\ 0)$ | $(0,\ -1,\ 0)$ | {1}⊕{3} or {2}⊕{4} | $(0,\ 0,\ 1)$ | {1}⊕{4} or {2}⊕{3} |
| 60 | DT$(0,\ v,\ 0)$ | $(-1,\ 0,\ 0)$ | {1}⊕{3} or {2}⊕{4} | $(0,\ 0,\ 1)$ | {1}⊕{4} or {2}⊕{3} |
| 60 | LD$(0,\ 0,\ w)$ | $(0,\ 1,\ 0)$ | {1}⊕{3} or {2}⊕{4} | $(-1,\ 0,\ 0)$ | {1}⊕{4} or {2}⊕{3} |
| 60 | SM$(u,\ 0,\ 0)$ | $(0,\ 0,\ 1)$ | {1}⊕{3} or {2}⊕{4} | $(0,\ 1,\ 0)$ | {1}⊕{4} or {2}⊕{3} |
| 61 | DT$(0,\ v,\ 0)$ | $(-1,\ 0,\ 0)$ | {1}⊕{3} or {2}⊕{4} | $(0,\ 0,\ 1)$ | {1}⊕{4} or {2}⊕{3} |

| SG | HSL | Location of nodal loop 1 | Irreps of BC | Location of nodal loop 2 | Irreps of BC |
|---|---|---|---|---|---|
| 61 | LD$(0,\ 0,\ w)$ | $(0,\ 1,\ 0)$ | $\{1\}\oplus\{3\}$ or $\{2\}\oplus\{4\}$ | $(-1,\ 0,\ 0)$ | $\{1\}\oplus\{4\}$ or $\{2\}\oplus\{3\}$ |
| 61 | SM$(u,\ 0,\ 0)$ | $(0,\ 0,\ 1)$ | $\{1\}\oplus\{3\}$ or $\{2\}\oplus\{4\}$ | $(0,\ 1,\ 0)$ | $\{1\}\oplus\{4\}$ or $\{2\}\oplus\{3\}$ |
| 62 | DT$(0,\ v,\ 0)$ | $(0,\ 0,\ 1)$ | $\{1\}\oplus\{3\}$ or $\{2\}\oplus\{4\}$ | $(-1,\ 0,\ 0)$ | $\{1\}\oplus\{4\}$ or $\{2\}\oplus\{3\}$ |
| 62 | LD$(0,\ 0,\ w)$ | $(-1,\ 0,\ 0)$ | $\{1\}\oplus\{3\}$ or $\{2\}\oplus\{4\}$ | $(0,\ -1,\ 0)$ | $\{1\}\oplus\{4\}$ or $\{2\}\oplus\{3\}$ |
| 62 | SM$(u,\ 0,\ 0)$ | $(0,\ -1,\ 0)$ | $\{1\}\oplus\{3\}$ or $\{2\}\oplus\{4\}$ | $(0,\ 0,\ 1)$ | $\{1\}\oplus\{4\}$ or $\{2\}\oplus\{3\}$ |
| 63 | DT$(0,\ v,\ 0)$ | $(0,\ 0,\ 1)$ | $\{1\}\oplus\{3\}$ or $\{2\}\oplus\{4\}$ | $(-1,\ 0,\ 0)$ | $\{1\}\oplus\{4\}$ or $\{2\}\oplus\{3\}$ |
| 63 | H$(1,\ 0,\ w)$ | $(-1,\ 0,\ 0)$ | $\{1\}\oplus\{3\}$ or $\{2\}\oplus\{4\}$ | $(0,\ -1,\ 0)$ | $\{1\}\oplus\{4\}$ or $\{2\}\oplus\{3\}$ |
| 63 | LD$(0,\ 0,\ w)$ | $(-1,\ 0,\ 0)$ | $\{1\}\oplus\{3\}$ or $\{2\}\oplus\{4\}$ | $(0,\ -1,\ 0)$ | $\{1\}\oplus\{4\}$ or $\{2\}\oplus\{3\}$ |
| 63 | SM$(u,\ 0,\ 0)$ | $(0,\ -1,\ 0)$ | $\{1\}\oplus\{3\}$ or $\{2\}\oplus\{4\}$ | $(0,\ 0,\ 1)$ | $\{1\}\oplus\{4\}$ or $\{2\}\oplus\{3\}$ |
| 64 | DT$(0,\ v,\ 0)$ | $(0,\ 0,\ 1)$ | $\{1\}\oplus\{3\}$ or $\{2\}\oplus\{4\}$ | $(-1,\ 0,\ 0)$ | $\{1\}\oplus\{4\}$ or $\{2\}\oplus\{3\}$ |
| 64 | H$(1,\ 0,\ w)$ | $(-1,\ 0,\ 0)$ | $\{1\}\oplus\{3\}$ or $\{2\}\oplus\{4\}$ | $(0,\ -1,\ 0)$ | $\{1\}\oplus\{4\}$ or $\{2\}\oplus\{3\}$ |
| 64 | LD$(0,\ 0,\ w)$ | $(-1,\ 0,\ 0)$ | $\{1\}\oplus\{3\}$ or $\{2\}\oplus\{4\}$ | $(0,\ -1,\ 0)$ | $\{1\}\oplus\{4\}$ or $\{2\}\oplus\{3\}$ |
| 64 | SM$(u,\ 0,\ 0)$ | $(0,\ -1,\ 0)$ | $\{1\}\oplus\{3\}$ or $\{2\}\oplus\{4\}$ | $(0,\ 0,\ 1)$ | $\{1\}\oplus\{4\}$ or $\{2\}\oplus\{3\}$ |
| 65 | A$\left(u,\ 0,\ \frac{1}{2}\right)$ | $(0,\ -1,\ 0)$ | $\{1\}\oplus\{3\}$ or $\{2\}\oplus\{4\}$ | $(0,\ 0,\ 1)$ | $\{1\}\oplus\{4\}$ or $\{2\}\oplus\{3\}$ |
| 65 | B$\left(0,\ v,\ \frac{1}{2}\right)$ | $(0,\ 0,\ 1)$ | $\{1\}\oplus\{3\}$ or $\{2\}\oplus\{4\}$ | $(-1,\ 0,\ 0)$ | $\{1\}\oplus\{4\}$ or $\{2\}\oplus\{3\}$ |
| 65 | DT$(0,\ v,\ 0)$ | $(0,\ 0,\ 1)$ | $\{1\}\oplus\{3\}$ or $\{2\}\oplus\{4\}$ | $(-1,\ 0,\ 0)$ | $\{1\}\oplus\{4\}$ or $\{2\}\oplus\{3\}$ |
| 65 | H$(1,\ 0,\ w)$ | $(-1,\ 0,\ 0)$ | $\{1\}\oplus\{3\}$ or $\{2\}\oplus\{4\}$ | $(0,\ -1,\ 0)$ | $\{1\}\oplus\{4\}$ or $\{2\}\oplus\{3\}$ |
| 65 | LD$(0,\ 0,\ w)$ | $(-1,\ 0,\ 0)$ | $\{1\}\oplus\{3\}$ or $\{2\}\oplus\{4\}$ | $(0,\ -1,\ 0)$ | $\{1\}\oplus\{4\}$ or $\{2\}\oplus\{3\}$ |
| 65 | SM$(u,\ 0,\ 0)$ | $(0,\ -1,\ 0)$ | $\{1\}\oplus\{3\}$ or $\{2\}\oplus\{4\}$ | $(0,\ 0,\ 1)$ | $\{1\}\oplus\{4\}$ or $\{2\}\oplus\{3\}$ |
| 66 | DT$(0,\ v,\ 0)$ | $(0,\ 0,\ 1)$ | $\{1\}\oplus\{3\}$ or $\{2\}\oplus\{4\}$ | $(-1,\ 0,\ 0)$ | $\{1\}\oplus\{4\}$ or $\{2\}\oplus\{3\}$ |
| 66 | H$(1,\ 0,\ w)$ | $(-1,\ 0,\ 0)$ | $\{1\}\oplus\{3\}$ or $\{2\}\oplus\{4\}$ | $(0,\ -1,\ 0)$ | $\{1\}\oplus\{4\}$ or $\{2\}\oplus\{3\}$ |
| 66 | LD$(0,\ 0,\ w)$ | $(-1,\ 0,\ 0)$ | $\{1\}\oplus\{3\}$ or $\{2\}\oplus\{4\}$ | $(0,\ -1,\ 0)$ | $\{1\}\oplus\{4\}$ or $\{2\}\oplus\{3\}$ |
| 66 | SM$(u,\ 0,\ 0)$ | $(0,\ -1,\ 0)$ | $\{1\}\oplus\{3\}$ or $\{2\}\oplus\{4\}$ | $(0,\ 0,\ 1)$ | $\{1\}\oplus\{4\}$ or $\{2\}\oplus\{3\}$ |
| 67 | A$\left(u,\ 0,\ \frac{1}{2}\right)$ | $(0,\ -1,\ 0)$ | $\{1\}\oplus\{3\}$ or $\{2\}\oplus\{4\}$ | $(0,\ 0,\ 1)$ | $\{1\}\oplus\{4\}$ or $\{2\}\oplus\{3\}$ |
| 67 | B$\left(0,\ v,\ \frac{1}{2}\right)$ | $(0,\ 0,\ 1)$ | $\{1\}\oplus\{3\}$ or $\{2\}\oplus\{4\}$ | $(-1,\ 0,\ 0)$ | $\{1\}\oplus\{4\}$ or $\{2\}\oplus\{3\}$ |
| 67 | DT$(0,\ v,\ 0)$ | $(0,\ 0,\ 1)$ | $\{1\}\oplus\{3\}$ or $\{2\}\oplus\{4\}$ | $(-1,\ 0,\ 0)$ | $\{1\}\oplus\{4\}$ or $\{2\}\oplus\{3\}$ |
| 67 | H$(1,\ 0,\ w)$ | $(-1,\ 0,\ 0)$ | $\{1\}\oplus\{3\}$ or $\{2\}\oplus\{4\}$ | $(0,\ -1,\ 0)$ | $\{1\}\oplus\{4\}$ or $\{2\}\oplus\{3\}$ |
| 67 | LD$(0,\ 0,\ w)$ | $(-1,\ 0,\ 0)$ | $\{1\}\oplus\{3\}$ or $\{2\}\oplus\{4\}$ | $(0,\ -1,\ 0)$ | $\{1\}\oplus\{4\}$ or $\{2\}\oplus\{3\}$ |
| 67 | SM$(u,\ 0,\ 0)$ | $(0,\ -1,\ 0)$ | $\{1\}\oplus\{3\}$ or $\{2\}\oplus\{4\}$ | $(0,\ 0,\ 1)$ | $\{1\}\oplus\{4\}$ or $\{2\}\oplus\{3\}$ |
| 68 | DT$(0,\ v,\ 0)$ | $(0,\ 0,\ 1)$ | $\{1\}\oplus\{3\}$ or $\{2\}\oplus\{4\}$ | $(-1,\ 0,\ 0)$ | $\{1\}\oplus\{4\}$ or $\{2\}\oplus\{3\}$ |
| 68 | H$(1,\ 0,\ w)$ | $(-1,\ 0,\ 0)$ | $\{1\}\oplus\{3\}$ or $\{2\}\oplus\{4\}$ | $(0,\ -1,\ 0)$ | $\{1\}\oplus\{4\}$ or $\{2\}\oplus\{3\}$ |
| 68 | LD$(0,\ 0,\ w)$ | $(-1,\ 0,\ 0)$ | $\{1\}\oplus\{3\}$ or $\{2\}\oplus\{4\}$ | $(0,\ -1,\ 0)$ | $\{1\}\oplus\{4\}$ or $\{2\}\oplus\{3\}$ |
| 68 | SM$(u,\ 0,\ 0)$ | $(0,\ -1,\ 0)$ | $\{1\}\oplus\{3\}$ or $\{2\}\oplus\{4\}$ | $(0,\ 0,\ 1)$ | $\{1\}\oplus\{4\}$ or $\{2\}\oplus\{3\}$ |
| 69 | A$(u,\ 0,\ 1)$ | $(0,\ 1,\ 0)$ | $\{1\}\oplus\{3\}$ or $\{2\}\oplus\{4\}$ | $(0,\ 0,\ -1)$ | $\{1\}\oplus\{4\}$ or $\{2\}\oplus\{3\}$ |
| 69 | B$(0,\ v,\ 1)$ | $(0,\ 0,\ -1)$ | $\{1\}\oplus\{3\}$ or $\{2\}\oplus\{4\}$ | $(1,\ 0,\ 0)$ | $\{1\}\oplus\{4\}$ or $\{2\}\oplus\{3\}$ |
| 69 | DT$(0,\ v,\ 0)$ | $(0,\ 0,\ -1)$ | $\{1\}\oplus\{3\}$ or $\{2\}\oplus\{4\}$ | $(1,\ 0,\ 0)$ | $\{1\}\oplus\{4\}$ or $\{2\}\oplus\{3\}$ |
| 69 | H$(0,\ 1,\ w)$ | $(1,\ 0,\ 0)$ | $\{1\}\oplus\{3\}$ or $\{2\}\oplus\{4\}$ | $(0,\ 1,\ 0)$ | $\{1\}\oplus\{4\}$ or $\{2\}\oplus\{3\}$ |
| 69 | LD$(0,\ 0,\ w)$ | $(1,\ 0,\ 0)$ | $\{1\}\oplus\{3\}$ or $\{2\}\oplus\{4\}$ | $(0,\ 1,\ 0)$ | $\{1\}\oplus\{4\}$ or $\{2\}\oplus\{3\}$ |
| 69 | SM$(u,\ 0,\ 0)$ | $(0,\ 1,\ 0)$ | $\{1\}\oplus\{3\}$ or $\{2\}\oplus\{4\}$ | $(0,\ 0,\ -1)$ | $\{1\}\oplus\{4\}$ or $\{2\}\oplus\{3\}$ |
| 70 | DT$(0,\ v,\ 0)$ | $(1,\ 0,\ 0)$ | $\{1\}\oplus\{3\}$ or $\{2\}\oplus\{4\}$ | $(0,\ 0,\ -1)$ | $\{1\}\oplus\{4\}$ or $\{2\}\oplus\{3\}$ |
| 70 | LD$(0,\ 0,\ w)$ | $(0,\ -1,\ 0)$ | $\{1\}\oplus\{3\}$ or $\{2\}\oplus\{4\}$ | $(1,\ 0,\ 0)$ | $\{1\}\oplus\{4\}$ or $\{2\}\oplus\{3\}$ |

| SG | HSL | Location of nodal loop 1 | Irreps of BC | Location of nodal loop 2 | Irreps of BC |
|---|---|---|---|---|---|
| 70 | SM$(u,\ 0,\ 0)$ | $(0,\ 0,\ -1)$ | $\{1\}\oplus\{3\}$ or $\{2\}\oplus\{4\}$ | $(0,\ -1,\ 0)$ | $\{1\}\oplus\{4\}$ or $\{2\}\oplus\{3\}$ |
| 71 | DT$(0,\ v,\ 0)$ | $(0,\ 0,\ -1)$ | $\{1\}\oplus\{3\}$ or $\{2\}\oplus\{4\}$ | $(1,\ 0,\ 0)$ | $\{1\}\oplus\{4\}$ or $\{2\}\oplus\{3\}$ |
| 71 | LD$(0,\ 0,\ w)$ | $(1,\ 0,\ 0)$ | $\{1\}\oplus\{3\}$ or $\{2\}\oplus\{4\}$ | $(0,\ -1,\ 0)$ | $\{1\}\oplus\{4\}$ or $\{2\}\oplus\{3\}$ |
| 71 | SM$(u,\ 0,\ 0)$ | $(0,\ -1,\ 0)$ | $\{1\}\oplus\{3\}$ or $\{2\}\oplus\{4\}$ | $(0,\ 0,\ -1)$ | $\{1\}\oplus\{4\}$ or $\{2\}\oplus\{3\}$ |
| 72 | DT$(0,\ v,\ 0)$ | $(0,\ 0,\ -1)$ | $\{1\}\oplus\{3\}$ or $\{2\}\oplus\{4\}$ | $(1,\ 0,\ 0)$ | $\{1\}\oplus\{4\}$ or $\{2\}\oplus\{3\}$ |
| 72 | LD$(0,\ 0,\ w)$ | $(1,\ 0,\ 0)$ | $\{1\}\oplus\{3\}$ or $\{2\}\oplus\{4\}$ | $(0,\ -1,\ 0)$ | $\{1\}\oplus\{4\}$ or $\{2\}\oplus\{3\}$ |
| 72 | SM$(u,\ 0,\ 0)$ | $(0,\ -1,\ 0)$ | $\{1\}\oplus\{3\}$ or $\{2\}\oplus\{4\}$ | $(0,\ 0,\ -1)$ | $\{1\}\oplus\{4\}$ or $\{2\}\oplus\{3\}$ |
| 73 | DT$(0,\ v,\ 0)$ | $(0,\ 0,\ -1)$ | $\{1\}\oplus\{3\}$ or $\{2\}\oplus\{4\}$ | $(1,\ 0,\ 0)$ | $\{1\}\oplus\{4\}$ or $\{2\}\oplus\{3\}$ |
| 73 | LD$(0,\ 0,\ w)$ | $(1,\ 0,\ 0)$ | $\{1\}\oplus\{3\}$ or $\{2\}\oplus\{4\}$ | $(0,\ -1,\ 0)$ | $\{1\}\oplus\{4\}$ or $\{2\}\oplus\{3\}$ |
| 73 | SM$(u,\ 0,\ 0)$ | $(0,\ -1,\ 0)$ | $\{1\}\oplus\{3\}$ or $\{2\}\oplus\{4\}$ | $(0,\ 0,\ -1)$ | $\{1\}\oplus\{4\}$ or $\{2\}\oplus\{3\}$ |
| 74 | DT$(0,\ v,\ 0)$ | $(0,\ 0,\ -1)$ | $\{1\}\oplus\{3\}$ or $\{2\}\oplus\{4\}$ | $(1,\ 0,\ 0)$ | $\{1\}\oplus\{4\}$ or $\{2\}\oplus\{3\}$ |
| 74 | LD$(0,\ 0,\ w)$ | $(1,\ 0,\ 0)$ | $\{1\}\oplus\{3\}$ or $\{2\}\oplus\{4\}$ | $(0,\ -1,\ 0)$ | $\{1\}\oplus\{4\}$ or $\{2\}\oplus\{3\}$ |
| 74 | SM$(u,\ 0,\ 0)$ | $(0,\ -1,\ 0)$ | $\{1\}\oplus\{3\}$ or $\{2\}\oplus\{4\}$ | $(0,\ 0,\ -1)$ | $\{1\}\oplus\{4\}$ or $\{2\}\oplus\{3\}$ |
| 99 | W$\left(0,\ \frac{1}{2},\ w\right)$ | $(1,\ 0,\ 0)$ | $1\oplus3$ or $2\oplus4$ | $(0,\ -1,\ 0)$ | $1\oplus4$ or $2\oplus3$ |
| 101 | W$\left(0,\ \frac{1}{2},\ w\right)$ | $(1,\ 0,\ 0)$ | $1\oplus3$ or $2\oplus4$ | $(0,\ -1,\ 0)$ | $1\oplus4$ or $2\oplus3$ |
| 103 | W$\left(0,\ \frac{1}{2},\ w\right)$ | $(1,\ 0,\ 0)$ | $1\oplus3$ or $2\oplus4$ | $(0,\ -1,\ 0)$ | $1\oplus4$ or $2\oplus3$ |
| 105 | W$\left(0,\ \frac{1}{2},\ w\right)$ | $(1,\ 0,\ 0)$ | $1\oplus3$ or $2\oplus4$ | $(0,\ -1,\ 0)$ | $1\oplus4$ or $2\oplus3$ |
| 107 | W$\left(\frac{1}{2},\ \frac{1}{2},\ w\right)$ | $\left(-\frac{\sqrt{2}}{2},\ -\frac{\sqrt{2}}{2},\ 0\right)$ | $1\oplus3$ or $2\oplus4$ | $\left(\frac{\sqrt{2}}{2},\ -\frac{\sqrt{2}}{2},\ 0\right)$ | $1\oplus4$ or $2\oplus3$ |
| 108 | W$\left(\frac{1}{2},\ \frac{1}{2},\ w\right)$ | $\left(-\frac{\sqrt{2}}{2},\ -\frac{\sqrt{2}}{2},\ 0\right)$ | $1\oplus3$ or $2\oplus4$ | $\left(\frac{\sqrt{2}}{2},\ -\frac{\sqrt{2}}{2},\ 0\right)$ | $1\oplus4$ or $2\oplus3$ |
| 115 | W$\left(0,\ \frac{1}{2},\ w\right)$ | $(1,\ 0,\ 0)$ | $1\oplus3$ or $2\oplus4$ | $(0,\ -1,\ 0)$ | $1\oplus4$ or $2\oplus3$ |
| 116 | W$\left(0,\ \frac{1}{2},\ w\right)$ | $(1,\ 0,\ 0)$ | $1\oplus3$ or $2\oplus4$ | $(0,\ -1,\ 0)$ | $1\oplus4$ or $2\oplus3$ |
| 121 | W$\left(\frac{1}{2},\ \frac{1}{2},\ w\right)$ | $\left(-\frac{\sqrt{2}}{2},\ -\frac{\sqrt{2}}{2},\ 0\right)$ | $1\oplus3$ or $2\oplus4$ | $\left(-\frac{\sqrt{2}}{2},\ \frac{\sqrt{2}}{2},\ 0\right)$ | $1\oplus4$ or $2\oplus3$ |
| 123 | DT$(0,\ v,\ 0)$ | $(0,\ 0,\ 1)$ | $\{1\}\oplus\{3\}$ or $\{2\}\oplus\{4\}$ | $(1,\ 0,\ 0)$ | $\{1\}\oplus\{4\}$ or $\{2\}\oplus\{3\}$ |
| 123 | S$\left(u,\ u,\ \frac{1}{2}\right)$ | $\left(\frac{\sqrt{2}}{2},\ -\frac{\sqrt{2}}{2},\ 0\right)$ | $\{1\}\oplus\{3\}$ or $\{2\}\oplus\{4\}$ | $(0,\ 0,\ 1)$ | $\{1\}\oplus\{4\}$ or $\{2\}\oplus\{3\}$ |
| 123 | SM$(u,\ u,\ 0)$ | $\left(\frac{\sqrt{2}}{2},\ -\frac{\sqrt{2}}{2},\ 0\right)$ | $\{1\}\oplus\{3\}$ or $\{2\}\oplus\{4\}$ | $(0,\ 0,\ 1)$ | $\{1\}\oplus\{4\}$ or $\{2\}\oplus\{3\}$ |
| 123 | T$\left(u,\ \frac{1}{2},\ \frac{1}{2}\right)$ | $(0,\ -1,\ 0)$ | $\{1\}\oplus\{3\}$ or $\{2\}\oplus\{4\}$ | $(0,\ 0,\ 1)$ | $\{1\}\oplus\{4\}$ or $\{2\}\oplus\{3\}$ |
| 123 | U$\left(0,\ v,\ \frac{1}{2}\right)$ | $(0,\ 0,\ 1)$ | $\{1\}\oplus\{3\}$ or $\{2\}\oplus\{4\}$ | $(1,\ 0,\ 0)$ | $\{1\}\oplus\{4\}$ or $\{2\}\oplus\{3\}$ |
| 123 | W$\left(0,\ \frac{1}{2},\ w\right)$ | $(1,\ 0,\ 0)$ | $\{1\}\oplus\{3\}$ or $\{2\}\oplus\{4\}$ | $(0,\ -1,\ 0)$ | $\{1\}\oplus\{4\}$ or $\{2\}\oplus\{3\}$ |
| 123 | Y$\left(u,\ \frac{1}{2},\ 0\right)$ | $(0,\ -1,\ 0)$ | $\{1\}\oplus\{3\}$ or $\{2\}\oplus\{4\}$ | $(0,\ 0,\ 1)$ | $\{1\}\oplus\{4\}$ or $\{2\}\oplus\{3\}$ |
| 124 | DT$(0,\ v,\ 0)$ | $(0,\ 0,\ 1)$ | $\{1\}\oplus\{3\}$ or $\{2\}\oplus\{4\}$ | $(1,\ 0,\ 0)$ | $\{1\}\oplus\{4\}$ or $\{2\}\oplus\{3\}$ |
| 124 | SM$(u,\ u,\ 0)$ | $\left(\frac{\sqrt{2}}{2},\ -\frac{\sqrt{2}}{2},\ 0\right)$ | $\{1\}\oplus\{3\}$ or $\{2\}\oplus\{4\}$ | $(0,\ 0,\ 1)$ | $\{1\}\oplus\{4\}$ or $\{2\}\oplus\{3\}$ |
| 124 | W$\left(0,\ \frac{1}{2},\ w\right)$ | $(1,\ 0,\ 0)$ | $\{1\}\oplus\{3\}$ or $\{2\}\oplus\{4\}$ | $(0,\ -1,\ 0)$ | $\{1\}\oplus\{4\}$ or $\{2\}\oplus\{3\}$ |
| 124 | Y$\left(u,\ \frac{1}{2},\ 0\right)$ | $(0,\ -1,\ 0)$ | $\{1\}\oplus\{3\}$ or $\{2\}\oplus\{4\}$ | $(0,\ 0,\ 1)$ | $\{1\}\oplus\{4\}$ or $\{2\}\oplus\{3\}$ |
| 125 | DT$(0,\ v,\ 0)$ | $(0,\ 0,\ 1)$ | $\{1\}\oplus\{3\}$ or $\{2\}\oplus\{4\}$ | $(1,\ 0,\ 0)$ | $\{1\}\oplus\{4\}$ or $\{2\}\oplus\{3\}$ |
| 125 | S$\left(u,\ u,\ \frac{1}{2}\right)$ | $\left(\frac{\sqrt{2}}{2},\ -\frac{\sqrt{2}}{2},\ 0\right)$ | $\{1\}\oplus\{3\}$ or $\{2\}\oplus\{4\}$ | $(0,\ 0,\ 1)$ | $\{1\}\oplus\{4\}$ or $\{2\}\oplus\{3\}$ |
| 125 | SM$(u,\ u,\ 0)$ | $\left(\frac{\sqrt{2}}{2},\ -\frac{\sqrt{2}}{2},\ 0\right)$ | $\{1\}\oplus\{3\}$ or $\{2\}\oplus\{4\}$ | $(0,\ 0,\ 1)$ | $\{1\}\oplus\{4\}$ or $\{2\}\oplus\{3\}$ |
| 125 | U$\left(0,\ v,\ \frac{1}{2}\right)$ | $(0,\ 0,\ 1)$ | $\{1\}\oplus\{3\}$ or $\{2\}\oplus\{4\}$ | $(1,\ 0,\ 0)$ | $\{1\}\oplus\{4\}$ or $\{2\}\oplus\{3\}$ |
| 126 | DT$(0,\ v,\ 0)$ | $(0,\ 0,\ 1)$ | $\{1\}\oplus\{3\}$ or $\{2\}\oplus\{4\}$ | $(1,\ 0,\ 0)$ | $\{1\}\oplus\{4\}$ or $\{2\}\oplus\{3\}$ |
| 126 | SM$(u,\ u,\ 0)$ | $\left(\frac{\sqrt{2}}{2},\ -\frac{\sqrt{2}}{2},\ 0\right)$ | $\{1\}\oplus\{3\}$ or $\{2\}\oplus\{4\}$ | $(0,\ 0,\ 1)$ | $\{1\}\oplus\{4\}$ or $\{2\}\oplus\{3\}$ |
| 126 | T$\left(u,\ \frac{1}{2},\ \frac{1}{2}\right)$ | $(0,\ 0,\ 1)$ | $\{1\}\oplus\{3\}$ or $\{2\}\oplus\{4\}$ | $(0,\ -1,\ 0)$ | $\{1\}\oplus\{4\}$ or $\{2\}\oplus\{3\}$ |

| SG | HSL | Location of nodal loop 1 | Irreps of BC | Location of nodal loop 2 | Irreps of BC |
|---|---|---|---|---|---|
| 127 | DT$(0,\ v,\ 0)$ | $(0,\ 0,\ 1)$ | $\{1\}\oplus\{3\}$ or $\{2\}\oplus\{4\}$ | $(1,\ 0,\ 0)$ | $\{1\}\oplus\{4\}$ or $\{2\}\oplus\{3\}$ |
| 127 | S$\left(u,\ u,\ \frac{1}{2}\right)$ | $\left(\frac{\sqrt{2}}{2},\ -\frac{\sqrt{2}}{2},\ 0\right)$ | $\{1\}\oplus\{3\}$ or $\{2\}\oplus\{4\}$ | $(0,\ 0,\ 1)$ | $\{1\}\oplus\{4\}$ or $\{2\}\oplus\{3\}$ |
| 127 | SM$(u,\ u,\ 0)$ | $\left(\frac{\sqrt{2}}{2},\ -\frac{\sqrt{2}}{2},\ 0\right)$ | $\{1\}\oplus\{3\}$ or $\{2\}\oplus\{4\}$ | $(0,\ 0,\ 1)$ | $\{1\}\oplus\{4\}$ or $\{2\}\oplus\{3\}$ |
| 127 | U$\left(0,\ v,\ \frac{1}{2}\right)$ | $(0,\ 0,\ 1)$ | $\{1\}\oplus\{3\}$ or $\{2\}\oplus\{4\}$ | $(1,\ 0,\ 0)$ | $\{1\}\oplus\{4\}$ or $\{2\}\oplus\{3\}$ |
| 128 | DT$(0,\ v,\ 0)$ | $(0,\ 0,\ 1)$ | $\{1\}\oplus\{3\}$ or $\{2\}\oplus\{4\}$ | $(1,\ 0,\ 0)$ | $\{1\}\oplus\{4\}$ or $\{2\}\oplus\{3\}$ |
| 128 | SM$(u,\ u,\ 0)$ | $\left(\frac{\sqrt{2}}{2},\ -\frac{\sqrt{2}}{2},\ 0\right)$ | $\{1\}\oplus\{3\}$ or $\{2\}\oplus\{4\}$ | $(0,\ 0,\ 1)$ | $\{1\}\oplus\{4\}$ or $\{2\}\oplus\{3\}$ |
| 129 | DT$(0,\ v,\ 0)$ | $(0,\ 0,\ 1)$ | $\{1\}\oplus\{3\}$ or $\{2\}\oplus\{4\}$ | $(1,\ 0,\ 0)$ | $\{1\}\oplus\{4\}$ or $\{2\}\oplus\{3\}$ |
| 129 | S$\left(u,\ u,\ \frac{1}{2}\right)$ | $\left(\frac{\sqrt{2}}{2},\ -\frac{\sqrt{2}}{2},\ 0\right)$ | $\{1\}\oplus\{3\}$ or $\{2\}\oplus\{4\}$ | $(0,\ 0,\ 1)$ | $\{1\}\oplus\{4\}$ or $\{2\}\oplus\{3\}$ |
| 129 | SM$(u,\ u,\ 0)$ | $\left(\frac{\sqrt{2}}{2},\ -\frac{\sqrt{2}}{2},\ 0\right)$ | $\{1\}\oplus\{3\}$ or $\{2\}\oplus\{4\}$ | $(0,\ 0,\ 1)$ | $\{1\}\oplus\{4\}$ or $\{2\}\oplus\{3\}$ |
| 129 | U$\left(0,\ v,\ \frac{1}{2}\right)$ | $(0,\ 0,\ 1)$ | $\{1\}\oplus\{3\}$ or $\{2\}\oplus\{4\}$ | $(1,\ 0,\ 0)$ | $\{1\}\oplus\{4\}$ or $\{2\}\oplus\{3\}$ |
| 130 | DT$(0,\ v,\ 0)$ | $(0,\ 0,\ 1)$ | $\{1\}\oplus\{3\}$ or $\{2\}\oplus\{4\}$ | $(1,\ 0,\ 0)$ | $\{1\}\oplus\{4\}$ or $\{2\}\oplus\{3\}$ |
| 130 | SM$(u,\ u,\ 0)$ | $\left(\frac{\sqrt{2}}{2},\ -\frac{\sqrt{2}}{2},\ 0\right)$ | $\{1\}\oplus\{3\}$ or $\{2\}\oplus\{4\}$ | $(0,\ 0,\ 1)$ | $\{1\}\oplus\{4\}$ or $\{2\}\oplus\{3\}$ |
| 131 | DT$(0,\ v,\ 0)$ | $(0,\ 0,\ 1)$ | $\{1\}\oplus\{3\}$ or $\{2\}\oplus\{4\}$ | $(1,\ 0,\ 0)$ | $\{1\}\oplus\{4\}$ or $\{2\}\oplus\{3\}$ |
| 131 | SM$(u,\ u,\ 0)$ | $\left(\frac{\sqrt{2}}{2},\ -\frac{\sqrt{2}}{2},\ 0\right)$ | $\{1\}\oplus\{3\}$ or $\{2\}\oplus\{4\}$ | $(0,\ 0,\ 1)$ | $\{1\}\oplus\{4\}$ or $\{2\}\oplus\{3\}$ |
| 131 | T$\left(u,\ \frac{1}{2},\ \frac{1}{2}\right)$ | $(0,\ -1,\ 0)$ | $\{1\}\oplus\{3\}$ or $\{2\}\oplus\{4\}$ | $(0,\ 0,\ 1)$ | $\{1\}\oplus\{4\}$ or $\{2\}\oplus\{3\}$ |
| 131 | U$\left(0,\ v,\ \frac{1}{2}\right)$ | $(0,\ 0,\ 1)$ | $\{1\}\oplus\{3\}$ or $\{2\}\oplus\{4\}$ | $(1,\ 0,\ 0)$ | $\{1\}\oplus\{4\}$ or $\{2\}\oplus\{3\}$ |
| 131 | W$\left(0,\ \frac{1}{2},\ w\right)$ | $(1,\ 0,\ 0)$ | $\{1\}\oplus\{3\}$ or $\{2\}\oplus\{4\}$ | $(0,\ -1,\ 0)$ | $\{1\}\oplus\{4\}$ or $\{2\}\oplus\{3\}$ |
| 131 | Y$\left(u,\ \frac{1}{2},\ 0\right)$ | $(0,\ -1,\ 0)$ | $\{1\}\oplus\{3\}$ or $\{2\}\oplus\{4\}$ | $(0,\ 0,\ 1)$ | $\{1\}\oplus\{4\}$ or $\{2\}\oplus\{3\}$ |
| 132 | DT$(0,\ v,\ 0)$ | $(0,\ 0,\ 1)$ | $\{1\}\oplus\{3\}$ or $\{2\}\oplus\{4\}$ | $(1,\ 0,\ 0)$ | $\{1\}\oplus\{4\}$ or $\{2\}\oplus\{3\}$ |
| 132 | S$\left(u,\ u,\ \frac{1}{2}\right)$ | $(0,\ 0,\ 1)$ | $\{1\}\oplus\{2\}$ or $\{3\}\oplus\{4\}$ | $\left(\frac{\sqrt{2}}{2},\ -\frac{\sqrt{2}}{2},\ 0\right)$ | $\{1\}\oplus\{4\}$ or $\{2\}\oplus\{3\}$ |
| 132 | SM$(u,\ u,\ 0)$ | $\left(\frac{\sqrt{2}}{2},\ -\frac{\sqrt{2}}{2},\ 0\right)$ | $\{1\}\oplus\{3\}$ or $\{2\}\oplus\{4\}$ | $(0,\ 0,\ 1)$ | $\{1\}\oplus\{4\}$ or $\{2\}\oplus\{3\}$ |
| 132 | W$\left(0,\ \frac{1}{2},\ w\right)$ | $(1,\ 0,\ 0)$ | $\{1\}\oplus\{3\}$ or $\{2\}\oplus\{4\}$ | $(0,\ -1,\ 0)$ | $\{1\}\oplus\{4\}$ or $\{2\}\oplus\{3\}$ |
| 132 | Y$\left(u,\ \frac{1}{2},\ 0\right)$ | $(0,\ -1,\ 0)$ | $\{1\}\oplus\{3\}$ or $\{2\}\oplus\{4\}$ | $(0,\ 0,\ 1)$ | $\{1\}\oplus\{4\}$ or $\{2\}\oplus\{3\}$ |
| 133 | DT$(0,\ v,\ 0)$ | $(0,\ 0,\ 1)$ | $\{1\}\oplus\{3\}$ or $\{2\}\oplus\{4\}$ | $(1,\ 0,\ 0)$ | $\{1\}\oplus\{4\}$ or $\{2\}\oplus\{3\}$ |
| 133 | SM$(u,\ u,\ 0)$ | $\left(\frac{\sqrt{2}}{2},\ -\frac{\sqrt{2}}{2},\ 0\right)$ | $\{1\}\oplus\{3\}$ or $\{2\}\oplus\{4\}$ | $(0,\ 0,\ 1)$ | $\{1\}\oplus\{4\}$ or $\{2\}\oplus\{3\}$ |
| 133 | U$\left(0,\ v,\ \frac{1}{2}\right)$ | $(0,\ 0,\ 1)$ | $\{1\}\oplus\{3\}$ or $\{2\}\oplus\{4\}$ | $(1,\ 0,\ 0)$ | $\{1\}\oplus\{4\}$ or $\{2\}\oplus\{3\}$ |
| 134 | DT$(0,\ v,\ 0)$ | $(0,\ 0,\ 1)$ | $\{1\}\oplus\{3\}$ or $\{2\}\oplus\{4\}$ | $(1,\ 0,\ 0)$ | $\{1\}\oplus\{4\}$ or $\{2\}\oplus\{3\}$ |
| 134 | S$\left(u,\ u,\ \frac{1}{2}\right)$ | $(0,\ 0,\ 1)$ | $\{1\}\oplus\{2\}$ or $\{3\}\oplus\{4\}$ | $\left(\frac{\sqrt{2}}{2},\ -\frac{\sqrt{2}}{2},\ 0\right)$ | $\{1\}\oplus\{4\}$ or $\{2\}\oplus\{3\}$ |
| 134 | SM$(u,\ u,\ 0)$ | $\left(\frac{\sqrt{2}}{2},\ -\frac{\sqrt{2}}{2},\ 0\right)$ | $\{1\}\oplus\{3\}$ or $\{2\}\oplus\{4\}$ | $(0,\ 0,\ 1)$ | $\{1\}\oplus\{4\}$ or $\{2\}\oplus\{3\}$ |
| 134 | T$\left(u,\ \frac{1}{2},\ \frac{1}{2}\right)$ | $(0,\ 0,\ 1)$ | $\{1\}\oplus\{3\}$ or $\{2\}\oplus\{4\}$ | $(0,\ -1,\ 0)$ | $\{1\}\oplus\{4\}$ or $\{2\}\oplus\{3\}$ |
| 135 | DT$(0,\ v,\ 0)$ | $(0,\ 0,\ 1)$ | $\{1\}\oplus\{3\}$ or $\{2\}\oplus\{4\}$ | $(1,\ 0,\ 0)$ | $\{1\}\oplus\{4\}$ or $\{2\}\oplus\{3\}$ |
| 135 | SM$(u,\ u,\ 0)$ | $\left(\frac{\sqrt{2}}{2},\ -\frac{\sqrt{2}}{2},\ 0\right)$ | $\{1\}\oplus\{3\}$ or $\{2\}\oplus\{4\}$ | $(0,\ 0,\ 1)$ | $\{1\}\oplus\{4\}$ or $\{2\}\oplus\{3\}$ |
| 135 | U$\left(0,\ v,\ \frac{1}{2}\right)$ | $(0,\ 0,\ 1)$ | $\{1\}\oplus\{3\}$ or $\{2\}\oplus\{4\}$ | $(1,\ 0,\ 0)$ | $\{1\}\oplus\{4\}$ or $\{2\}\oplus\{3\}$ |
| 136 | DT$(0,\ v,\ 0)$ | $(0,\ 0,\ 1)$ | $\{1\}\oplus\{3\}$ or $\{2\}\oplus\{4\}$ | $(1,\ 0,\ 0)$ | $\{1\}\oplus\{4\}$ or $\{2\}\oplus\{3\}$ |
| 136 | S$\left(u,\ u,\ \frac{1}{2}\right)$ | $(0,\ 0,\ 1)$ | $\{1\}\oplus\{2\}$ or $\{3\}\oplus\{4\}$ | $\left(\frac{\sqrt{2}}{2},\ -\frac{\sqrt{2}}{2},\ 0\right)$ | $\{1\}\oplus\{4\}$ or $\{2\}\oplus\{3\}$ |
| 136 | SM$(u,\ u,\ 0)$ | $\left(\frac{\sqrt{2}}{2},\ -\frac{\sqrt{2}}{2},\ 0\right)$ | $\{1\}\oplus\{3\}$ or $\{2\}\oplus\{4\}$ | $(0,\ 0,\ 1)$ | $\{1\}\oplus\{4\}$ or $\{2\}\oplus\{3\}$ |
| 137 | DT$(0,\ v,\ 0)$ | $(0,\ 0,\ 1)$ | $\{1\}\oplus\{3\}$ or $\{2\}\oplus\{4\}$ | $(1,\ 0,\ 0)$ | $\{1\}\oplus\{4\}$ or $\{2\}\oplus\{3\}$ |
| 137 | SM$(u,\ u,\ 0)$ | $\left(\frac{\sqrt{2}}{2},\ -\frac{\sqrt{2}}{2},\ 0\right)$ | $\{1\}\oplus\{3\}$ or $\{2\}\oplus\{4\}$ | $(0,\ 0,\ 1)$ | $\{1\}\oplus\{4\}$ or $\{2\}\oplus\{3\}$ |
| 137 | U$\left(0,\ v,\ \frac{1}{2}\right)$ | $(0,\ 0,\ 1)$ | $\{1\}\oplus\{3\}$ or $\{2\}\oplus\{4\}$ | $(1,\ 0,\ 0)$ | $\{1\}\oplus\{4\}$ or $\{2\}\oplus\{3\}$ |

| SG | HSL | Location of nodal loop 1 | Irreps of BC | Location of nodal loop 2 | Irreps of BC |
|---|---|---|---|---|---|
| 138 | DT$(0,\ v,\ 0)$ | $(0,\ 0,\ 1)$ | $\{1\}\oplus\{3\}$ or $\{2\}\oplus\{4\}$ | $(1,\ 0,\ 0)$ | $\{1\}\oplus\{4\}$ or $\{2\}\oplus\{3\}$ |
| 138 | S$(u,\ u,\ \frac{1}{2})$ | $(0,\ 0,\ 1)$ | $\{1\}\oplus\{2\}$ or $\{3\}\oplus\{4\}$ | $\left(\frac{\sqrt{2}}{2},\ -\frac{\sqrt{2}}{2},\ 0\right)$ | $\{1\}\oplus\{4\}$ or $\{2\}\oplus\{3\}$ |
| 138 | SM$(u,\ u,\ 0)$ | $\left(\frac{\sqrt{2}}{2},\ -\frac{\sqrt{2}}{2},\ 0\right)$ | $\{1\}\oplus\{3\}$ or $\{2\}\oplus\{4\}$ | $(0,\ 0,\ 1)$ | $\{1\}\oplus\{4\}$ or $\{2\}\oplus\{3\}$ |
| 139 | DT$(u,\ u,\ 0)$ | $\left(\frac{\sqrt{2}}{2},\ -\frac{\sqrt{2}}{2},\ 0\right)$ | $\{1\}\oplus\{3\}$ or $\{2\}\oplus\{4\}$ | $(0,\ 0,\ -1)$ | $\{1\}\oplus\{4\}$ or $\{2\}\oplus\{3\}$ |
| 139 | SM$(u,\ 0,\ 0)$ | $(0,\ 1,\ 0)$ | $\{1\}\oplus\{3\}$ or $\{2\}\oplus\{4\}$ | $(0,\ 0,\ -1)$ | $\{1\}\oplus\{4\}$ or $\{2\}\oplus\{3\}$ |
| 139 | W$(\frac{1}{2},\ \frac{1}{2},\ w)$ | $\left(-\frac{\sqrt{2}}{2},\ -\frac{\sqrt{2}}{2},\ 0\right)$ | $\{1\}\oplus\{3\}$ or $\{2\}\oplus\{4\}$ | $\left(\frac{\sqrt{2}}{2},\ -\frac{\sqrt{2}}{2},\ 0\right)$ | $\{1\}\oplus\{4\}$ or $\{2\}\oplus\{3\}$ |
| 139 | Y$(u,\ 1-u,\ 0)$ | $(0,\ 0,\ -1)$ | $\{1\}\oplus\{3\}$ or $\{2\}\oplus\{4\}$ | $\left(-\frac{\sqrt{2}}{2},\ -\frac{\sqrt{2}}{2},\ 0\right)$ | $\{1\}\oplus\{4\}$ or $\{2\}\oplus\{3\}$ |
| 140 | DT$(u,\ u,\ 0)$ | $\left(\frac{\sqrt{2}}{2},\ -\frac{\sqrt{2}}{2},\ 0\right)$ | $\{1\}\oplus\{3\}$ or $\{2\}\oplus\{4\}$ | $(0,\ 0,\ -1)$ | $\{1\}\oplus\{4\}$ or $\{2\}\oplus\{3\}$ |
| 140 | SM$(u,\ 0,\ 0)$ | $(0,\ 1,\ 0)$ | $\{1\}\oplus\{3\}$ or $\{2\}\oplus\{4\}$ | $(0,\ 0,\ -1)$ | $\{1\}\oplus\{4\}$ or $\{2\}\oplus\{3\}$ |
| 140 | W$(\frac{1}{2},\ \frac{1}{2},\ w)$ | $\left(-\frac{\sqrt{2}}{2},\ -\frac{\sqrt{2}}{2},\ 0\right)$ | $\{1\}\oplus\{3\}$ or $\{2\}\oplus\{4\}$ | $\left(\frac{\sqrt{2}}{2},\ -\frac{\sqrt{2}}{2},\ 0\right)$ | $\{1\}\oplus\{4\}$ or $\{2\}\oplus\{3\}$ |
| 140 | Y$(u,\ 1-u,\ 0)$ | $(0,\ 0,\ -1)$ | $\{1\}\oplus\{3\}$ or $\{2\}\oplus\{4\}$ | $\left(-\frac{\sqrt{2}}{2},\ -\frac{\sqrt{2}}{2},\ 0\right)$ | $\{1\}\oplus\{4\}$ or $\{2\}\oplus\{3\}$ |
| 141 | DT$(u,\ u,\ 0)$ | $\left(\frac{\sqrt{2}}{2},\ -\frac{\sqrt{2}}{2},\ 0\right)$ | $\{1\}\oplus\{3\}$ or $\{2\}\oplus\{4\}$ | $(0,\ 0,\ -1)$ | $\{1\}\oplus\{4\}$ or $\{2\}\oplus\{3\}$ |
| 141 | SM$(u,\ 0,\ 0)$ | $(0,\ 1,\ 0)$ | $\{1\}\oplus\{3\}$ or $\{2\}\oplus\{4\}$ | $(0,\ 0,\ -1)$ | $\{1\}\oplus\{4\}$ or $\{2\}\oplus\{3\}$ |
| 142 | DT$(u,\ u,\ 0)$ | $\left(-\frac{\sqrt{2}}{2},\ \frac{\sqrt{2}}{2},\ 0\right)$ | $\{1\}\oplus\{3\}$ or $\{2\}\oplus\{4\}$ | $(0,\ 0,\ -1)$ | $\{1\}\oplus\{4\}$ or $\{2\}\oplus\{3\}$ |
| 142 | SM$(u,\ 0,\ 0)$ | $(0,\ -1,\ 0)$ | $\{1\}\oplus\{3\}$ or $\{2\}\oplus\{4\}$ | $(0,\ 0,\ -1)$ | $\{1\}\oplus\{4\}$ or $\{2\}\oplus\{3\}$ |
| 183 | U$(\frac{1}{2},\ 0,\ w)$ | $\left(-\frac{\sqrt{3}}{2},\ -\frac{1}{2},\ 0\right)$ | $1\oplus3$ or $2\oplus4$ | $\left(\frac{1}{2},\ -\frac{\sqrt{3}}{2},\ 0\right)$ | $1\oplus4$ or $2\oplus3$ |
| 184 | U$(\frac{1}{2},\ 0,\ w)$ | $\left(-\frac{\sqrt{3}}{2},\ -\frac{1}{2},\ 0\right)$ | $1\oplus3$ or $2\oplus4$ | $\left(\frac{1}{2},\ -\frac{\sqrt{3}}{2},\ 0\right)$ | $1\oplus4$ or $2\oplus3$ |
| 185 | U$(\frac{1}{2},\ 0,\ w)$ | $\left(-\frac{\sqrt{3}}{2},\ -\frac{1}{2},\ 0\right)$ | $1\oplus3$ or $2\oplus4$ | $\left(\frac{1}{2},\ -\frac{\sqrt{3}}{2},\ 0\right)$ | $1\oplus4$ or $2\oplus3$ |
| 186 | U$(\frac{1}{2},\ 0,\ w)$ | $\left(-\frac{\sqrt{3}}{2},\ -\frac{1}{2},\ 0\right)$ | $1\oplus3$ or $2\oplus4$ | $\left(\frac{1}{2},\ -\frac{\sqrt{3}}{2},\ 0\right)$ | $1\oplus4$ or $2\oplus3$ |
| 187 | R$(u,\ 0,\ \frac{1}{2})$ | $(0,\ 0,\ 1)$ | $1\oplus3$ or $2\oplus4$ | $\left(-\frac{1}{2},\ \frac{\sqrt{3}}{2},\ 0\right)$ | $1\oplus4$ or $2\oplus3$ |
| 187 | SM$(u,\ 0,\ 0)$ | $(0,\ 0,\ 1)$ | $1\oplus3$ or $2\oplus4$ | $\left(-\frac{1}{2},\ \frac{\sqrt{3}}{2},\ 0\right)$ | $1\oplus4$ or $2\oplus3$ |
| 188 | SM$(u,\ 0,\ 0)$ | $(0,\ 0,\ 1)$ | $1\oplus3$ or $2\oplus4$ | $\left(-\frac{1}{2},\ \frac{\sqrt{3}}{2},\ 0\right)$ | $1\oplus4$ or $2\oplus3$ |
| 189 | LD$(u,\ u,\ 0)$ | $(0,\ 0,\ 1)$ | $1\oplus3$ or $2\oplus4$ | $\left(\frac{\sqrt{3}}{2},\ -\frac{1}{2},\ 0\right)$ | $1\oplus4$ or $2\oplus3$ |
| 189 | Q$(u,\ u,\ \frac{1}{2})$ | $(0,\ 0,\ 1)$ | $1\oplus3$ or $2\oplus4$ | $\left(\frac{\sqrt{3}}{2},\ -\frac{1}{2},\ 0\right)$ | $1\oplus4$ or $2\oplus3$ |
| 190 | LD$(u,\ u,\ 0)$ | $(0,\ 0,\ 1)$ | $1\oplus3$ or $2\oplus4$ | $\left(\frac{\sqrt{3}}{2},\ -\frac{1}{2},\ 0\right)$ | $1\oplus4$ or $2\oplus3$ |
| 191 | LD$(u,\ u,\ 0)$ | $(0,\ 0,\ 1)$ | $\{1\}\oplus\{3\}$ or $\{2\}\oplus\{4\}$ | $\left(-\frac{\sqrt{3}}{2},\ \frac{1}{2},\ 0\right)$ | $\{1\}\oplus\{4\}$ or $\{2\}\oplus\{3\}$ |
| 191 | Q$(u,\ u,\ \frac{1}{2})$ | $(0,\ 0,\ 1)$ | $\{1\}\oplus\{3\}$ or $\{2\}\oplus\{4\}$ | $\left(-\frac{\sqrt{3}}{2},\ \frac{1}{2},\ 0\right)$ | $\{1\}\oplus\{4\}$ or $\{2\}\oplus\{3\}$ |
| 191 | R$(u,\ 0,\ \frac{1}{2})$ | $(0,\ 0,\ 1)$ | $\{1\}\oplus\{3\}$ or $\{2\}\oplus\{4\}$ | $\left(\frac{1}{2},\ -\frac{\sqrt{3}}{2},\ 0\right)$ | $\{1\}\oplus\{4\}$ or $\{2\}\oplus\{3\}$ |
| 191 | SM$(u,\ 0,\ 0)$ | $(0,\ 0,\ 1)$ | $\{1\}\oplus\{3\}$ or $\{2\}\oplus\{4\}$ | $\left(\frac{1}{2},\ -\frac{\sqrt{3}}{2},\ 0\right)$ | $\{1\}\oplus\{4\}$ or $\{2\}\oplus\{3\}$ |
| 191 | U$(\frac{1}{2},\ 0,\ w)$ | $\left(-\frac{\sqrt{3}}{2},\ -\frac{1}{2},\ 0\right)$ | $\{1\}\oplus\{3\}$ or $\{2\}\oplus\{4\}$ | $\left(\frac{1}{2},\ -\frac{\sqrt{3}}{2},\ 0\right)$ | $\{1\}\oplus\{4\}$ or $\{2\}\oplus\{3\}$ |
| 192 | LD$(u,\ u,\ 0)$ | $(0,\ 0,\ 1)$ | $\{1\}\oplus\{3\}$ or $\{2\}\oplus\{4\}$ | $\left(-\frac{\sqrt{3}}{2},\ \frac{1}{2},\ 0\right)$ | $\{1\}\oplus\{4\}$ or $\{2\}\oplus\{3\}$ |
| 192 | SM$(u,\ 0,\ 0)$ | $(0,\ 0,\ 1)$ | $\{1\}\oplus\{3\}$ or $\{2\}\oplus\{4\}$ | $\left(\frac{1}{2},\ -\frac{\sqrt{3}}{2},\ 0\right)$ | $\{1\}\oplus\{4\}$ or $\{2\}\oplus\{3\}$ |
| 192 | U$(\frac{1}{2},\ 0,\ w)$ | $\left(-\frac{\sqrt{3}}{2},\ -\frac{1}{2},\ 0\right)$ | $\{1\}\oplus\{3\}$ or $\{2\}\oplus\{4\}$ | $\left(\frac{1}{2},\ -\frac{\sqrt{3}}{2},\ 0\right)$ | $\{1\}\oplus\{4\}$ or $\{2\}\oplus\{3\}$ |
| 193 | LD$(u,\ u,\ 0)$ | $(0,\ 0,\ 1)$ | $\{1\}\oplus\{3\}$ or $\{2\}\oplus\{4\}$ | $\left(-\frac{\sqrt{3}}{2},\ \frac{1}{2},\ 0\right)$ | $\{1\}\oplus\{4\}$ or $\{2\}\oplus\{3\}$ |
| 193 | SM$(u,\ 0,\ 0)$ | $(0,\ 0,\ 1)$ | $\{1\}\oplus\{3\}$ or $\{2\}\oplus\{4\}$ | $\left(\frac{1}{2},\ -\frac{\sqrt{3}}{2},\ 0\right)$ | $\{1\}\oplus\{4\}$ or $\{2\}\oplus\{3\}$ |
| 193 | U$(\frac{1}{2},\ 0,\ w)$ | $\left(-\frac{\sqrt{3}}{2},\ -\frac{1}{2},\ 0\right)$ | $\{1\}\oplus\{3\}$ or $\{2\}\oplus\{4\}$ | $\left(\frac{1}{2},\ -\frac{\sqrt{3}}{2},\ 0\right)$ | $\{1\}\oplus\{4\}$ or $\{2\}\oplus\{3\}$ |
| 194 | LD$(u,\ u,\ 0)$ | $(0,\ 0,\ 1)$ | $\{1\}\oplus\{3\}$ or $\{2\}\oplus\{4\}$ | $\left(-\frac{\sqrt{3}}{2},\ \frac{1}{2},\ 0\right)$ | $\{1\}\oplus\{4\}$ or $\{2\}\oplus\{3\}$ |

| SG | HSL | Location of nodal loop 1 | Irreps of BC | Location of nodal loop 2 | Irreps of BC |
|---|---|---|---|---|---|
| 194 | SM$(u,\ 0,\ 0)$ | $(0,\ 0,\ 1)$ | $\{1\}\oplus\{3\}$ or $\{2\}\oplus\{4\}$ | $\left(\frac{1}{2},\ -\frac{\sqrt{3}}{2},\ 0\right)$ | $\{1\}\oplus\{4\}$ or $\{2\}\oplus\{3\}$ |
| 194 | U$\left(\frac{1}{2},\ 0,\ w\right)$ | $\left(-\frac{\sqrt{3}}{2},\ -\frac{1}{2},\ 0\right)$ | $\{1\}\oplus\{3\}$ or $\{2\}\oplus\{4\}$ | $\left(\frac{1}{2},\ -\frac{\sqrt{3}}{2},\ 0\right)$ | $\{1\}\oplus\{4\}$ or $\{2\}\oplus\{3\}$ |
| 200 | DT$(0,\ v,\ 0)$ | $(0,\ 0,\ 1)$ | $\{1\}\oplus\{3\}$ or $\{2\}\oplus\{4\}$ | $(1,\ 0,\ 0)$ | $\{1\}\oplus\{4\}$ or $\{2\}\oplus\{3\}$ |
| 200 | T$\left(\frac{1}{2},\ \frac{1}{2},\ w\right)$ | $(-1,\ 0,\ 0)$ | $\{1\}\oplus\{3\}$ or $\{2\}\oplus\{4\}$ | $(0,\ -1,\ 0)$ | $\{1\}\oplus\{4\}$ or $\{2\}\oplus\{3\}$ |
| 200 | ZA$\left(\frac{1}{2},\ u,\ 0\right)$ | $(-1,\ 0,\ 0)$ | $\{1\}\oplus\{3\}$ or $\{2\}\oplus\{4\}$ | $(0,\ 0,\ 1)$ | $\{1\}\oplus\{4\}$ or $\{2\}\oplus\{3\}$ |
| 200 | Z$\left(u,\ \frac{1}{2},\ 0\right)$ | $(0,\ -1,\ 0)$ | $\{1\}\oplus\{3\}$ or $\{2\}\oplus\{4\}$ | $(0,\ 0,\ 1)$ | $\{1\}\oplus\{4\}$ or $\{2\}\oplus\{3\}$ |
| 201 | DT$(0,\ v,\ 0)$ | $(0,\ 0,\ 1)$ | $\{1\}\oplus\{3\}$ or $\{2\}\oplus\{4\}$ | $(1,\ 0,\ 0)$ | $\{1\}\oplus\{4\}$ or $\{2\}\oplus\{3\}$ |
| 201 | T$\left(\frac{1}{2},\ \frac{1}{2},\ w\right)$ | $(-1,\ 0,\ 0)$ | $\{1\}\oplus\{3\}$ or $\{2\}\oplus\{4\}$ | $(0,\ -1,\ 0)$ | $\{1\}\oplus\{4\}$ or $\{2\}\oplus\{3\}$ |
| 202 | DT$(0,\ v,\ 0)$ | $(0,\ 0,\ -1)$ | $\{1\}\oplus\{3\}$ or $\{2\}\oplus\{4\}$ | $(-1,\ 0,\ 0)$ | $\{1\}\oplus\{4\}$ or $\{2\}\oplus\{3\}$ |
| 202 | V$(u,\ 1,\ 0)$ | $(0,\ -1,\ 0)$ | $\{1\}\oplus\{3\}$ or $\{2\}\oplus\{4\}$ | $(0,\ 0,\ -1)$ | $\{1\}\oplus\{4\}$ or $\{2\}\oplus\{3\}$ |
| 203 | DT$(0,\ v,\ 0)$ | $(0,\ 0,\ -1)$ | $\{1\}\oplus\{3\}$ or $\{2\}\oplus\{4\}$ | $(-1,\ 0,\ 0)$ | $\{1\}\oplus\{4\}$ or $\{2\}\oplus\{3\}$ |
| 204 | DT$(0,\ v,\ 0)$ | $(0,\ 0,\ -1)$ | $\{1\}\oplus\{3\}$ or $\{2\}\oplus\{4\}$ | $(-1,\ 0,\ 0)$ | $\{1\}\oplus\{4\}$ or $\{2\}\oplus\{3\}$ |
| 205 | DT$(0,\ v,\ 0)$ | $(0,\ 0,\ 1)$ | $\{1\}\oplus\{3\}$ or $\{2\}\oplus\{4\}$ | $(1,\ 0,\ 0)$ | $\{1\}\oplus\{4\}$ or $\{2\}\oplus\{3\}$ |
| 206 | DT$(0,\ v,\ 0)$ | $(0,\ 0,\ -1)$ | $\{1\}\oplus\{3\}$ or $\{2\}\oplus\{4\}$ | $(-1,\ 0,\ 0)$ | $\{1\}\oplus\{4\}$ or $\{2\}\oplus\{3\}$ |
| 217 | D$\left(\frac{1}{2},\ \frac{1}{2},\ w\right)$ | $\left(-\frac{\sqrt{2}}{2},\ -\frac{\sqrt{2}}{2},\ 0\right)$ | $1\oplus3$ or $2\oplus4$ | $\left(-\frac{\sqrt{2}}{2},\ \frac{\sqrt{2}}{2},\ 0\right)$ | $1\oplus4$ or $2\oplus3$ |
| 221 | S$\left(u,\ \frac{1}{2},\ u\right)$ | $\left(-\frac{\sqrt{2}}{2},\ 0,\ \frac{\sqrt{2}}{2}\right)$ | $\{1\}\oplus\{3\}$ or $\{2\}\oplus\{4\}$ | $(0,\ -1,\ 0)$ | $\{1\}\oplus\{4\}$ or $\{2\}\oplus\{3\}$ |
| 221 | SM$(u,\ u,\ 0)$ | $\left(\frac{\sqrt{2}}{2},\ -\frac{\sqrt{2}}{2},\ 0\right)$ | $\{1\}\oplus\{3\}$ or $\{2\}\oplus\{4\}$ | $(0,\ 0,\ 1)$ | $\{1\}\oplus\{4\}$ or $\{2\}\oplus\{3\}$ |
| 221 | Z$\left(u,\ \frac{1}{2},\ 0\right)$ | $(0,\ -1,\ 0)$ | $\{1\}\oplus\{3\}$ or $\{2\}\oplus\{4\}$ | $(0,\ 0,\ 1)$ | $\{1\}\oplus\{4\}$ or $\{2\}\oplus\{3\}$ |
| 222 | SM$(u,\ u,\ 0)$ | $\left(\frac{\sqrt{2}}{2},\ -\frac{\sqrt{2}}{2},\ 0\right)$ | $\{1\}\oplus\{3\}$ or $\{2\}\oplus\{4\}$ | $(0,\ 0,\ 1)$ | $\{1\}\oplus\{4\}$ or $\{2\}\oplus\{3\}$ |
| 223 | SM$(u,\ u,\ 0)$ | $\left(\frac{\sqrt{2}}{2},\ -\frac{\sqrt{2}}{2},\ 0\right)$ | $\{1\}\oplus\{3\}$ or $\{2\}\oplus\{4\}$ | $(0,\ 0,\ 1)$ | $\{1\}\oplus\{4\}$ or $\{2\}\oplus\{3\}$ |
| 223 | Z$\left(u,\ \frac{1}{2},\ 0\right)$ | $(0,\ -1,\ 0)$ | $\{1\}\oplus\{3\}$ or $\{2\}\oplus\{4\}$ | $(0,\ 0,\ 1)$ | $\{1\}\oplus\{4\}$ or $\{2\}\oplus\{3\}$ |
| 224 | S$\left(u,\ \frac{1}{2},\ u\right)$ | $(0,\ -1,\ 0)$ | $\{1\}\oplus\{2\}$ or $\{3\}\oplus\{4\}$ | $\left(-\frac{\sqrt{2}}{2},\ 0,\ \frac{\sqrt{2}}{2}\right)$ | $\{1\}\oplus\{4\}$ or $\{2\}\oplus\{3\}$ |
| 224 | SM$(u,\ u,\ 0)$ | $\left(\frac{\sqrt{2}}{2},\ -\frac{\sqrt{2}}{2},\ 0\right)$ | $\{1\}\oplus\{3\}$ or $\{2\}\oplus\{4\}$ | $(0,\ 0,\ 1)$ | $\{1\}\oplus\{4\}$ or $\{2\}\oplus\{3\}$ |
| 225 | SM$(u,\ u,\ 0)$ | $\left(-\frac{\sqrt{2}}{2},\ \frac{\sqrt{2}}{2},\ 0\right)$ | $\{1\}\oplus\{3\}$ or $\{2\}\oplus\{4\}$ | $(0,\ 0,\ -1)$ | $\{1\}\oplus\{4\}$ or $\{2\}\oplus\{3\}$ |
| 225 | V$(u,\ 1,\ 0)$ | $(0,\ -1,\ 0)$ | $\{1\}\oplus\{3\}$ or $\{2\}\oplus\{4\}$ | $(0,\ 0,\ -1)$ | $\{1\}\oplus\{4\}$ or $\{2\}\oplus\{3\}$ |
| 226 | SM$(u,\ u,\ 0)$ | $\left(-\frac{\sqrt{2}}{2},\ \frac{\sqrt{2}}{2},\ 0\right)$ | $\{1\}\oplus\{3\}$ or $\{2\}\oplus\{4\}$ | $(0,\ 0,\ -1)$ | $\{1\}\oplus\{4\}$ or $\{2\}\oplus\{3\}$ |
| 226 | V$(u,\ 1,\ 0)$ | $(0,\ -1,\ 0)$ | $\{1\}\oplus\{3\}$ or $\{2\}\oplus\{4\}$ | $(0,\ 0,\ -1)$ | $\{1\}\oplus\{4\}$ or $\{2\}\oplus\{3\}$ |
| 227 | SM$(u,\ u,\ 0)$ | $\left(-\frac{\sqrt{2}}{2},\ \frac{\sqrt{2}}{2},\ 0\right)$ | $\{1\}\oplus\{3\}$ or $\{2\}\oplus\{4\}$ | $(0,\ 0,\ -1)$ | $\{1\}\oplus\{4\}$ or $\{2\}\oplus\{3\}$ |
| 228 | SM$(u,\ u,\ 0)$ | $\left(-\frac{\sqrt{2}}{2},\ \frac{\sqrt{2}}{2},\ 0\right)$ | $\{1\}\oplus\{3\}$ or $\{2\}\oplus\{4\}$ | $(0,\ 0,\ -1)$ | $\{1\}\oplus\{4\}$ or $\{2\}\oplus\{3\}$ |
| 229 | D$\left(\frac{1}{2},\ \frac{1}{2},\ w\right)$ | $\left(-\frac{\sqrt{2}}{2},\ -\frac{\sqrt{2}}{2},\ 0\right)$ | $\{1\}\oplus\{3\}$ or $\{2\}\oplus\{4\}$ | $\left(-\frac{\sqrt{2}}{2},\ \frac{\sqrt{2}}{2},\ 0\right)$ | $\{1\}\oplus\{4\}$ or $\{2\}\oplus\{3\}$ |
| 229 | G$(u+1,\ 1-u,\ 1)$ | $(0,\ 0,\ -1)$ | $\{1\}\oplus\{3\}$ or $\{2\}\oplus\{4\}$ | $\left(-\frac{\sqrt{2}}{2},\ -\frac{\sqrt{2}}{2},\ 0\right)$ | $\{1\}\oplus\{4\}$ or $\{2\}\oplus\{3\}$ |
| 229 | SM$(u,\ u,\ 0)$ | $\left(-\frac{\sqrt{2}}{2},\ \frac{\sqrt{2}}{2},\ 0\right)$ | $\{1\}\oplus\{3\}$ or $\{2\}\oplus\{4\}$ | $(0,\ 0,\ -1)$ | $\{1\}\oplus\{4\}$ or $\{2\}\oplus\{3\}$ |
| 230 | SM$(u,\ u,\ 0)$ | $\left(-\frac{\sqrt{2}}{2},\ \frac{\sqrt{2}}{2},\ 0\right)$ | $\{1\}\oplus\{3\}$ or $\{2\}\oplus\{4\}$ | $(0,\ 0,\ -1)$ | $\{1\}\oplus\{4\}$ or $\{2\}\oplus\{3\}$ |

Table S14: Loop-chain structure

| SG | HSL | Location of nodal chain | Irreps of BC | Location of nodal loop | Irreps of BC |
|---|---|---|---|---|---|
| 25 | G$(\frac{1}{2},\ 0,\ w)$ | $(0,\ -1,\ 0)$, $(-1,\ 0,\ 0)$ | 1⊕2 or 3⊕4 | $(-1,\ 0,\ 0)$ | 1⊕3 or 2⊕4 |
| | | | | $(0,\ -1,\ 0)$ | 1⊕4 or 2⊕3 |
| 25 | H$(0,\ \frac{1}{2},\ w)$ | $(-1,\ 0,\ 0)$, $(0,\ -1,\ 0)$ | 1⊕2 or 3⊕4 | $(-1,\ 0,\ 0)$ | 1⊕3 or 2⊕4 |
| | | | | $(0,\ -1,\ 0)$ | 1⊕4 or 2⊕3 |
| 25 | LD$(0,\ 0,\ w)$ | $(-1,\ 0,\ 0)$, $(0,\ -1,\ 0)$ | 1⊕2 or 3⊕4 | $(-1,\ 0,\ 0)$ | 1⊕3 or 2⊕4 |
| | | | | $(0,\ -1,\ 0)$ | 1⊕4 or 2⊕3 |
| 25 | Q$(\frac{1}{2},\ \frac{1}{2},\ w)$ | $(-1,\ 0,\ 0)$, $(0,\ -1,\ 0)$ | 1⊕2 or 3⊕4 | $(-1,\ 0,\ 0)$ | 1⊕3 or 2⊕4 |
| | | | | $(0,\ -1,\ 0)$ | 1⊕4 or 2⊕3 |
| 26 | G$(\frac{1}{2},\ 0,\ w)$ | $(0,\ -1,\ 0)$, $(-1,\ 0,\ 0)$ | 1⊕2 or 3⊕4 | $(-1,\ 0,\ 0)$ | 1⊕3 or 2⊕4 |
| | | | | $(0,\ -1,\ 0)$ | 1⊕4 or 2⊕3 |
| 26 | H$(0,\ \frac{1}{2},\ w)$ | $(-1,\ 0,\ 0)$, $(0,\ -1,\ 0)$ | 1⊕2 or 3⊕4 | $(-1,\ 0,\ 0)$ | 1⊕3 or 2⊕4 |
| | | | | $(0,\ -1,\ 0)$ | 1⊕4 or 2⊕3 |
| 26 | LD$(0,\ 0,\ w)$ | $(-1,\ 0,\ 0)$, $(0,\ -1,\ 0)$ | 1⊕2 or 3⊕4 | $(-1,\ 0,\ 0)$ | 1⊕3 or 2⊕4 |
| | | | | $(0,\ -1,\ 0)$ | 1⊕4 or 2⊕3 |
| 26 | Q$(\frac{1}{2},\ \frac{1}{2},\ w)$ | $(-1,\ 0,\ 0)$, $(0,\ -1,\ 0)$ | 1⊕2 or 3⊕4 | $(-1,\ 0,\ 0)$ | 1⊕3 or 2⊕4 |
| | | | | $(0,\ -1,\ 0)$ | 1⊕4 or 2⊕3 |
| 27 | G$(\frac{1}{2},\ 0,\ w)$ | $(0,\ -1,\ 0)$, $(-1,\ 0,\ 0)$ | 1⊕2 or 3⊕4 | $(-1,\ 0,\ 0)$ | 1⊕3 or 2⊕4 |
| | | | | $(0,\ -1,\ 0)$ | 1⊕4 or 2⊕3 |
| 27 | H$(0,\ \frac{1}{2},\ w)$ | $(-1,\ 0,\ 0)$, $(0,\ -1,\ 0)$ | 1⊕2 or 3⊕4 | $(-1,\ 0,\ 0)$ | 1⊕3 or 2⊕4 |
| | | | | $(0,\ -1,\ 0)$ | 1⊕4 or 2⊕3 |
| 27 | LD$(0,\ 0,\ w)$ | $(-1,\ 0,\ 0)$, $(0,\ -1,\ 0)$ | 1⊕2 or 3⊕4 | $(-1,\ 0,\ 0)$ | 1⊕3 or 2⊕4 |
| | | | | $(0,\ -1,\ 0)$ | 1⊕4 or 2⊕3 |
| 27 | Q$(\frac{1}{2},\ \frac{1}{2},\ w)$ | $(-1,\ 0,\ 0)$, $(0,\ -1,\ 0)$ | 1⊕2 or 3⊕4 | $(-1,\ 0,\ 0)$ | 1⊕3 or 2⊕4 |
| | | | | $(0,\ -1,\ 0)$ | 1⊕4 or 2⊕3 |
| 28 | H$(0,\ \frac{1}{2},\ w)$ | $(-1,\ 0,\ 0)$, $(0,\ 1,\ 0)$ | 1⊕2 or 3⊕4 | $(0,\ 1,\ 0)$ | 1⊕3 or 2⊕4 |
| | | | | $(-1,\ 0,\ 0)$ | 1⊕4 or 2⊕3 |
| 28 | LD$(0,\ 0,\ w)$ | $(0,\ 1,\ 0)$, $(-1,\ 0,\ 0)$ | 1⊕2 or 3⊕4 | $(0,\ 1,\ 0)$ | 1⊕3 or 2⊕4 |
| | | | | $(-1,\ 0,\ 0)$ | 1⊕4 or 2⊕3 |
| 29 | H$(0,\ \frac{1}{2},\ w)$ | $(-1,\ 0,\ 0)$, $(0,\ 1,\ 0)$ | 1⊕2 or 3⊕4 | $(0,\ 1,\ 0)$ | 1⊕3 or 2⊕4 |
| | | | | $(-1,\ 0,\ 0)$ | 1⊕4 or 2⊕3 |
| 29 | LD$(0,\ 0,\ w)$ | $(0,\ 1,\ 0)$, $(-1,\ 0,\ 0)$ | 1⊕2 or 3⊕4 | $(0,\ 1,\ 0)$ | 1⊕3 or 2⊕4 |
| | | | | $(-1,\ 0,\ 0)$ | 1⊕4 or 2⊕3 |
| 30 | G$(\frac{1}{2},\ 0,\ w)$ | $(0,\ -1,\ 0)$, $(-1,\ 0,\ 0)$ | 1⊕2 or 3⊕4 | $(-1,\ 0,\ 0)$ | 1⊕3 or 2⊕4 |
| | | | | $(0,\ -1,\ 0)$ | 1⊕4 or 2⊕3 |
| 30 | LD$(0,\ 0,\ w)$ | $(-1,\ 0,\ 0)$, $(0,\ -1,\ 0)$ | 1⊕2 or 3⊕4 | $(-1,\ 0,\ 0)$ | 1⊕3 or 2⊕4 |
| | | | | $(0,\ -1,\ 0)$ | 1⊕4 or 2⊕3 |
| 31 | H$(0,\ \frac{1}{2},\ w)$ | $(-1,\ 0,\ 0)$, $(0,\ 1,\ 0)$ | 1⊕2 or 3⊕4 | $(0,\ 1,\ 0)$ | 1⊕3 or 2⊕4 |
| | | | | $(-1,\ 0,\ 0)$ | 1⊕4 or 2⊕3 |
| 31 | LD$(0,\ 0,\ w)$ | $(0,\ 1,\ 0)$, $(-1,\ 0,\ 0)$ | 1⊕2 or 3⊕4 | $(0,\ 1,\ 0)$ | 1⊕3 or 2⊕4 |
| | | | | $(-1,\ 0,\ 0)$ | 1⊕4 or 2⊕3 |

| SG | HSL | Location of nodal chain | Irreps of BC | Location of nodal loop | Irreps of BC |
|---|---|---|---|---|---|
| 32 | LD(0, 0, $w$) | (−1, 0, 0), (0, −1, 0) | 1⊕2 or 3⊕4 | (−1, 0, 0) | 1⊕3 or 2⊕4 |
| | | | | (0, −1, 0) | 1⊕4 or 2⊕3 |
| 32 | Q$\left(\frac{1}{2},\ \frac{1}{2},\ w\right)$ | (−1, 0, 0), (0, −1, 0) | 1⊕3 or 2⊕4 | (−1, 0, 0) | 1⊕2 or 3⊕4 |
| | | | | (0, −1, 0) | 1⊕4 or 2⊕3 |
| 33 | LD(0, 0, $w$) | (0, 1, 0), (−1, 0, 0) | 1⊕2 or 3⊕4 | (0, 1, 0) | 1⊕3 or 2⊕4 |
| | | | | (−1, 0, 0) | 1⊕4 or 2⊕3 |
| 33 | Q$\left(\frac{1}{2},\ \frac{1}{2},\ w\right)$ | (0, 1, 0), (−1, 0, 0) | 1⊕3 or 2⊕4 | (0, 1, 0) | 1⊕2 or 3⊕4 |
| | | | | (−1, 0, 0) | 1⊕4 or 2⊕3 |
| 34 | LD(0, 0, $w$) | (−1, 0, 0), (0, −1, 0) | 1⊕2 or 3⊕4 | (−1, 0, 0) | 1⊕3 or 2⊕4 |
| | | | | (0, −1, 0) | 1⊕4 or 2⊕3 |
| 34 | Q$\left(\frac{1}{2},\ \frac{1}{2},\ w\right)$ | (−1, 0, 0), (0, −1, 0) | 1⊕3 or 2⊕4 | (−1, 0, 0) | 1⊕2 or 3⊕4 |
| | | | | (0, −1, 0) | 1⊕4 or 2⊕3 |
| 35 | H(1, 0, $w$) | (0, −1, 0), (−1, 0, 0) | 1⊕2 or 3⊕4 | (−1, 0, 0) | 1⊕3 or 2⊕4 |
| | | | | (0, −1, 0) | 1⊕4 or 2⊕3 |
| 35 | LD(0, 0, $w$) | (0, −1, 0), (−1, 0, 0) | 1⊕2 or 3⊕4 | (−1, 0, 0) | 1⊕3 or 2⊕4 |
| | | | | (0, −1, 0) | 1⊕4 or 2⊕3 |
| 36 | H(1, 0, $w$) | (−1, 0, 0), (0, 1, 0) | 1⊕2 or 3⊕4 | (0, 1, 0) | 1⊕3 or 2⊕4 |
| | | | | (−1, 0, 0) | 1⊕4 or 2⊕3 |
| 36 | LD(0, 0, $w$) | (−1, 0, 0), (0, 1, 0) | 1⊕2 or 3⊕4 | (0, 1, 0) | 1⊕3 or 2⊕4 |
| | | | | (−1, 0, 0) | 1⊕4 or 2⊕3 |
| 37 | H(1, 0, $w$) | (0, −1, 0), (−1, 0, 0) | 1⊕2 or 3⊕4 | (−1, 0, 0) | 1⊕3 or 2⊕4 |
| | | | | (0, −1, 0) | 1⊕4 or 2⊕3 |
| 37 | LD(0, 0, $w$) | (0, −1, 0), (−1, 0, 0) | 1⊕2 or 3⊕4 | (−1, 0, 0) | 1⊕3 or 2⊕4 |
| | | | | (0, −1, 0) | 1⊕4 or 2⊕3 |
| 38 | A$\left(\frac{1}{2},\ 0,\ w\right)$ | (0, −1, 0), (1, 0, 0) | 1⊕2 or 3⊕4 | (1, 0, 0) | 1⊕3 or 2⊕4 |
| | | | | (0, −1, 0) | 1⊕4 or 2⊕3 |
| 38 | SM(0, 0, $w$) | (0, −1, 0), (1, 0, 0) | 1⊕2 or 3⊕4 | (1, 0, 0) | 1⊕3 or 2⊕4 |
| | | | | (0, −1, 0) | 1⊕4 or 2⊕3 |
| 39 | A$\left(\frac{1}{2},\ 0,\ w\right)$ | (0, −1, 0), (1, 0, 0) | 1⊕2 or 3⊕4 | (1, 0, 0) | 1⊕3 or 2⊕4 |
| | | | | (0, −1, 0) | 1⊕4 or 2⊕3 |
| 39 | SM(0, 0, $w$) | (0, −1, 0), (1, 0, 0) | 1⊕2 or 3⊕4 | (1, 0, 0) | 1⊕3 or 2⊕4 |
| | | | | (0, −1, 0) | 1⊕4 or 2⊕3 |
| 40 | SM(0, 0, $w$) | (0, −1, 0), (1, 0, 0) | 1⊕2 or 3⊕4 | (1, 0, 0) | 1⊕3 or 2⊕4 |
| | | | | (0, −1, 0) | 1⊕4 or 2⊕3 |
| 41 | SM(0, 0, $w$) | (0, −1, 0), (1, 0, 0) | 1⊕2 or 3⊕4 | (1, 0, 0) | 1⊕3 or 2⊕4 |
| | | | | (0, −1, 0) | 1⊕4 or 2⊕3 |
| 42 | H(0, 1, $w$) | (0, 1, 0), (1, 0, 0) | 1⊕2 or 3⊕4 | (1, 0, 0) | 1⊕3 or 2⊕4 |
| | | | | (0, 1, 0) | 1⊕4 or 2⊕3 |
| 42 | LD(0, 0, $w$) | (0, 1, 0), (1, 0, 0) | 1⊕2 or 3⊕4 | (1, 0, 0) | 1⊕3 or 2⊕4 |
| | | | | (0, 1, 0) | 1⊕4 or 2⊕3 |
| 43 | LD(0, 0, $w$) | (0, 1, 0), (1, 0, 0) | 1⊕2 or 3⊕4 | (1, 0, 0) | 1⊕3 or 2⊕4 |
| | | | | (0, 1, 0) | 1⊕4 or 2⊕3 |

| SG | HSL | Location of nodal chain | Irreps of BC | Location of nodal loop | Irreps of BC |
|---|---|---|---|---|---|
| 44 | LD(0, 0, $w$) | (0, −1, 0), (1, 0, 0) | 1⊕2 or 3⊕4 | (1, 0, 0) | 1⊕3 or 2⊕4 |
| | | | | (0, −1, 0) | 1⊕4 or 2⊕3 |
| 45 | LD(0, 0, $w$) | (0, −1, 0), (1, 0, 0) | 1⊕2 or 3⊕4 | (1, 0, 0) | 1⊕3 or 2⊕4 |
| | | | | (0, −1, 0) | 1⊕4 or 2⊕3 |
| 46 | LD(0, 0, $w$) | (−1, 0, 0), (0, −1, 0) | 1⊕2 or 3⊕4 | (0, −1, 0) | 1⊕3 or 2⊕4 |
| | | | | (−1, 0, 0) | 1⊕4 or 2⊕3 |
| 47 | A$(u, 0, \frac{1}{2})$ | (0, −1, 0), (0, 0, 1) | {1}⊕{2} or {3}⊕{4} | (0, −1, 0) | {1}⊕{3} or {2}⊕{4} |
| | | | | (0, 0, 1) | {1}⊕{4} or {2}⊕{3} |
| 47 | B$(0, v, \frac{1}{2})$ | (−1, 0, 0), (0, 0, 1) | {1}⊕{2} or {3}⊕{4} | (0, 0, 1) | {1}⊕{3} or {2}⊕{4} |
| | | | | (−1, 0, 0) | {1}⊕{4} or {2}⊕{3} |
| 47 | C$(u, \frac{1}{2}, 0)$ | (0, 0, 1), (0, −1, 0) | {1}⊕{2} or {3}⊕{4} | (0, −1, 0) | {1}⊕{3} or {2}⊕{4} |
| | | | | (0, 0, 1) | {1}⊕{4} or {2}⊕{3} |
| 47 | D$(\frac{1}{2}, v, 0)$ | (0, 0, 1), (−1, 0, 0) | {1}⊕{2} or {3}⊕{4} | (0, 0, 1) | {1}⊕{3} or {2}⊕{4} |
| | | | | (−1, 0, 0) | {1}⊕{4} or {2}⊕{3} |
| 47 | DT(0, $v$, 0) | (0, 0, 1), (−1, 0, 0) | {1}⊕{2} or {3}⊕{4} | (0, 0, 1) | {1}⊕{3} or {2}⊕{4} |
| | | | | (−1, 0, 0) | {1}⊕{4} or {2}⊕{3} |
| 47 | E$(u, \frac{1}{2}, \frac{1}{2})$ | (0, 0, 1), (0, −1, 0) | {1}⊕{2} or {3}⊕{4} | (0, −1, 0) | {1}⊕{3} or {2}⊕{4} |
| | | | | (0, 0, 1) | {1}⊕{4} or {2}⊕{3} |
| 47 | G$(\frac{1}{2}, 0, w)$ | (0, −1, 0), (−1, 0, 0) | {1}⊕{2} or {3}⊕{4} | (−1, 0, 0) | {1}⊕{3} or {2}⊕{4} |
| | | | | (0, −1, 0) | {1}⊕{4} or {2}⊕{3} |
| 47 | H$(0, \frac{1}{2}, w)$ | (−1, 0, 0), (0, −1, 0) | {1}⊕{2} or {3}⊕{4} | (−1, 0, 0) | {1}⊕{3} or {2}⊕{4} |
| | | | | (0, −1, 0) | {1}⊕{4} or {2}⊕{3} |
| 47 | LD(0, 0, $w$) | (−1, 0, 0), (0, −1, 0) | {1}⊕{2} or {3}⊕{4} | (−1, 0, 0) | {1}⊕{3} or {2}⊕{4} |
| | | | | (0, −1, 0) | {1}⊕{4} or {2}⊕{3} |
| 47 | P$(\frac{1}{2}, v, \frac{1}{2})$ | (0, 0, 1), (−1, 0, 0) | {1}⊕{2} or {3}⊕{4} | (0, 0, 1) | {1}⊕{3} or {2}⊕{4} |
| | | | | (−1, 0, 0) | {1}⊕{4} or {2}⊕{3} |
| 47 | Q$(\frac{1}{2}, \frac{1}{2}, w)$ | (−1, 0, 0), (0, −1, 0) | {1}⊕{2} or {3}⊕{4} | (−1, 0, 0) | {1}⊕{3} or {2}⊕{4} |
| | | | | (0, −1, 0) | {1}⊕{4} or {2}⊕{3} |
| 47 | SM($u$, 0, 0) | (0, 0, 1), (0, −1, 0) | {1}⊕{2} or {3}⊕{4} | (0, −1, 0) | {1}⊕{3} or {2}⊕{4} |
| | | | | (0, 0, 1) | {1}⊕{4} or {2}⊕{3} |
| 48 | DT(0, $v$, 0) | (0, 0, 1), (−1, 0, 0) | {1}⊕{2} or {3}⊕{4} | (0, 0, 1) | {1}⊕{3} or {2}⊕{4} |
| | | | | (−1, 0, 0) | {1}⊕{4} or {2}⊕{3} |
| 48 | E$(u, \frac{1}{2}, \frac{1}{2})$ | (0, 0, 1), (0, −1, 0) | {1}⊕{2} or {3}⊕{4} | (0, −1, 0) | {1}⊕{3} or {2}⊕{4} |
| | | | | (0, 0, 1) | {1}⊕{4} or {2}⊕{3} |
| 48 | LD(0, 0, $w$) | (−1, 0, 0), (0, −1, 0) | {1}⊕{2} or {3}⊕{4} | (−1, 0, 0) | {1}⊕{3} or {2}⊕{4} |
| | | | | (0, −1, 0) | {1}⊕{4} or {2}⊕{3} |
| 48 | P$(\frac{1}{2}, v, \frac{1}{2})$ | (0, 0, 1), (−1, 0, 0) | {1}⊕{2} or {3}⊕{4} | (−1, 0, 0) | {1}⊕{3} or {2}⊕{4} |
| | | | | (0, 0, 1) | {1}⊕{4} or {2}⊕{3} |
| 48 | Q$(\frac{1}{2}, \frac{1}{2}, w)$ | (−1, 0, 0), (0, −1, 0) | {1}⊕{2} or {3}⊕{4} | (0, −1, 0) | {1}⊕{3} or {2}⊕{4} |
| | | | | (−1, 0, 0) | {1}⊕{4} or {2}⊕{3} |
| 48 | SM($u$, 0, 0) | (0, 0, 1), (0, −1, 0) | {1}⊕{2} or {3}⊕{4} | (0, 0, 1) | {1}⊕{3} or {2}⊕{4} |
| | | | | (0, −1, 0) | {1}⊕{4} or {2}⊕{3} |

<table>
<tr><th>SG</th><th>HSL</th><th>Location of nodal chain</th><th>Irreps of BC</th><th>Location of nodal loop</th><th>Irreps of BC</th></tr>
<tr><td rowspan="2">49</td><td rowspan="2">C$(u,\ \frac{1}{2},\ 0)$</td><td rowspan="2">(0, 0, 1), (0, −1, 0)</td><td rowspan="2">{1}⊕{2} or {3}⊕{4}</td><td>(0, −1, 0)</td><td>{1}⊕{3} or {2}⊕{4}</td></tr>
<tr><td>(0, 0, 1)</td><td>{1}⊕{4} or {2}⊕{3}</td></tr>
<tr><td rowspan="2">49</td><td rowspan="2">D$(\frac{1}{2},\ v,\ 0)$</td><td rowspan="2">(0, 0, 1), (−1, 0, 0)</td><td rowspan="2">{1}⊕{2} or {3}⊕{4}</td><td>(0, 0, 1)</td><td>{1}⊕{3} or {2}⊕{4}</td></tr>
<tr><td>(−1, 0, 0)</td><td>{1}⊕{4} or {2}⊕{3}</td></tr>
<tr><td rowspan="2">49</td><td rowspan="2">DT$(0,\ v,\ 0)$</td><td rowspan="2">(0, 0, 1), (−1, 0, 0)</td><td rowspan="2">{1}⊕{2} or {3}⊕{4}</td><td>(0, 0, 1)</td><td>{1}⊕{3} or {2}⊕{4}</td></tr>
<tr><td>(−1, 0, 0)</td><td>{1}⊕{4} or {2}⊕{3}</td></tr>
<tr><td rowspan="2">49</td><td rowspan="2">G$(\frac{1}{2},\ 0,\ w)$</td><td rowspan="2">(0, −1, 0), (−1, 0, 0)</td><td rowspan="2">{1}⊕{2} or {3}⊕{4}</td><td>(−1, 0, 0)</td><td>{1}⊕{3} or {2}⊕{4}</td></tr>
<tr><td>(0, −1, 0)</td><td>{1}⊕{4} or {2}⊕{3}</td></tr>
<tr><td rowspan="2">49</td><td rowspan="2">H$(0,\ \frac{1}{2},\ w)$</td><td rowspan="2">(−1, 0, 0), (0, −1, 0)</td><td rowspan="2">{1}⊕{2} or {3}⊕{4}</td><td>(−1, 0, 0)</td><td>{1}⊕{3} or {2}⊕{4}</td></tr>
<tr><td>(0, −1, 0)</td><td>{1}⊕{4} or {2}⊕{3}</td></tr>
<tr><td rowspan="2">49</td><td rowspan="2">LD$(0,\ 0,\ w)$</td><td rowspan="2">(−1, 0, 0), (0, −1, 0)</td><td rowspan="2">{1}⊕{2} or {3}⊕{4}</td><td>(−1, 0, 0)</td><td>{1}⊕{3} or {2}⊕{4}</td></tr>
<tr><td>(0, −1, 0)</td><td>{1}⊕{4} or {2}⊕{3}</td></tr>
<tr><td rowspan="2">49</td><td rowspan="2">Q$(\frac{1}{2},\ \frac{1}{2},\ w)$</td><td rowspan="2">(−1, 0, 0), (0, −1, 0)</td><td rowspan="2">{1}⊕{2} or {3}⊕{4}</td><td>(−1, 0, 0)</td><td>{1}⊕{3} or {2}⊕{4}</td></tr>
<tr><td>(0, −1, 0)</td><td>{1}⊕{4} or {2}⊕{3}</td></tr>
<tr><td rowspan="2">49</td><td rowspan="2">SM$(u,\ 0,\ 0)$</td><td rowspan="2">(0, 0, 1), (0, −1, 0)</td><td rowspan="2">{1}⊕{2} or {3}⊕{4}</td><td>(0, −1, 0)</td><td>{1}⊕{3} or {2}⊕{4}</td></tr>
<tr><td>(0, 0, 1)</td><td>{1}⊕{4} or {2}⊕{3}</td></tr>
<tr><td rowspan="2">50</td><td rowspan="2">A$(u,\ 0,\ \frac{1}{2})$</td><td rowspan="2">(0, −1, 0), (0, 0, 1)</td><td rowspan="2">{1}⊕{2} or {3}⊕{4}</td><td>(0, −1, 0)</td><td>{1}⊕{3} or {2}⊕{4}</td></tr>
<tr><td>(0, 0, 1)</td><td>{1}⊕{4} or {2}⊕{3}</td></tr>
<tr><td rowspan="2">50</td><td rowspan="2">B$(0,\ v,\ \frac{1}{2})$</td><td rowspan="2">(−1, 0, 0), (0, 0, 1)</td><td rowspan="2">{1}⊕{2} or {3}⊕{4}</td><td>(0, 0, 1)</td><td>{1}⊕{3} or {2}⊕{4}</td></tr>
<tr><td>(−1, 0, 0)</td><td>{1}⊕{4} or {2}⊕{3}</td></tr>
<tr><td rowspan="2">50</td><td rowspan="2">DT$(0,\ v,\ 0)$</td><td rowspan="2">(0, 0, 1), (−1, 0, 0)</td><td rowspan="2">{1}⊕{2} or {3}⊕{4}</td><td>(0, 0, 1)</td><td>{1}⊕{3} or {2}⊕{4}</td></tr>
<tr><td>(−1, 0, 0)</td><td>{1}⊕{4} or {2}⊕{3}</td></tr>
<tr><td rowspan="2">50</td><td rowspan="2">LD$(0,\ 0,\ w)$</td><td rowspan="2">(−1, 0, 0), (0, −1, 0)</td><td rowspan="2">{1}⊕{2} or {3}⊕{4}</td><td>(−1, 0, 0)</td><td>{1}⊕{3} or {2}⊕{4}</td></tr>
<tr><td>(0, −1, 0)</td><td>{1}⊕{4} or {2}⊕{3}</td></tr>
<tr><td rowspan="2">50</td><td rowspan="2">Q$(\frac{1}{2},\ \frac{1}{2},\ w)$</td><td rowspan="2">(−1, 0, 0), (0, −1, 0)</td><td rowspan="2">{1}⊕{2} or {3}⊕{4}</td><td>(−1, 0, 0)</td><td>{1}⊕{3} or {2}⊕{4}</td></tr>
<tr><td>(0, −1, 0)</td><td>{1}⊕{4} or {2}⊕{3}</td></tr>
<tr><td rowspan="2">50</td><td rowspan="2">SM$(u,\ 0,\ 0)$</td><td rowspan="2">(0, 0, 1), (0, −1, 0)</td><td rowspan="2">{1}⊕{2} or {3}⊕{4}</td><td>(0, −1, 0)</td><td>{1}⊕{3} or {2}⊕{4}</td></tr>
<tr><td>(0, 0, 1)</td><td>{1}⊕{4} or {2}⊕{3}</td></tr>
<tr><td rowspan="2">51</td><td rowspan="2">A$(u,\ 0,\ \frac{1}{2})$</td><td rowspan="2">(0, −1, 0), (0, 0, −1)</td><td rowspan="2">{1}⊕{2} or {3}⊕{4}</td><td>(0, 0, −1)</td><td>{1}⊕{3} or {2}⊕{4}</td></tr>
<tr><td>(0, −1, 0)</td><td>{1}⊕{4} or {2}⊕{3}</td></tr>
<tr><td rowspan="2">51</td><td rowspan="2">B$(0,\ v,\ \frac{1}{2})$</td><td rowspan="2">(−1, 0, 0), (0, 0, −1)</td><td rowspan="2">{1}⊕{2} or {3}⊕{4}</td><td>(−1, 0, 0)</td><td>{1}⊕{3} or {2}⊕{4}</td></tr>
<tr><td>(0, 0, −1)</td><td>{1}⊕{4} or {2}⊕{3}</td></tr>
<tr><td rowspan="2">51</td><td rowspan="2">C$(u,\ \frac{1}{2},\ 0)$</td><td rowspan="2">(0, 0, −1), (0, −1, 0)</td><td rowspan="2">{1}⊕{2} or {3}⊕{4}</td><td>(0, 0, −1)</td><td>{1}⊕{3} or {2}⊕{4}</td></tr>
<tr><td>(0, −1, 0)</td><td>{1}⊕{4} or {2}⊕{3}</td></tr>
<tr><td rowspan="2">51</td><td rowspan="2">DT$(0,\ v,\ 0)$</td><td rowspan="2">(−1, 0, 0), (0, 0, −1)</td><td rowspan="2">{1}⊕{2} or {3}⊕{4}</td><td>(−1, 0, 0)</td><td>{1}⊕{3} or {2}⊕{4}</td></tr>
<tr><td>(0, 0, −1)</td><td>{1}⊕{4} or {2}⊕{3}</td></tr>
<tr><td rowspan="2">51</td><td rowspan="2">E$(u,\ \frac{1}{2},\ \frac{1}{2})$</td><td rowspan="2">(0, 0, −1), (0, −1, 0)</td><td rowspan="2">{1}⊕{2} or {3}⊕{4}</td><td>(0, 0, −1)</td><td>{1}⊕{3} or {2}⊕{4}</td></tr>
<tr><td>(0, −1, 0)</td><td>{1}⊕{4} or {2}⊕{3}</td></tr>
<tr><td rowspan="2">51</td><td rowspan="2">H$(0,\ \frac{1}{2},\ w)$</td><td rowspan="2">(−1, 0, 0), (0, −1, 0)</td><td rowspan="2">{1}⊕{2} or {3}⊕{4}</td><td>(0, −1, 0)</td><td>{1}⊕{3} or {2}⊕{4}</td></tr>
<tr><td>(−1, 0, 0)</td><td>{1}⊕{4} or {2}⊕{3}</td></tr>
<tr><td rowspan="2">51</td><td rowspan="2">LD$(0,\ 0,\ w)$</td><td rowspan="2">(−1, 0, 0), (0, −1, 0)</td><td rowspan="2">{1}⊕{2} or {3}⊕{4}</td><td>(0, −1, 0)</td><td>{1}⊕{3} or {2}⊕{4}</td></tr>
<tr><td>(−1, 0, 0)</td><td>{1}⊕{4} or {2}⊕{3}</td></tr>
</table>

| SG | HSL | Location of nodal chain | Irreps of BC | Location of nodal loop | Irreps of BC |
|---|---|---|---|---|---|
| 51 | SM$(u,\ 0,\ 0)$ | $(0,\ 0,\ -1)$, $(0,\ -1,\ 0)$ | {1}⊕{2} or {3}⊕{4} | $(0,\ 0,\ -1)$ | {1}⊕{3} or {2}⊕{4} |
| | | | | $(0,\ -1,\ 0)$ | {1}⊕{4} or {2}⊕{3} |
| 52 | DT$(0,\ v,\ 0)$ | $(-1,\ 0,\ 0)$, $(0,\ 0,\ 1)$ | {1}⊕{2} or {3}⊕{4} | $(-1,\ 0,\ 0)$ | {1}⊕{3} or {2}⊕{4} |
| | | | | $(0,\ 0,\ 1)$ | {1}⊕{4} or {2}⊕{3} |
| 52 | LD$(0,\ 0,\ w)$ | $(0,\ 1,\ 0)$, $(-1,\ 0,\ 0)$ | {1}⊕{2} or {3}⊕{4} | $(0,\ 1,\ 0)$ | {1}⊕{3} or {2}⊕{4} |
| | | | | $(-1,\ 0,\ 0)$ | {1}⊕{4} or {2}⊕{3} |
| 52 | P$\left(\frac{1}{2},\ v,\ \frac{1}{2}\right)$ | $(-1,\ 0,\ 0)$, $(0,\ 0,\ 1)$ | {1}⊕{2} or {3}⊕{4} | $(-1,\ 0,\ 0)$ | {1}⊕{3} or {2}⊕{4} |
| | | | | $(0,\ 0,\ 1)$ | {1}⊕{4} or {2}⊕{3} |
| 52 | SM$(u,\ 0,\ 0)$ | $(0,\ 1,\ 0)$, $(0,\ 0,\ 1)$ | {1}⊕{2} or {3}⊕{4} | $(0,\ 0,\ 1)$ | {1}⊕{3} or {2}⊕{4} |
| | | | | $(0,\ 1,\ 0)$ | {1}⊕{4} or {2}⊕{3} |
| 53 | C$\left(u,\ \frac{1}{2},\ 0\right)$ | $(0,\ 0,\ 1)$, $(0,\ 1,\ 0)$ | {1}⊕{2} or {3}⊕{4} | $(0,\ 0,\ 1)$ | {1}⊕{3} or {2}⊕{4} |
| | | | | $(0,\ 1,\ 0)$ | {1}⊕{4} or {2}⊕{3} |
| 53 | DT$(0,\ v,\ 0)$ | $(0,\ 0,\ 1)$, $(-1,\ 0,\ 0)$ | {1}⊕{2} or {3}⊕{4} | $(-1,\ 0,\ 0)$ | {1}⊕{3} or {2}⊕{4} |
| | | | | $(0,\ 0,\ 1)$ | {1}⊕{4} or {2}⊕{3} |
| 53 | H$\left(0,\ \frac{1}{2},\ w\right)$ | $(-1,\ 0,\ 0)$, $(0,\ 1,\ 0)$ | {1}⊕{2} or {3}⊕{4} | $(0,\ 1,\ 0)$ | {1}⊕{3} or {2}⊕{4} |
| | | | | $(-1,\ 0,\ 0)$ | {1}⊕{4} or {2}⊕{3} |
| 53 | LD$(0,\ 0,\ w)$ | $(0,\ 1,\ 0)$, $(-1,\ 0,\ 0)$ | {1}⊕{2} or {3}⊕{4} | $(0,\ 1,\ 0)$ | {1}⊕{3} or {2}⊕{4} |
| | | | | $(-1,\ 0,\ 0)$ | {1}⊕{4} or {2}⊕{3} |
| 53 | SM$(u,\ 0,\ 0)$ | $(0,\ 0,\ 1)$, $(0,\ 1,\ 0)$ | {1}⊕{2} or {3}⊕{4} | $(0,\ 0,\ 1)$ | {1}⊕{3} or {2}⊕{4} |
| | | | | $(0,\ 1,\ 0)$ | {1}⊕{4} or {2}⊕{3} |
| 54 | C$\left(u,\ \frac{1}{2},\ 0\right)$ | $(0,\ 0,\ -1)$, $(0,\ -1,\ 0)$ | {1}⊕{2} or {3}⊕{4} | $(0,\ 0,\ -1)$ | {1}⊕{3} or {2}⊕{4} |
| | | | | $(0,\ -1,\ 0)$ | {1}⊕{4} or {2}⊕{3} |
| 54 | DT$(0,\ v,\ 0)$ | $(-1,\ 0,\ 0)$, $(0,\ 0,\ -1)$ | {1}⊕{2} or {3}⊕{4} | $(-1,\ 0,\ 0)$ | {1}⊕{3} or {2}⊕{4} |
| | | | | $(0,\ 0,\ -1)$ | {1}⊕{4} or {2}⊕{3} |
| 54 | H$\left(0,\ \frac{1}{2},\ w\right)$ | $(-1,\ 0,\ 0)$, $(0,\ -1,\ 0)$ | {1}⊕{2} or {3}⊕{4} | $(0,\ -1,\ 0)$ | {1}⊕{3} or {2}⊕{4} |
| | | | | $(-1,\ 0,\ 0)$ | {1}⊕{4} or {2}⊕{3} |
| 54 | LD$(0,\ 0,\ w)$ | $(-1,\ 0,\ 0)$, $(0,\ -1,\ 0)$ | {1}⊕{2} or {3}⊕{4} | $(0,\ -1,\ 0)$ | {1}⊕{3} or {2}⊕{4} |
| | | | | $(-1,\ 0,\ 0)$ | {1}⊕{4} or {2}⊕{3} |
| 54 | SM$(u,\ 0,\ 0)$ | $(0,\ 0,\ -1)$, $(0,\ -1,\ 0)$ | {1}⊕{2} or {3}⊕{4} | $(0,\ 0,\ -1)$ | {1}⊕{3} or {2}⊕{4} |
| | | | | $(0,\ -1,\ 0)$ | {1}⊕{4} or {2}⊕{3} |
| 55 | A$\left(u,\ 0,\ \frac{1}{2}\right)$ | $(0,\ -1,\ 0)$, $(0,\ 0,\ 1)$ | {1}⊕{2} or {3}⊕{4} | $(0,\ -1,\ 0)$ | {1}⊕{3} or {2}⊕{4} |
| | | | | $(0,\ 0,\ 1)$ | {1}⊕{4} or {2}⊕{3} |
| 55 | B$\left(0,\ v,\ \frac{1}{2}\right)$ | $(-1,\ 0,\ 0)$, $(0,\ 0,\ 1)$ | {1}⊕{2} or {3}⊕{4} | $(0,\ 0,\ 1)$ | {1}⊕{3} or {2}⊕{4} |
| | | | | $(-1,\ 0,\ 0)$ | {1}⊕{4} or {2}⊕{3} |
| 55 | DT$(0,\ v,\ 0)$ | $(0,\ 0,\ 1)$, $(-1,\ 0,\ 0)$ | {1}⊕{2} or {3}⊕{4} | $(0,\ 0,\ 1)$ | {1}⊕{3} or {2}⊕{4} |
| | | | | $(-1,\ 0,\ 0)$ | {1}⊕{4} or {2}⊕{3} |
| 55 | LD$(0,\ 0,\ w)$ | $(-1,\ 0,\ 0)$, $(0,\ -1,\ 0)$ | {1}⊕{2} or {3}⊕{4} | $(-1,\ 0,\ 0)$ | {1}⊕{3} or {2}⊕{4} |
| | | | | $(0,\ -1,\ 0)$ | {1}⊕{4} or {2}⊕{3} |
| 55 | SM$(u,\ 0,\ 0)$ | $(0,\ 0,\ 1)$, $(0,\ -1,\ 0)$ | {1}⊕{2} or {3}⊕{4} | $(0,\ -1,\ 0)$ | {1}⊕{3} or {2}⊕{4} |
| | | | | $(0,\ 0,\ 1)$ | {1}⊕{4} or {2}⊕{3} |
| 56 | DT$(0,\ v,\ 0)$ | $(0,\ 0,\ 1)$, $(-1,\ 0,\ 0)$ | {1}⊕{2} or {3}⊕{4} | $(0,\ 0,\ 1)$ | {1}⊕{3} or {2}⊕{4} |
| | | | | $(-1,\ 0,\ 0)$ | {1}⊕{4} or {2}⊕{3} |

| SG | HSL | Location of nodal chain | Irreps of BC | Location of nodal loop | Irreps of BC |
|---|---|---|---|---|---|
| 56 | LD(0, 0, $w$) | (−1, 0, 0), (0, −1, 0) | {1}⊕{2} or {3}⊕{4} | (−1, 0, 0) | {1}⊕{3} or {2}⊕{4} |
| | | | | (0, −1, 0) | {1}⊕{4} or {2}⊕{3} |
| 56 | SM($u$, 0, 0) | (0, 0, 1), (0, −1, 0) | {1}⊕{2} or {3}⊕{4} | (0, −1, 0) | {1}⊕{3} or {2}⊕{4} |
| | | | | (0, 0, 1) | {1}⊕{4} or {2}⊕{3} |
| 57 | D$\left(\frac{1}{2},\ v,\ 0\right)$ | (0, 0, −1), (1, 0, 0) | {1}⊕{2} or {3}⊕{4} | (0, 0, −1) | {1}⊕{3} or {2}⊕{4} |
| | | | | (1, 0, 0) | {1}⊕{4} or {2}⊕{3} |
| 57 | DT(0, $v$, 0) | (1, 0, 0), (0, 0, −1) | {1}⊕{2} or {3}⊕{4} | (0, 0, −1) | {1}⊕{3} or {2}⊕{4} |
| | | | | (1, 0, 0) | {1}⊕{4} or {2}⊕{3} |
| 57 | G$\left(\frac{1}{2},\ 0,\ w\right)$ | (0, −1, 0), (1, 0, 0) | {1}⊕{2} or {3}⊕{4} | (1, 0, 0) | {1}⊕{3} or {2}⊕{4} |
| | | | | (0, −1, 0) | {1}⊕{4} or {2}⊕{3} |
| 57 | LD(0, 0, $w$) | (1, 0, 0), (0, −1, 0) | {1}⊕{2} or {3}⊕{4} | (1, 0, 0) | {1}⊕{3} or {2}⊕{4} |
| | | | | (0, −1, 0) | {1}⊕{4} or {2}⊕{3} |
| 57 | SM($u$, 0, 0) | (0, −1, 0), (0, 0, −1) | {1}⊕{2} or {3}⊕{4} | (0, −1, 0) | {1}⊕{3} or {2}⊕{4} |
| | | | | (0, 0, −1) | {1}⊕{4} or {2}⊕{3} |
| 58 | DT(0, $v$, 0) | (0, 0, 1), (−1, 0, 0) | {1}⊕{2} or {3}⊕{4} | (0, 0, 1) | {1}⊕{3} or {2}⊕{4} |
| | | | | (−1, 0, 0) | {1}⊕{4} or {2}⊕{3} |
| 58 | LD(0, 0, $w$) | (−1, 0, 0), (0, −1, 0) | {1}⊕{2} or {3}⊕{4} | (−1, 0, 0) | {1}⊕{3} or {2}⊕{4} |
| | | | | (0, −1, 0) | {1}⊕{4} or {2}⊕{3} |
| 58 | SM($u$, 0, 0) | (0, 0, 1), (0, −1, 0) | {1}⊕{2} or {3}⊕{4} | (0, −1, 0) | {1}⊕{3} or {2}⊕{4} |
| | | | | (0, 0, 1) | {1}⊕{4} or {2}⊕{3} |
| 59 | A$\left(u,\ 0,\ \frac{1}{2}\right)$ | (0, −1, 0), (0, 0, 1) | {1}⊕{2} or {3}⊕{4} | (0, −1, 0) | {1}⊕{3} or {2}⊕{4} |
| | | | | (0, 0, 1) | {1}⊕{4} or {2}⊕{3} |
| 59 | B$\left(0,\ v,\ \frac{1}{2}\right)$ | (−1, 0, 0), (0, 0, 1) | {1}⊕{2} or {3}⊕{4} | (0, 0, 1) | {1}⊕{3} or {2}⊕{4} |
| | | | | (−1, 0, 0) | {1}⊕{4} or {2}⊕{3} |
| 59 | DT(0, $v$, 0) | (0, 0, 1), (−1, 0, 0) | {1}⊕{2} or {3}⊕{4} | (0, 0, 1) | {1}⊕{3} or {2}⊕{4} |
| | | | | (−1, 0, 0) | {1}⊕{4} or {2}⊕{3} |
| 59 | LD(0, 0, $w$) | (−1, 0, 0), (0, −1, 0) | {1}⊕{2} or {3}⊕{4} | (−1, 0, 0) | {1}⊕{3} or {2}⊕{4} |
| | | | | (0, −1, 0) | {1}⊕{4} or {2}⊕{3} |
| 59 | SM($u$, 0, 0) | (0, 0, 1), (0, −1, 0) | {1}⊕{2} or {3}⊕{4} | (0, −1, 0) | {1}⊕{3} or {2}⊕{4} |
| | | | | (0, 0, 1) | {1}⊕{4} or {2}⊕{3} |
| 60 | DT(0, $v$, 0) | (−1, 0, 0), (0, 0, 1) | {1}⊕{2} or {3}⊕{4} | (−1, 0, 0) | {1}⊕{3} or {2}⊕{4} |
| | | | | (0, 0, 1) | {1}⊕{4} or {2}⊕{3} |
| 60 | LD(0, 0, $w$) | (0, 1, 0), (−1, 0, 0) | {1}⊕{2} or {3}⊕{4} | (0, 1, 0) | {1}⊕{3} or {2}⊕{4} |
| | | | | (−1, 0, 0) | {1}⊕{4} or {2}⊕{3} |
| 60 | SM($u$, 0, 0) | (0, 1, 0), (0, 0, 1) | {1}⊕{2} or {3}⊕{4} | (0, 0, 1) | {1}⊕{3} or {2}⊕{4} |
| | | | | (0, 1, 0) | {1}⊕{4} or {2}⊕{3} |
| 61 | DT(0, $v$, 0) | (−1, 0, 0), (0, 0, 1) | {1}⊕{2} or {3}⊕{4} | (−1, 0, 0) | {1}⊕{3} or {2}⊕{4} |
| | | | | (0, 0, 1) | {1}⊕{4} or {2}⊕{3} |
| 61 | LD(0, 0, $w$) | (0, 1, 0), (−1, 0, 0) | {1}⊕{2} or {3}⊕{4} | (0, 1, 0) | {1}⊕{3} or {2}⊕{4} |
| | | | | (−1, 0, 0) | {1}⊕{4} or {2}⊕{3} |
| 61 | SM($u$, 0, 0) | (0, 1, 0), (0, 0, 1) | {1}⊕{2} or {3}⊕{4} | (0, 0, 1) | {1}⊕{3} or {2}⊕{4} |
| | | | | (0, 1, 0) | {1}⊕{4} or {2}⊕{3} |

| SG | HSL | Location of nodal chain | Irreps of BC | Location of nodal loop | Irreps of BC |
|---|---|---|---|---|---|
| 62 | DT(0, $v$, 0) | (0, 0, 1), (−1, 0, 0) | {1}⊕{2} or {3}⊕{4} | (0, 0, 1) | {1}⊕{3} or {2}⊕{4} |
| | | | | (−1, 0, 0) | {1}⊕{4} or {2}⊕{3} |
| 62 | LD(0, 0, $w$) | (−1, 0, 0), (0, −1, 0) | {1}⊕{2} or {3}⊕{4} | (−1, 0, 0) | {1}⊕{3} or {2}⊕{4} |
| | | | | (0, −1, 0) | {1}⊕{4} or {2}⊕{3} |
| 62 | SM($u$, 0, 0) | (0, 0, 1), (0, −1, 0) | {1}⊕{2} or {3}⊕{4} | (0, −1, 0) | {1}⊕{3} or {2}⊕{4} |
| | | | | (0, 0, 1) | {1}⊕{4} or {2}⊕{3} |
| 63 | DT(0, $v$, 0) | (−1, 0, 0), (0, 0, 1) | {1}⊕{2} or {3}⊕{4} | (0, 0, 1) | {1}⊕{3} or {2}⊕{4} |
| | | | | (−1, 0, 0) | {1}⊕{4} or {2}⊕{3} |
| 63 | H(1, 0, $w$) | (0, −1, 0), (−1, 0, 0) | {1}⊕{2} or {3}⊕{4} | (−1, 0, 0) | {1}⊕{3} or {2}⊕{4} |
| | | | | (0, −1, 0) | {1}⊕{4} or {2}⊕{3} |
| 63 | LD(0, 0, $w$) | (0, −1, 0), (−1, 0, 0) | {1}⊕{2} or {3}⊕{4} | (−1, 0, 0) | {1}⊕{3} or {2}⊕{4} |
| | | | | (0, −1, 0) | {1}⊕{4} or {2}⊕{3} |
| 63 | SM($u$, 0, 0) | (0, −1, 0), (0, 0, 1) | {1}⊕{2} or {3}⊕{4} | (0, −1, 0) | {1}⊕{3} or {2}⊕{4} |
| | | | | (0, 0, 1) | {1}⊕{4} or {2}⊕{3} |
| 64 | DT(0, $v$, 0) | (−1, 0, 0), (0, 0, 1) | {1}⊕{2} or {3}⊕{4} | (0, 0, 1) | {1}⊕{3} or {2}⊕{4} |
| | | | | (−1, 0, 0) | {1}⊕{4} or {2}⊕{3} |
| 64 | H(1, 0, $w$) | (0, −1, 0), (−1, 0, 0) | {1}⊕{2} or {3}⊕{4} | (−1, 0, 0) | {1}⊕{3} or {2}⊕{4} |
| | | | | (0, −1, 0) | {1}⊕{4} or {2}⊕{3} |
| 64 | LD(0, 0, $w$) | (0, −1, 0), (−1, 0, 0) | {1}⊕{2} or {3}⊕{4} | (−1, 0, 0) | {1}⊕{3} or {2}⊕{4} |
| | | | | (0, −1, 0) | {1}⊕{4} or {2}⊕{3} |
| 64 | SM($u$, 0, 0) | (0, −1, 0), (0, 0, 1) | {1}⊕{2} or {3}⊕{4} | (0, −1, 0) | {1}⊕{3} or {2}⊕{4} |
| | | | | (0, 0, 1) | {1}⊕{4} or {2}⊕{3} |
| 65 | A($u$, 0, $\frac{1}{2}$) | (0, −1, 0), (0, 0, 1) | {1}⊕{2} or {3}⊕{4} | (0, −1, 0) | {1}⊕{3} or {2}⊕{4} |
| | | | | (0, 0, 1) | {1}⊕{4} or {2}⊕{3} |
| 65 | B(0, $v$, $\frac{1}{2}$) | (−1, 0, 0), (0, 0, 1) | {1}⊕{2} or {3}⊕{4} | (0, 0, 1) | {1}⊕{3} or {2}⊕{4} |
| | | | | (−1, 0, 0) | {1}⊕{4} or {2}⊕{3} |
| 65 | DT(0, $v$, 0) | (−1, 0, 0), (0, 0, 1) | {1}⊕{2} or {3}⊕{4} | (0, 0, 1) | {1}⊕{3} or {2}⊕{4} |
| | | | | (−1, 0, 0) | {1}⊕{4} or {2}⊕{3} |
| 65 | H(1, 0, $w$) | (0, −1, 0), (−1, 0, 0) | {1}⊕{2} or {3}⊕{4} | (−1, 0, 0) | {1}⊕{3} or {2}⊕{4} |
| | | | | (0, −1, 0) | {1}⊕{4} or {2}⊕{3} |
| 65 | LD(0, 0, $w$) | (0, −1, 0), (−1, 0, 0) | {1}⊕{2} or {3}⊕{4} | (−1, 0, 0) | {1}⊕{3} or {2}⊕{4} |
| | | | | (0, −1, 0) | {1}⊕{4} or {2}⊕{3} |
| 65 | SM($u$, 0, 0) | (0, −1, 0), (0, 0, 1) | {1}⊕{2} or {3}⊕{4} | (0, −1, 0) | {1}⊕{3} or {2}⊕{4} |
| | | | | (0, 0, 1) | {1}⊕{4} or {2}⊕{3} |
| 66 | DT(0, $v$, 0) | (−1, 0, 0), (0, 0, 1) | {1}⊕{2} or {3}⊕{4} | (0, 0, 1) | {1}⊕{3} or {2}⊕{4} |
| | | | | (−1, 0, 0) | {1}⊕{4} or {2}⊕{3} |
| 66 | H(1, 0, $w$) | (0, −1, 0), (−1, 0, 0) | {1}⊕{2} or {3}⊕{4} | (−1, 0, 0) | {1}⊕{3} or {2}⊕{4} |
| | | | | (0, −1, 0) | {1}⊕{4} or {2}⊕{3} |
| 66 | LD(0, 0, $w$) | (0, −1, 0), (−1, 0, 0) | {1}⊕{2} or {3}⊕{4} | (−1, 0, 0) | {1}⊕{3} or {2}⊕{4} |
| | | | | (0, −1, 0) | {1}⊕{4} or {2}⊕{3} |
| 66 | SM($u$, 0, 0) | (0, −1, 0), (0, 0, 1) | {1}⊕{2} or {3}⊕{4} | (0, −1, 0) | {1}⊕{3} or {2}⊕{4} |
| | | | | (0, 0, 1) | {1}⊕{4} or {2}⊕{3} |

| SG | HSL | Location of nodal chain | Irreps of BC | Location of nodal loop | Irreps of BC |
|---|---|---|---|---|---|
| 67 | $A(u,\ 0,\ \frac{1}{2})$ | $(0,\ -1,\ 0)$, $(0,\ 0,\ 1)$ | $\{1\}\oplus\{2\}$ or $\{3\}\oplus\{4\}$ | $(0,\ -1,\ 0)$ | $\{1\}\oplus\{3\}$ or $\{2\}\oplus\{4\}$ |
| | | | | $(0,\ 0,\ 1)$ | $\{1\}\oplus\{4\}$ or $\{2\}\oplus\{3\}$ |
| 67 | $B(0,\ v,\ \frac{1}{2})$ | $(-1,\ 0,\ 0)$, $(0,\ 0,\ 1)$ | $\{1\}\oplus\{2\}$ or $\{3\}\oplus\{4\}$ | $(0,\ 0,\ 1)$ | $\{1\}\oplus\{3\}$ or $\{2\}\oplus\{4\}$ |
| | | | | $(-1,\ 0,\ 0)$ | $\{1\}\oplus\{4\}$ or $\{2\}\oplus\{3\}$ |
| 67 | $DT(0,\ v,\ 0)$ | $(-1,\ 0,\ 0)$, $(0,\ 0,\ 1)$ | $\{1\}\oplus\{2\}$ or $\{3\}\oplus\{4\}$ | $(0,\ 0,\ 1)$ | $\{1\}\oplus\{3\}$ or $\{2\}\oplus\{4\}$ |
| | | | | $(-1,\ 0,\ 0)$ | $\{1\}\oplus\{4\}$ or $\{2\}\oplus\{3\}$ |
| 67 | $H(1,\ 0,\ w)$ | $(0,\ -1,\ 0)$, $(-1,\ 0,\ 0)$ | $\{1\}\oplus\{2\}$ or $\{3\}\oplus\{4\}$ | $(-1,\ 0,\ 0)$ | $\{1\}\oplus\{3\}$ or $\{2\}\oplus\{4\}$ |
| | | | | $(0,\ -1,\ 0)$ | $\{1\}\oplus\{4\}$ or $\{2\}\oplus\{3\}$ |
| 67 | $LD(0,\ 0,\ w)$ | $(0,\ -1,\ 0)$, $(-1,\ 0,\ 0)$ | $\{1\}\oplus\{2\}$ or $\{3\}\oplus\{4\}$ | $(-1,\ 0,\ 0)$ | $\{1\}\oplus\{3\}$ or $\{2\}\oplus\{4\}$ |
| | | | | $(0,\ -1,\ 0)$ | $\{1\}\oplus\{4\}$ or $\{2\}\oplus\{3\}$ |
| 67 | $SM(u,\ 0,\ 0)$ | $(0,\ -1,\ 0)$, $(0,\ 0,\ 1)$ | $\{1\}\oplus\{2\}$ or $\{3\}\oplus\{4\}$ | $(0,\ -1,\ 0)$ | $\{1\}\oplus\{3\}$ or $\{2\}\oplus\{4\}$ |
| | | | | $(0,\ 0,\ 1)$ | $\{1\}\oplus\{4\}$ or $\{2\}\oplus\{3\}$ |
| 68 | $DT(0,\ v,\ 0)$ | $(-1,\ 0,\ 0)$, $(0,\ 0,\ 1)$ | $\{1\}\oplus\{2\}$ or $\{3\}\oplus\{4\}$ | $(0,\ 0,\ 1)$ | $\{1\}\oplus\{3\}$ or $\{2\}\oplus\{4\}$ |
| | | | | $(-1,\ 0,\ 0)$ | $\{1\}\oplus\{4\}$ or $\{2\}\oplus\{3\}$ |
| 68 | $H(1,\ 0,\ w)$ | $(0,\ -1,\ 0)$, $(-1,\ 0,\ 0)$ | $\{1\}\oplus\{2\}$ or $\{3\}\oplus\{4\}$ | $(-1,\ 0,\ 0)$ | $\{1\}\oplus\{3\}$ or $\{2\}\oplus\{4\}$ |
| | | | | $(0,\ -1,\ 0)$ | $\{1\}\oplus\{4\}$ or $\{2\}\oplus\{3\}$ |
| 68 | $LD(0,\ 0,\ w)$ | $(0,\ -1,\ 0)$, $(-1,\ 0,\ 0)$ | $\{1\}\oplus\{2\}$ or $\{3\}\oplus\{4\}$ | $(-1,\ 0,\ 0)$ | $\{1\}\oplus\{3\}$ or $\{2\}\oplus\{4\}$ |
| | | | | $(0,\ -1,\ 0)$ | $\{1\}\oplus\{4\}$ or $\{2\}\oplus\{3\}$ |
| 68 | $SM(u,\ 0,\ 0)$ | $(0,\ -1,\ 0)$, $(0,\ 0,\ 1)$ | $\{1\}\oplus\{2\}$ or $\{3\}\oplus\{4\}$ | $(0,\ -1,\ 0)$ | $\{1\}\oplus\{3\}$ or $\{2\}\oplus\{4\}$ |
| | | | | $(0,\ 0,\ 1)$ | $\{1\}\oplus\{4\}$ or $\{2\}\oplus\{3\}$ |
| 69 | $A(u,\ 0,\ 1)$ | $(0,\ 0,\ -1)$, $(0,\ 1,\ 0)$ | $\{1\}\oplus\{2\}$ or $\{3\}\oplus\{4\}$ | $(0,\ 1,\ 0)$ | $\{1\}\oplus\{3\}$ or $\{2\}\oplus\{4\}$ |
| | | | | $(0,\ 0,\ -1)$ | $\{1\}\oplus\{4\}$ or $\{2\}\oplus\{3\}$ |
| 69 | $B(0,\ v,\ 1)$ | $(0,\ 0,\ -1)$, $(1,\ 0,\ 0)$ | $\{1\}\oplus\{2\}$ or $\{3\}\oplus\{4\}$ | $(0,\ 0,\ -1)$ | $\{1\}\oplus\{3\}$ or $\{2\}\oplus\{4\}$ |
| | | | | $(1,\ 0,\ 0)$ | $\{1\}\oplus\{4\}$ or $\{2\}\oplus\{3\}$ |
| 69 | $DT(0,\ v,\ 0)$ | $(0,\ 0,\ -1)$, $(1,\ 0,\ 0)$ | $\{1\}\oplus\{2\}$ or $\{3\}\oplus\{4\}$ | $(0,\ 0,\ -1)$ | $\{1\}\oplus\{3\}$ or $\{2\}\oplus\{4\}$ |
| | | | | $(1,\ 0,\ 0)$ | $\{1\}\oplus\{4\}$ or $\{2\}\oplus\{3\}$ |
| 69 | $H(0,\ 1,\ w)$ | $(0,\ 1,\ 0)$, $(1,\ 0,\ 0)$ | $\{1\}\oplus\{2\}$ or $\{3\}\oplus\{4\}$ | $(1,\ 0,\ 0)$ | $\{1\}\oplus\{3\}$ or $\{2\}\oplus\{4\}$ |
| | | | | $(0,\ 1,\ 0)$ | $\{1\}\oplus\{4\}$ or $\{2\}\oplus\{3\}$ |
| 69 | $LD(0,\ 0,\ w)$ | $(0,\ 1,\ 0)$, $(1,\ 0,\ 0)$ | $\{1\}\oplus\{2\}$ or $\{3\}\oplus\{4\}$ | $(1,\ 0,\ 0)$ | $\{1\}\oplus\{3\}$ or $\{2\}\oplus\{4\}$ |
| | | | | $(0,\ 1,\ 0)$ | $\{1\}\oplus\{4\}$ or $\{2\}\oplus\{3\}$ |
| 69 | $SM(u,\ 0,\ 0)$ | $(0,\ 0,\ -1)$, $(0,\ 1,\ 0)$ | $\{1\}\oplus\{2\}$ or $\{3\}\oplus\{4\}$ | $(0,\ 1,\ 0)$ | $\{1\}\oplus\{3\}$ or $\{2\}\oplus\{4\}$ |
| | | | | $(0,\ 0,\ -1)$ | $\{1\}\oplus\{4\}$ or $\{2\}\oplus\{3\}$ |
| 70 | $DT(0,\ v,\ 0)$ | $(0,\ 0,\ -1)$, $(1,\ 0,\ 0)$ | $\{1\}\oplus\{2\}$ or $\{3\}\oplus\{4\}$ | $(1,\ 0,\ 0)$ | $\{1\}\oplus\{3\}$ or $\{2\}\oplus\{4\}$ |
| | | | | $(0,\ 0,\ -1)$ | $\{1\}\oplus\{4\}$ or $\{2\}\oplus\{3\}$ |
| 70 | $LD(0,\ 0,\ w)$ | $(0,\ -1,\ 0)$, $(1,\ 0,\ 0)$ | $\{1\}\oplus\{2\}$ or $\{3\}\oplus\{4\}$ | $(0,\ -1,\ 0)$ | $\{1\}\oplus\{3\}$ or $\{2\}\oplus\{4\}$ |
| | | | | $(1,\ 0,\ 0)$ | $\{1\}\oplus\{4\}$ or $\{2\}\oplus\{3\}$ |
| 70 | $SM(u,\ 0,\ 0)$ | $(0,\ -1,\ 0)$, $(0,\ 0,\ -1)$ | $\{1\}\oplus\{2\}$ or $\{3\}\oplus\{4\}$ | $(0,\ 0,\ -1)$ | $\{1\}\oplus\{3\}$ or $\{2\}\oplus\{4\}$ |
| | | | | $(0,\ -1,\ 0)$ | $\{1\}\oplus\{4\}$ or $\{2\}\oplus\{3\}$ |
| 71 | $DT(0,\ v,\ 0)$ | $(0,\ 0,\ -1)$, $(1,\ 0,\ 0)$ | $\{1\}\oplus\{2\}$ or $\{3\}\oplus\{4\}$ | $(0,\ 0,\ -1)$ | $\{1\}\oplus\{3\}$ or $\{2\}\oplus\{4\}$ |
| | | | | $(1,\ 0,\ 0)$ | $\{1\}\oplus\{4\}$ or $\{2\}\oplus\{3\}$ |
| 71 | $LD(0,\ 0,\ w)$ | $(0,\ -1,\ 0)$, $(1,\ 0,\ 0)$ | $\{1\}\oplus\{2\}$ or $\{3\}\oplus\{4\}$ | $(1,\ 0,\ 0)$ | $\{1\}\oplus\{3\}$ or $\{2\}\oplus\{4\}$ |
| | | | | $(0,\ -1,\ 0)$ | $\{1\}\oplus\{4\}$ or $\{2\}\oplus\{3\}$ |

| SG | HSL | Location of nodal chain | Irreps of BC | Location of nodal loop | Irreps of BC |
|---|---|---|---|---|---|
| 71 | SM$(u,\ 0,\ 0)$ | $(0,\ 0,\ -1)$, $(0,\ -1,\ 0)$ | {1}⊕{2} or {3}⊕{4} | $(0,\ -1,\ 0)$ | {1}⊕{3} or {2}⊕{4} |
| | | | | $(0,\ 0,\ -1)$ | {1}⊕{4} or {2}⊕{3} |
| 72 | DT$(0,\ v,\ 0)$ | $(0,\ 0,\ -1)$, $(1,\ 0,\ 0)$ | {1}⊕{2} or {3}⊕{4} | $(0,\ 0,\ -1)$ | {1}⊕{3} or {2}⊕{4} |
| | | | | $(1,\ 0,\ 0)$ | {1}⊕{4} or {2}⊕{3} |
| 72 | LD$(0,\ 0,\ w)$ | $(0,\ -1,\ 0)$, $(1,\ 0,\ 0)$ | {1}⊕{2} or {3}⊕{4} | $(1,\ 0,\ 0)$ | {1}⊕{3} or {2}⊕{4} |
| | | | | $(0,\ -1,\ 0)$ | {1}⊕{4} or {2}⊕{3} |
| 72 | SM$(u,\ 0,\ 0)$ | $(0,\ 0,\ -1)$, $(0,\ -1,\ 0)$ | {1}⊕{2} or {3}⊕{4} | $(0,\ -1,\ 0)$ | {1}⊕{3} or {2}⊕{4} |
| | | | | $(0,\ 0,\ -1)$ | {1}⊕{4} or {2}⊕{3} |
| 73 | DT$(0,\ v,\ 0)$ | $(0,\ 0,\ -1)$, $(1,\ 0,\ 0)$ | {1}⊕{2} or {3}⊕{4} | $(0,\ 0,\ -1)$ | {1}⊕{3} or {2}⊕{4} |
| | | | | $(1,\ 0,\ 0)$ | {1}⊕{4} or {2}⊕{3} |
| 73 | LD$(0,\ 0,\ w)$ | $(0,\ -1,\ 0)$, $(1,\ 0,\ 0)$ | {1}⊕{2} or {3}⊕{4} | $(1,\ 0,\ 0)$ | {1}⊕{3} or {2}⊕{4} |
| | | | | $(0,\ -1,\ 0)$ | {1}⊕{4} or {2}⊕{3} |
| 73 | SM$(u,\ 0,\ 0)$ | $(0,\ 0,\ -1)$, $(0,\ -1,\ 0)$ | {1}⊕{2} or {3}⊕{4} | $(0,\ -1,\ 0)$ | {1}⊕{3} or {2}⊕{4} |
| | | | | $(0,\ 0,\ -1)$ | {1}⊕{4} or {2}⊕{3} |
| 74 | DT$(0,\ v,\ 0)$ | $(0,\ 0,\ -1)$, $(1,\ 0,\ 0)$ | {1}⊕{2} or {3}⊕{4} | $(0,\ 0,\ -1)$ | {1}⊕{3} or {2}⊕{4} |
| | | | | $(1,\ 0,\ 0)$ | {1}⊕{4} or {2}⊕{3} |
| 74 | LD$(0,\ 0,\ w)$ | $(0,\ -1,\ 0)$, $(1,\ 0,\ 0)$ | {1}⊕{2} or {3}⊕{4} | $(1,\ 0,\ 0)$ | {1}⊕{3} or {2}⊕{4} |
| | | | | $(0,\ -1,\ 0)$ | {1}⊕{4} or {2}⊕{3} |
| 74 | SM$(u,\ 0,\ 0)$ | $(0,\ 0,\ -1)$, $(0,\ -1,\ 0)$ | {1}⊕{2} or {3}⊕{4} | $(0,\ -1,\ 0)$ | {1}⊕{3} or {2}⊕{4} |
| | | | | $(0,\ 0,\ -1)$ | {1}⊕{4} or {2}⊕{3} |
| 99 | W$\left(0,\ \frac{1}{2},\ w\right)$ | $(1,\ 0,\ 0)$, $(0,\ -1,\ 0)$ | 1⊕2 or 3⊕4 | $(1,\ 0,\ 0)$ | 1⊕3 or 2⊕4 |
| | | | | $(0,\ -1,\ 0)$ | 1⊕4 or 2⊕3 |
| 101 | W$\left(0,\ \frac{1}{2},\ w\right)$ | $(1,\ 0,\ 0)$, $(0,\ -1,\ 0)$ | 1⊕2 or 3⊕4 | $(1,\ 0,\ 0)$ | 1⊕3 or 2⊕4 |
| | | | | $(0,\ -1,\ 0)$ | 1⊕4 or 2⊕3 |
| 103 | W$\left(0,\ \frac{1}{2},\ w\right)$ | $(1,\ 0,\ 0)$, $(0,\ -1,\ 0)$ | 1⊕2 or 3⊕4 | $(1,\ 0,\ 0)$ | 1⊕3 or 2⊕4 |
| | | | | $(0,\ -1,\ 0)$ | 1⊕4 or 2⊕3 |
| 105 | W$\left(0,\ \frac{1}{2},\ w\right)$ | $(1,\ 0,\ 0)$, $(0,\ -1,\ 0)$ | 1⊕2 or 3⊕4 | $(1,\ 0,\ 0)$ | 1⊕3 or 2⊕4 |
| | | | | $(0,\ -1,\ 0)$ | 1⊕4 or 2⊕3 |
| 107 | W$\left(\frac{1}{2},\ \frac{1}{2},\ w\right)$ | $\left(-\frac{\sqrt{2}}{2},\ -\frac{\sqrt{2}}{2},\ 0\right)$, $\left(\frac{\sqrt{2}}{2},\ -\frac{\sqrt{2}}{2},\ 0\right)$ | 1⊕2 or 3⊕4 | $\left(-\frac{\sqrt{2}}{2},\ -\frac{\sqrt{2}}{2},\ 0\right)$ | 1⊕3 or 2⊕4 |
| | | | | $\left(\frac{\sqrt{2}}{2},\ -\frac{\sqrt{2}}{2},\ 0\right)$ | 1⊕4 or 2⊕3 |
| 108 | W$\left(\frac{1}{2},\ \frac{1}{2},\ w\right)$ | $\left(-\frac{\sqrt{2}}{2},\ -\frac{\sqrt{2}}{2},\ 0\right)$, $\left(\frac{\sqrt{2}}{2},\ -\frac{\sqrt{2}}{2},\ 0\right)$ | 1⊕2 or 3⊕4 | $\left(-\frac{\sqrt{2}}{2},\ -\frac{\sqrt{2}}{2},\ 0\right)$ | 1⊕3 or 2⊕4 |
| | | | | $\left(\frac{\sqrt{2}}{2},\ -\frac{\sqrt{2}}{2},\ 0\right)$ | 1⊕4 or 2⊕3 |
| 115 | W$\left(0,\ \frac{1}{2},\ w\right)$ | $(1,\ 0,\ 0)$, $(0,\ -1,\ 0)$ | 1⊕2 or 3⊕4 | $(1,\ 0,\ 0)$ | 1⊕3 or 2⊕4 |
| | | | | $(0,\ -1,\ 0)$ | 1⊕4 or 2⊕3 |
| 116 | W$\left(0,\ \frac{1}{2},\ w\right)$ | $(1,\ 0,\ 0)$, $(0,\ -1,\ 0)$ | 1⊕2 or 3⊕4 | $(1,\ 0,\ 0)$ | 1⊕3 or 2⊕4 |
| | | | | $(0,\ -1,\ 0)$ | 1⊕4 or 2⊕3 |
| 121 | W$\left(\frac{1}{2},\ \frac{1}{2},\ w\right)$ | $\left(-\frac{\sqrt{2}}{2},\ -\frac{\sqrt{2}}{2},\ 0\right)$, $\left(-\frac{\sqrt{2}}{2},\ \frac{\sqrt{2}}{2},\ 0\right)$ | 1⊕2 or 3⊕4 | $\left(-\frac{\sqrt{2}}{2},\ -\frac{\sqrt{2}}{2},\ 0\right)$ | 1⊕3 or 2⊕4 |
| | | | | $\left(-\frac{\sqrt{2}}{2},\ \frac{\sqrt{2}}{2},\ 0\right)$ | 1⊕4 or 2⊕3 |
| 123 | DT$(0,\ v,\ 0)$ | $(0,\ 0,\ 1)$, $(1,\ 0,\ 0)$ | {1}⊕{2} or {3}⊕{4} | $(0,\ 0,\ 1)$ | {1}⊕{3} or {2}⊕{4} |
| | | | | $(1,\ 0,\ 0)$ | {1}⊕{4} or {2}⊕{3} |
| 123 | S$\left(u,\ u,\ \frac{1}{2}\right)$ | $(0,\ 0,\ 1)$, $\left(\frac{\sqrt{2}}{2},\ -\frac{\sqrt{2}}{2},\ 0\right)$ | {1}⊕{2} or {3}⊕{4} | $\left(\frac{\sqrt{2}}{2},\ -\frac{\sqrt{2}}{2},\ 0\right)$ | {1}⊕{3} or {2}⊕{4} |
| | | | | $(0,\ 0,\ 1)$ | {1}⊕{4} or {2}⊕{3} |

| SG | HSL | Location of nodal chain | Irreps of BC | Location of nodal loop | Irreps of BC |
|---|---|---|---|---|---|
| 123 | SM$(u,\ u,\ 0)$ | $(0,\ 0,\ 1)$, $\left(\frac{\sqrt{2}}{2},\ -\frac{\sqrt{2}}{2},\ 0\right)$ | {1}⊕{2} or {3}⊕{4} | $\left(\frac{\sqrt{2}}{2},\ -\frac{\sqrt{2}}{2},\ 0\right)$ | {1}⊕{3} or {2}⊕{4} |
| | | | | $(0,\ 0,\ 1)$ | {1}⊕{4} or {2}⊕{3} |
| 123 | T$\left(u,\ \frac{1}{2},\ \frac{1}{2}\right)$ | $(0,\ 0,\ 1)$, $(0,\ -1,\ 0)$ | {1}⊕{2} or {3}⊕{4} | $(0,\ -1,\ 0)$ | {1}⊕{3} or {2}⊕{4} |
| | | | | $(0,\ 0,\ 1)$ | {1}⊕{4} or {2}⊕{3} |
| 123 | U$\left(0,\ v,\ \frac{1}{2}\right)$ | $(0,\ 0,\ 1)$, $(1,\ 0,\ 0)$ | {1}⊕{2} or {3}⊕{4} | $(0,\ 0,\ 1)$ | {1}⊕{3} or {2}⊕{4} |
| | | | | $(1,\ 0,\ 0)$ | {1}⊕{4} or {2}⊕{3} |
| 123 | W$\left(0,\ \frac{1}{2},\ w\right)$ | $(1,\ 0,\ 0)$, $(0,\ -1,\ 0)$ | {1}⊕{2} or {3}⊕{4} | $(1,\ 0,\ 0)$ | {1}⊕{3} or {2}⊕{4} |
| | | | | $(0,\ -1,\ 0)$ | {1}⊕{4} or {2}⊕{3} |
| 123 | Y$\left(u,\ \frac{1}{2},\ 0\right)$ | $(0,\ 0,\ 1)$, $(0,\ -1,\ 0)$ | {1}⊕{2} or {3}⊕{4} | $(0,\ -1,\ 0)$ | {1}⊕{3} or {2}⊕{4} |
| | | | | $(0,\ 0,\ 1)$ | {1}⊕{4} or {2}⊕{3} |
| 124 | DT$(0,\ v,\ 0)$ | $(0,\ 0,\ 1)$, $(1,\ 0,\ 0)$ | {1}⊕{2} or {3}⊕{4} | $(0,\ 0,\ 1)$ | {1}⊕{3} or {2}⊕{4} |
| | | | | $(1,\ 0,\ 0)$ | {1}⊕{4} or {2}⊕{3} |
| 124 | SM$(u,\ u,\ 0)$ | $(0,\ 0,\ 1)$, $\left(\frac{\sqrt{2}}{2},\ -\frac{\sqrt{2}}{2},\ 0\right)$ | {1}⊕{2} or {3}⊕{4} | $\left(\frac{\sqrt{2}}{2},\ -\frac{\sqrt{2}}{2},\ 0\right)$ | {1}⊕{3} or {2}⊕{4} |
| | | | | $(0,\ 0,\ 1)$ | {1}⊕{4} or {2}⊕{3} |
| 124 | W$\left(0,\ \frac{1}{2},\ w\right)$ | $(1,\ 0,\ 0)$, $(0,\ -1,\ 0)$ | {1}⊕{2} or {3}⊕{4} | $(1,\ 0,\ 0)$ | {1}⊕{3} or {2}⊕{4} |
| | | | | $(0,\ -1,\ 0)$ | {1}⊕{4} or {2}⊕{3} |
| 124 | Y$\left(u,\ \frac{1}{2},\ 0\right)$ | $(0,\ 0,\ 1)$, $(0,\ -1,\ 0)$ | {1}⊕{2} or {3}⊕{4} | $(0,\ -1,\ 0)$ | {1}⊕{3} or {2}⊕{4} |
| | | | | $(0,\ 0,\ 1)$ | {1}⊕{4} or {2}⊕{3} |
| 125 | DT$(0,\ v,\ 0)$ | $(0,\ 0,\ 1)$, $(1,\ 0,\ 0)$ | {1}⊕{2} or {3}⊕{4} | $(0,\ 0,\ 1)$ | {1}⊕{3} or {2}⊕{4} |
| | | | | $(1,\ 0,\ 0)$ | {1}⊕{4} or {2}⊕{3} |
| 125 | S$\left(u,\ u,\ \frac{1}{2}\right)$ | $(0,\ 0,\ 1)$, $\left(\frac{\sqrt{2}}{2},\ -\frac{\sqrt{2}}{2},\ 0\right)$ | {1}⊕{2} or {3}⊕{4} | $\left(\frac{\sqrt{2}}{2},\ -\frac{\sqrt{2}}{2},\ 0\right)$ | {1}⊕{3} or {2}⊕{4} |
| | | | | $(0,\ 0,\ 1)$ | {1}⊕{4} or {2}⊕{3} |
| 125 | SM$(u,\ u,\ 0)$ | $(0,\ 0,\ 1)$, $\left(\frac{\sqrt{2}}{2},\ -\frac{\sqrt{2}}{2},\ 0\right)$ | {1}⊕{2} or {3}⊕{4} | $\left(\frac{\sqrt{2}}{2},\ -\frac{\sqrt{2}}{2},\ 0\right)$ | {1}⊕{3} or {2}⊕{4} |
| | | | | $(0,\ 0,\ 1)$ | {1}⊕{4} or {2}⊕{3} |
| 125 | U$\left(0,\ v,\ \frac{1}{2}\right)$ | $(0,\ 0,\ 1)$, $(1,\ 0,\ 0)$ | {1}⊕{2} or {3}⊕{4} | $(0,\ 0,\ 1)$ | {1}⊕{3} or {2}⊕{4} |
| | | | | $(1,\ 0,\ 0)$ | {1}⊕{4} or {2}⊕{3} |
| 126 | DT$(0,\ v,\ 0)$ | $(0,\ 0,\ 1)$, $(1,\ 0,\ 0)$ | {1}⊕{2} or {3}⊕{4} | $(0,\ 0,\ 1)$ | {1}⊕{3} or {2}⊕{4} |
| | | | | $(1,\ 0,\ 0)$ | {1}⊕{4} or {2}⊕{3} |
| 126 | SM$(u,\ u,\ 0)$ | $(0,\ 0,\ 1)$, $\left(\frac{\sqrt{2}}{2},\ -\frac{\sqrt{2}}{2},\ 0\right)$ | {1}⊕{2} or {3}⊕{4} | $\left(\frac{\sqrt{2}}{2},\ -\frac{\sqrt{2}}{2},\ 0\right)$ | {1}⊕{3} or {2}⊕{4} |
| | | | | $(0,\ 0,\ 1)$ | {1}⊕{4} or {2}⊕{3} |
| 126 | T$\left(u,\ \frac{1}{2},\ \frac{1}{2}\right)$ | $(0,\ 0,\ 1)$, $(0,\ -1,\ 0)$ | {1}⊕{2} or {3}⊕{4} | $(0,\ 0,\ 1)$ | {1}⊕{3} or {2}⊕{4} |
| | | | | $(0,\ -1,\ 0)$ | {1}⊕{4} or {2}⊕{3} |
| 127 | DT$(0,\ v,\ 0)$ | $(0,\ 0,\ 1)$, $(1,\ 0,\ 0)$ | {1}⊕{2} or {3}⊕{4} | $(0,\ 0,\ 1)$ | {1}⊕{3} or {2}⊕{4} |
| | | | | $(1,\ 0,\ 0)$ | {1}⊕{4} or {2}⊕{3} |
| 127 | S$\left(u,\ u,\ \frac{1}{2}\right)$ | $(0,\ 0,\ 1)$, $\left(\frac{\sqrt{2}}{2},\ -\frac{\sqrt{2}}{2},\ 0\right)$ | {1}⊕{2} or {3}⊕{4} | $\left(\frac{\sqrt{2}}{2},\ -\frac{\sqrt{2}}{2},\ 0\right)$ | {1}⊕{3} or {2}⊕{4} |
| | | | | $(0,\ 0,\ 1)$ | {1}⊕{4} or {2}⊕{3} |
| 127 | SM$(u,\ u,\ 0)$ | $(0,\ 0,\ 1)$, $\left(\frac{\sqrt{2}}{2},\ -\frac{\sqrt{2}}{2},\ 0\right)$ | {1}⊕{2} or {3}⊕{4} | $\left(\frac{\sqrt{2}}{2},\ -\frac{\sqrt{2}}{2},\ 0\right)$ | {1}⊕{3} or {2}⊕{4} |
| | | | | $(0,\ 0,\ 1)$ | {1}⊕{4} or {2}⊕{3} |
| 127 | U$\left(0,\ v,\ \frac{1}{2}\right)$ | $(0,\ 0,\ 1)$, $(1,\ 0,\ 0)$ | {1}⊕{2} or {3}⊕{4} | $(0,\ 0,\ 1)$ | {1}⊕{3} or {2}⊕{4} |
| | | | | $(1,\ 0,\ 0)$ | {1}⊕{4} or {2}⊕{3} |
| 128 | DT$(0,\ v,\ 0)$ | $(0,\ 0,\ 1)$, $(1,\ 0,\ 0)$ | {1}⊕{2} or {3}⊕{4} | $(0,\ 0,\ 1)$ | {1}⊕{3} or {2}⊕{4} |
| | | | | $(1,\ 0,\ 0)$ | {1}⊕{4} or {2}⊕{3} |

| SG | HSL | Location of nodal chain | Irreps of BC | Location of nodal loop | Irreps of BC |
|---|---|---|---|---|---|
| 128 | SM$(u,\ u,\ 0)$ | $(0,\ 0,\ 1)$, $\left(\frac{\sqrt{2}}{2},\ -\frac{\sqrt{2}}{2},\ 0\right)$ | $\{1\}\oplus\{2\}$ or $\{3\}\oplus\{4\}$ | $\left(\frac{\sqrt{2}}{2},\ -\frac{\sqrt{2}}{2},\ 0\right)$ | $\{1\}\oplus\{3\}$ or $\{2\}\oplus\{4\}$ |
| | | | | $(0,\ 0,\ 1)$ | $\{1\}\oplus\{4\}$ or $\{2\}\oplus\{3\}$ |
| 129 | DT$(0,\ v,\ 0)$ | $(0,\ 0,\ 1)$, $(1,\ 0,\ 0)$ | $\{1\}\oplus\{2\}$ or $\{3\}\oplus\{4\}$ | $(0,\ 0,\ 1)$ | $\{1\}\oplus\{3\}$ or $\{2\}\oplus\{4\}$ |
| | | | | $(1,\ 0,\ 0)$ | $\{1\}\oplus\{4\}$ or $\{2\}\oplus\{3\}$ |
| 129 | S$\left(u,\ u,\ \frac{1}{2}\right)$ | $(0,\ 0,\ 1)$, $\left(\frac{\sqrt{2}}{2},\ -\frac{\sqrt{2}}{2},\ 0\right)$ | $\{1\}\oplus\{2\}$ or $\{3\}\oplus\{4\}$ | $\left(\frac{\sqrt{2}}{2},\ -\frac{\sqrt{2}}{2},\ 0\right)$ | $\{1\}\oplus\{3\}$ or $\{2\}\oplus\{4\}$ |
| | | | | $(0,\ 0,\ 1)$ | $\{1\}\oplus\{4\}$ or $\{2\}\oplus\{3\}$ |
| 129 | SM$(u,\ u,\ 0)$ | $(0,\ 0,\ 1)$, $\left(\frac{\sqrt{2}}{2},\ -\frac{\sqrt{2}}{2},\ 0\right)$ | $\{1\}\oplus\{2\}$ or $\{3\}\oplus\{4\}$ | $\left(\frac{\sqrt{2}}{2},\ -\frac{\sqrt{2}}{2},\ 0\right)$ | $\{1\}\oplus\{3\}$ or $\{2\}\oplus\{4\}$ |
| | | | | $(0,\ 0,\ 1)$ | $\{1\}\oplus\{4\}$ or $\{2\}\oplus\{3\}$ |
| 129 | U$\left(0,\ v,\ \frac{1}{2}\right)$ | $(0,\ 0,\ 1)$, $(1,\ 0,\ 0)$ | $\{1\}\oplus\{2\}$ or $\{3\}\oplus\{4\}$ | $(0,\ 0,\ 1)$ | $\{1\}\oplus\{3\}$ or $\{2\}\oplus\{4\}$ |
| | | | | $(1,\ 0,\ 0)$ | $\{1\}\oplus\{4\}$ or $\{2\}\oplus\{3\}$ |
| 130 | DT$(0,\ v,\ 0)$ | $(0,\ 0,\ 1)$, $(1,\ 0,\ 0)$ | $\{1\}\oplus\{2\}$ or $\{3\}\oplus\{4\}$ | $(0,\ 0,\ 1)$ | $\{1\}\oplus\{3\}$ or $\{2\}\oplus\{4\}$ |
| | | | | $(1,\ 0,\ 0)$ | $\{1\}\oplus\{4\}$ or $\{2\}\oplus\{3\}$ |
| 130 | SM$(u,\ u,\ 0)$ | $(0,\ 0,\ 1)$, $\left(\frac{\sqrt{2}}{2},\ -\frac{\sqrt{2}}{2},\ 0\right)$ | $\{1\}\oplus\{2\}$ or $\{3\}\oplus\{4\}$ | $\left(\frac{\sqrt{2}}{2},\ -\frac{\sqrt{2}}{2},\ 0\right)$ | $\{1\}\oplus\{3\}$ or $\{2\}\oplus\{4\}$ |
| | | | | $(0,\ 0,\ 1)$ | $\{1\}\oplus\{4\}$ or $\{2\}\oplus\{3\}$ |
| 131 | DT$(0,\ v,\ 0)$ | $(0,\ 0,\ 1)$, $(1,\ 0,\ 0)$ | $\{1\}\oplus\{2\}$ or $\{3\}\oplus\{4\}$ | $(0,\ 0,\ 1)$ | $\{1\}\oplus\{3\}$ or $\{2\}\oplus\{4\}$ |
| | | | | $(1,\ 0,\ 0)$ | $\{1\}\oplus\{4\}$ or $\{2\}\oplus\{3\}$ |
| 131 | SM$(u,\ u,\ 0)$ | $(0,\ 0,\ 1)$, $\left(\frac{\sqrt{2}}{2},\ -\frac{\sqrt{2}}{2},\ 0\right)$ | $\{1\}\oplus\{2\}$ or $\{3\}\oplus\{4\}$ | $\left(\frac{\sqrt{2}}{2},\ -\frac{\sqrt{2}}{2},\ 0\right)$ | $\{1\}\oplus\{3\}$ or $\{2\}\oplus\{4\}$ |
| | | | | $(0,\ 0,\ 1)$ | $\{1\}\oplus\{4\}$ or $\{2\}\oplus\{3\}$ |
| 131 | T$\left(u,\ \frac{1}{2},\ \frac{1}{2}\right)$ | $(0,\ 0,\ 1)$, $(0,\ -1,\ 0)$ | $\{1\}\oplus\{2\}$ or $\{3\}\oplus\{4\}$ | $(0,\ -1,\ 0)$ | $\{1\}\oplus\{3\}$ or $\{2\}\oplus\{4\}$ |
| | | | | $(0,\ 0,\ 1)$ | $\{1\}\oplus\{4\}$ or $\{2\}\oplus\{3\}$ |
| 131 | U$\left(0,\ v,\ \frac{1}{2}\right)$ | $(0,\ 0,\ 1)$, $(1,\ 0,\ 0)$ | $\{1\}\oplus\{2\}$ or $\{3\}\oplus\{4\}$ | $(0,\ 0,\ 1)$ | $\{1\}\oplus\{3\}$ or $\{2\}\oplus\{4\}$ |
| | | | | $(1,\ 0,\ 0)$ | $\{1\}\oplus\{4\}$ or $\{2\}\oplus\{3\}$ |
| 131 | W$\left(0,\ \frac{1}{2},\ w\right)$ | $(1,\ 0,\ 0)$, $(0,\ -1,\ 0)$ | $\{1\}\oplus\{2\}$ or $\{3\}\oplus\{4\}$ | $(1,\ 0,\ 0)$ | $\{1\}\oplus\{3\}$ or $\{2\}\oplus\{4\}$ |
| | | | | $(0,\ -1,\ 0)$ | $\{1\}\oplus\{4\}$ or $\{2\}\oplus\{3\}$ |
| 131 | Y$\left(u,\ \frac{1}{2},\ 0\right)$ | $(0,\ 0,\ 1)$, $(0,\ -1,\ 0)$ | $\{1\}\oplus\{2\}$ or $\{3\}\oplus\{4\}$ | $(0,\ -1,\ 0)$ | $\{1\}\oplus\{3\}$ or $\{2\}\oplus\{4\}$ |
| | | | | $(0,\ 0,\ 1)$ | $\{1\}\oplus\{4\}$ or $\{2\}\oplus\{3\}$ |
| 132 | DT$(0,\ v,\ 0)$ | $(0,\ 0,\ 1)$, $(1,\ 0,\ 0)$ | $\{1\}\oplus\{2\}$ or $\{3\}\oplus\{4\}$ | $(0,\ 0,\ 1)$ | $\{1\}\oplus\{3\}$ or $\{2\}\oplus\{4\}$ |
| | | | | $(1,\ 0,\ 0)$ | $\{1\}\oplus\{4\}$ or $\{2\}\oplus\{3\}$ |
| 132 | S$\left(u,\ u,\ \frac{1}{2}\right)$ | $(0,\ 0,\ 1)$, $\left(\frac{\sqrt{2}}{2},\ -\frac{\sqrt{2}}{2},\ 0\right)$ | $\{1\}\oplus\{3\}$ or $\{2\}\oplus\{4\}$ | $(0,\ 0,\ 1)$ | $\{1\}\oplus\{2\}$ or $\{3\}\oplus\{4\}$ |
| | | | | $\left(\frac{\sqrt{2}}{2},\ -\frac{\sqrt{2}}{2},\ 0\right)$ | $\{1\}\oplus\{4\}$ or $\{2\}\oplus\{3\}$ |
| 132 | SM$(u,\ u,\ 0)$ | $(0,\ 0,\ 1)$, $\left(\frac{\sqrt{2}}{2},\ -\frac{\sqrt{2}}{2},\ 0\right)$ | $\{1\}\oplus\{2\}$ or $\{3\}\oplus\{4\}$ | $\left(\frac{\sqrt{2}}{2},\ -\frac{\sqrt{2}}{2},\ 0\right)$ | $\{1\}\oplus\{3\}$ or $\{2\}\oplus\{4\}$ |
| | | | | $(0,\ 0,\ 1)$ | $\{1\}\oplus\{4\}$ or $\{2\}\oplus\{3\}$ |
| 132 | W$\left(0,\ \frac{1}{2},\ w\right)$ | $(1,\ 0,\ 0)$, $(0,\ -1,\ 0)$ | $\{1\}\oplus\{2\}$ or $\{3\}\oplus\{4\}$ | $(1,\ 0,\ 0)$ | $\{1\}\oplus\{3\}$ or $\{2\}\oplus\{4\}$ |
| | | | | $(0,\ -1,\ 0)$ | $\{1\}\oplus\{4\}$ or $\{2\}\oplus\{3\}$ |
| 132 | Y$\left(u,\ \frac{1}{2},\ 0\right)$ | $(0,\ 0,\ 1)$, $(0,\ -1,\ 0)$ | $\{1\}\oplus\{2\}$ or $\{3\}\oplus\{4\}$ | $(0,\ -1,\ 0)$ | $\{1\}\oplus\{3\}$ or $\{2\}\oplus\{4\}$ |
| | | | | $(0,\ 0,\ 1)$ | $\{1\}\oplus\{4\}$ or $\{2\}\oplus\{3\}$ |
| 133 | DT$(0,\ v,\ 0)$ | $(0,\ 0,\ 1)$, $(1,\ 0,\ 0)$ | $\{1\}\oplus\{2\}$ or $\{3\}\oplus\{4\}$ | $(0,\ 0,\ 1)$ | $\{1\}\oplus\{3\}$ or $\{2\}\oplus\{4\}$ |
| | | | | $(1,\ 0,\ 0)$ | $\{1\}\oplus\{4\}$ or $\{2\}\oplus\{3\}$ |
| 133 | SM$(u,\ u,\ 0)$ | $(0,\ 0,\ 1)$, $\left(\frac{\sqrt{2}}{2},\ -\frac{\sqrt{2}}{2},\ 0\right)$ | $\{1\}\oplus\{2\}$ or $\{3\}\oplus\{4\}$ | $\left(\frac{\sqrt{2}}{2},\ -\frac{\sqrt{2}}{2},\ 0\right)$ | $\{1\}\oplus\{3\}$ or $\{2\}\oplus\{4\}$ |
| | | | | $(0,\ 0,\ 1)$ | $\{1\}\oplus\{4\}$ or $\{2\}\oplus\{3\}$ |

| SG | HSL | Location of nodal chain | Irreps of BC | Location of nodal loop | Irreps of BC |
|---|---|---|---|---|---|
| 133 | U$\left(0,\ v,\ \frac{1}{2}\right)$ | (0, 0, 1), (1, 0, 0) | {1}⊕{2} or {3}⊕{4} | (0, 0, 1) | {1}⊕{3} or {2}⊕{4} |
| | | | | (1, 0, 0) | {1}⊕{4} or {2}⊕{3} |
| 134 | DT(0, $v$, 0) | (0, 0, 1), (1, 0, 0) | {1}⊕{2} or {3}⊕{4} | (0, 0, 1) | {1}⊕{3} or {2}⊕{4} |
| | | | | (1, 0, 0) | {1}⊕{4} or {2}⊕{3} |
| 134 | S$\left(u,\ u,\ \frac{1}{2}\right)$ | (0, 0, 1), $\left(\frac{\sqrt{2}}{2},\ -\frac{\sqrt{2}}{2},\ 0\right)$ | {1}⊕{3} or {2}⊕{4} | (0, 0, 1) | {1}⊕{2} or {3}⊕{4} |
| | | | | $\left(\frac{\sqrt{2}}{2},\ -\frac{\sqrt{2}}{2},\ 0\right)$ | {1}⊕{4} or {2}⊕{3} |
| 134 | SM($u$, $u$, 0) | (0, 0, 1), $\left(\frac{\sqrt{2}}{2},\ -\frac{\sqrt{2}}{2},\ 0\right)$ | {1}⊕{2} or {3}⊕{4} | $\left(\frac{\sqrt{2}}{2},\ -\frac{\sqrt{2}}{2},\ 0\right)$ | {1}⊕{3} or {2}⊕{4} |
| | | | | (0, 0, 1) | {1}⊕{4} or {2}⊕{3} |
| 134 | T$\left(u,\ \frac{1}{2},\ \frac{1}{2}\right)$ | (0, 0, 1), (0, −1, 0) | {1}⊕{2} or {3}⊕{4} | (0, 0, 1) | {1}⊕{3} or {2}⊕{4} |
| | | | | (0, −1, 0) | {1}⊕{4} or {2}⊕{3} |
| 135 | DT(0, $v$, 0) | (0, 0, 1), (1, 0, 0) | {1}⊕{2} or {3}⊕{4} | (0, 0, 1) | {1}⊕{3} or {2}⊕{4} |
| | | | | (1, 0, 0) | {1}⊕{4} or {2}⊕{3} |
| 135 | SM($u$, $u$, 0) | (0, 0, 1), $\left(\frac{\sqrt{2}}{2},\ -\frac{\sqrt{2}}{2},\ 0\right)$ | {1}⊕{2} or {3}⊕{4} | $\left(\frac{\sqrt{2}}{2},\ -\frac{\sqrt{2}}{2},\ 0\right)$ | {1}⊕{3} or {2}⊕{4} |
| | | | | (0, 0, 1) | {1}⊕{4} or {2}⊕{3} |
| 135 | U$\left(0,\ v,\ \frac{1}{2}\right)$ | (0, 0, 1), (1, 0, 0) | {1}⊕{2} or {3}⊕{4} | (0, 0, 1) | {1}⊕{3} or {2}⊕{4} |
| | | | | (1, 0, 0) | {1}⊕{4} or {2}⊕{3} |
| 136 | DT(0, $v$, 0) | (0, 0, 1), (1, 0, 0) | {1}⊕{2} or {3}⊕{4} | (0, 0, 1) | {1}⊕{3} or {2}⊕{4} |
| | | | | (1, 0, 0) | {1}⊕{4} or {2}⊕{3} |
| 136 | S$\left(u,\ u,\ \frac{1}{2}\right)$ | (0, 0, 1), $\left(\frac{\sqrt{2}}{2},\ -\frac{\sqrt{2}}{2},\ 0\right)$ | {1}⊕{3} or {2}⊕{4} | (0, 0, 1) | {1}⊕{2} or {3}⊕{4} |
| | | | | $\left(\frac{\sqrt{2}}{2},\ -\frac{\sqrt{2}}{2},\ 0\right)$ | {1}⊕{4} or {2}⊕{3} |
| 136 | SM($u$, $u$, 0) | (0, 0, 1), $\left(\frac{\sqrt{2}}{2},\ -\frac{\sqrt{2}}{2},\ 0\right)$ | {1}⊕{2} or {3}⊕{4} | $\left(\frac{\sqrt{2}}{2},\ -\frac{\sqrt{2}}{2},\ 0\right)$ | {1}⊕{3} or {2}⊕{4} |
| | | | | (0, 0, 1) | {1}⊕{4} or {2}⊕{3} |
| 137 | DT(0, $v$, 0) | (0, 0, 1), (1, 0, 0) | {1}⊕{2} or {3}⊕{4} | (0, 0, 1) | {1}⊕{3} or {2}⊕{4} |
| | | | | (1, 0, 0) | {1}⊕{4} or {2}⊕{3} |
| 137 | SM($u$, $u$, 0) | (0, 0, 1), $\left(\frac{\sqrt{2}}{2},\ -\frac{\sqrt{2}}{2},\ 0\right)$ | {1}⊕{2} or {3}⊕{4} | $\left(\frac{\sqrt{2}}{2},\ -\frac{\sqrt{2}}{2},\ 0\right)$ | {1}⊕{3} or {2}⊕{4} |
| | | | | (0, 0, 1) | {1}⊕{4} or {2}⊕{3} |
| 137 | U$\left(0,\ v,\ \frac{1}{2}\right)$ | (0, 0, 1), (1, 0, 0) | {1}⊕{2} or {3}⊕{4} | (0, 0, 1) | {1}⊕{3} or {2}⊕{4} |
| | | | | (1, 0, 0) | {1}⊕{4} or {2}⊕{3} |
| 138 | DT(0, $v$, 0) | (0, 0, 1), (1, 0, 0) | {1}⊕{2} or {3}⊕{4} | (0, 0, 1) | {1}⊕{3} or {2}⊕{4} |
| | | | | (1, 0, 0) | {1}⊕{4} or {2}⊕{3} |
| 138 | S$\left(u,\ u,\ \frac{1}{2}\right)$ | (0, 0, 1), $\left(\frac{\sqrt{2}}{2},\ -\frac{\sqrt{2}}{2},\ 0\right)$ | {1}⊕{3} or {2}⊕{4} | (0, 0, 1) | {1}⊕{2} or {3}⊕{4} |
| | | | | $\left(\frac{\sqrt{2}}{2},\ -\frac{\sqrt{2}}{2},\ 0\right)$ | {1}⊕{4} or {2}⊕{3} |
| 138 | SM($u$, $u$, 0) | (0, 0, 1), $\left(\frac{\sqrt{2}}{2},\ -\frac{\sqrt{2}}{2},\ 0\right)$ | {1}⊕{2} or {3}⊕{4} | $\left(\frac{\sqrt{2}}{2},\ -\frac{\sqrt{2}}{2},\ 0\right)$ | {1}⊕{3} or {2}⊕{4} |
| | | | | (0, 0, 1) | {1}⊕{4} or {2}⊕{3} |
| 139 | DT($u$, $u$, 0) | $\left(\frac{\sqrt{2}}{2},\ -\frac{\sqrt{2}}{2},\ 0\right)$, (0, 0, −1) | {1}⊕{2} or {3}⊕{4} | $\left(\frac{\sqrt{2}}{2},\ -\frac{\sqrt{2}}{2},\ 0\right)$ | {1}⊕{3} or {2}⊕{4} |
| | | | | (0, 0, −1) | {1}⊕{4} or {2}⊕{3} |
| 139 | SM($u$, 0, 0) | (0, 1, 0), (0, 0, −1) | {1}⊕{2} or {3}⊕{4} | (0, 1, 0) | {1}⊕{3} or {2}⊕{4} |
| | | | | (0, 0, −1) | {1}⊕{4} or {2}⊕{3} |
| 139 | W$\left(\frac{1}{2},\ \frac{1}{2},\ w\right)$ | $\left(-\frac{\sqrt{2}}{2},\ -\frac{\sqrt{2}}{2},\ 0\right)$, $\left(\frac{\sqrt{2}}{2},\ -\frac{\sqrt{2}}{2},\ 0\right)$ | {1}⊕{2} or {3}⊕{4} | $\left(-\frac{\sqrt{2}}{2},\ -\frac{\sqrt{2}}{2},\ 0\right)$ | {1}⊕{3} or {2}⊕{4} |
| | | | | $\left(\frac{\sqrt{2}}{2},\ -\frac{\sqrt{2}}{2},\ 0\right)$ | {1}⊕{4} or {2}⊕{3} |

| SG | HSL | Location of nodal chain | Irreps of BC | Location of nodal loop | Irreps of BC |
|---|---|---|---|---|---|
| 139 | Y$(u,\ 1-u,\ 0)$ | $\left(-\frac{\sqrt{2}}{2},\ -\frac{\sqrt{2}}{2},\ 0\right)$, $(0,\ 0,\ -1)$ | $\{1\}\oplus\{2\}$ or $\{3\}\oplus\{4\}$ | $(0,\ 0,\ -1)$ | $\{1\}\oplus\{3\}$ or $\{2\}\oplus\{4\}$ |
| | | | | $\left(-\frac{\sqrt{2}}{2},\ -\frac{\sqrt{2}}{2},\ 0\right)$ | $\{1\}\oplus\{4\}$ or $\{2\}\oplus\{3\}$ |
| 140 | DT$(u,\ u,\ 0)$ | $\left(\frac{\sqrt{2}}{2},\ -\frac{\sqrt{2}}{2},\ 0\right)$, $(0,\ 0,\ -1)$ | $\{1\}\oplus\{2\}$ or $\{3\}\oplus\{4\}$ | $\left(\frac{\sqrt{2}}{2},\ -\frac{\sqrt{2}}{2},\ 0\right)$ | $\{1\}\oplus\{3\}$ or $\{2\}\oplus\{4\}$ |
| | | | | $(0,\ 0,\ -1)$ | $\{1\}\oplus\{4\}$ or $\{2\}\oplus\{3\}$ |
| 140 | SM$(u,\ 0,\ 0)$ | $(0,\ 1,\ 0)$, $(0,\ 0,\ -1)$ | $\{1\}\oplus\{2\}$ or $\{3\}\oplus\{4\}$ | $(0,\ 1,\ 0)$ | $\{1\}\oplus\{3\}$ or $\{2\}\oplus\{4\}$ |
| | | | | $(0,\ 0,\ -1)$ | $\{1\}\oplus\{4\}$ or $\{2\}\oplus\{3\}$ |
| 140 | W$\left(\frac{1}{2},\ \frac{1}{2},\ w\right)$ | $\left(-\frac{\sqrt{2}}{2},\ -\frac{\sqrt{2}}{2},\ 0\right)$, $\left(\frac{\sqrt{2}}{2},\ -\frac{\sqrt{2}}{2},\ 0\right)$ | $\{1\}\oplus\{2\}$ or $\{3\}\oplus\{4\}$ | $\left(-\frac{\sqrt{2}}{2},\ -\frac{\sqrt{2}}{2},\ 0\right)$ | $\{1\}\oplus\{3\}$ or $\{2\}\oplus\{4\}$ |
| | | | | $\left(\frac{\sqrt{2}}{2},\ -\frac{\sqrt{2}}{2},\ 0\right)$ | $\{1\}\oplus\{4\}$ or $\{2\}\oplus\{3\}$ |
| 140 | Y$(u,\ 1-u,\ 0)$ | $\left(-\frac{\sqrt{2}}{2},\ -\frac{\sqrt{2}}{2},\ 0\right)$, $(0,\ 0,\ -1)$ | $\{1\}\oplus\{2\}$ or $\{3\}\oplus\{4\}$ | $(0,\ 0,\ -1)$ | $\{1\}\oplus\{3\}$ or $\{2\}\oplus\{4\}$ |
| | | | | $\left(-\frac{\sqrt{2}}{2},\ -\frac{\sqrt{2}}{2},\ 0\right)$ | $\{1\}\oplus\{4\}$ or $\{2\}\oplus\{3\}$ |
| 141 | DT$(u,\ u,\ 0)$ | $\left(\frac{\sqrt{2}}{2},\ -\frac{\sqrt{2}}{2},\ 0\right)$, $(0,\ 0,\ -1)$ | $\{1\}\oplus\{2\}$ or $\{3\}\oplus\{4\}$ | $\left(\frac{\sqrt{2}}{2},\ -\frac{\sqrt{2}}{2},\ 0\right)$ | $\{1\}\oplus\{3\}$ or $\{2\}\oplus\{4\}$ |
| | | | | $(0,\ 0,\ -1)$ | $\{1\}\oplus\{4\}$ or $\{2\}\oplus\{3\}$ |
| 141 | SM$(u,\ 0,\ 0)$ | $(0,\ 1,\ 0)$, $(0,\ 0,\ -1)$ | $\{1\}\oplus\{2\}$ or $\{3\}\oplus\{4\}$ | $(0,\ 1,\ 0)$ | $\{1\}\oplus\{3\}$ or $\{2\}\oplus\{4\}$ |
| | | | | $(0,\ 0,\ -1)$ | $\{1\}\oplus\{4\}$ or $\{2\}\oplus\{3\}$ |
| 142 | DT$(u,\ u,\ 0)$ | $\left(-\frac{\sqrt{2}}{2},\ \frac{\sqrt{2}}{2},\ 0\right)$, $(0,\ 0,\ -1)$ | $\{1\}\oplus\{2\}$ or $\{3\}\oplus\{4\}$ | $\left(-\frac{\sqrt{2}}{2},\ \frac{\sqrt{2}}{2},\ 0\right)$ | $\{1\}\oplus\{3\}$ or $\{2\}\oplus\{4\}$ |
| | | | | $(0,\ 0,\ -1)$ | $\{1\}\oplus\{4\}$ or $\{2\}\oplus\{3\}$ |
| 142 | SM$(u,\ 0,\ 0)$ | $(0,\ -1,\ 0)$, $(0,\ 0,\ -1)$ | $\{1\}\oplus\{2\}$ or $\{3\}\oplus\{4\}$ | $(0,\ -1,\ 0)$ | $\{1\}\oplus\{3\}$ or $\{2\}\oplus\{4\}$ |
| | | | | $(0,\ 0,\ -1)$ | $\{1\}\oplus\{4\}$ or $\{2\}\oplus\{3\}$ |
| 183 | U$\left(\frac{1}{2},\ 0,\ w\right)$ | $\left(\frac{1}{2},\ -\frac{\sqrt{3}}{2},\ 0\right)$, $\left(-\frac{\sqrt{3}}{2},\ -\frac{1}{2},\ 0\right)$ | $1\oplus2$ or $3\oplus4$ | $\left(-\frac{\sqrt{3}}{2},\ -\frac{1}{2},\ 0\right)$ | $1\oplus3$ or $2\oplus4$ |
| | | | | $\left(\frac{1}{2},\ -\frac{\sqrt{3}}{2},\ 0\right)$ | $1\oplus4$ or $2\oplus3$ |
| 184 | U$\left(\frac{1}{2},\ 0,\ w\right)$ | $\left(\frac{1}{2},\ -\frac{\sqrt{3}}{2},\ 0\right)$, $\left(-\frac{\sqrt{3}}{2},\ -\frac{1}{2},\ 0\right)$ | $1\oplus2$ or $3\oplus4$ | $\left(-\frac{\sqrt{3}}{2},\ -\frac{1}{2},\ 0\right)$ | $1\oplus3$ or $2\oplus4$ |
| | | | | $\left(\frac{1}{2},\ -\frac{\sqrt{3}}{2},\ 0\right)$ | $1\oplus4$ or $2\oplus3$ |
| 185 | U$\left(\frac{1}{2},\ 0,\ w\right)$ | $\left(\frac{1}{2},\ -\frac{\sqrt{3}}{2},\ 0\right)$, $\left(-\frac{\sqrt{3}}{2},\ -\frac{1}{2},\ 0\right)$ | $1\oplus2$ or $3\oplus4$ | $\left(-\frac{\sqrt{3}}{2},\ -\frac{1}{2},\ 0\right)$ | $1\oplus3$ or $2\oplus4$ |
| | | | | $\left(\frac{1}{2},\ -\frac{\sqrt{3}}{2},\ 0\right)$ | $1\oplus4$ or $2\oplus3$ |
| 186 | U$\left(\frac{1}{2},\ 0,\ w\right)$ | $\left(\frac{1}{2},\ -\frac{\sqrt{3}}{2},\ 0\right)$, $\left(-\frac{\sqrt{3}}{2},\ -\frac{1}{2},\ 0\right)$ | $1\oplus2$ or $3\oplus4$ | $\left(-\frac{\sqrt{3}}{2},\ -\frac{1}{2},\ 0\right)$ | $1\oplus3$ or $2\oplus4$ |
| | | | | $\left(\frac{1}{2},\ -\frac{\sqrt{3}}{2},\ 0\right)$ | $1\oplus4$ or $2\oplus3$ |
| 187 | R$\left(u,\ 0,\ \frac{1}{2}\right)$ | $\left(-\frac{1}{2},\ \frac{\sqrt{3}}{2},\ 0\right)$, $(0,\ 0,\ 1)$ | $1\oplus2$ or $3\oplus4$ | $(0,\ 0,\ 1)$ | $1\oplus3$ or $2\oplus4$ |
| | | | | $\left(-\frac{1}{2},\ \frac{\sqrt{3}}{2},\ 0\right)$ | $1\oplus4$ or $2\oplus3$ |
| 187 | SM$(u,\ 0,\ 0)$ | $\left(-\frac{1}{2},\ \frac{\sqrt{3}}{2},\ 0\right)$, $(0,\ 0,\ 1)$ | $1\oplus2$ or $3\oplus4$ | $(0,\ 0,\ 1)$ | $1\oplus3$ or $2\oplus4$ |
| | | | | $\left(-\frac{1}{2},\ \frac{\sqrt{3}}{2},\ 0\right)$ | $1\oplus4$ or $2\oplus3$ |
| 188 | SM$(u,\ 0,\ 0)$ | $\left(-\frac{1}{2},\ \frac{\sqrt{3}}{2},\ 0\right)$, $(0,\ 0,\ 1)$ | $1\oplus2$ or $3\oplus4$ | $(0,\ 0,\ 1)$ | $1\oplus3$ or $2\oplus4$ |
| | | | | $\left(-\frac{1}{2},\ \frac{\sqrt{3}}{2},\ 0\right)$ | $1\oplus4$ or $2\oplus3$ |
| 189 | LD$(u,\ u,\ 0)$ | $(0,\ 0,\ 1)$, $\left(\frac{\sqrt{3}}{2},\ -\frac{1}{2},\ 0\right)$ | $1\oplus2$ or $3\oplus4$ | $(0,\ 0,\ 1)$ | $1\oplus3$ or $2\oplus4$ |
| | | | | $\left(\frac{\sqrt{3}}{2},\ -\frac{1}{2},\ 0\right)$ | $1\oplus4$ or $2\oplus3$ |
| 189 | Q$\left(u,\ u,\ \frac{1}{2}\right)$ | $\left(\frac{\sqrt{3}}{2},\ -\frac{1}{2},\ 0\right)$, $(0,\ 0,\ 1)$ | $1\oplus2$ or $3\oplus4$ | $(0,\ 0,\ 1)$ | $1\oplus3$ or $2\oplus4$ |
| | | | | $\left(\frac{\sqrt{3}}{2},\ -\frac{1}{2},\ 0\right)$ | $1\oplus4$ or $2\oplus3$ |
| 190 | LD$(u,\ u,\ 0)$ | $(0,\ 0,\ 1)$, $\left(\frac{\sqrt{3}}{2},\ -\frac{1}{2},\ 0\right)$ | $1\oplus2$ or $3\oplus4$ | $(0,\ 0,\ 1)$ | $1\oplus3$ or $2\oplus4$ |
| | | | | $\left(\frac{\sqrt{3}}{2},\ -\frac{1}{2},\ 0\right)$ | $1\oplus4$ or $2\oplus3$ |
| 191 | LD$(u,\ u,\ 0)$ | $(0,\ 0,\ 1)$, $\left(-\frac{\sqrt{3}}{2},\ \frac{1}{2},\ 0\right)$ | $\{1\}\oplus\{2\}$ or $\{3\}\oplus\{4\}$ | $(0,\ 0,\ 1)$ | $\{1\}\oplus\{3\}$ or $\{2\}\oplus\{4\}$ |
| | | | | $\left(-\frac{\sqrt{3}}{2},\ \frac{1}{2},\ 0\right)$ | $\{1\}\oplus\{4\}$ or $\{2\}\oplus\{3\}$ |

| SG | HSL | Location of nodal chain | Irreps of BC | Location of nodal loop | Irreps of BC |
|---|---|---|---|---|---|
| 191 | Q$\left(u,\ u,\ \frac{1}{2}\right)$ | $\left(-\frac{\sqrt{3}}{2},\ \frac{1}{2},\ 0\right)$, $(0,\ 0,\ 1)$ | $\{1\}\oplus\{2\}$ or $\{3\}\oplus\{4\}$ | $(0,\ 0,\ 1)$ | $\{1\}\oplus\{3\}$ or $\{2\}\oplus\{4\}$ |
| | | | | $\left(-\frac{\sqrt{3}}{2},\ \frac{1}{2},\ 0\right)$ | $\{1\}\oplus\{4\}$ or $\{2\}\oplus\{3\}$ |
| 191 | R$\left(u,\ 0,\ \frac{1}{2}\right)$ | $\left(\frac{1}{2},\ -\frac{\sqrt{3}}{2},\ 0\right)$, $(0,\ 0,\ 1)$ | $\{1\}\oplus\{2\}$ or $\{3\}\oplus\{4\}$ | $(0,\ 0,\ 1)$ | $\{1\}\oplus\{3\}$ or $\{2\}\oplus\{4\}$ |
| | | | | $\left(\frac{1}{2},\ -\frac{\sqrt{3}}{2},\ 0\right)$ | $\{1\}\oplus\{4\}$ or $\{2\}\oplus\{3\}$ |
| 191 | SM$(u,\ 0,\ 0)$ | $\left(\frac{1}{2},\ -\frac{\sqrt{3}}{2},\ 0\right)$, $(0,\ 0,\ 1)$ | $\{1\}\oplus\{2\}$ or $\{3\}\oplus\{4\}$ | $(0,\ 0,\ 1)$ | $\{1\}\oplus\{3\}$ or $\{2\}\oplus\{4\}$ |
| | | | | $\left(\frac{1}{2},\ -\frac{\sqrt{3}}{2},\ 0\right)$ | $\{1\}\oplus\{4\}$ or $\{2\}\oplus\{3\}$ |
| 191 | U$\left(\frac{1}{2},\ 0,\ w\right)$ | $\left(\frac{1}{2},\ -\frac{\sqrt{3}}{2},\ 0\right)$, $\left(-\frac{\sqrt{3}}{2},\ -\frac{1}{2},\ 0\right)$ | $\{1\}\oplus\{2\}$ or $\{3\}\oplus\{4\}$ | $\left(-\frac{\sqrt{3}}{2},\ -\frac{1}{2},\ 0\right)$ | $\{1\}\oplus\{3\}$ or $\{2\}\oplus\{4\}$ |
| | | | | $\left(\frac{1}{2},\ -\frac{\sqrt{3}}{2},\ 0\right)$ | $\{1\}\oplus\{4\}$ or $\{2\}\oplus\{3\}$ |
| 192 | LD$(u,\ u,\ 0)$ | $(0,\ 0,\ 1)$, $\left(-\frac{\sqrt{3}}{2},\ \frac{1}{2},\ 0\right)$ | $\{1\}\oplus\{2\}$ or $\{3\}\oplus\{4\}$ | $(0,\ 0,\ 1)$ | $\{1\}\oplus\{3\}$ or $\{2\}\oplus\{4\}$ |
| | | | | $\left(-\frac{\sqrt{3}}{2},\ \frac{1}{2},\ 0\right)$ | $\{1\}\oplus\{4\}$ or $\{2\}\oplus\{3\}$ |
| 192 | SM$(u,\ 0,\ 0)$ | $\left(\frac{1}{2},\ -\frac{\sqrt{3}}{2},\ 0\right)$, $(0,\ 0,\ 1)$ | $\{1\}\oplus\{2\}$ or $\{3\}\oplus\{4\}$ | $(0,\ 0,\ 1)$ | $\{1\}\oplus\{3\}$ or $\{2\}\oplus\{4\}$ |
| | | | | $\left(\frac{1}{2},\ -\frac{\sqrt{3}}{2},\ 0\right)$ | $\{1\}\oplus\{4\}$ or $\{2\}\oplus\{3\}$ |
| 192 | U$\left(\frac{1}{2},\ 0,\ w\right)$ | $\left(\frac{1}{2},\ -\frac{\sqrt{3}}{2},\ 0\right)$, $\left(-\frac{\sqrt{3}}{2},\ -\frac{1}{2},\ 0\right)$ | $\{1\}\oplus\{2\}$ or $\{3\}\oplus\{4\}$ | $\left(-\frac{\sqrt{3}}{2},\ -\frac{1}{2},\ 0\right)$ | $\{1\}\oplus\{3\}$ or $\{2\}\oplus\{4\}$ |
| | | | | $\left(\frac{1}{2},\ -\frac{\sqrt{3}}{2},\ 0\right)$ | $\{1\}\oplus\{4\}$ or $\{2\}\oplus\{3\}$ |
| 193 | LD$(u,\ u,\ 0)$ | $(0,\ 0,\ 1)$, $\left(-\frac{\sqrt{3}}{2},\ \frac{1}{2},\ 0\right)$ | $\{1\}\oplus\{2\}$ or $\{3\}\oplus\{4\}$ | $(0,\ 0,\ 1)$ | $\{1\}\oplus\{3\}$ or $\{2\}\oplus\{4\}$ |
| | | | | $\left(-\frac{\sqrt{3}}{2},\ \frac{1}{2},\ 0\right)$ | $\{1\}\oplus\{4\}$ or $\{2\}\oplus\{3\}$ |
| 193 | SM$(u,\ 0,\ 0)$ | $\left(\frac{1}{2},\ -\frac{\sqrt{3}}{2},\ 0\right)$, $(0,\ 0,\ 1)$ | $\{1\}\oplus\{2\}$ or $\{3\}\oplus\{4\}$ | $(0,\ 0,\ 1)$ | $\{1\}\oplus\{3\}$ or $\{2\}\oplus\{4\}$ |
| | | | | $\left(\frac{1}{2},\ -\frac{\sqrt{3}}{2},\ 0\right)$ | $\{1\}\oplus\{4\}$ or $\{2\}\oplus\{3\}$ |
| 193 | U$\left(\frac{1}{2},\ 0,\ w\right)$ | $\left(\frac{1}{2},\ -\frac{\sqrt{3}}{2},\ 0\right)$, $\left(-\frac{\sqrt{3}}{2},\ -\frac{1}{2},\ 0\right)$ | $\{1\}\oplus\{2\}$ or $\{3\}\oplus\{4\}$ | $\left(-\frac{\sqrt{3}}{2},\ -\frac{1}{2},\ 0\right)$ | $\{1\}\oplus\{3\}$ or $\{2\}\oplus\{4\}$ |
| | | | | $\left(\frac{1}{2},\ -\frac{\sqrt{3}}{2},\ 0\right)$ | $\{1\}\oplus\{4\}$ or $\{2\}\oplus\{3\}$ |
| 194 | LD$(u,\ u,\ 0)$ | $(0,\ 0,\ 1)$, $\left(-\frac{\sqrt{3}}{2},\ \frac{1}{2},\ 0\right)$ | $\{1\}\oplus\{2\}$ or $\{3\}\oplus\{4\}$ | $(0,\ 0,\ 1)$ | $\{1\}\oplus\{3\}$ or $\{2\}\oplus\{4\}$ |
| | | | | $\left(-\frac{\sqrt{3}}{2},\ \frac{1}{2},\ 0\right)$ | $\{1\}\oplus\{4\}$ or $\{2\}\oplus\{3\}$ |
| 194 | SM$(u,\ 0,\ 0)$ | $\left(\frac{1}{2},\ -\frac{\sqrt{3}}{2},\ 0\right)$, $(0,\ 0,\ 1)$ | $\{1\}\oplus\{2\}$ or $\{3\}\oplus\{4\}$ | $(0,\ 0,\ 1)$ | $\{1\}\oplus\{3\}$ or $\{2\}\oplus\{4\}$ |
| | | | | $\left(\frac{1}{2},\ -\frac{\sqrt{3}}{2},\ 0\right)$ | $\{1\}\oplus\{4\}$ or $\{2\}\oplus\{3\}$ |
| 194 | U$\left(\frac{1}{2},\ 0,\ w\right)$ | $\left(\frac{1}{2},\ -\frac{\sqrt{3}}{2},\ 0\right)$, $\left(-\frac{\sqrt{3}}{2},\ -\frac{1}{2},\ 0\right)$ | $\{1\}\oplus\{2\}$ or $\{3\}\oplus\{4\}$ | $\left(-\frac{\sqrt{3}}{2},\ -\frac{1}{2},\ 0\right)$ | $\{1\}\oplus\{3\}$ or $\{2\}\oplus\{4\}$ |
| | | | | $\left(\frac{1}{2},\ -\frac{\sqrt{3}}{2},\ 0\right)$ | $\{1\}\oplus\{4\}$ or $\{2\}\oplus\{3\}$ |
| 200 | DT$(0,\ v,\ 0)$ | $(0,\ 0,\ 1)$, $(1,\ 0,\ 0)$ | $\{1\}\oplus\{2\}$ or $\{3\}\oplus\{4\}$ | $(0,\ 0,\ 1)$ | $\{1\}\oplus\{3\}$ or $\{2\}\oplus\{4\}$ |
| | | | | $(1,\ 0,\ 0)$ | $\{1\}\oplus\{4\}$ or $\{2\}\oplus\{3\}$ |
| 200 | T$\left(\frac{1}{2},\ \frac{1}{2},\ w\right)$ | $(0,\ -1,\ 0)$, $(-1,\ 0,\ 0)$ | $\{1\}\oplus\{2\}$ or $\{3\}\oplus\{4\}$ | $(-1,\ 0,\ 0)$ | $\{1\}\oplus\{3\}$ or $\{2\}\oplus\{4\}$ |
| | | | | $(0,\ -1,\ 0)$ | $\{1\}\oplus\{4\}$ or $\{2\}\oplus\{3\}$ |
| 200 | ZA$\left(\frac{1}{2},\ u,\ 0\right)$ | $(0,\ 0,\ 1)$, $(-1,\ 0,\ 0)$ | $\{1\}\oplus\{2\}$ or $\{3\}\oplus\{4\}$ | $(-1,\ 0,\ 0)$ | $\{1\}\oplus\{3\}$ or $\{2\}\oplus\{4\}$ |
| | | | | $(0,\ 0,\ 1)$ | $\{1\}\oplus\{4\}$ or $\{2\}\oplus\{3\}$ |
| 200 | Z$\left(u,\ \frac{1}{2},\ 0\right)$ | $(0,\ 0,\ 1)$, $(0,\ -1,\ 0)$ | $\{1\}\oplus\{2\}$ or $\{3\}\oplus\{4\}$ | $(0,\ -1,\ 0)$ | $\{1\}\oplus\{3\}$ or $\{2\}\oplus\{4\}$ |
| | | | | $(0,\ 0,\ 1)$ | $\{1\}\oplus\{4\}$ or $\{2\}\oplus\{3\}$ |
| 201 | DT$(0,\ v,\ 0)$ | $(0,\ 0,\ 1)$, $(1,\ 0,\ 0)$ | $\{1\}\oplus\{2\}$ or $\{3\}\oplus\{4\}$ | $(0,\ 0,\ 1)$ | $\{1\}\oplus\{3\}$ or $\{2\}\oplus\{4\}$ |
| | | | | $(1,\ 0,\ 0)$ | $\{1\}\oplus\{4\}$ or $\{2\}\oplus\{3\}$ |
| 201 | T$\left(\frac{1}{2},\ \frac{1}{2},\ w\right)$ | $(0,\ -1,\ 0)$, $(-1,\ 0,\ 0)$ | $\{1\}\oplus\{2\}$ or $\{3\}\oplus\{4\}$ | $(-1,\ 0,\ 0)$ | $\{1\}\oplus\{3\}$ or $\{2\}\oplus\{4\}$ |
| | | | | $(0,\ -1,\ 0)$ | $\{1\}\oplus\{4\}$ or $\{2\}\oplus\{3\}$ |
| 202 | DT$(0,\ v,\ 0)$ | $(0,\ 0,\ -1)$, $(-1,\ 0,\ 0)$ | $\{1\}\oplus\{2\}$ or $\{3\}\oplus\{4\}$ | $(0,\ 0,\ -1)$ | $\{1\}\oplus\{3\}$ or $\{2\}\oplus\{4\}$ |
| | | | | $(-1,\ 0,\ 0)$ | $\{1\}\oplus\{4\}$ or $\{2\}\oplus\{3\}$ |

| SG | HSL | Location of nodal chain | Irreps of BC | Location of nodal loop | Irreps of BC |
|---|---|---|---|---|---|
| 202 | V$(u,\ 1,\ 0)$ | $(0,\ 0,\ -1)$, $(0,\ -1,\ 0)$ | $\{1\}\oplus\{2\}$ or $\{3\}\oplus\{4\}$ | $(0,\ -1,\ 0)$ | $\{1\}\oplus\{3\}$ or $\{2\}\oplus\{4\}$ |
| | | | | $(0,\ 0,\ -1)$ | $\{1\}\oplus\{4\}$ or $\{2\}\oplus\{3\}$ |
| 203 | DT$(0,\ v,\ 0)$ | $(0,\ 0,\ -1)$, $(-1,\ 0,\ 0)$ | $\{1\}\oplus\{2\}$ or $\{3\}\oplus\{4\}$ | $(0,\ 0,\ -1)$ | $\{1\}\oplus\{3\}$ or $\{2\}\oplus\{4\}$ |
| | | | | $(-1,\ 0,\ 0)$ | $\{1\}\oplus\{4\}$ or $\{2\}\oplus\{3\}$ |
| 204 | DT$(0,\ v,\ 0)$ | $(0,\ 0,\ -1)$, $(-1,\ 0,\ 0)$ | $\{1\}\oplus\{2\}$ or $\{3\}\oplus\{4\}$ | $(0,\ 0,\ -1)$ | $\{1\}\oplus\{3\}$ or $\{2\}\oplus\{4\}$ |
| | | | | $(-1,\ 0,\ 0)$ | $\{1\}\oplus\{4\}$ or $\{2\}\oplus\{3\}$ |
| 205 | DT$(0,\ v,\ 0)$ | $(0,\ 0,\ 1)$, $(1,\ 0,\ 0)$ | $\{1\}\oplus\{2\}$ or $\{3\}\oplus\{4\}$ | $(0,\ 0,\ 1)$ | $\{1\}\oplus\{3\}$ or $\{2\}\oplus\{4\}$ |
| | | | | $(1,\ 0,\ 0)$ | $\{1\}\oplus\{4\}$ or $\{2\}\oplus\{3\}$ |
| 206 | DT$(0,\ v,\ 0)$ | $(0,\ 0,\ -1)$, $(-1,\ 0,\ 0)$ | $\{1\}\oplus\{2\}$ or $\{3\}\oplus\{4\}$ | $(0,\ 0,\ -1)$ | $\{1\}\oplus\{3\}$ or $\{2\}\oplus\{4\}$ |
| | | | | $(-1,\ 0,\ 0)$ | $\{1\}\oplus\{4\}$ or $\{2\}\oplus\{3\}$ |
| 217 | D$\left(\frac{1}{2},\ \frac{1}{2},\ w\right)$ | $\left(-\frac{\sqrt{2}}{2},\ \frac{\sqrt{2}}{2},\ 0\right)$, $\left(-\frac{\sqrt{2}}{2},\ -\frac{\sqrt{2}}{2},\ 0\right)$ | $1\oplus2$ or $3\oplus4$ | $\left(-\frac{\sqrt{2}}{2},\ -\frac{\sqrt{2}}{2},\ 0\right)$ | $1\oplus3$ or $2\oplus4$ |
| | | | | $\left(-\frac{\sqrt{2}}{2},\ \frac{\sqrt{2}}{2},\ 0\right)$ | $1\oplus4$ or $2\oplus3$ |
| 221 | S$\left(u,\ \frac{1}{2},\ u\right)$ | $\left(-\frac{\sqrt{2}}{2},\ 0,\ \frac{\sqrt{2}}{2}\right)$, $(0,\ -1,\ 0)$ | $\{1\}\oplus\{2\}$ or $\{3\}\oplus\{4\}$ | $\left(-\frac{\sqrt{2}}{2},\ 0,\ \frac{\sqrt{2}}{2}\right)$ | $\{1\}\oplus\{3\}$ or $\{2\}\oplus\{4\}$ |
| | | | | $(0,\ -1,\ 0)$ | $\{1\}\oplus\{4\}$ or $\{2\}\oplus\{3\}$ |
| 221 | SM$(u,\ u,\ 0)$ | $\left(\frac{\sqrt{2}}{2},\ -\frac{\sqrt{2}}{2},\ 0\right)$, $(0,\ 0,\ 1)$ | $\{1\}\oplus\{2\}$ or $\{3\}\oplus\{4\}$ | $\left(\frac{\sqrt{2}}{2},\ -\frac{\sqrt{2}}{2},\ 0\right)$ | $\{1\}\oplus\{3\}$ or $\{2\}\oplus\{4\}$ |
| | | | | $(0,\ 0,\ 1)$ | $\{1\}\oplus\{4\}$ or $\{2\}\oplus\{3\}$ |
| 221 | Z$\left(u,\ \frac{1}{2},\ 0\right)$ | $(0,\ 0,\ 1)$, $(0,\ -1,\ 0)$ | $\{1\}\oplus\{2\}$ or $\{3\}\oplus\{4\}$ | $(0,\ -1,\ 0)$ | $\{1\}\oplus\{3\}$ or $\{2\}\oplus\{4\}$ |
| | | | | $(0,\ 0,\ 1)$ | $\{1\}\oplus\{4\}$ or $\{2\}\oplus\{3\}$ |
| 222 | SM$(u,\ u,\ 0)$ | $\left(\frac{\sqrt{2}}{2},\ -\frac{\sqrt{2}}{2},\ 0\right)$, $(0,\ 0,\ 1)$ | $\{1\}\oplus\{2\}$ or $\{3\}\oplus\{4\}$ | $\left(\frac{\sqrt{2}}{2},\ -\frac{\sqrt{2}}{2},\ 0\right)$ | $\{1\}\oplus\{3\}$ or $\{2\}\oplus\{4\}$ |
| | | | | $(0,\ 0,\ 1)$ | $\{1\}\oplus\{4\}$ or $\{2\}\oplus\{3\}$ |
| 223 | SM$(u,\ u,\ 0)$ | $\left(\frac{\sqrt{2}}{2},\ -\frac{\sqrt{2}}{2},\ 0\right)$, $(0,\ 0,\ 1)$ | $\{1\}\oplus\{2\}$ or $\{3\}\oplus\{4\}$ | $\left(\frac{\sqrt{2}}{2},\ -\frac{\sqrt{2}}{2},\ 0\right)$ | $\{1\}\oplus\{3\}$ or $\{2\}\oplus\{4\}$ |
| | | | | $(0,\ 0,\ 1)$ | $\{1\}\oplus\{4\}$ or $\{2\}\oplus\{3\}$ |
| 223 | Z$\left(u,\ \frac{1}{2},\ 0\right)$ | $(0,\ 0,\ 1)$, $(0,\ -1,\ 0)$ | $\{1\}\oplus\{2\}$ or $\{3\}\oplus\{4\}$ | $(0,\ -1,\ 0)$ | $\{1\}\oplus\{3\}$ or $\{2\}\oplus\{4\}$ |
| | | | | $(0,\ 0,\ 1)$ | $\{1\}\oplus\{4\}$ or $\{2\}\oplus\{3\}$ |
| 224 | S$\left(u,\ \frac{1}{2},\ u\right)$ | $\left(-\frac{\sqrt{2}}{2},\ 0,\ \frac{\sqrt{2}}{2}\right)$, $(0,\ -1,\ 0)$ | $\{1\}\oplus\{3\}$ or $\{2\}\oplus\{4\}$ | $(0,\ -1,\ 0)$ | $\{1\}\oplus\{2\}$ or $\{3\}\oplus\{4\}$ |
| | | | | $\left(-\frac{\sqrt{2}}{2},\ 0,\ \frac{\sqrt{2}}{2}\right)$ | $\{1\}\oplus\{4\}$ or $\{2\}\oplus\{3\}$ |
| 224 | SM$(u,\ u,\ 0)$ | $\left(\frac{\sqrt{2}}{2},\ -\frac{\sqrt{2}}{2},\ 0\right)$, $(0,\ 0,\ 1)$ | $\{1\}\oplus\{2\}$ or $\{3\}\oplus\{4\}$ | $\left(\frac{\sqrt{2}}{2},\ -\frac{\sqrt{2}}{2},\ 0\right)$ | $\{1\}\oplus\{3\}$ or $\{2\}\oplus\{4\}$ |
| | | | | $(0,\ 0,\ 1)$ | $\{1\}\oplus\{4\}$ or $\{2\}\oplus\{3\}$ |
| 225 | SM$(u,\ u,\ 0)$ | $(0,\ 0,\ -1)$, $\left(-\frac{\sqrt{2}}{2},\ \frac{\sqrt{2}}{2},\ 0\right)$ | $\{1\}\oplus\{2\}$ or $\{3\}\oplus\{4\}$ | $\left(-\frac{\sqrt{2}}{2},\ \frac{\sqrt{2}}{2},\ 0\right)$ | $\{1\}\oplus\{3\}$ or $\{2\}\oplus\{4\}$ |
| | | | | $(0,\ 0,\ -1)$ | $\{1\}\oplus\{4\}$ or $\{2\}\oplus\{3\}$ |
| 225 | V$(u,\ 1,\ 0)$ | $(0,\ 0,\ -1)$, $(0,\ -1,\ 0)$ | $\{1\}\oplus\{2\}$ or $\{3\}\oplus\{4\}$ | $(0,\ -1,\ 0)$ | $\{1\}\oplus\{3\}$ or $\{2\}\oplus\{4\}$ |
| | | | | $(0,\ 0,\ -1)$ | $\{1\}\oplus\{4\}$ or $\{2\}\oplus\{3\}$ |
| 226 | SM$(u,\ u,\ 0)$ | $(0,\ 0,\ -1)$, $\left(-\frac{\sqrt{2}}{2},\ \frac{\sqrt{2}}{2},\ 0\right)$ | $\{1\}\oplus\{2\}$ or $\{3\}\oplus\{4\}$ | $\left(-\frac{\sqrt{2}}{2},\ \frac{\sqrt{2}}{2},\ 0\right)$ | $\{1\}\oplus\{3\}$ or $\{2\}\oplus\{4\}$ |
| | | | | $(0,\ 0,\ -1)$ | $\{1\}\oplus\{4\}$ or $\{2\}\oplus\{3\}$ |
| 226 | V$(u,\ 1,\ 0)$ | $(0,\ 0,\ -1)$, $(0,\ -1,\ 0)$ | $\{1\}\oplus\{2\}$ or $\{3\}\oplus\{4\}$ | $(0,\ -1,\ 0)$ | $\{1\}\oplus\{3\}$ or $\{2\}\oplus\{4\}$ |
| | | | | $(0,\ 0,\ -1)$ | $\{1\}\oplus\{4\}$ or $\{2\}\oplus\{3\}$ |
| 227 | SM$(u,\ u,\ 0)$ | $(0,\ 0,\ -1)$, $\left(-\frac{\sqrt{2}}{2},\ \frac{\sqrt{2}}{2},\ 0\right)$ | $\{1\}\oplus\{2\}$ or $\{3\}\oplus\{4\}$ | $\left(-\frac{\sqrt{2}}{2},\ \frac{\sqrt{2}}{2},\ 0\right)$ | $\{1\}\oplus\{3\}$ or $\{2\}\oplus\{4\}$ |
| | | | | $(0,\ 0,\ -1)$ | $\{1\}\oplus\{4\}$ or $\{2\}\oplus\{3\}$ |
| 228 | SM$(u,\ u,\ 0)$ | $(0,\ 0,\ -1)$, $\left(-\frac{\sqrt{2}}{2},\ \frac{\sqrt{2}}{2},\ 0\right)$ | $\{1\}\oplus\{2\}$ or $\{3\}\oplus\{4\}$ | $\left(-\frac{\sqrt{2}}{2},\ \frac{\sqrt{2}}{2},\ 0\right)$ | $\{1\}\oplus\{3\}$ or $\{2\}\oplus\{4\}$ |
| | | | | $(0,\ 0,\ -1)$ | $\{1\}\oplus\{4\}$ or $\{2\}\oplus\{3\}$ |

| SG | HSL | Location of nodal chain | Irreps of BC | Location of nodal loop | Irreps of BC |
|---|---|---|---|---|---|
| 229 | D$\left(\frac{1}{2},\ \frac{1}{2},\ w\right)$ | $\left(-\frac{\sqrt{2}}{2},\ \frac{\sqrt{2}}{2},\ 0\right)$, $\left(-\frac{\sqrt{2}}{2},\ -\frac{\sqrt{2}}{2},\ 0\right)$ | $\{1\}\oplus\{2\}$ or $\{3\}\oplus\{4\}$ | $\left(-\frac{\sqrt{2}}{2},\ -\frac{\sqrt{2}}{2},\ 0\right)$ | $\{1\}\oplus\{3\}$ or $\{2\}\oplus\{4\}$ |
| | | | | $\left(-\frac{\sqrt{2}}{2},\ \frac{\sqrt{2}}{2},\ 0\right)$ | $\{1\}\oplus\{4\}$ or $\{2\}\oplus\{3\}$ |
| 229 | G$(u+1,\ 1-u,\ 1)$ | $\left(-\frac{\sqrt{2}}{2},\ -\frac{\sqrt{2}}{2},\ 0\right)$, $(0,\ 0,\ -1)$ | $\{1\}\oplus\{2\}$ or $\{3\}\oplus\{4\}$ | $(0,\ 0,\ -1)$ | $\{1\}\oplus\{3\}$ or $\{2\}\oplus\{4\}$ |
| | | | | $\left(-\frac{\sqrt{2}}{2},\ -\frac{\sqrt{2}}{2},\ 0\right)$ | $\{1\}\oplus\{4\}$ or $\{2\}\oplus\{3\}$ |
| 229 | SM$(u,\ u,\ 0)$ | $\left(-\frac{\sqrt{2}}{2},\ \frac{\sqrt{2}}{2},\ 0\right)$, $(0,\ 0,\ -1)$ | $\{1\}\oplus\{2\}$ or $\{3\}\oplus\{4\}$ | $\left(-\frac{\sqrt{2}}{2},\ \frac{\sqrt{2}}{2},\ 0\right)$ | $\{1\}\oplus\{3\}$ or $\{2\}\oplus\{4\}$ |
| | | | | $(0,\ 0,\ -1)$ | $\{1\}\oplus\{4\}$ or $\{2\}\oplus\{3\}$ |
| 230 | SM$(u,\ u,\ 0)$ | $\left(-\frac{\sqrt{2}}{2},\ \frac{\sqrt{2}}{2},\ 0\right)$, $(0,\ 0,\ -1)$ | $\{1\}\oplus\{2\}$ or $\{3\}\oplus\{4\}$ | $\left(-\frac{\sqrt{2}}{2},\ \frac{\sqrt{2}}{2},\ 0\right)$ | $\{1\}\oplus\{3\}$ or $\{2\}\oplus\{4\}$ |
| | | | | $(0,\ 0,\ -1)$ | $\{1\}\oplus\{4\}$ or $\{2\}\oplus\{3\}$ |

Table S15: Inter-chain structure

| SG | HSL | Location of nodal chain | Irreps of BC |
|---|---|---|---|
| 25 | G$(\frac{1}{2},\ 0,\ w)$ | $(0,\ -1,\ 0),\ (-1,\ 0,\ 0)$ | 1⊕2 or 3⊕4 |
| 25 | H$(0,\ \frac{1}{2},\ w)$ | $(-1,\ 0,\ 0),\ (0,\ -1,\ 0)$ | 1⊕2 or 3⊕4 |
| 25 | LD$(0,\ 0,\ w)$ | $(-1,\ 0,\ 0),\ (0,\ -1,\ 0)$ | 1⊕2 or 3⊕4 |
| 25 | Q$(\frac{1}{2},\ \frac{1}{2},\ w)$ | $(-1,\ 0,\ 0),\ (0,\ -1,\ 0)$ | 1⊕2 or 3⊕4 |
| 26 | G$(\frac{1}{2},\ 0,\ w)$ | $(0,\ -1,\ 0),\ (-1,\ 0,\ 0)$ | 1⊕2 or 3⊕4 |
| 26 | H$(0,\ \frac{1}{2},\ w)$ | $(-1,\ 0,\ 0),\ (0,\ -1,\ 0)$ | 1⊕2 or 3⊕4 |
| 26 | LD$(0,\ 0,\ w)$ | $(-1,\ 0,\ 0),\ (0,\ -1,\ 0)$ | 1⊕2 or 3⊕4 |
| 26 | Q$(\frac{1}{2},\ \frac{1}{2},\ w)$ | $(-1,\ 0,\ 0),\ (0,\ -1,\ 0)$ | 1⊕2 or 3⊕4 |
| 27 | G$(\frac{1}{2},\ 0,\ w)$ | $(0,\ -1,\ 0),\ (-1,\ 0,\ 0)$ | 1⊕2 or 3⊕4 |
| 27 | H$(0,\ \frac{1}{2},\ w)$ | $(-1,\ 0,\ 0),\ (0,\ -1,\ 0)$ | 1⊕2 or 3⊕4 |
| 27 | LD$(0,\ 0,\ w)$ | $(-1,\ 0,\ 0),\ (0,\ -1,\ 0)$ | 1⊕2 or 3⊕4 |
| 27 | Q$(\frac{1}{2},\ \frac{1}{2},\ w)$ | $(-1,\ 0,\ 0),\ (0,\ -1,\ 0)$ | 1⊕2 or 3⊕4 |
| 28 | H$(0,\ \frac{1}{2},\ w)$ | $(-1,\ 0,\ 0),\ (0,\ 1,\ 0)$ | 1⊕2 or 3⊕4 |
| 28 | LD$(0,\ 0,\ w)$ | $(0,\ 1,\ 0),\ (-1,\ 0,\ 0)$ | 1⊕2 or 3⊕4 |
| 29 | H$(0,\ \frac{1}{2},\ w)$ | $(-1,\ 0,\ 0),\ (0,\ 1,\ 0)$ | 1⊕2 or 3⊕4 |
| 29 | LD$(0,\ 0,\ w)$ | $(0,\ 1,\ 0),\ (-1,\ 0,\ 0)$ | 1⊕2 or 3⊕4 |
| 30 | G$(\frac{1}{2},\ 0,\ w)$ | $(0,\ -1,\ 0),\ (-1,\ 0,\ 0)$ | 1⊕2 or 3⊕4 |
| 30 | LD$(0,\ 0,\ w)$ | $(-1,\ 0,\ 0),\ (0,\ -1,\ 0)$ | 1⊕2 or 3⊕4 |
| 31 | H$(0,\ \frac{1}{2},\ w)$ | $(-1,\ 0,\ 0),\ (0,\ 1,\ 0)$ | 1⊕2 or 3⊕4 |
| 31 | LD$(0,\ 0,\ w)$ | $(0,\ 1,\ 0),\ (-1,\ 0,\ 0)$ | 1⊕2 or 3⊕4 |
| 32 | LD$(0,\ 0,\ w)$ | $(-1,\ 0,\ 0),\ (0,\ -1,\ 0)$ | 1⊕2 or 3⊕4 |
| 32 | Q$(\frac{1}{2},\ \frac{1}{2},\ w)$ | $(-1,\ 0,\ 0),\ (0,\ -1,\ 0)$ | 1⊕3 or 2⊕4 |
| 33 | LD$(0,\ 0,\ w)$ | $(0,\ 1,\ 0),\ (-1,\ 0,\ 0)$ | 1⊕2 or 3⊕4 |
| 33 | Q$(\frac{1}{2},\ \frac{1}{2},\ w)$ | $(0,\ 1,\ 0),\ (-1,\ 0,\ 0)$ | 1⊕3 or 2⊕4 |
| 34 | LD$(0,\ 0,\ w)$ | $(-1,\ 0,\ 0),\ (0,\ -1,\ 0)$ | 1⊕2 or 3⊕4 |
| 34 | Q$(\frac{1}{2},\ \frac{1}{2},\ w)$ | $(-1,\ 0,\ 0),\ (0,\ -1,\ 0)$ | 1⊕3 or 2⊕4 |
| 35 | H$(1,\ 0,\ w)$ | $(0,\ -1,\ 0),\ (-1,\ 0,\ 0)$ | 1⊕2 or 3⊕4 |
| 35 | LD$(0,\ 0,\ w)$ | $(0,\ -1,\ 0),\ (-1,\ 0,\ 0)$ | 1⊕2 or 3⊕4 |
| 36 | H$(1,\ 0,\ w)$ | $(-1,\ 0,\ 0),\ (0,\ 1,\ 0)$ | 1⊕2 or 3⊕4 |
| 36 | LD$(0,\ 0,\ w)$ | $(-1,\ 0,\ 0),\ (0,\ 1,\ 0)$ | 1⊕2 or 3⊕4 |
| 37 | H$(1,\ 0,\ w)$ | $(0,\ -1,\ 0),\ (-1,\ 0,\ 0)$ | 1⊕2 or 3⊕4 |
| 37 | LD$(0,\ 0,\ w)$ | $(0,\ -1,\ 0),\ (-1,\ 0,\ 0)$ | 1⊕2 or 3⊕4 |
| 38 | A$(\frac{1}{2},\ 0,\ w)$ | $(0,\ -1,\ 0),\ (1,\ 0,\ 0)$ | 1⊕2 or 3⊕4 |
| 38 | SM$(0,\ 0,\ w)$ | $(0,\ -1,\ 0),\ (1,\ 0,\ 0)$ | 1⊕2 or 3⊕4 |
| 39 | A$(\frac{1}{2},\ 0,\ w)$ | $(0,\ -1,\ 0),\ (1,\ 0,\ 0)$ | 1⊕2 or 3⊕4 |
| 39 | SM$(0,\ 0,\ w)$ | $(0,\ -1,\ 0),\ (1,\ 0,\ 0)$ | 1⊕2 or 3⊕4 |
| 40 | SM$(0,\ 0,\ w)$ | $(0,\ -1,\ 0),\ (1,\ 0,\ 0)$ | 1⊕2 or 3⊕4 |
| 41 | SM$(0,\ 0,\ w)$ | $(0,\ -1,\ 0),\ (1,\ 0,\ 0)$ | 1⊕2 or 3⊕4 |
| 42 | H$(0,\ 1,\ w)$ | $(0,\ 1,\ 0),\ (1,\ 0,\ 0)$ | 1⊕2 or 3⊕4 |
| 42 | LD$(0,\ 0,\ w)$ | $(0,\ 1,\ 0),\ (1,\ 0,\ 0)$ | 1⊕2 or 3⊕4 |
| 43 | LD$(0,\ 0,\ w)$ | $(0,\ 1,\ 0),\ (1,\ 0,\ 0)$ | 1⊕2 or 3⊕4 |

| SG | HSL | Location of nodal chain | Irreps of BC |
|---|---|---|---|
| 44 | LD$(0,\ 0,\ w)$ | $(0,\ -1,\ 0)$, $(1,\ 0,\ 0)$ | 1⊕2 or 3⊕4 |
| 45 | LD$(0,\ 0,\ w)$ | $(0,\ -1,\ 0)$, $(1,\ 0,\ 0)$ | 1⊕2 or 3⊕4 |
| 46 | LD$(0,\ 0,\ w)$ | $(-1,\ 0,\ 0)$, $(0,\ -1,\ 0)$ | 1⊕2 or 3⊕4 |
| 47 | A$\left(u,\ 0,\ \frac{1}{2}\right)$ | $(0,\ -1,\ 0)$, $(0,\ 0,\ 1)$ | {1}⊕{2} or {3}⊕{4} |
| 47 | B$\left(0,\ v,\ \frac{1}{2}\right)$ | $(-1,\ 0,\ 0)$, $(0,\ 0,\ 1)$ | {1}⊕{2} or {3}⊕{4} |
| 47 | C$\left(u,\ \frac{1}{2},\ 0\right)$ | $(0,\ 0,\ 1)$, $(0,\ -1,\ 0)$ | {1}⊕{2} or {3}⊕{4} |
| 47 | D$\left(\frac{1}{2},\ v,\ 0\right)$ | $(0,\ 0,\ 1)$, $(-1,\ 0,\ 0)$ | {1}⊕{2} or {3}⊕{4} |
| 47 | DT$(0,\ v,\ 0)$ | $(0,\ 0,\ 1)$, $(-1,\ 0,\ 0)$ | {1}⊕{2} or {3}⊕{4} |
| 47 | E$\left(u,\ \frac{1}{2},\ \frac{1}{2}\right)$ | $(0,\ 0,\ 1)$, $(0,\ -1,\ 0)$ | {1}⊕{2} or {3}⊕{4} |
| 47 | G$\left(\frac{1}{2},\ 0,\ w\right)$ | $(0,\ -1,\ 0)$, $(-1,\ 0,\ 0)$ | {1}⊕{2} or {3}⊕{4} |
| 47 | H$\left(0,\ \frac{1}{2},\ w\right)$ | $(-1,\ 0,\ 0)$, $(0,\ -1,\ 0)$ | {1}⊕{2} or {3}⊕{4} |
| 47 | LD$(0,\ 0,\ w)$ | $(-1,\ 0,\ 0)$, $(0,\ -1,\ 0)$ | {1}⊕{2} or {3}⊕{4} |
| 47 | P$\left(\frac{1}{2},\ v,\ \frac{1}{2}\right)$ | $(0,\ 0,\ 1)$, $(-1,\ 0,\ 0)$ | {1}⊕{2} or {3}⊕{4} |
| 47 | Q$\left(\frac{1}{2},\ \frac{1}{2},\ w\right)$ | $(-1,\ 0,\ 0)$, $(0,\ -1,\ 0)$ | {1}⊕{2} or {3}⊕{4} |
| 47 | SM$(u,\ 0,\ 0)$ | $(0,\ 0,\ 1)$, $(0,\ -1,\ 0)$ | {1}⊕{2} or {3}⊕{4} |
| 48 | DT$(0,\ v,\ 0)$ | $(0,\ 0,\ 1)$, $(-1,\ 0,\ 0)$ | {1}⊕{2} or {3}⊕{4} |
| 48 | E$\left(u,\ \frac{1}{2},\ \frac{1}{2}\right)$ | $(0,\ 0,\ 1)$, $(0,\ -1,\ 0)$ | {1}⊕{2} or {3}⊕{4} |
| 48 | LD$(0,\ 0,\ w)$ | $(-1,\ 0,\ 0)$, $(0,\ -1,\ 0)$ | {1}⊕{2} or {3}⊕{4} |
| 48 | P$\left(\frac{1}{2},\ v,\ \frac{1}{2}\right)$ | $(0,\ 0,\ 1)$, $(-1,\ 0,\ 0)$ | {1}⊕{2} or {3}⊕{4} |
| 48 | Q$\left(\frac{1}{2},\ \frac{1}{2},\ w\right)$ | $(-1,\ 0,\ 0)$, $(0,\ -1,\ 0)$ | {1}⊕{2} or {3}⊕{4} |
| 48 | SM$(u,\ 0,\ 0)$ | $(0,\ 0,\ 1)$, $(0,\ -1,\ 0)$ | {1}⊕{2} or {3}⊕{4} |
| 49 | C$\left(u,\ \frac{1}{2},\ 0\right)$ | $(0,\ 0,\ 1)$, $(0,\ -1,\ 0)$ | {1}⊕{2} or {3}⊕{4} |
| 49 | D$\left(\frac{1}{2},\ v,\ 0\right)$ | $(0,\ 0,\ 1)$, $(-1,\ 0,\ 0)$ | {1}⊕{2} or {3}⊕{4} |
| 49 | DT$(0,\ v,\ 0)$ | $(0,\ 0,\ 1)$, $(-1,\ 0,\ 0)$ | {1}⊕{2} or {3}⊕{4} |
| 49 | G$\left(\frac{1}{2},\ 0,\ w\right)$ | $(0,\ -1,\ 0)$, $(-1,\ 0,\ 0)$ | {1}⊕{2} or {3}⊕{4} |
| 49 | H$\left(0,\ \frac{1}{2},\ w\right)$ | $(-1,\ 0,\ 0)$, $(0,\ -1,\ 0)$ | {1}⊕{2} or {3}⊕{4} |
| 49 | LD$(0,\ 0,\ w)$ | $(-1,\ 0,\ 0)$, $(0,\ -1,\ 0)$ | {1}⊕{2} or {3}⊕{4} |
| 49 | Q$\left(\frac{1}{2},\ \frac{1}{2},\ w\right)$ | $(-1,\ 0,\ 0)$, $(0,\ -1,\ 0)$ | {1}⊕{2} or {3}⊕{4} |
| 49 | SM$(u,\ 0,\ 0)$ | $(0,\ 0,\ 1)$, $(0,\ -1,\ 0)$ | {1}⊕{2} or {3}⊕{4} |
| 50 | A$\left(u,\ 0,\ \frac{1}{2}\right)$ | $(0,\ -1,\ 0)$, $(0,\ 0,\ 1)$ | {1}⊕{2} or {3}⊕{4} |
| 50 | B$\left(0,\ v,\ \frac{1}{2}\right)$ | $(-1,\ 0,\ 0)$, $(0,\ 0,\ 1)$ | {1}⊕{2} or {3}⊕{4} |
| 50 | DT$(0,\ v,\ 0)$ | $(0,\ 0,\ 1)$, $(-1,\ 0,\ 0)$ | {1}⊕{2} or {3}⊕{4} |
| 50 | LD$(0,\ 0,\ w)$ | $(-1,\ 0,\ 0)$, $(0,\ -1,\ 0)$ | {1}⊕{2} or {3}⊕{4} |
| 50 | Q$\left(\frac{1}{2},\ \frac{1}{2},\ w\right)$ | $(-1,\ 0,\ 0)$, $(0,\ -1,\ 0)$ | {1}⊕{2} or {3}⊕{4} |
| 50 | SM$(u,\ 0,\ 0)$ | $(0,\ 0,\ 1)$, $(0,\ -1,\ 0)$ | {1}⊕{2} or {3}⊕{4} |
| 51 | A$\left(u,\ 0,\ \frac{1}{2}\right)$ | $(0,\ -1,\ 0)$, $(0,\ 0,\ -1)$ | {1}⊕{2} or {3}⊕{4} |
| 51 | B$\left(0,\ v,\ \frac{1}{2}\right)$ | $(-1,\ 0,\ 0)$, $(0,\ 0,\ -1)$ | {1}⊕{2} or {3}⊕{4} |
| 51 | C$\left(u,\ \frac{1}{2},\ 0\right)$ | $(0,\ 0,\ -1)$, $(0,\ -1,\ 0)$ | {1}⊕{2} or {3}⊕{4} |
| 51 | DT$(0,\ v,\ 0)$ | $(-1,\ 0,\ 0)$, $(0,\ 0,\ -1)$ | {1}⊕{2} or {3}⊕{4} |
| 51 | E$\left(u,\ \frac{1}{2},\ \frac{1}{2}\right)$ | $(0,\ 0,\ -1)$, $(0,\ -1,\ 0)$ | {1}⊕{2} or {3}⊕{4} |
| 51 | H$\left(0,\ \frac{1}{2},\ w\right)$ | $(-1,\ 0,\ 0)$, $(0,\ -1,\ 0)$ | {1}⊕{2} or {3}⊕{4} |

| SG | HSL | Location of nodal chain | Irreps of BC |
|---|---|---|---|
| 51 | LD$(0,\ 0,\ w)$ | $(-1,\ 0,\ 0)$, $(0,\ -1,\ 0)$ | $\{1\}\oplus\{2\}$ or $\{3\}\oplus\{4\}$ |
| 51 | SM$(u,\ 0,\ 0)$ | $(0,\ 0,\ -1)$, $(0,\ -1,\ 0)$ | $\{1\}\oplus\{2\}$ or $\{3\}\oplus\{4\}$ |
| 52 | DT$(0,\ v,\ 0)$ | $(-1,\ 0,\ 0)$, $(0,\ 0,\ 1)$ | $\{1\}\oplus\{2\}$ or $\{3\}\oplus\{4\}$ |
| 52 | LD$(0,\ 0,\ w)$ | $(0,\ 1,\ 0)$, $(-1,\ 0,\ 0)$ | $\{1\}\oplus\{2\}$ or $\{3\}\oplus\{4\}$ |
| 52 | P$\left(\frac{1}{2},\ v,\ \frac{1}{2}\right)$ | $(-1,\ 0,\ 0)$, $(0,\ 0,\ 1)$ | $\{1\}\oplus\{2\}$ or $\{3\}\oplus\{4\}$ |
| 52 | SM$(u,\ 0,\ 0)$ | $(0,\ 1,\ 0)$, $(0,\ 0,\ 1)$ | $\{1\}\oplus\{2\}$ or $\{3\}\oplus\{4\}$ |
| 53 | C$\left(u,\ \frac{1}{2},\ 0\right)$ | $(0,\ 0,\ 1)$, $(0,\ 1,\ 0)$ | $\{1\}\oplus\{2\}$ or $\{3\}\oplus\{4\}$ |
| 53 | DT$(0,\ v,\ 0)$ | $(0,\ 0,\ 1)$, $(-1,\ 0,\ 0)$ | $\{1\}\oplus\{2\}$ or $\{3\}\oplus\{4\}$ |
| 53 | H$\left(0,\ \frac{1}{2},\ w\right)$ | $(-1,\ 0,\ 0)$, $(0,\ 1,\ 0)$ | $\{1\}\oplus\{2\}$ or $\{3\}\oplus\{4\}$ |
| 53 | LD$(0,\ 0,\ w)$ | $(0,\ 1,\ 0)$, $(-1,\ 0,\ 0)$ | $\{1\}\oplus\{2\}$ or $\{3\}\oplus\{4\}$ |
| 53 | SM$(u,\ 0,\ 0)$ | $(0,\ 0,\ 1)$, $(0,\ 1,\ 0)$ | $\{1\}\oplus\{2\}$ or $\{3\}\oplus\{4\}$ |
| 54 | C$\left(u,\ \frac{1}{2},\ 0\right)$ | $(0,\ 0,\ -1)$, $(0,\ -1,\ 0)$ | $\{1\}\oplus\{2\}$ or $\{3\}\oplus\{4\}$ |
| 54 | DT$(0,\ v,\ 0)$ | $(-1,\ 0,\ 0)$, $(0,\ 0,\ -1)$ | $\{1\}\oplus\{2\}$ or $\{3\}\oplus\{4\}$ |
| 54 | H$\left(0,\ \frac{1}{2},\ w\right)$ | $(-1,\ 0,\ 0)$, $(0,\ -1,\ 0)$ | $\{1\}\oplus\{2\}$ or $\{3\}\oplus\{4\}$ |
| 54 | LD$(0,\ 0,\ w)$ | $(-1,\ 0,\ 0)$, $(0,\ -1,\ 0)$ | $\{1\}\oplus\{2\}$ or $\{3\}\oplus\{4\}$ |
| 54 | SM$(u,\ 0,\ 0)$ | $(0,\ 0,\ -1)$, $(0,\ -1,\ 0)$ | $\{1\}\oplus\{2\}$ or $\{3\}\oplus\{4\}$ |
| 55 | A$\left(u,\ 0,\ \frac{1}{2}\right)$ | $(0,\ -1,\ 0)$, $(0,\ 0,\ 1)$ | $\{1\}\oplus\{2\}$ or $\{3\}\oplus\{4\}$ |
| 55 | B$\left(0,\ v,\ \frac{1}{2}\right)$ | $(-1,\ 0,\ 0)$, $(0,\ 0,\ 1)$ | $\{1\}\oplus\{2\}$ or $\{3\}\oplus\{4\}$ |
| 55 | DT$(0,\ v,\ 0)$ | $(0,\ 0,\ 1)$, $(-1,\ 0,\ 0)$ | $\{1\}\oplus\{2\}$ or $\{3\}\oplus\{4\}$ |
| 55 | LD$(0,\ 0,\ w)$ | $(-1,\ 0,\ 0)$, $(0,\ -1,\ 0)$ | $\{1\}\oplus\{2\}$ or $\{3\}\oplus\{4\}$ |
| 55 | SM$(u,\ 0,\ 0)$ | $(0,\ 0,\ 1)$, $(0,\ -1,\ 0)$ | $\{1\}\oplus\{2\}$ or $\{3\}\oplus\{4\}$ |
| 56 | DT$(0,\ v,\ 0)$ | $(0,\ 0,\ 1)$, $(-1,\ 0,\ 0)$ | $\{1\}\oplus\{2\}$ or $\{3\}\oplus\{4\}$ |
| 56 | LD$(0,\ 0,\ w)$ | $(-1,\ 0,\ 0)$, $(0,\ -1,\ 0)$ | $\{1\}\oplus\{2\}$ or $\{3\}\oplus\{4\}$ |
| 56 | SM$(u,\ 0,\ 0)$ | $(0,\ 0,\ 1)$, $(0,\ -1,\ 0)$ | $\{1\}\oplus\{2\}$ or $\{3\}\oplus\{4\}$ |
| 57 | D$\left(\frac{1}{2},\ v,\ 0\right)$ | $(0,\ 0,\ -1)$, $(1,\ 0,\ 0)$ | $\{1\}\oplus\{2\}$ or $\{3\}\oplus\{4\}$ |
| 57 | DT$(0,\ v,\ 0)$ | $(1,\ 0,\ 0)$, $(0,\ 0,\ -1)$ | $\{1\}\oplus\{2\}$ or $\{3\}\oplus\{4\}$ |
| 57 | G$\left(\frac{1}{2},\ 0,\ w\right)$ | $(0,\ -1,\ 0)$, $(1,\ 0,\ 0)$ | $\{1\}\oplus\{2\}$ or $\{3\}\oplus\{4\}$ |
| 57 | LD$(0,\ 0,\ w)$ | $(1,\ 0,\ 0)$, $(0,\ -1,\ 0)$ | $\{1\}\oplus\{2\}$ or $\{3\}\oplus\{4\}$ |
| 57 | SM$(u,\ 0,\ 0)$ | $(0,\ -1,\ 0)$, $(0,\ 0,\ -1)$ | $\{1\}\oplus\{2\}$ or $\{3\}\oplus\{4\}$ |
| 58 | DT$(0,\ v,\ 0)$ | $(0,\ 0,\ 1)$, $(-1,\ 0,\ 0)$ | $\{1\}\oplus\{2\}$ or $\{3\}\oplus\{4\}$ |
| 58 | LD$(0,\ 0,\ w)$ | $(-1,\ 0,\ 0)$, $(0,\ -1,\ 0)$ | $\{1\}\oplus\{2\}$ or $\{3\}\oplus\{4\}$ |
| 58 | SM$(u,\ 0,\ 0)$ | $(0,\ 0,\ 1)$, $(0,\ -1,\ 0)$ | $\{1\}\oplus\{2\}$ or $\{3\}\oplus\{4\}$ |
| 59 | A$\left(u,\ 0,\ \frac{1}{2}\right)$ | $(0,\ -1,\ 0)$, $(0,\ 0,\ 1)$ | $\{1\}\oplus\{2\}$ or $\{3\}\oplus\{4\}$ |
| 59 | B$\left(0,\ v,\ \frac{1}{2}\right)$ | $(-1,\ 0,\ 0)$, $(0,\ 0,\ 1)$ | $\{1\}\oplus\{2\}$ or $\{3\}\oplus\{4\}$ |
| 59 | DT$(0,\ v,\ 0)$ | $(0,\ 0,\ 1)$, $(-1,\ 0,\ 0)$ | $\{1\}\oplus\{2\}$ or $\{3\}\oplus\{4\}$ |
| 59 | LD$(0,\ 0,\ w)$ | $(-1,\ 0,\ 0)$, $(0,\ -1,\ 0)$ | $\{1\}\oplus\{2\}$ or $\{3\}\oplus\{4\}$ |
| 59 | SM$(u,\ 0,\ 0)$ | $(0,\ 0,\ 1)$, $(0,\ -1,\ 0)$ | $\{1\}\oplus\{2\}$ or $\{3\}\oplus\{4\}$ |
| 60 | DT$(0,\ v,\ 0)$ | $(-1,\ 0,\ 0)$, $(0,\ 0,\ 1)$ | $\{1\}\oplus\{2\}$ or $\{3\}\oplus\{4\}$ |
| 60 | LD$(0,\ 0,\ w)$ | $(0,\ 1,\ 0)$, $(-1,\ 0,\ 0)$ | $\{1\}\oplus\{2\}$ or $\{3\}\oplus\{4\}$ |
| 60 | SM$(u,\ 0,\ 0)$ | $(0,\ 1,\ 0)$, $(0,\ 0,\ 1)$ | $\{1\}\oplus\{2\}$ or $\{3\}\oplus\{4\}$ |
| 61 | DT$(0,\ v,\ 0)$ | $(-1,\ 0,\ 0)$, $(0,\ 0,\ 1)$ | $\{1\}\oplus\{2\}$ or $\{3\}\oplus\{4\}$ |

| SG | HSL | Location of nodal chain | Irreps of BC |
|---|---|---|---|
| 61 | LD$(0,\ 0,\ w)$ | $(0,\ 1,\ 0)$, $(-1,\ 0,\ 0)$ | $\{1\}\oplus\{2\}$ or $\{3\}\oplus\{4\}$ |
| 61 | SM$(u,\ 0,\ 0)$ | $(0,\ 1,\ 0)$, $(0,\ 0,\ 1)$ | $\{1\}\oplus\{2\}$ or $\{3\}\oplus\{4\}$ |
| 62 | DT$(0,\ v,\ 0)$ | $(0,\ 0,\ 1)$, $(-1,\ 0,\ 0)$ | $\{1\}\oplus\{2\}$ or $\{3\}\oplus\{4\}$ |
| 62 | LD$(0,\ 0,\ w)$ | $(-1,\ 0,\ 0)$, $(0,\ -1,\ 0)$ | $\{1\}\oplus\{2\}$ or $\{3\}\oplus\{4\}$ |
| 62 | SM$(u,\ 0,\ 0)$ | $(0,\ 0,\ 1)$, $(0,\ -1,\ 0)$ | $\{1\}\oplus\{2\}$ or $\{3\}\oplus\{4\}$ |
| 63 | DT$(0,\ v,\ 0)$ | $(-1,\ 0,\ 0)$, $(0,\ 0,\ 1)$ | $\{1\}\oplus\{2\}$ or $\{3\}\oplus\{4\}$ |
| 63 | H$(1,\ 0,\ w)$ | $(0,\ -1,\ 0)$, $(-1,\ 0,\ 0)$ | $\{1\}\oplus\{2\}$ or $\{3\}\oplus\{4\}$ |
| 63 | LD$(0,\ 0,\ w)$ | $(0,\ -1,\ 0)$, $(-1,\ 0,\ 0)$ | $\{1\}\oplus\{2\}$ or $\{3\}\oplus\{4\}$ |
| 63 | SM$(u,\ 0,\ 0)$ | $(0,\ -1,\ 0)$, $(0,\ 0,\ 1)$ | $\{1\}\oplus\{2\}$ or $\{3\}\oplus\{4\}$ |
| 64 | DT$(0,\ v,\ 0)$ | $(-1,\ 0,\ 0)$, $(0,\ 0,\ 1)$ | $\{1\}\oplus\{2\}$ or $\{3\}\oplus\{4\}$ |
| 64 | H$(1,\ 0,\ w)$ | $(0,\ -1,\ 0)$, $(-1,\ 0,\ 0)$ | $\{1\}\oplus\{2\}$ or $\{3\}\oplus\{4\}$ |
| 64 | LD$(0,\ 0,\ w)$ | $(0,\ -1,\ 0)$, $(-1,\ 0,\ 0)$ | $\{1\}\oplus\{2\}$ or $\{3\}\oplus\{4\}$ |
| 64 | SM$(u,\ 0,\ 0)$ | $(0,\ -1,\ 0)$, $(0,\ 0,\ 1)$ | $\{1\}\oplus\{2\}$ or $\{3\}\oplus\{4\}$ |
| 65 | A$\left(u,\ 0,\ \frac{1}{2}\right)$ | $(0,\ -1,\ 0)$, $(0,\ 0,\ 1)$ | $\{1\}\oplus\{2\}$ or $\{3\}\oplus\{4\}$ |
| 65 | B$\left(0,\ v,\ \frac{1}{2}\right)$ | $(-1,\ 0,\ 0)$, $(0,\ 0,\ 1)$ | $\{1\}\oplus\{2\}$ or $\{3\}\oplus\{4\}$ |
| 65 | DT$(0,\ v,\ 0)$ | $(-1,\ 0,\ 0)$, $(0,\ 0,\ 1)$ | $\{1\}\oplus\{2\}$ or $\{3\}\oplus\{4\}$ |
| 65 | H$(1,\ 0,\ w)$ | $(0,\ -1,\ 0)$, $(-1,\ 0,\ 0)$ | $\{1\}\oplus\{2\}$ or $\{3\}\oplus\{4\}$ |
| 65 | LD$(0,\ 0,\ w)$ | $(0,\ -1,\ 0)$, $(-1,\ 0,\ 0)$ | $\{1\}\oplus\{2\}$ or $\{3\}\oplus\{4\}$ |
| 65 | SM$(u,\ 0,\ 0)$ | $(0,\ -1,\ 0)$, $(0,\ 0,\ 1)$ | $\{1\}\oplus\{2\}$ or $\{3\}\oplus\{4\}$ |
| 66 | DT$(0,\ v,\ 0)$ | $(-1,\ 0,\ 0)$, $(0,\ 0,\ 1)$ | $\{1\}\oplus\{2\}$ or $\{3\}\oplus\{4\}$ |
| 66 | H$(1,\ 0,\ w)$ | $(0,\ -1,\ 0)$, $(-1,\ 0,\ 0)$ | $\{1\}\oplus\{2\}$ or $\{3\}\oplus\{4\}$ |
| 66 | LD$(0,\ 0,\ w)$ | $(0,\ -1,\ 0)$, $(-1,\ 0,\ 0)$ | $\{1\}\oplus\{2\}$ or $\{3\}\oplus\{4\}$ |
| 66 | SM$(u,\ 0,\ 0)$ | $(0,\ -1,\ 0)$, $(0,\ 0,\ 1)$ | $\{1\}\oplus\{2\}$ or $\{3\}\oplus\{4\}$ |
| 67 | A$\left(u,\ 0,\ \frac{1}{2}\right)$ | $(0,\ -1,\ 0)$, $(0,\ 0,\ 1)$ | $\{1\}\oplus\{2\}$ or $\{3\}\oplus\{4\}$ |
| 67 | B$\left(0,\ v,\ \frac{1}{2}\right)$ | $(-1,\ 0,\ 0)$, $(0,\ 0,\ 1)$ | $\{1\}\oplus\{2\}$ or $\{3\}\oplus\{4\}$ |
| 67 | DT$(0,\ v,\ 0)$ | $(-1,\ 0,\ 0)$, $(0,\ 0,\ 1)$ | $\{1\}\oplus\{2\}$ or $\{3\}\oplus\{4\}$ |
| 67 | H$(1,\ 0,\ w)$ | $(0,\ -1,\ 0)$, $(-1,\ 0,\ 0)$ | $\{1\}\oplus\{2\}$ or $\{3\}\oplus\{4\}$ |
| 67 | LD$(0,\ 0,\ w)$ | $(0,\ -1,\ 0)$, $(-1,\ 0,\ 0)$ | $\{1\}\oplus\{2\}$ or $\{3\}\oplus\{4\}$ |
| 67 | SM$(u,\ 0,\ 0)$ | $(0,\ -1,\ 0)$, $(0,\ 0,\ 1)$ | $\{1\}\oplus\{2\}$ or $\{3\}\oplus\{4\}$ |
| 68 | DT$(0,\ v,\ 0)$ | $(-1,\ 0,\ 0)$, $(0,\ 0,\ 1)$ | $\{1\}\oplus\{2\}$ or $\{3\}\oplus\{4\}$ |
| 68 | H$(1,\ 0,\ w)$ | $(0,\ -1,\ 0)$, $(-1,\ 0,\ 0)$ | $\{1\}\oplus\{2\}$ or $\{3\}\oplus\{4\}$ |
| 68 | LD$(0,\ 0,\ w)$ | $(0,\ -1,\ 0)$, $(-1,\ 0,\ 0)$ | $\{1\}\oplus\{2\}$ or $\{3\}\oplus\{4\}$ |
| 68 | SM$(u,\ 0,\ 0)$ | $(0,\ -1,\ 0)$, $(0,\ 0,\ 1)$ | $\{1\}\oplus\{2\}$ or $\{3\}\oplus\{4\}$ |
| 69 | A$(u,\ 0,\ 1)$ | $(0,\ 0,\ -1)$, $(0,\ 1,\ 0)$ | $\{1\}\oplus\{2\}$ or $\{3\}\oplus\{4\}$ |
| 69 | B$(0,\ v,\ 1)$ | $(0,\ 0,\ -1)$, $(1,\ 0,\ 0)$ | $\{1\}\oplus\{2\}$ or $\{3\}\oplus\{4\}$ |
| 69 | DT$(0,\ v,\ 0)$ | $(0,\ 0,\ -1)$, $(1,\ 0,\ 0)$ | $\{1\}\oplus\{2\}$ or $\{3\}\oplus\{4\}$ |
| 69 | H$(0,\ 1,\ w)$ | $(0,\ 1,\ 0)$, $(1,\ 0,\ 0)$ | $\{1\}\oplus\{2\}$ or $\{3\}\oplus\{4\}$ |
| 69 | LD$(0,\ 0,\ w)$ | $(0,\ 1,\ 0)$, $(1,\ 0,\ 0)$ | $\{1\}\oplus\{2\}$ or $\{3\}\oplus\{4\}$ |
| 69 | SM$(u,\ 0,\ 0)$ | $(0,\ 0,\ -1)$, $(0,\ 1,\ 0)$ | $\{1\}\oplus\{2\}$ or $\{3\}\oplus\{4\}$ |
| 70 | DT$(0,\ v,\ 0)$ | $(0,\ 0,\ -1)$, $(1,\ 0,\ 0)$ | $\{1\}\oplus\{2\}$ or $\{3\}\oplus\{4\}$ |
| 70 | LD$(0,\ 0,\ w)$ | $(0,\ -1,\ 0)$, $(1,\ 0,\ 0)$ | $\{1\}\oplus\{2\}$ or $\{3\}\oplus\{4\}$ |

| SG | HSL | Location of nodal chain | Irreps of BC |
|---|---|---|---|
| 70 | SM$(u,\ 0,\ 0)$ | $(0,\ -1,\ 0)$, $(0,\ 0,\ -1)$ | $\{1\}\oplus\{2\}$ or $\{3\}\oplus\{4\}$ |
| 71 | DT$(0,\ v,\ 0)$ | $(0,\ 0,\ -1)$, $(1,\ 0,\ 0)$ | $\{1\}\oplus\{2\}$ or $\{3\}\oplus\{4\}$ |
| 71 | LD$(0,\ 0,\ w)$ | $(0,\ -1,\ 0)$, $(1,\ 0,\ 0)$ | $\{1\}\oplus\{2\}$ or $\{3\}\oplus\{4\}$ |
| 71 | SM$(u,\ 0,\ 0)$ | $(0,\ 0,\ -1)$, $(0,\ -1,\ 0)$ | $\{1\}\oplus\{2\}$ or $\{3\}\oplus\{4\}$ |
| 72 | DT$(0,\ v,\ 0)$ | $(0,\ 0,\ -1)$, $(1,\ 0,\ 0)$ | $\{1\}\oplus\{2\}$ or $\{3\}\oplus\{4\}$ |
| 72 | LD$(0,\ 0,\ w)$ | $(0,\ -1,\ 0)$, $(1,\ 0,\ 0)$ | $\{1\}\oplus\{2\}$ or $\{3\}\oplus\{4\}$ |
| 72 | SM$(u,\ 0,\ 0)$ | $(0,\ 0,\ -1)$, $(0,\ -1,\ 0)$ | $\{1\}\oplus\{2\}$ or $\{3\}\oplus\{4\}$ |
| 73 | DT$(0,\ v,\ 0)$ | $(0,\ 0,\ -1)$, $(1,\ 0,\ 0)$ | $\{1\}\oplus\{2\}$ or $\{3\}\oplus\{4\}$ |
| 73 | LD$(0,\ 0,\ w)$ | $(0,\ -1,\ 0)$, $(1,\ 0,\ 0)$ | $\{1\}\oplus\{2\}$ or $\{3\}\oplus\{4\}$ |
| 73 | SM$(u,\ 0,\ 0)$ | $(0,\ 0,\ -1)$, $(0,\ -1,\ 0)$ | $\{1\}\oplus\{2\}$ or $\{3\}\oplus\{4\}$ |
| 74 | DT$(0,\ v,\ 0)$ | $(0,\ 0,\ -1)$, $(1,\ 0,\ 0)$ | $\{1\}\oplus\{2\}$ or $\{3\}\oplus\{4\}$ |
| 74 | LD$(0,\ 0,\ w)$ | $(0,\ -1,\ 0)$, $(1,\ 0,\ 0)$ | $\{1\}\oplus\{2\}$ or $\{3\}\oplus\{4\}$ |
| 74 | SM$(u,\ 0,\ 0)$ | $(0,\ 0,\ -1)$, $(0,\ -1,\ 0)$ | $\{1\}\oplus\{2\}$ or $\{3\}\oplus\{4\}$ |
| 99 | LD$(0,\ 0,\ w)$ | $(1,\ 0,\ 0)$, $(0,\ 1,\ 0)$, $\left(\frac{\sqrt{2}}{2},\ -\frac{\sqrt{2}}{2},\ 0\right)$, $\left(\frac{\sqrt{2}}{2},\ \frac{\sqrt{2}}{2},\ 0\right)$<br>$\left(\frac{\sqrt{2}}{2},\ -\frac{\sqrt{2}}{2},\ 0\right)$, $\left(\frac{\sqrt{2}}{2},\ \frac{\sqrt{2}}{2},\ 0\right)$<br>$(1,\ 0,\ 0)$, $(0,\ 1,\ 0)$ | $1\oplus2$ or $3\oplus4$<br>$1\oplus3$ or $2\oplus4$<br>$1\oplus4$ or $2\oplus3$ |
| 99 | V$\left(\frac{1}{2},\ \frac{1}{2},\ w\right)$ | $\left(\frac{\sqrt{2}}{2},\ -\frac{\sqrt{2}}{2},\ 0\right)$, $\left(\frac{\sqrt{2}}{2},\ \frac{\sqrt{2}}{2},\ 0\right)$, $(0,\ -1,\ 0)$, $(1,\ 0,\ 0)$<br>$\left(\frac{\sqrt{2}}{2},\ -\frac{\sqrt{2}}{2},\ 0\right)$, $\left(\frac{\sqrt{2}}{2},\ \frac{\sqrt{2}}{2},\ 0\right)$<br>$(0,\ -1,\ 0)$, $(1,\ 0,\ 0)$ | $1\oplus2$ or $3\oplus4$<br>$1\oplus3$ or $2\oplus4$<br>$1\oplus4$ or $2\oplus3$ |
| 99 | W$\left(0,\ \frac{1}{2},\ w\right)$ | $(1,\ 0,\ 0)$, $(0,\ -1,\ 0)$ | $1\oplus2$ or $3\oplus4$ |
| 100 | LD$(0,\ 0,\ w)$ | $(1,\ 0,\ 0)$, $(0,\ 1,\ 0)$, $\left(\frac{\sqrt{2}}{2},\ -\frac{\sqrt{2}}{2},\ 0\right)$, $\left(\frac{\sqrt{2}}{2},\ \frac{\sqrt{2}}{2},\ 0\right)$<br>$\left(\frac{\sqrt{2}}{2},\ -\frac{\sqrt{2}}{2},\ 0\right)$, $\left(\frac{\sqrt{2}}{2},\ \frac{\sqrt{2}}{2},\ 0\right)$<br>$(1,\ 0,\ 0)$, $(0,\ 1,\ 0)$ | $1\oplus2$ or $3\oplus4$<br>$1\oplus3$ or $2\oplus4$<br>$1\oplus4$ or $2\oplus3$ |
| 100 | V$\left(\frac{1}{2},\ \frac{1}{2},\ w\right)$ | $(0,\ -1,\ 0)$, $(1,\ 0,\ 0)$<br>$\left(\frac{\sqrt{2}}{2},\ -\frac{\sqrt{2}}{2},\ 0\right)$, $\left(\frac{\sqrt{2}}{2},\ \frac{\sqrt{2}}{2},\ 0\right)$<br>$\left(\frac{\sqrt{2}}{2},\ -\frac{\sqrt{2}}{2},\ 0\right)$, $\left(\frac{\sqrt{2}}{2},\ \frac{\sqrt{2}}{2},\ 0\right)$, $(0,\ -1,\ 0)$, $(1,\ 0,\ 0)$ | $1\oplus2$ or $3\oplus4$<br>$1\oplus3$ or $2\oplus4$<br>$1\oplus4$ or $2\oplus3$ |
| 101 | LD$(0,\ 0,\ w)$ | $(1,\ 0,\ 0)$, $(0,\ 1,\ 0)$, $\left(\frac{\sqrt{2}}{2},\ -\frac{\sqrt{2}}{2},\ 0\right)$, $\left(\frac{\sqrt{2}}{2},\ \frac{\sqrt{2}}{2},\ 0\right)$<br>$\left(\frac{\sqrt{2}}{2},\ -\frac{\sqrt{2}}{2},\ 0\right)$, $\left(\frac{\sqrt{2}}{2},\ \frac{\sqrt{2}}{2},\ 0\right)$<br>$(1,\ 0,\ 0)$, $(0,\ 1,\ 0)$ | $1\oplus2$ or $3\oplus4$<br>$1\oplus3$ or $2\oplus4$<br>$1\oplus4$ or $2\oplus3$ |
| 101 | V$\left(\frac{1}{2},\ \frac{1}{2},\ w\right)$ | $\left(\frac{\sqrt{2}}{2},\ -\frac{\sqrt{2}}{2},\ 0\right)$, $\left(\frac{\sqrt{2}}{2},\ \frac{\sqrt{2}}{2},\ 0\right)$, $(0,\ -1,\ 0)$, $(1,\ 0,\ 0)$<br>$\left(\frac{\sqrt{2}}{2},\ -\frac{\sqrt{2}}{2},\ 0\right)$, $\left(\frac{\sqrt{2}}{2},\ \frac{\sqrt{2}}{2},\ 0\right)$<br>$(0,\ -1,\ 0)$, $(1,\ 0,\ 0)$ | $1\oplus2$ or $3\oplus4$<br>$1\oplus3$ or $2\oplus4$<br>$1\oplus4$ or $2\oplus3$ |
| 101 | W$\left(0,\ \frac{1}{2},\ w\right)$ | $(1,\ 0,\ 0)$, $(0,\ -1,\ 0)$ | $1\oplus2$ or $3\oplus4$ |
| 102 | LD$(0,\ 0,\ w)$ | $(1,\ 0,\ 0)$, $(0,\ 1,\ 0)$, $\left(\frac{\sqrt{2}}{2},\ -\frac{\sqrt{2}}{2},\ 0\right)$, $\left(\frac{\sqrt{2}}{2},\ \frac{\sqrt{2}}{2},\ 0\right)$<br>$\left(\frac{\sqrt{2}}{2},\ -\frac{\sqrt{2}}{2},\ 0\right)$, $\left(\frac{\sqrt{2}}{2},\ \frac{\sqrt{2}}{2},\ 0\right)$<br>$(1,\ 0,\ 0)$, $(0,\ 1,\ 0)$ | $1\oplus2$ or $3\oplus4$<br>$1\oplus3$ or $2\oplus4$<br>$1\oplus4$ or $2\oplus3$ |
| 102 | V$\left(\frac{1}{2},\ \frac{1}{2},\ w\right)$ | $(0,\ -1,\ 0)$, $(1,\ 0,\ 0)$<br>$\left(\frac{\sqrt{2}}{2},\ -\frac{\sqrt{2}}{2},\ 0\right)$, $\left(\frac{\sqrt{2}}{2},\ \frac{\sqrt{2}}{2},\ 0\right)$<br>$\left(\frac{\sqrt{2}}{2},\ -\frac{\sqrt{2}}{2},\ 0\right)$, $\left(\frac{\sqrt{2}}{2},\ \frac{\sqrt{2}}{2},\ 0\right)$, $(0,\ -1,\ 0)$, $(1,\ 0,\ 0)$ | $1\oplus2$ or $3\oplus4$<br>$1\oplus3$ or $2\oplus4$<br>$1\oplus4$ or $2\oplus3$ |
| 103 | LD$(0,\ 0,\ w)$ | $(1,\ 0,\ 0)$, $(0,\ 1,\ 0)$, $\left(\frac{\sqrt{2}}{2},\ -\frac{\sqrt{2}}{2},\ 0\right)$, $\left(\frac{\sqrt{2}}{2},\ \frac{\sqrt{2}}{2},\ 0\right)$<br>$\left(\frac{\sqrt{2}}{2},\ -\frac{\sqrt{2}}{2},\ 0\right)$, $\left(\frac{\sqrt{2}}{2},\ \frac{\sqrt{2}}{2},\ 0\right)$<br>$(1,\ 0,\ 0)$, $(0,\ 1,\ 0)$ | $1\oplus2$ or $3\oplus4$<br>$1\oplus3$ or $2\oplus4$<br>$1\oplus4$ or $2\oplus3$ |

| SG | HSL | Location of nodal chain | Irreps of BC |
|---|---|---|---|
| 103 | V$(\frac{1}{2},\ \frac{1}{2},\ w)$ | $\left(\frac{\sqrt{2}}{2},\ -\frac{\sqrt{2}}{2},\ 0\right),\ \left(\frac{\sqrt{2}}{2},\ \frac{\sqrt{2}}{2},\ 0\right),\ (0,\ -1,\ 0),\ (1,\ 0,\ 0)$<br>$\left(\frac{\sqrt{2}}{2},\ -\frac{\sqrt{2}}{2},\ 0\right),\ \left(\frac{\sqrt{2}}{2},\ \frac{\sqrt{2}}{2},\ 0\right)$<br>$(0,\ -1,\ 0),\ (1,\ 0,\ 0)$ | 1⊕2 or 3⊕4<br>1⊕3 or 2⊕4<br>1⊕4 or 2⊕3 |
| 103 | W$(0,\ \frac{1}{2},\ w)$ | $(1,\ 0,\ 0),\ (0,\ -1,\ 0)$ | 1⊕2 or 3⊕4 |
| 104 | LD$(0,\ 0,\ w)$ | $(1,\ 0,\ 0),\ (0,\ 1,\ 0),\ \left(\frac{\sqrt{2}}{2},\ -\frac{\sqrt{2}}{2},\ 0\right),\ \left(\frac{\sqrt{2}}{2},\ \frac{\sqrt{2}}{2},\ 0\right)$<br>$\left(\frac{\sqrt{2}}{2},\ -\frac{\sqrt{2}}{2},\ 0\right),\ \left(\frac{\sqrt{2}}{2},\ \frac{\sqrt{2}}{2},\ 0\right)$<br>$(1,\ 0,\ 0),\ (0,\ 1,\ 0)$ | 1⊕2 or 3⊕4<br>1⊕3 or 2⊕4<br>1⊕4 or 2⊕3 |
| 104 | V$(\frac{1}{2},\ \frac{1}{2},\ w)$ | $(0,\ -1,\ 0),\ (1,\ 0,\ 0)$<br>$\left(\frac{\sqrt{2}}{2},\ -\frac{\sqrt{2}}{2},\ 0\right),\ \left(\frac{\sqrt{2}}{2},\ \frac{\sqrt{2}}{2},\ 0\right)$<br>$\left(\frac{\sqrt{2}}{2},\ -\frac{\sqrt{2}}{2},\ 0\right),\ \left(\frac{\sqrt{2}}{2},\ \frac{\sqrt{2}}{2},\ 0\right),\ (0,\ -1,\ 0),\ (1,\ 0,\ 0)$ | 1⊕2 or 3⊕4<br>1⊕3 or 2⊕4<br>1⊕4 or 2⊕3 |
| 105 | LD$(0,\ 0,\ w)$ | $(1,\ 0,\ 0),\ (0,\ 1,\ 0),\ \left(\frac{\sqrt{2}}{2},\ -\frac{\sqrt{2}}{2},\ 0\right),\ \left(\frac{\sqrt{2}}{2},\ \frac{\sqrt{2}}{2},\ 0\right)$<br>$\left(\frac{\sqrt{2}}{2},\ -\frac{\sqrt{2}}{2},\ 0\right),\ \left(\frac{\sqrt{2}}{2},\ \frac{\sqrt{2}}{2},\ 0\right)$<br>$(1,\ 0,\ 0),\ (0,\ 1,\ 0)$ | 1⊕2 or 3⊕4<br>1⊕3 or 2⊕4<br>1⊕4 or 2⊕3 |
| 105 | V$(\frac{1}{2},\ \frac{1}{2},\ w)$ | $\left(\frac{\sqrt{2}}{2},\ -\frac{\sqrt{2}}{2},\ 0\right),\ \left(\frac{\sqrt{2}}{2},\ \frac{\sqrt{2}}{2},\ 0\right),\ (0,\ -1,\ 0),\ (1,\ 0,\ 0)$<br>$\left(\frac{\sqrt{2}}{2},\ -\frac{\sqrt{2}}{2},\ 0\right),\ \left(\frac{\sqrt{2}}{2},\ \frac{\sqrt{2}}{2},\ 0\right)$<br>$(0,\ -1,\ 0),\ (1,\ 0,\ 0)$ | 1⊕2 or 3⊕4<br>1⊕3 or 2⊕4<br>1⊕4 or 2⊕3 |
| 105 | W$(0,\ \frac{1}{2},\ w)$ | $(1,\ 0,\ 0),\ (0,\ -1,\ 0)$ | 1⊕2 or 3⊕4 |
| 106 | LD$(0,\ 0,\ w)$ | $(1,\ 0,\ 0),\ (0,\ 1,\ 0),\ \left(\frac{\sqrt{2}}{2},\ -\frac{\sqrt{2}}{2},\ 0\right),\ \left(\frac{\sqrt{2}}{2},\ \frac{\sqrt{2}}{2},\ 0\right)$<br>$\left(\frac{\sqrt{2}}{2},\ -\frac{\sqrt{2}}{2},\ 0\right),\ \left(\frac{\sqrt{2}}{2},\ \frac{\sqrt{2}}{2},\ 0\right)$<br>$(1,\ 0,\ 0),\ (0,\ 1,\ 0)$ | 1⊕2 or 3⊕4<br>1⊕3 or 2⊕4<br>1⊕4 or 2⊕3 |
| 106 | V$(\frac{1}{2},\ \frac{1}{2},\ w)$ | $(0,\ -1,\ 0),\ (1,\ 0,\ 0)$<br>$\left(\frac{\sqrt{2}}{2},\ -\frac{\sqrt{2}}{2},\ 0\right),\ \left(\frac{\sqrt{2}}{2},\ \frac{\sqrt{2}}{2},\ 0\right)$<br>$\left(\frac{\sqrt{2}}{2},\ -\frac{\sqrt{2}}{2},\ 0\right),\ \left(\frac{\sqrt{2}}{2},\ \frac{\sqrt{2}}{2},\ 0\right),\ (0,\ -1,\ 0),\ (1,\ 0,\ 0)$ | 1⊕2 or 3⊕4<br>1⊕3 or 2⊕4<br>1⊕4 or 2⊕3 |
| 107 | LD$(0,\ 0,\ w)$ | $\left(-\frac{\sqrt{2}}{2},\ -\frac{\sqrt{2}}{2},\ 0\right),\ \left(\frac{\sqrt{2}}{2},\ -\frac{\sqrt{2}}{2},\ 0\right),\ (0,\ 1,\ 0),\ (-1,\ 0,\ 0)$<br>$\left(-\frac{\sqrt{2}}{2},\ -\frac{\sqrt{2}}{2},\ 0\right),\ \left(\frac{\sqrt{2}}{2},\ -\frac{\sqrt{2}}{2},\ 0\right)$<br>$(0,\ 1,\ 0),\ (-1,\ 0,\ 0)$ | 1⊕2 or 3⊕4<br>1⊕3 or 2⊕4<br>1⊕4 or 2⊕3 |
| 107 | W$(\frac{1}{2},\ \frac{1}{2},\ w)$ | $\left(-\frac{\sqrt{2}}{2},\ -\frac{\sqrt{2}}{2},\ 0\right),\ \left(\frac{\sqrt{2}}{2},\ -\frac{\sqrt{2}}{2},\ 0\right)$ | 1⊕2 or 3⊕4 |
| 108 | LD$(0,\ 0,\ w)$ | $\left(-\frac{\sqrt{2}}{2},\ -\frac{\sqrt{2}}{2},\ 0\right),\ \left(\frac{\sqrt{2}}{2},\ -\frac{\sqrt{2}}{2},\ 0\right),\ (0,\ 1,\ 0),\ (-1,\ 0,\ 0)$<br>$\left(-\frac{\sqrt{2}}{2},\ -\frac{\sqrt{2}}{2},\ 0\right),\ \left(\frac{\sqrt{2}}{2},\ -\frac{\sqrt{2}}{2},\ 0\right)$<br>$(0,\ 1,\ 0),\ (-1,\ 0,\ 0)$ | 1⊕2 or 3⊕4<br>1⊕3 or 2⊕4<br>1⊕4 or 2⊕3 |
| 108 | W$(\frac{1}{2},\ \frac{1}{2},\ w)$ | $\left(-\frac{\sqrt{2}}{2},\ -\frac{\sqrt{2}}{2},\ 0\right),\ \left(\frac{\sqrt{2}}{2},\ -\frac{\sqrt{2}}{2},\ 0\right)$ | 1⊕2 or 3⊕4 |
| 109 | LD$(0,\ 0,\ w)$ | $\left(-\frac{\sqrt{2}}{2},\ -\frac{\sqrt{2}}{2},\ 0\right),\ \left(\frac{\sqrt{2}}{2},\ -\frac{\sqrt{2}}{2},\ 0\right),\ (0,\ 1,\ 0),\ (-1,\ 0,\ 0)$<br>$\left(-\frac{\sqrt{2}}{2},\ -\frac{\sqrt{2}}{2},\ 0\right),\ \left(\frac{\sqrt{2}}{2},\ -\frac{\sqrt{2}}{2},\ 0\right)$<br>$(0,\ 1,\ 0),\ (-1,\ 0,\ 0)$ | 1⊕2 or 3⊕4<br>1⊕3 or 2⊕4<br>1⊕4 or 2⊕3 |
| 110 | LD$(0,\ 0,\ w)$ | $\left(-\frac{\sqrt{2}}{2},\ -\frac{\sqrt{2}}{2},\ 0\right),\ \left(\frac{\sqrt{2}}{2},\ -\frac{\sqrt{2}}{2},\ 0\right),\ (0,\ 1,\ 0),\ (-1,\ 0,\ 0)$<br>$\left(-\frac{\sqrt{2}}{2},\ -\frac{\sqrt{2}}{2},\ 0\right),\ \left(\frac{\sqrt{2}}{2},\ -\frac{\sqrt{2}}{2},\ 0\right)$<br>$(0,\ 1,\ 0),\ (-1,\ 0,\ 0)$ | 1⊕2 or 3⊕4<br>1⊕3 or 2⊕4<br>1⊕4 or 2⊕3 |
| 111 | LD$(0,\ 0,\ w)$ | $\left(\frac{\sqrt{2}}{2},\ -\frac{\sqrt{2}}{2},\ 0\right),\ \left(\frac{\sqrt{2}}{2},\ \frac{\sqrt{2}}{2},\ 0\right)$ | {1}⊕{2} |
| 111 | V$(\frac{1}{2},\ \frac{1}{2},\ w)$ | $\left(\frac{\sqrt{2}}{2},\ -\frac{\sqrt{2}}{2},\ 0\right),\ \left(\frac{\sqrt{2}}{2},\ \frac{\sqrt{2}}{2},\ 0\right)$ | {1}⊕{2} |
| 112 | LD$(0,\ 0,\ w)$ | $\left(\frac{\sqrt{2}}{2},\ -\frac{\sqrt{2}}{2},\ 0\right),\ \left(\frac{\sqrt{2}}{2},\ \frac{\sqrt{2}}{2},\ 0\right)$ | {1}⊕{2} |
| 112 | V$(\frac{1}{2},\ \frac{1}{2},\ w)$ | $\left(\frac{\sqrt{2}}{2},\ -\frac{\sqrt{2}}{2},\ 0\right),\ \left(\frac{\sqrt{2}}{2},\ \frac{\sqrt{2}}{2},\ 0\right)$ | {1}⊕{2} |

| SG | HSL | Location of nodal chain | Irreps of BC |
|---|---|---|---|
| 113 | LD$(0,\ 0,\ w)$ | $\left(\frac{\sqrt{2}}{2},\ -\frac{\sqrt{2}}{2},\ 0\right),\ \left(\frac{\sqrt{2}}{2},\ \frac{\sqrt{2}}{2},\ 0\right)$ | $\{1\}\oplus\{2\}$ |
| 114 | LD$(0,\ 0,\ w)$ | $\left(\frac{\sqrt{2}}{2},\ -\frac{\sqrt{2}}{2},\ 0\right),\ \left(\frac{\sqrt{2}}{2},\ \frac{\sqrt{2}}{2},\ 0\right)$ | $\{1\}\oplus\{2\}$ |
| 115 | LD$(0,\ 0,\ w)$ | $(1,\ 0,\ 0),\ (0,\ 1,\ 0)$ | $\{1\}\oplus\{2\}$ |
| 115 | V$\left(\frac{1}{2},\ \frac{1}{2},\ w\right)$ | $(0,\ -1,\ 0),\ (-1,\ 0,\ 0)$ | $\{1\}\oplus\{2\}$ |
| 115 | W$\left(0,\ \frac{1}{2},\ w\right)$ | $(1,\ 0,\ 0),\ (0,\ -1,\ 0)$ | $1\oplus2$ or $3\oplus4$ |
| 116 | LD$(0,\ 0,\ w)$ | $(1,\ 0,\ 0),\ (0,\ 1,\ 0)$ | $\{1\}\oplus\{2\}$ |
| 116 | V$\left(\frac{1}{2},\ \frac{1}{2},\ w\right)$ | $(0,\ -1,\ 0),\ (-1,\ 0,\ 0)$ | $\{1\}\oplus\{2\}$ |
| 116 | W$\left(0,\ \frac{1}{2},\ w\right)$ | $(1,\ 0,\ 0),\ (0,\ -1,\ 0)$ | $1\oplus2$ or $3\oplus4$ |
| 117 | LD$(0,\ 0,\ w)$ | $(1,\ 0,\ 0),\ (0,\ 1,\ 0)$ | $\{1\}\oplus\{2\}$ |
| 117 | V$\left(\frac{1}{2},\ \frac{1}{2},\ w\right)$ | $(0,\ -1,\ 0),\ (-1,\ 0,\ 0)$ | $\{1\}\oplus\{2\}$ |
| 118 | LD$(0,\ 0,\ w)$ | $(1,\ 0,\ 0),\ (0,\ 1,\ 0)$ | $\{1\}\oplus\{2\}$ |
| 118 | V$\left(\frac{1}{2},\ \frac{1}{2},\ w\right)$ | $(0,\ -1,\ 0),\ (-1,\ 0,\ 0)$ | $\{1\}\oplus\{2\}$ |
| 119 | LD$(0,\ 0,\ w)$ | $(0,\ 1,\ 0),\ (1,\ 0,\ 0)$ | $\{1\}\oplus\{2\}$ |
| 120 | LD$(0,\ 0,\ w)$ | $(0,\ 1,\ 0),\ (1,\ 0,\ 0)$ | $\{1\}\oplus\{2\}$ |
| 121 | LD$(0,\ 0,\ w)$ | $\left(-\frac{\sqrt{2}}{2},\ -\frac{\sqrt{2}}{2},\ 0\right),\ \left(-\frac{\sqrt{2}}{2},\ \frac{\sqrt{2}}{2},\ 0\right)$ | $\{1\}\oplus\{2\}$ |
| 121 | W$\left(\frac{1}{2},\ \frac{1}{2},\ w\right)$ | $\left(-\frac{\sqrt{2}}{2},\ -\frac{\sqrt{2}}{2},\ 0\right),\ \left(-\frac{\sqrt{2}}{2},\ \frac{\sqrt{2}}{2},\ 0\right)$ | $1\oplus2$ or $3\oplus4$ |
| 122 | LD$(0,\ 0,\ w)$ | $\left(-\frac{\sqrt{2}}{2},\ \frac{\sqrt{2}}{2},\ 0\right),\ \left(\frac{\sqrt{2}}{2},\ \frac{\sqrt{2}}{2},\ 0\right)$ | $\{1\}\oplus\{2\}$ |
| 123 | DT$(0,\ v,\ 0)$ | $(0,\ 0,\ 1),\ (1,\ 0,\ 0)$ | $\{1\}\oplus\{2\}$ or $\{3\}\oplus\{4\}$ |
| 123 | LD$(0,\ 0,\ w)$ | $(1,\ 0,\ 0),\ (0,\ 1,\ 0),\ \left(\frac{\sqrt{2}}{2},\ -\frac{\sqrt{2}}{2},\ 0\right),\ \left(\frac{\sqrt{2}}{2},\ \frac{\sqrt{2}}{2},\ 0\right)$<br>$\left(\frac{\sqrt{2}}{2},\ -\frac{\sqrt{2}}{2},\ 0\right),\ \left(\frac{\sqrt{2}}{2},\ \frac{\sqrt{2}}{2},\ 0\right)$<br>$(1,\ 0,\ 0),\ (0,\ 1,\ 0)$ | $\{1\}\oplus\{2\}$ or $\{3\}\oplus\{4\}$<br>$\{1\}\oplus\{3\}$ or $\{2\}\oplus\{4\}$<br>$\{1\}\oplus\{4\}$ or $\{2\}\oplus\{3\}$ |
| 123 | S$\left(u,\ u,\ \frac{1}{2}\right)$ | $(0,\ 0,\ 1),\ \left(\frac{\sqrt{2}}{2},\ -\frac{\sqrt{2}}{2},\ 0\right)$ | $\{1\}\oplus\{2\}$ or $\{3\}\oplus\{4\}$ |
| 123 | SM$(u,\ u,\ 0)$ | $(0,\ 0,\ 1),\ \left(\frac{\sqrt{2}}{2},\ -\frac{\sqrt{2}}{2},\ 0\right)$ | $\{1\}\oplus\{2\}$ or $\{3\}\oplus\{4\}$ |
| 123 | T$\left(u,\ \frac{1}{2},\ \frac{1}{2}\right)$ | $(0,\ 0,\ 1),\ (0,\ -1,\ 0)$ | $\{1\}\oplus\{2\}$ or $\{3\}\oplus\{4\}$ |
| 123 | U$\left(0,\ v,\ \frac{1}{2}\right)$ | $(0,\ 0,\ 1),\ (1,\ 0,\ 0)$ | $\{1\}\oplus\{2\}$ or $\{3\}\oplus\{4\}$ |
| 123 | V$\left(\frac{1}{2},\ \frac{1}{2},\ w\right)$ | $\left(\frac{\sqrt{2}}{2},\ -\frac{\sqrt{2}}{2},\ 0\right),\ \left(\frac{\sqrt{2}}{2},\ \frac{\sqrt{2}}{2},\ 0\right),\ (0,\ -1,\ 0),\ (1,\ 0,\ 0)$<br>$\left(\frac{\sqrt{2}}{2},\ -\frac{\sqrt{2}}{2},\ 0\right),\ \left(\frac{\sqrt{2}}{2},\ \frac{\sqrt{2}}{2},\ 0\right)$<br>$(0,\ -1,\ 0),\ (1,\ 0,\ 0)$ | $\{1\}\oplus\{2\}$ or $\{3\}\oplus\{4\}$<br>$\{1\}\oplus\{3\}$ or $\{2\}\oplus\{4\}$<br>$\{1\}\oplus\{4\}$ or $\{2\}\oplus\{3\}$ |
| 123 | W$\left(0,\ \frac{1}{2},\ w\right)$ | $(1,\ 0,\ 0),\ (0,\ -1,\ 0)$ | $\{1\}\oplus\{2\}$ or $\{3\}\oplus\{4\}$ |
| 123 | Y$\left(u,\ \frac{1}{2},\ 0\right)$ | $(0,\ 0,\ 1),\ (0,\ -1,\ 0)$ | $\{1\}\oplus\{2\}$ or $\{3\}\oplus\{4\}$ |
| 124 | DT$(0,\ v,\ 0)$ | $(0,\ 0,\ 1),\ (1,\ 0,\ 0)$ | $\{1\}\oplus\{2\}$ or $\{3\}\oplus\{4\}$ |
| 124 | LD$(0,\ 0,\ w)$ | $(1,\ 0,\ 0),\ (0,\ 1,\ 0),\ \left(\frac{\sqrt{2}}{2},\ -\frac{\sqrt{2}}{2},\ 0\right),\ \left(\frac{\sqrt{2}}{2},\ \frac{\sqrt{2}}{2},\ 0\right)$<br>$\left(\frac{\sqrt{2}}{2},\ -\frac{\sqrt{2}}{2},\ 0\right),\ \left(\frac{\sqrt{2}}{2},\ \frac{\sqrt{2}}{2},\ 0\right)$<br>$(1,\ 0,\ 0),\ (0,\ 1,\ 0)$ | $\{1\}\oplus\{2\}$ or $\{3\}\oplus\{4\}$<br>$\{1\}\oplus\{3\}$ or $\{2\}\oplus\{4\}$<br>$\{1\}\oplus\{4\}$ or $\{2\}\oplus\{3\}$ |
| 124 | SM$(u,\ u,\ 0)$ | $(0,\ 0,\ 1),\ \left(\frac{\sqrt{2}}{2},\ -\frac{\sqrt{2}}{2},\ 0\right)$ | $\{1\}\oplus\{2\}$ or $\{3\}\oplus\{4\}$ |
| 124 | V$\left(\frac{1}{2},\ \frac{1}{2},\ w\right)$ | $\left(\frac{\sqrt{2}}{2},\ -\frac{\sqrt{2}}{2},\ 0\right),\ \left(\frac{\sqrt{2}}{2},\ \frac{\sqrt{2}}{2},\ 0\right),\ (0,\ -1,\ 0),\ (1,\ 0,\ 0)$<br>$\left(\frac{\sqrt{2}}{2},\ -\frac{\sqrt{2}}{2},\ 0\right),\ \left(\frac{\sqrt{2}}{2},\ \frac{\sqrt{2}}{2},\ 0\right)$<br>$(0,\ -1,\ 0),\ (1,\ 0,\ 0)$ | $\{1\}\oplus\{2\}$ or $\{3\}\oplus\{4\}$<br>$\{1\}\oplus\{3\}$ or $\{2\}\oplus\{4\}$<br>$\{1\}\oplus\{4\}$ or $\{2\}\oplus\{3\}$ |
| 124 | W$\left(0,\ \frac{1}{2},\ w\right)$ | $(1,\ 0,\ 0),\ (0,\ -1,\ 0)$ | $\{1\}\oplus\{2\}$ or $\{3\}\oplus\{4\}$ |
| 124 | Y$\left(u,\ \frac{1}{2},\ 0\right)$ | $(0,\ 0,\ 1),\ (0,\ -1,\ 0)$ | $\{1\}\oplus\{2\}$ or $\{3\}\oplus\{4\}$ |
| 125 | DT$(0,\ v,\ 0)$ | $(0,\ 0,\ 1),\ (1,\ 0,\ 0)$ | $\{1\}\oplus\{2\}$ or $\{3\}\oplus\{4\}$ |

| SG | HSL | Location of nodal chain | Irreps of BC |
|---|---|---|---|
| 125 | LD$(0,\ 0,\ w)$ | $(1,\ 0,\ 0)$, $(0,\ 1,\ 0)$, $\left(\frac{\sqrt{2}}{2},\ -\frac{\sqrt{2}}{2},\ 0\right)$, $\left(\frac{\sqrt{2}}{2},\ \frac{\sqrt{2}}{2},\ 0\right)$<br>$\left(\frac{\sqrt{2}}{2},\ -\frac{\sqrt{2}}{2},\ 0\right)$, $\left(\frac{\sqrt{2}}{2},\ \frac{\sqrt{2}}{2},\ 0\right)$<br>$(1,\ 0,\ 0)$, $(0,\ 1,\ 0)$ | {1}⊕{2} or {3}⊕{4}<br>{1}⊕{3} or {2}⊕{4}<br>{1}⊕{4} or {2}⊕{3} |
| 125 | S$\left(u,\ u,\ \frac{1}{2}\right)$ | $(0,\ 0,\ 1)$, $\left(\frac{\sqrt{2}}{2},\ -\frac{\sqrt{2}}{2},\ 0\right)$ | {1}⊕{2} or {3}⊕{4} |
| 125 | SM$(u,\ u,\ 0)$ | $(0,\ 0,\ 1)$, $\left(\frac{\sqrt{2}}{2},\ -\frac{\sqrt{2}}{2},\ 0\right)$ | {1}⊕{2} or {3}⊕{4} |
| 125 | U$\left(0,\ v,\ \frac{1}{2}\right)$ | $(0,\ 0,\ 1)$, $(1,\ 0,\ 0)$ | {1}⊕{2} or {3}⊕{4} |
| 125 | V$\left(\frac{1}{2},\ \frac{1}{2},\ w\right)$ | $(0,\ -1,\ 0)$, $(1,\ 0,\ 0)$<br>$\left(\frac{\sqrt{2}}{2},\ -\frac{\sqrt{2}}{2},\ 0\right)$, $\left(\frac{\sqrt{2}}{2},\ \frac{\sqrt{2}}{2},\ 0\right)$<br>$\left(\frac{\sqrt{2}}{2},\ -\frac{\sqrt{2}}{2},\ 0\right)$, $\left(\frac{\sqrt{2}}{2},\ \frac{\sqrt{2}}{2},\ 0\right)$, $(0,\ -1,\ 0)$, $(1,\ 0,\ 0)$ | {1}⊕{2} or {3}⊕{4}<br>{1}⊕{3} or {2}⊕{4}<br>{1}⊕{4} or {2}⊕{3} |
| 126 | DT$(0,\ v,\ 0)$ | $(0,\ 0,\ 1)$, $(1,\ 0,\ 0)$ | {1}⊕{2} or {3}⊕{4} |
| 126 | LD$(0,\ 0,\ w)$ | $(1,\ 0,\ 0)$, $(0,\ 1,\ 0)$, $\left(\frac{\sqrt{2}}{2},\ -\frac{\sqrt{2}}{2},\ 0\right)$, $\left(\frac{\sqrt{2}}{2},\ \frac{\sqrt{2}}{2},\ 0\right)$<br>$\left(\frac{\sqrt{2}}{2},\ -\frac{\sqrt{2}}{2},\ 0\right)$, $\left(\frac{\sqrt{2}}{2},\ \frac{\sqrt{2}}{2},\ 0\right)$<br>$(1,\ 0,\ 0)$, $(0,\ 1,\ 0)$ | {1}⊕{2} or {3}⊕{4}<br>{1}⊕{3} or {2}⊕{4}<br>{1}⊕{4} or {2}⊕{3} |
| 126 | SM$(u,\ u,\ 0)$ | $(0,\ 0,\ 1)$, $\left(\frac{\sqrt{2}}{2},\ -\frac{\sqrt{2}}{2},\ 0\right)$ | {1}⊕{2} or {3}⊕{4} |
| 126 | T$\left(u,\ \frac{1}{2},\ \frac{1}{2}\right)$ | $(0,\ 0,\ 1)$, $(0,\ -1,\ 0)$ | {1}⊕{2} or {3}⊕{4} |
| 126 | V$\left(\frac{1}{2},\ \frac{1}{2},\ w\right)$ | $(0,\ -1,\ 0)$, $(1,\ 0,\ 0)$<br>$\left(\frac{\sqrt{2}}{2},\ -\frac{\sqrt{2}}{2},\ 0\right)$, $\left(\frac{\sqrt{2}}{2},\ \frac{\sqrt{2}}{2},\ 0\right)$<br>$\left(\frac{\sqrt{2}}{2},\ -\frac{\sqrt{2}}{2},\ 0\right)$, $\left(\frac{\sqrt{2}}{2},\ \frac{\sqrt{2}}{2},\ 0\right)$, $(0,\ -1,\ 0)$, $(1,\ 0,\ 0)$ | {1}⊕{2} or {3}⊕{4}<br>{1}⊕{3} or {2}⊕{4}<br>{1}⊕{4} or {2}⊕{3} |
| 127 | DT$(0,\ v,\ 0)$ | $(0,\ 0,\ 1)$, $(1,\ 0,\ 0)$ | {1}⊕{2} or {3}⊕{4} |
| 127 | LD$(0,\ 0,\ w)$ | $(1,\ 0,\ 0)$, $(0,\ 1,\ 0)$, $\left(\frac{\sqrt{2}}{2},\ -\frac{\sqrt{2}}{2},\ 0\right)$, $\left(\frac{\sqrt{2}}{2},\ \frac{\sqrt{2}}{2},\ 0\right)$<br>$\left(\frac{\sqrt{2}}{2},\ -\frac{\sqrt{2}}{2},\ 0\right)$, $\left(\frac{\sqrt{2}}{2},\ \frac{\sqrt{2}}{2},\ 0\right)$<br>$(1,\ 0,\ 0)$, $(0,\ 1,\ 0)$ | {1}⊕{2} or {3}⊕{4}<br>{1}⊕{3} or {2}⊕{4}<br>{1}⊕{4} or {2}⊕{3} |
| 127 | S$\left(u,\ u,\ \frac{1}{2}\right)$ | $(0,\ 0,\ 1)$, $\left(\frac{\sqrt{2}}{2},\ -\frac{\sqrt{2}}{2},\ 0\right)$ | {1}⊕{2} or {3}⊕{4} |
| 127 | SM$(u,\ u,\ 0)$ | $(0,\ 0,\ 1)$, $\left(\frac{\sqrt{2}}{2},\ -\frac{\sqrt{2}}{2},\ 0\right)$ | {1}⊕{2} or {3}⊕{4} |
| 127 | U$\left(0,\ v,\ \frac{1}{2}\right)$ | $(0,\ 0,\ 1)$, $(1,\ 0,\ 0)$ | {1}⊕{2} or {3}⊕{4} |
| 128 | DT$(0,\ v,\ 0)$ | $(0,\ 0,\ 1)$, $(1,\ 0,\ 0)$ | {1}⊕{2} or {3}⊕{4} |
| 128 | LD$(0,\ 0,\ w)$ | $(1,\ 0,\ 0)$, $(0,\ 1,\ 0)$, $\left(\frac{\sqrt{2}}{2},\ -\frac{\sqrt{2}}{2},\ 0\right)$, $\left(\frac{\sqrt{2}}{2},\ \frac{\sqrt{2}}{2},\ 0\right)$<br>$\left(\frac{\sqrt{2}}{2},\ -\frac{\sqrt{2}}{2},\ 0\right)$, $\left(\frac{\sqrt{2}}{2},\ \frac{\sqrt{2}}{2},\ 0\right)$<br>$(1,\ 0,\ 0)$, $(0,\ 1,\ 0)$ | {1}⊕{2} or {3}⊕{4}<br>{1}⊕{3} or {2}⊕{4}<br>{1}⊕{4} or {2}⊕{3} |
| 128 | SM$(u,\ u,\ 0)$ | $(0,\ 0,\ 1)$, $\left(\frac{\sqrt{2}}{2},\ -\frac{\sqrt{2}}{2},\ 0\right)$ | {1}⊕{2} or {3}⊕{4} |
| 129 | DT$(0,\ v,\ 0)$ | $(0,\ 0,\ 1)$, $(1,\ 0,\ 0)$ | {1}⊕{2} or {3}⊕{4} |
| 129 | LD$(0,\ 0,\ w)$ | $(1,\ 0,\ 0)$, $(0,\ 1,\ 0)$, $\left(\frac{\sqrt{2}}{2},\ -\frac{\sqrt{2}}{2},\ 0\right)$, $\left(\frac{\sqrt{2}}{2},\ \frac{\sqrt{2}}{2},\ 0\right)$<br>$\left(\frac{\sqrt{2}}{2},\ -\frac{\sqrt{2}}{2},\ 0\right)$, $\left(\frac{\sqrt{2}}{2},\ \frac{\sqrt{2}}{2},\ 0\right)$<br>$(1,\ 0,\ 0)$, $(0,\ 1,\ 0)$ | {1}⊕{2} or {3}⊕{4}<br>{1}⊕{3} or {2}⊕{4}<br>{1}⊕{4} or {2}⊕{3} |
| 129 | S$\left(u,\ u,\ \frac{1}{2}\right)$ | $(0,\ 0,\ 1)$, $\left(\frac{\sqrt{2}}{2},\ -\frac{\sqrt{2}}{2},\ 0\right)$ | {1}⊕{2} or {3}⊕{4} |
| 129 | SM$(u,\ u,\ 0)$ | $(0,\ 0,\ 1)$, $\left(\frac{\sqrt{2}}{2},\ -\frac{\sqrt{2}}{2},\ 0\right)$ | {1}⊕{2} or {3}⊕{4} |
| 129 | U$\left(0,\ v,\ \frac{1}{2}\right)$ | $(0,\ 0,\ 1)$, $(1,\ 0,\ 0)$ | {1}⊕{2} or {3}⊕{4} |
| 130 | DT$(0,\ v,\ 0)$ | $(0,\ 0,\ 1)$, $(1,\ 0,\ 0)$ | {1}⊕{2} or {3}⊕{4} |
| 130 | LD$(0,\ 0,\ w)$ | $(1,\ 0,\ 0)$, $(0,\ 1,\ 0)$, $\left(\frac{\sqrt{2}}{2},\ -\frac{\sqrt{2}}{2},\ 0\right)$, $\left(\frac{\sqrt{2}}{2},\ \frac{\sqrt{2}}{2},\ 0\right)$<br>$\left(\frac{\sqrt{2}}{2},\ -\frac{\sqrt{2}}{2},\ 0\right)$, $\left(\frac{\sqrt{2}}{2},\ \frac{\sqrt{2}}{2},\ 0\right)$<br>$(1,\ 0,\ 0)$, $(0,\ 1,\ 0)$ | {1}⊕{2} or {3}⊕{4}<br>{1}⊕{3} or {2}⊕{4}<br>{1}⊕{4} or {2}⊕{3} |

| SG | HSL | Location of nodal chain | Irreps of BC |
|---|---|---|---|
| 130 | SM$(u,\ u,\ 0)$ | $(0,\ 0,\ 1)$, $\left(\frac{\sqrt{2}}{2},\ -\frac{\sqrt{2}}{2},\ 0\right)$ | $\{1\}\oplus\{2\}$ or $\{3\}\oplus\{4\}$ |
| 131 | DT$(0,\ v,\ 0)$ | $(0,\ 0,\ 1)$, $(1,\ 0,\ 0)$ | $\{1\}\oplus\{2\}$ or $\{3\}\oplus\{4\}$ |
| 131 | LD$(0,\ 0,\ w)$ | $(1,\ 0,\ 0)$, $(0,\ 1,\ 0)$, $\left(\frac{\sqrt{2}}{2},\ -\frac{\sqrt{2}}{2},\ 0\right)$, $\left(\frac{\sqrt{2}}{2},\ \frac{\sqrt{2}}{2},\ 0\right)$<br>$\left(\frac{\sqrt{2}}{2},\ -\frac{\sqrt{2}}{2},\ 0\right)$, $\left(\frac{\sqrt{2}}{2},\ \frac{\sqrt{2}}{2},\ 0\right)$<br>$(1,\ 0,\ 0)$, $(0,\ 1,\ 0)$ | $\{1\}\oplus\{2\}$ or $\{3\}\oplus\{4\}$<br>$\{1\}\oplus\{3\}$ or $\{2\}\oplus\{4\}$<br>$\{1\}\oplus\{4\}$ or $\{2\}\oplus\{3\}$ |
| 131 | SM$(u,\ u,\ 0)$ | $(0,\ 0,\ 1)$, $\left(\frac{\sqrt{2}}{2},\ -\frac{\sqrt{2}}{2},\ 0\right)$ | $\{1\}\oplus\{2\}$ or $\{3\}\oplus\{4\}$ |
| 131 | T$\left(u,\ \frac{1}{2},\ \frac{1}{2}\right)$ | $(0,\ 0,\ 1)$, $(0,\ -1,\ 0)$ | $\{1\}\oplus\{2\}$ or $\{3\}\oplus\{4\}$ |
| 131 | U$\left(0,\ v,\ \frac{1}{2}\right)$ | $(0,\ 0,\ 1)$, $(1,\ 0,\ 0)$ | $\{1\}\oplus\{2\}$ or $\{3\}\oplus\{4\}$ |
| 131 | V$\left(\frac{1}{2},\ \frac{1}{2},\ w\right)$ | $\left(\frac{\sqrt{2}}{2},\ -\frac{\sqrt{2}}{2},\ 0\right)$, $\left(\frac{\sqrt{2}}{2},\ \frac{\sqrt{2}}{2},\ 0\right)$, $(0,\ -1,\ 0)$, $(1,\ 0,\ 0)$<br>$\left(\frac{\sqrt{2}}{2},\ -\frac{\sqrt{2}}{2},\ 0\right)$, $\left(\frac{\sqrt{2}}{2},\ \frac{\sqrt{2}}{2},\ 0\right)$<br>$(0,\ -1,\ 0)$, $(1,\ 0,\ 0)$ | $\{1\}\oplus\{2\}$ or $\{3\}\oplus\{4\}$<br>$\{1\}\oplus\{3\}$ or $\{2\}\oplus\{4\}$<br>$\{1\}\oplus\{4\}$ or $\{2\}\oplus\{3\}$ |
| 131 | W$\left(0,\ \frac{1}{2},\ w\right)$ | $(1,\ 0,\ 0)$, $(0,\ -1,\ 0)$ | $\{1\}\oplus\{2\}$ or $\{3\}\oplus\{4\}$ |
| 131 | Y$\left(u,\ \frac{1}{2},\ 0\right)$ | $(0,\ 0,\ 1)$, $(0,\ -1,\ 0)$ | $\{1\}\oplus\{2\}$ or $\{3\}\oplus\{4\}$ |
| 132 | DT$(0,\ v,\ 0)$ | $(0,\ 0,\ 1)$, $(1,\ 0,\ 0)$ | $\{1\}\oplus\{2\}$ or $\{3\}\oplus\{4\}$ |
| 132 | LD$(0,\ 0,\ w)$ | $(1,\ 0,\ 0)$, $(0,\ 1,\ 0)$, $\left(\frac{\sqrt{2}}{2},\ -\frac{\sqrt{2}}{2},\ 0\right)$, $\left(\frac{\sqrt{2}}{2},\ \frac{\sqrt{2}}{2},\ 0\right)$<br>$\left(\frac{\sqrt{2}}{2},\ -\frac{\sqrt{2}}{2},\ 0\right)$, $\left(\frac{\sqrt{2}}{2},\ \frac{\sqrt{2}}{2},\ 0\right)$<br>$(1,\ 0,\ 0)$, $(0,\ 1,\ 0)$ | $\{1\}\oplus\{2\}$ or $\{3\}\oplus\{4\}$<br>$\{1\}\oplus\{3\}$ or $\{2\}\oplus\{4\}$<br>$\{1\}\oplus\{4\}$ or $\{2\}\oplus\{3\}$ |
| 132 | S$\left(u,\ u,\ \frac{1}{2}\right)$ | $(0,\ 0,\ 1)$, $\left(\frac{\sqrt{2}}{2},\ -\frac{\sqrt{2}}{2},\ 0\right)$ | $\{1\}\oplus\{3\}$ or $\{2\}\oplus\{4\}$ |
| 132 | SM$(u,\ u,\ 0)$ | $(0,\ 0,\ 1)$, $\left(\frac{\sqrt{2}}{2},\ -\frac{\sqrt{2}}{2},\ 0\right)$ | $\{1\}\oplus\{2\}$ or $\{3\}\oplus\{4\}$ |
| 132 | V$\left(\frac{1}{2},\ \frac{1}{2},\ w\right)$ | $\left(\frac{\sqrt{2}}{2},\ -\frac{\sqrt{2}}{2},\ 0\right)$, $\left(\frac{\sqrt{2}}{2},\ \frac{\sqrt{2}}{2},\ 0\right)$, $(0,\ -1,\ 0)$, $(1,\ 0,\ 0)$<br>$\left(\frac{\sqrt{2}}{2},\ -\frac{\sqrt{2}}{2},\ 0\right)$, $\left(\frac{\sqrt{2}}{2},\ \frac{\sqrt{2}}{2},\ 0\right)$<br>$(0,\ -1,\ 0)$, $(1,\ 0,\ 0)$ | $\{1\}\oplus\{2\}$ or $\{3\}\oplus\{4\}$<br>$\{1\}\oplus\{3\}$ or $\{2\}\oplus\{4\}$<br>$\{1\}\oplus\{4\}$ or $\{2\}\oplus\{3\}$ |
| 132 | W$\left(0,\ \frac{1}{2},\ w\right)$ | $(1,\ 0,\ 0)$, $(0,\ -1,\ 0)$ | $\{1\}\oplus\{2\}$ or $\{3\}\oplus\{4\}$ |
| 132 | Y$\left(u,\ \frac{1}{2},\ 0\right)$ | $(0,\ 0,\ 1)$, $(0,\ -1,\ 0)$ | $\{1\}\oplus\{2\}$ or $\{3\}\oplus\{4\}$ |
| 133 | DT$(0,\ v,\ 0)$ | $(0,\ 0,\ 1)$, $(1,\ 0,\ 0)$ | $\{1\}\oplus\{2\}$ or $\{3\}\oplus\{4\}$ |
| 133 | LD$(0,\ 0,\ w)$ | $(1,\ 0,\ 0)$, $(0,\ 1,\ 0)$, $\left(\frac{\sqrt{2}}{2},\ -\frac{\sqrt{2}}{2},\ 0\right)$, $\left(\frac{\sqrt{2}}{2},\ \frac{\sqrt{2}}{2},\ 0\right)$<br>$\left(\frac{\sqrt{2}}{2},\ -\frac{\sqrt{2}}{2},\ 0\right)$, $\left(\frac{\sqrt{2}}{2},\ \frac{\sqrt{2}}{2},\ 0\right)$<br>$(1,\ 0,\ 0)$, $(0,\ 1,\ 0)$ | $\{1\}\oplus\{2\}$ or $\{3\}\oplus\{4\}$<br>$\{1\}\oplus\{3\}$ or $\{2\}\oplus\{4\}$<br>$\{1\}\oplus\{4\}$ or $\{2\}\oplus\{3\}$ |
| 133 | SM$(u,\ u,\ 0)$ | $(0,\ 0,\ 1)$, $\left(\frac{\sqrt{2}}{2},\ -\frac{\sqrt{2}}{2},\ 0\right)$ | $\{1\}\oplus\{2\}$ or $\{3\}\oplus\{4\}$ |
| 133 | U$\left(0,\ v,\ \frac{1}{2}\right)$ | $(0,\ 0,\ 1)$, $(1,\ 0,\ 0)$ | $\{1\}\oplus\{2\}$ or $\{3\}\oplus\{4\}$ |
| 133 | V$\left(\frac{1}{2},\ \frac{1}{2},\ w\right)$ | $(0,\ -1,\ 0)$, $(1,\ 0,\ 0)$<br>$\left(\frac{\sqrt{2}}{2},\ -\frac{\sqrt{2}}{2},\ 0\right)$, $\left(\frac{\sqrt{2}}{2},\ \frac{\sqrt{2}}{2},\ 0\right)$<br>$\left(\frac{\sqrt{2}}{2},\ -\frac{\sqrt{2}}{2},\ 0\right)$, $\left(\frac{\sqrt{2}}{2},\ \frac{\sqrt{2}}{2},\ 0\right)$, $(0,\ -1,\ 0)$, $(1,\ 0,\ 0)$ | $\{1\}\oplus\{2\}$ or $\{3\}\oplus\{4\}$<br>$\{1\}\oplus\{3\}$ or $\{2\}\oplus\{4\}$<br>$\{1\}\oplus\{4\}$ or $\{2\}\oplus\{3\}$ |
| 134 | DT$(0,\ v,\ 0)$ | $(0,\ 0,\ 1)$, $(1,\ 0,\ 0)$ | $\{1\}\oplus\{2\}$ or $\{3\}\oplus\{4\}$ |
| 134 | LD$(0,\ 0,\ w)$ | $(1,\ 0,\ 0)$, $(0,\ 1,\ 0)$, $\left(\frac{\sqrt{2}}{2},\ -\frac{\sqrt{2}}{2},\ 0\right)$, $\left(\frac{\sqrt{2}}{2},\ \frac{\sqrt{2}}{2},\ 0\right)$<br>$\left(\frac{\sqrt{2}}{2},\ -\frac{\sqrt{2}}{2},\ 0\right)$, $\left(\frac{\sqrt{2}}{2},\ \frac{\sqrt{2}}{2},\ 0\right)$<br>$(1,\ 0,\ 0)$, $(0,\ 1,\ 0)$ | $\{1\}\oplus\{2\}$ or $\{3\}\oplus\{4\}$<br>$\{1\}\oplus\{3\}$ or $\{2\}\oplus\{4\}$<br>$\{1\}\oplus\{4\}$ or $\{2\}\oplus\{3\}$ |
| 134 | S$\left(u,\ u,\ \frac{1}{2}\right)$ | $(0,\ 0,\ 1)$, $\left(\frac{\sqrt{2}}{2},\ -\frac{\sqrt{2}}{2},\ 0\right)$ | $\{1\}\oplus\{3\}$ or $\{2\}\oplus\{4\}$ |
| 134 | SM$(u,\ u,\ 0)$ | $(0,\ 0,\ 1)$, $\left(\frac{\sqrt{2}}{2},\ -\frac{\sqrt{2}}{2},\ 0\right)$ | $\{1\}\oplus\{2\}$ or $\{3\}\oplus\{4\}$ |
| 134 | T$\left(u,\ \frac{1}{2},\ \frac{1}{2}\right)$ | $(0,\ 0,\ 1)$, $(0,\ -1,\ 0)$ | $\{1\}\oplus\{2\}$ or $\{3\}\oplus\{4\}$ |

| SG | HSL | Location of nodal chain | Irreps of BC |
|---|---|---|---|
| 134 | $\mathrm{V}\left(\frac{1}{2},\ \frac{1}{2},\ w\right)$ | $(0,\ -1,\ 0),\ (1,\ 0,\ 0)$<br>$\left(\frac{\sqrt{2}}{2},\ -\frac{\sqrt{2}}{2},\ 0\right),\ \left(\frac{\sqrt{2}}{2},\ \frac{\sqrt{2}}{2},\ 0\right)$<br>$\left(\frac{\sqrt{2}}{2},\ -\frac{\sqrt{2}}{2},\ 0\right),\ \left(\frac{\sqrt{2}}{2},\ \frac{\sqrt{2}}{2},\ 0\right),\ (0,\ -1,\ 0),\ (1,\ 0,\ 0)$ | $\{1\}\oplus\{2\}$ or $\{3\}\oplus\{4\}$<br>$\{1\}\oplus\{3\}$ or $\{2\}\oplus\{4\}$<br>$\{1\}\oplus\{4\}$ or $\{2\}\oplus\{3\}$ |
| 135 | $\mathrm{DT}(0,\ v,\ 0)$ | $(0,\ 0,\ 1),\ (1,\ 0,\ 0)$ | $\{1\}\oplus\{2\}$ or $\{3\}\oplus\{4\}$ |
| 135 | $\mathrm{LD}(0,\ 0,\ w)$ | $(1,\ 0,\ 0),\ (0,\ 1,\ 0),\ \left(\frac{\sqrt{2}}{2},\ -\frac{\sqrt{2}}{2},\ 0\right),\ \left(\frac{\sqrt{2}}{2},\ \frac{\sqrt{2}}{2},\ 0\right)$<br>$\left(\frac{\sqrt{2}}{2},\ -\frac{\sqrt{2}}{2},\ 0\right),\ \left(\frac{\sqrt{2}}{2},\ \frac{\sqrt{2}}{2},\ 0\right)$<br>$(1,\ 0,\ 0),\ (0,\ 1,\ 0)$ | $\{1\}\oplus\{2\}$ or $\{3\}\oplus\{4\}$<br>$\{1\}\oplus\{3\}$ or $\{2\}\oplus\{4\}$<br>$\{1\}\oplus\{4\}$ or $\{2\}\oplus\{3\}$ |
| 135 | $\mathrm{SM}(u,\ u,\ 0)$ | $(0,\ 0,\ 1),\ \left(\frac{\sqrt{2}}{2},\ -\frac{\sqrt{2}}{2},\ 0\right)$ | $\{1\}\oplus\{2\}$ or $\{3\}\oplus\{4\}$ |
| 135 | $\mathrm{U}\left(0,\ v,\ \frac{1}{2}\right)$ | $(0,\ 0,\ 1),\ (1,\ 0,\ 0)$ | $\{1\}\oplus\{2\}$ or $\{3\}\oplus\{4\}$ |
| 136 | $\mathrm{DT}(0,\ v,\ 0)$ | $(0,\ 0,\ 1),\ (1,\ 0,\ 0)$ | $\{1\}\oplus\{2\}$ or $\{3\}\oplus\{4\}$ |
| 136 | $\mathrm{LD}(0,\ 0,\ w)$ | $(1,\ 0,\ 0),\ (0,\ 1,\ 0),\ \left(\frac{\sqrt{2}}{2},\ -\frac{\sqrt{2}}{2},\ 0\right),\ \left(\frac{\sqrt{2}}{2},\ \frac{\sqrt{2}}{2},\ 0\right)$<br>$\left(\frac{\sqrt{2}}{2},\ -\frac{\sqrt{2}}{2},\ 0\right),\ \left(\frac{\sqrt{2}}{2},\ \frac{\sqrt{2}}{2},\ 0\right)$<br>$(1,\ 0,\ 0),\ (0,\ 1,\ 0)$ | $\{1\}\oplus\{2\}$ or $\{3\}\oplus\{4\}$<br>$\{1\}\oplus\{3\}$ or $\{2\}\oplus\{4\}$<br>$\{1\}\oplus\{4\}$ or $\{2\}\oplus\{3\}$ |
| 136 | $\mathrm{S}\left(u,\ u,\ \frac{1}{2}\right)$ | $(0,\ 0,\ 1),\ \left(\frac{\sqrt{2}}{2},\ -\frac{\sqrt{2}}{2},\ 0\right)$ | $\{1\}\oplus\{3\}$ or $\{2\}\oplus\{4\}$ |
| 136 | $\mathrm{SM}(u,\ u,\ 0)$ | $(0,\ 0,\ 1),\ \left(\frac{\sqrt{2}}{2},\ -\frac{\sqrt{2}}{2},\ 0\right)$ | $\{1\}\oplus\{2\}$ or $\{3\}\oplus\{4\}$ |
| 137 | $\mathrm{DT}(0,\ v,\ 0)$ | $(0,\ 0,\ 1),\ (1,\ 0,\ 0)$ | $\{1\}\oplus\{2\}$ or $\{3\}\oplus\{4\}$ |
| 137 | $\mathrm{LD}(0,\ 0,\ w)$ | $(1,\ 0,\ 0),\ (0,\ 1,\ 0),\ \left(\frac{\sqrt{2}}{2},\ -\frac{\sqrt{2}}{2},\ 0\right),\ \left(\frac{\sqrt{2}}{2},\ \frac{\sqrt{2}}{2},\ 0\right)$<br>$\left(\frac{\sqrt{2}}{2},\ -\frac{\sqrt{2}}{2},\ 0\right),\ \left(\frac{\sqrt{2}}{2},\ \frac{\sqrt{2}}{2},\ 0\right)$<br>$(1,\ 0,\ 0),\ (0,\ 1,\ 0)$ | $\{1\}\oplus\{2\}$ or $\{3\}\oplus\{4\}$<br>$\{1\}\oplus\{3\}$ or $\{2\}\oplus\{4\}$<br>$\{1\}\oplus\{4\}$ or $\{2\}\oplus\{3\}$ |
| 137 | $\mathrm{SM}(u,\ u,\ 0)$ | $(0,\ 0,\ 1),\ \left(\frac{\sqrt{2}}{2},\ -\frac{\sqrt{2}}{2},\ 0\right)$ | $\{1\}\oplus\{2\}$ or $\{3\}\oplus\{4\}$ |
| 137 | $\mathrm{U}\left(0,\ v,\ \frac{1}{2}\right)$ | $(0,\ 0,\ 1),\ (1,\ 0,\ 0)$ | $\{1\}\oplus\{2\}$ or $\{3\}\oplus\{4\}$ |
| 138 | $\mathrm{DT}(0,\ v,\ 0)$ | $(0,\ 0,\ 1),\ (1,\ 0,\ 0)$ | $\{1\}\oplus\{2\}$ or $\{3\}\oplus\{4\}$ |
| 138 | $\mathrm{LD}(0,\ 0,\ w)$ | $(1,\ 0,\ 0),\ (0,\ 1,\ 0),\ \left(\frac{\sqrt{2}}{2},\ -\frac{\sqrt{2}}{2},\ 0\right),\ \left(\frac{\sqrt{2}}{2},\ \frac{\sqrt{2}}{2},\ 0\right)$<br>$\left(\frac{\sqrt{2}}{2},\ -\frac{\sqrt{2}}{2},\ 0\right),\ \left(\frac{\sqrt{2}}{2},\ \frac{\sqrt{2}}{2},\ 0\right)$<br>$(1,\ 0,\ 0),\ (0,\ 1,\ 0)$ | $\{1\}\oplus\{2\}$ or $\{3\}\oplus\{4\}$<br>$\{1\}\oplus\{3\}$ or $\{2\}\oplus\{4\}$<br>$\{1\}\oplus\{4\}$ or $\{2\}\oplus\{3\}$ |
| 138 | $\mathrm{S}\left(u,\ u,\ \frac{1}{2}\right)$ | $(0,\ 0,\ 1),\ \left(\frac{\sqrt{2}}{2},\ -\frac{\sqrt{2}}{2},\ 0\right)$ | $\{1\}\oplus\{3\}$ or $\{2\}\oplus\{4\}$ |
| 138 | $\mathrm{SM}(u,\ u,\ 0)$ | $(0,\ 0,\ 1),\ \left(\frac{\sqrt{2}}{2},\ -\frac{\sqrt{2}}{2},\ 0\right)$ | $\{1\}\oplus\{2\}$ or $\{3\}\oplus\{4\}$ |
| 139 | $\mathrm{DT}(u,\ u,\ 0)$ | $\left(\frac{\sqrt{2}}{2},\ -\frac{\sqrt{2}}{2},\ 0\right),\ (0,\ 0,\ -1)$ | $\{1\}\oplus\{2\}$ or $\{3\}\oplus\{4\}$ |
| 139 | $\mathrm{LD}(0,\ 0,\ w)$ | $\left(-\frac{\sqrt{2}}{2},\ -\frac{\sqrt{2}}{2},\ 0\right),\ \left(\frac{\sqrt{2}}{2},\ -\frac{\sqrt{2}}{2},\ 0\right),\ (0,\ 1,\ 0),\ (-1,\ 0,\ 0)$<br>$\left(-\frac{\sqrt{2}}{2},\ -\frac{\sqrt{2}}{2},\ 0\right),\ \left(\frac{\sqrt{2}}{2},\ -\frac{\sqrt{2}}{2},\ 0\right)$<br>$(0,\ 1,\ 0),\ (-1,\ 0,\ 0)$ | $\{1\}\oplus\{2\}$ or $\{3\}\oplus\{4\}$<br>$\{1\}\oplus\{3\}$ or $\{2\}\oplus\{4\}$<br>$\{1\}\oplus\{4\}$ or $\{2\}\oplus\{3\}$ |
| 139 | $\mathrm{SM}(u,\ 0,\ 0)$ | $(0,\ 1,\ 0),\ (0,\ 0,\ -1)$ | $\{1\}\oplus\{2\}$ or $\{3\}\oplus\{4\}$ |
| 139 | $\mathrm{W}\left(\frac{1}{2},\ \frac{1}{2},\ w\right)$ | $\left(-\frac{\sqrt{2}}{2},\ -\frac{\sqrt{2}}{2},\ 0\right),\ \left(\frac{\sqrt{2}}{2},\ -\frac{\sqrt{2}}{2},\ 0\right)$ | $\{1\}\oplus\{2\}$ or $\{3\}\oplus\{4\}$ |
| 139 | $\mathrm{Y}(u,\ 1-u,\ 0)$ | $\left(-\frac{\sqrt{2}}{2},\ -\frac{\sqrt{2}}{2},\ 0\right),\ (0,\ 0,\ -1)$ | $\{1\}\oplus\{2\}$ or $\{3\}\oplus\{4\}$ |
| 140 | $\mathrm{DT}(u,\ u,\ 0)$ | $\left(\frac{\sqrt{2}}{2},\ -\frac{\sqrt{2}}{2},\ 0\right),\ (0,\ 0,\ -1)$ | $\{1\}\oplus\{2\}$ or $\{3\}\oplus\{4\}$ |
| 140 | $\mathrm{LD}(0,\ 0,\ w)$ | $\left(-\frac{\sqrt{2}}{2},\ -\frac{\sqrt{2}}{2},\ 0\right),\ \left(\frac{\sqrt{2}}{2},\ -\frac{\sqrt{2}}{2},\ 0\right),\ (0,\ 1,\ 0),\ (-1,\ 0,\ 0)$<br>$\left(-\frac{\sqrt{2}}{2},\ -\frac{\sqrt{2}}{2},\ 0\right),\ \left(\frac{\sqrt{2}}{2},\ -\frac{\sqrt{2}}{2},\ 0\right)$<br>$(0,\ 1,\ 0),\ (-1,\ 0,\ 0)$ | $\{1\}\oplus\{2\}$ or $\{3\}\oplus\{4\}$<br>$\{1\}\oplus\{3\}$ or $\{2\}\oplus\{4\}$<br>$\{1\}\oplus\{4\}$ or $\{2\}\oplus\{3\}$ |
| 140 | $\mathrm{SM}(u,\ 0,\ 0)$ | $(0,\ 1,\ 0),\ (0,\ 0,\ -1)$ | $\{1\}\oplus\{2\}$ or $\{3\}\oplus\{4\}$ |
| 140 | $\mathrm{W}\left(\frac{1}{2},\ \frac{1}{2},\ w\right)$ | $\left(-\frac{\sqrt{2}}{2},\ -\frac{\sqrt{2}}{2},\ 0\right),\ \left(\frac{\sqrt{2}}{2},\ -\frac{\sqrt{2}}{2},\ 0\right)$ | $\{1\}\oplus\{2\}$ or $\{3\}\oplus\{4\}$ |
| 140 | $\mathrm{Y}(u,\ 1-u,\ 0)$ | $\left(-\frac{\sqrt{2}}{2},\ -\frac{\sqrt{2}}{2},\ 0\right),\ (0,\ 0,\ -1)$ | $\{1\}\oplus\{2\}$ or $\{3\}\oplus\{4\}$ |

| SG | HSL | Location of nodal chain | Irreps of BC |
|---|---|---|---|
| 141 | DT$(u, u, 0)$ | $\left(\frac{\sqrt{2}}{2}, -\frac{\sqrt{2}}{2}, 0\right), (0, 0, -1)$ | $\{1\}\oplus\{2\}$ or $\{3\}\oplus\{4\}$ |
| 141 | LD$(0, 0, w)$ | $\left(-\frac{\sqrt{2}}{2}, -\frac{\sqrt{2}}{2}, 0\right), \left(\frac{\sqrt{2}}{2}, -\frac{\sqrt{2}}{2}, 0\right), (0, 1, 0), (-1, 0, 0)$<br>$\left(-\frac{\sqrt{2}}{2}, -\frac{\sqrt{2}}{2}, 0\right), \left(\frac{\sqrt{2}}{2}, -\frac{\sqrt{2}}{2}, 0\right)$<br>$(0, 1, 0), (-1, 0, 0)$ | $\{1\}\oplus\{2\}$ or $\{3\}\oplus\{4\}$<br>$\{1\}\oplus\{3\}$ or $\{2\}\oplus\{4\}$<br>$\{1\}\oplus\{4\}$ or $\{2\}\oplus\{3\}$ |
| 141 | SM$(u, 0, 0)$ | $(0, 1, 0), (0, 0, -1)$ | $\{1\}\oplus\{2\}$ or $\{3\}\oplus\{4\}$ |
| 142 | DT$(u, u, 0)$ | $\left(-\frac{\sqrt{2}}{2}, \frac{\sqrt{2}}{2}, 0\right), (0, 0, -1)$ | $\{1\}\oplus\{2\}$ or $\{3\}\oplus\{4\}$ |
| 142 | LD$(0, 0, w)$ | $\left(\frac{\sqrt{2}}{2}, \frac{\sqrt{2}}{2}, 0\right), \left(-\frac{\sqrt{2}}{2}, \frac{\sqrt{2}}{2}, 0\right), (0, -1, 0), (1, 0, 0)$<br>$\left(\frac{\sqrt{2}}{2}, \frac{\sqrt{2}}{2}, 0\right), \left(-\frac{\sqrt{2}}{2}, \frac{\sqrt{2}}{2}, 0\right)$<br>$(0, -1, 0), (1, 0, 0)$ | $\{1\}\oplus\{2\}$ or $\{3\}\oplus\{4\}$<br>$\{1\}\oplus\{3\}$ or $\{2\}\oplus\{4\}$<br>$\{1\}\oplus\{4\}$ or $\{2\}\oplus\{3\}$ |
| 142 | SM$(u, 0, 0)$ | $(0, -1, 0), (0, 0, -1)$ | $\{1\}\oplus\{2\}$ or $\{3\}\oplus\{4\}$ |
| 156 | DT$(0, 0, w)$ | $(1, 0, 0), \left(-\frac{1}{2}, \frac{\sqrt{3}}{2}, 0\right)$ | $1\oplus2$ |
| 157 | DT$(0, 0, w)$ | $\left(-\frac{\sqrt{3}}{2}, -\frac{1}{2}, 0\right), \left(\frac{\sqrt{3}}{2}, -\frac{1}{2}, 0\right)$ | $1\oplus2$ |
| 157 | PA$\left(-\frac{1}{3}, -\frac{1}{3}, -w\right)$ | $\left(-\frac{\sqrt{3}}{2}, -\frac{1}{2}, 0\right), \left(\frac{\sqrt{3}}{2}, -\frac{1}{2}, 0\right)$ | $1\oplus2$ |
| 157 | P$\left(\frac{1}{3}, \frac{1}{3}, w\right)$ | $\left(-\frac{\sqrt{3}}{2}, -\frac{1}{2}, 0\right), \left(\frac{\sqrt{3}}{2}, -\frac{1}{2}, 0\right)$ | $1\oplus2$ |
| 158 | DT$(0, 0, w)$ | $(1, 0, 0), \left(-\frac{1}{2}, \frac{\sqrt{3}}{2}, 0\right)$ | $1\oplus2$ |
| 159 | DT$(0, 0, w)$ | $\left(-\frac{\sqrt{3}}{2}, -\frac{1}{2}, 0\right), \left(\frac{\sqrt{3}}{2}, -\frac{1}{2}, 0\right)$ | $1\oplus2$ |
| 159 | PA$\left(-\frac{1}{3}, -\frac{1}{3}, -w\right)$ | $\left(-\frac{\sqrt{3}}{2}, -\frac{1}{2}, 0\right), \left(\frac{\sqrt{3}}{2}, -\frac{1}{2}, 0\right)$ | $1\oplus2$ |
| 159 | P$\left(\frac{1}{3}, \frac{1}{3}, w\right)$ | $\left(-\frac{\sqrt{3}}{2}, -\frac{1}{2}, 0\right), \left(\frac{\sqrt{3}}{2}, -\frac{1}{2}, 0\right)$ | $1\oplus2$ |
| 160 | LD$\left(\frac{w}{3}, \frac{w}{3}, \frac{w}{3}\right)$ | $\left(\frac{1}{2}, -\frac{\sqrt{3}}{2}, 0\right), \left(\frac{1}{2}, \frac{\sqrt{3}}{2}, 0\right)$ | $1\oplus2$ |
| 161 | LD$\left(\frac{w}{3}, \frac{w}{3}, \frac{w}{3}\right)$ | $\left(\frac{1}{2}, -\frac{\sqrt{3}}{2}, 0\right), \left(\frac{1}{2}, \frac{\sqrt{3}}{2}, 0\right)$ | $1\oplus2$ |
| 162 | DT$(0, 0, w)$ | $\left(-\frac{\sqrt{3}}{2}, -\frac{1}{2}, 0\right), \left(\frac{\sqrt{3}}{2}, -\frac{1}{2}, 0\right)$ | $\{1\}\oplus\{2\}$ |
| 162 | P$\left(\frac{1}{3}, \frac{1}{3}, w\right)$ | $\left(-\frac{\sqrt{3}}{2}, -\frac{1}{2}, 0\right), \left(\frac{\sqrt{3}}{2}, -\frac{1}{2}, 0\right)$ | $\{1\}\oplus\{2\}$ |
| 163 | DT$(0, 0, w)$ | $\left(-\frac{\sqrt{3}}{2}, -\frac{1}{2}, 0\right), \left(\frac{\sqrt{3}}{2}, -\frac{1}{2}, 0\right)$ | $\{1\}\oplus\{2\}$ |
| 163 | P$\left(\frac{1}{3}, \frac{1}{3}, w\right)$ | $\left(-\frac{\sqrt{3}}{2}, -\frac{1}{2}, 0\right), \left(\frac{\sqrt{3}}{2}, -\frac{1}{2}, 0\right)$ | $\{1\}\oplus\{2\}$ |
| 164 | DT$(0, 0, w)$ | $(1, 0, 0), \left(-\frac{1}{2}, \frac{\sqrt{3}}{2}, 0\right)$ | $\{1\}\oplus\{2\}$ |
| 165 | DT$(0, 0, w)$ | $(1, 0, 0), \left(-\frac{1}{2}, \frac{\sqrt{3}}{2}, 0\right)$ | $\{1\}\oplus\{2\}$ |
| 166 | LD$\left(\frac{w}{3}, \frac{w}{3}, \frac{w}{3}\right)$ | $\left(\frac{1}{2}, -\frac{\sqrt{3}}{2}, 0\right), \left(\frac{1}{2}, \frac{\sqrt{3}}{2}, 0\right)$ | $\{1\}\oplus\{2\}$ |
| 167 | LD$\left(\frac{w}{3}, \frac{w}{3}, \frac{w}{3}\right)$ | $\left(\frac{1}{2}, -\frac{\sqrt{3}}{2}, 0\right), \left(\frac{1}{2}, \frac{\sqrt{3}}{2}, 0\right)$ | $\{1\}\oplus\{2\}$ |
| 183 | DT$(0, 0, w)$ | $(1, 0, 0), \left(\frac{1}{2}, \frac{\sqrt{3}}{2}, 0\right), \left(\frac{1}{2}, -\frac{\sqrt{3}}{2}, 0\right), \left(-\frac{\sqrt{3}}{2}, -\frac{1}{2}, 0\right), (0, -1, 0), \left(-\frac{\sqrt{3}}{2}, \frac{1}{2}, 0\right)$<br>$\left(-\frac{\sqrt{3}}{2}, -\frac{1}{2}, 0\right), (0, -1, 0), \left(-\frac{\sqrt{3}}{2}, \frac{1}{2}, 0\right)$<br>$(1, 0, 0), \left(\frac{1}{2}, \frac{\sqrt{3}}{2}, 0\right), \left(\frac{1}{2}, -\frac{\sqrt{3}}{2}, 0\right)$ | $1\oplus2$ or $3\oplus4$<br>$1\oplus3$ or $2\oplus4$<br>$1\oplus4$ or $2\oplus3$ |
| 183 | P$\left(\frac{1}{3}, \frac{1}{3}, w\right)$ | $\left(-\frac{\sqrt{3}}{2}, -\frac{1}{2}, 0\right), (0, -1, 0)$ | $1\oplus2$ |
| 183 | U$\left(\frac{1}{2}, 0, w\right)$ | $\left(\frac{1}{2}, -\frac{\sqrt{3}}{2}, 0\right), \left(-\frac{\sqrt{3}}{2}, -\frac{1}{2}, 0\right)$ | $1\oplus2$ or $3\oplus4$ |
| 184 | DT$(0, 0, w)$ | $(1, 0, 0), \left(\frac{1}{2}, \frac{\sqrt{3}}{2}, 0\right), \left(\frac{1}{2}, -\frac{\sqrt{3}}{2}, 0\right), \left(-\frac{\sqrt{3}}{2}, -\frac{1}{2}, 0\right), (0, -1, 0), \left(-\frac{\sqrt{3}}{2}, \frac{1}{2}, 0\right)$<br>$\left(-\frac{\sqrt{3}}{2}, -\frac{1}{2}, 0\right), (0, -1, 0), \left(-\frac{\sqrt{3}}{2}, \frac{1}{2}, 0\right)$<br>$(1, 0, 0), \left(\frac{1}{2}, \frac{\sqrt{3}}{2}, 0\right), \left(\frac{1}{2}, -\frac{\sqrt{3}}{2}, 0\right)$ | $1\oplus2$ or $3\oplus4$<br>$1\oplus3$ or $2\oplus4$<br>$1\oplus4$ or $2\oplus3$ |
| 184 | P$\left(\frac{1}{3}, \frac{1}{3}, w\right)$ | $\left(-\frac{\sqrt{3}}{2}, -\frac{1}{2}, 0\right), (0, -1, 0)$ | $1\oplus2$ |
| 184 | U$\left(\frac{1}{2}, 0, w\right)$ | $\left(\frac{1}{2}, -\frac{\sqrt{3}}{2}, 0\right), \left(-\frac{\sqrt{3}}{2}, -\frac{1}{2}, 0\right)$ | $1\oplus2$ or $3\oplus4$ |

| SG | HSL | Location of nodal chain | Irreps of BC |
|---|---|---|---|
| 185 | DT$(0, 0, w)$ | $(1, 0, 0), \left(\frac{1}{2}, \frac{\sqrt{3}}{2}, 0\right), \left(\frac{1}{2}, -\frac{\sqrt{3}}{2}, 0\right), \left(-\frac{\sqrt{3}}{2}, -\frac{1}{2}, 0\right), (0, -1, 0), \left(-\frac{\sqrt{3}}{2}, \frac{1}{2}, 0\right)$<br>$\left(-\frac{\sqrt{3}}{2}, -\frac{1}{2}, 0\right), (0, -1, 0), \left(-\frac{\sqrt{3}}{2}, \frac{1}{2}, 0\right)$<br>$(1, 0, 0), \left(\frac{1}{2}, \frac{\sqrt{3}}{2}, 0\right), \left(\frac{1}{2}, -\frac{\sqrt{3}}{2}, 0\right)$ | $1\oplus2$ or $3\oplus4$<br>$1\oplus3$ or $2\oplus4$<br>$1\oplus4$ or $2\oplus3$ |
| 185 | P$\left(\frac{1}{3}, \frac{1}{3}, w\right)$ | $\left(-\frac{\sqrt{3}}{2}, -\frac{1}{2}, 0\right), (0, -1, 0)$ | $1\oplus2$ |
| 185 | U$\left(\frac{1}{2}, 0, w\right)$ | $\left(\frac{1}{2}, -\frac{\sqrt{3}}{2}, 0\right), \left(-\frac{\sqrt{3}}{2}, -\frac{1}{2}, 0\right)$ | $1\oplus2$ or $3\oplus4$ |
| 186 | DT$(0, 0, w)$ | $(1, 0, 0), \left(\frac{1}{2}, \frac{\sqrt{3}}{2}, 0\right), \left(\frac{1}{2}, -\frac{\sqrt{3}}{2}, 0\right), \left(-\frac{\sqrt{3}}{2}, -\frac{1}{2}, 0\right), (0, -1, 0), \left(-\frac{\sqrt{3}}{2}, \frac{1}{2}, 0\right)$<br>$\left(-\frac{\sqrt{3}}{2}, -\frac{1}{2}, 0\right), (0, -1, 0), \left(-\frac{\sqrt{3}}{2}, \frac{1}{2}, 0\right)$<br>$(1, 0, 0), \left(\frac{1}{2}, \frac{\sqrt{3}}{2}, 0\right), \left(\frac{1}{2}, -\frac{\sqrt{3}}{2}, 0\right)$ | $1\oplus2$ or $3\oplus4$<br>$1\oplus3$ or $2\oplus4$<br>$1\oplus4$ or $2\oplus3$ |
| 186 | P$\left(\frac{1}{3}, \frac{1}{3}, w\right)$ | $\left(-\frac{\sqrt{3}}{2}, -\frac{1}{2}, 0\right), (0, -1, 0)$ | $1\oplus2$ |
| 186 | U$\left(\frac{1}{2}, 0, w\right)$ | $\left(\frac{1}{2}, -\frac{\sqrt{3}}{2}, 0\right), \left(-\frac{\sqrt{3}}{2}, -\frac{1}{2}, 0\right)$ | $1\oplus2$ or $3\oplus4$ |
| 187 | DT$(0, 0, w)$ | $(1, 0, 0), \left(-\frac{1}{2}, \frac{\sqrt{3}}{2}, 0\right)$ | $\{1\}\oplus\{2\}$ |
| 187 | R$\left(u, 0, \frac{1}{2}\right)$ | $\left(-\frac{1}{2}, \frac{\sqrt{3}}{2}, 0\right), (0, 0, 1)$ | $1\oplus2$ or $3\oplus4$ |
| 187 | SM$(u, 0, 0)$ | $\left(-\frac{1}{2}, \frac{\sqrt{3}}{2}, 0\right), (0, 0, 1)$ | $1\oplus2$ or $3\oplus4$ |
| 188 | DT$(0, 0, w)$ | $(1, 0, 0), \left(-\frac{1}{2}, \frac{\sqrt{3}}{2}, 0\right)$ | $\{1\}\oplus\{2\}$ |
| 188 | SM$(u, 0, 0)$ | $\left(-\frac{1}{2}, \frac{\sqrt{3}}{2}, 0\right), (0, 0, 1)$ | $1\oplus2$ or $3\oplus4$ |
| 189 | DT$(0, 0, w)$ | $\left(-\frac{\sqrt{3}}{2}, -\frac{1}{2}, 0\right), \left(\frac{\sqrt{3}}{2}, -\frac{1}{2}, 0\right)$ | $\{1\}\oplus\{2\}$ |
| 189 | LD$(u, u, 0)$ | $(0, 0, 1), \left(\frac{\sqrt{3}}{2}, -\frac{1}{2}, 0\right)$ | $1\oplus2$ or $3\oplus4$ |
| 189 | PA$\left(-\frac{1}{3}, -\frac{1}{3}, -w\right)$ | $\left(-\frac{\sqrt{3}}{2}, -\frac{1}{2}, 0\right), \left(\frac{\sqrt{3}}{2}, -\frac{1}{2}, 0\right)$ | $1\oplus2$ |
| 189 | Q$\left(u, u, \frac{1}{2}\right)$ | $\left(\frac{\sqrt{3}}{2}, -\frac{1}{2}, 0\right), (0, 0, 1)$ | $1\oplus2$ or $3\oplus4$ |
| 190 | DT$(0, 0, w)$ | $\left(-\frac{\sqrt{3}}{2}, -\frac{1}{2}, 0\right), \left(\frac{\sqrt{3}}{2}, -\frac{1}{2}, 0\right)$ | $\{1\}\oplus\{2\}$ |
| 190 | LD$(u, u, 0)$ | $(0, 0, 1), \left(\frac{\sqrt{3}}{2}, -\frac{1}{2}, 0\right)$ | $1\oplus2$ or $3\oplus4$ |
| 190 | PA$\left(-\frac{1}{3}, -\frac{1}{3}, -w\right)$ | $\left(-\frac{\sqrt{3}}{2}, -\frac{1}{2}, 0\right), \left(\frac{\sqrt{3}}{2}, -\frac{1}{2}, 0\right)$ | $1\oplus2$ |
| 191 | DT$(0, 0, w)$ | $(1, 0, 0), \left(\frac{1}{2}, \frac{\sqrt{3}}{2}, 0\right), \left(\frac{1}{2}, -\frac{\sqrt{3}}{2}, 0\right), \left(-\frac{\sqrt{3}}{2}, -\frac{1}{2}, 0\right), (0, -1, 0), \left(-\frac{\sqrt{3}}{2}, \frac{1}{2}, 0\right)$<br>$\left(-\frac{\sqrt{3}}{2}, -\frac{1}{2}, 0\right), (0, -1, 0), \left(-\frac{\sqrt{3}}{2}, \frac{1}{2}, 0\right)$<br>$(1, 0, 0), \left(\frac{1}{2}, \frac{\sqrt{3}}{2}, 0\right), \left(\frac{1}{2}, -\frac{\sqrt{3}}{2}, 0\right)$ | $\{1\}\oplus\{2\}$ or $\{3\}\oplus\{4\}$<br>$\{1\}\oplus\{3\}$ or $\{2\}\oplus\{4\}$<br>$\{1\}\oplus\{4\}$ or $\{2\}\oplus\{3\}$ |
| 191 | LD$(u, u, 0)$ | $(0, 0, 1), \left(-\frac{\sqrt{3}}{2}, \frac{1}{2}, 0\right)$ | $\{1\}\oplus\{2\}$ or $\{3\}\oplus\{4\}$ |
| 191 | P$\left(\frac{1}{3}, \frac{1}{3}, w\right)$ | $\left(-\frac{\sqrt{3}}{2}, -\frac{1}{2}, 0\right), (0, -1, 0)$ | $\{1\}\oplus\{2\}$ |
| 191 | Q$\left(u, u, \frac{1}{2}\right)$ | $\left(-\frac{\sqrt{3}}{2}, \frac{1}{2}, 0\right), (0, 0, 1)$ | $\{1\}\oplus\{2\}$ or $\{3\}\oplus\{4\}$ |
| 191 | R$\left(u, 0, \frac{1}{2}\right)$ | $\left(\frac{1}{2}, -\frac{\sqrt{3}}{2}, 0\right), (0, 0, 1)$ | $\{1\}\oplus\{2\}$ or $\{3\}\oplus\{4\}$ |
| 191 | SM$(u, 0, 0)$ | $\left(\frac{1}{2}, -\frac{\sqrt{3}}{2}, 0\right), (0, 0, 1)$ | $\{1\}\oplus\{2\}$ or $\{3\}\oplus\{4\}$ |
| 191 | U$\left(\frac{1}{2}, 0, w\right)$ | $\left(\frac{1}{2}, -\frac{\sqrt{3}}{2}, 0\right), \left(-\frac{\sqrt{3}}{2}, -\frac{1}{2}, 0\right)$ | $\{1\}\oplus\{2\}$ or $\{3\}\oplus\{4\}$ |
| 192 | DT$(0, 0, w)$ | $(1, 0, 0), \left(\frac{1}{2}, \frac{\sqrt{3}}{2}, 0\right), \left(\frac{1}{2}, -\frac{\sqrt{3}}{2}, 0\right), \left(-\frac{\sqrt{3}}{2}, -\frac{1}{2}, 0\right), (0, -1, 0), \left(-\frac{\sqrt{3}}{2}, \frac{1}{2}, 0\right)$<br>$\left(-\frac{\sqrt{3}}{2}, -\frac{1}{2}, 0\right), (0, -1, 0), \left(-\frac{\sqrt{3}}{2}, \frac{1}{2}, 0\right)$<br>$(1, 0, 0), \left(\frac{1}{2}, \frac{\sqrt{3}}{2}, 0\right), \left(\frac{1}{2}, -\frac{\sqrt{3}}{2}, 0\right)$ | $\{1\}\oplus\{2\}$ or $\{3\}\oplus\{4\}$<br>$\{1\}\oplus\{3\}$ or $\{2\}\oplus\{4\}$<br>$\{1\}\oplus\{4\}$ or $\{2\}\oplus\{3\}$ |
| 192 | LD$(u, u, 0)$ | $(0, 0, 1), \left(-\frac{\sqrt{3}}{2}, \frac{1}{2}, 0\right)$ | $\{1\}\oplus\{2\}$ or $\{3\}\oplus\{4\}$ |
| 192 | P$\left(\frac{1}{3}, \frac{1}{3}, w\right)$ | $\left(-\frac{\sqrt{3}}{2}, -\frac{1}{2}, 0\right), (0, -1, 0)$ | $\{1\}\oplus\{2\}$ |
| 192 | SM$(u, 0, 0)$ | $\left(\frac{1}{2}, -\frac{\sqrt{3}}{2}, 0\right), (0, 0, 1)$ | $\{1\}\oplus\{2\}$ or $\{3\}\oplus\{4\}$ |
| 192 | U$\left(\frac{1}{2}, 0, w\right)$ | $\left(\frac{1}{2}, -\frac{\sqrt{3}}{2}, 0\right), \left(-\frac{\sqrt{3}}{2}, -\frac{1}{2}, 0\right)$ | $\{1\}\oplus\{2\}$ or $\{3\}\oplus\{4\}$ |

| SG | HSL | Location of nodal chain | Irreps of BC |
|---|---|---|---|
| 193 | DT$(0,\ 0,\ w)$ | $(1,\ 0,\ 0)$, $\left(\frac{1}{2},\ \frac{\sqrt{3}}{2},\ 0\right)$, $\left(\frac{1}{2},\ -\frac{\sqrt{3}}{2},\ 0\right)$, $\left(-\frac{\sqrt{3}}{2},\ -\frac{1}{2},\ 0\right)$, $(0,\ -1,\ 0)$, $\left(-\frac{\sqrt{3}}{2},\ \frac{1}{2},\ 0\right)$<br>$\left(-\frac{\sqrt{3}}{2},\ -\frac{1}{2},\ 0\right)$, $(0,\ -1,\ 0)$, $\left(-\frac{\sqrt{3}}{2},\ \frac{1}{2},\ 0\right)$<br>$(1,\ 0,\ 0)$, $\left(\frac{1}{2},\ \frac{\sqrt{3}}{2},\ 0\right)$, $\left(\frac{1}{2},\ -\frac{\sqrt{3}}{2},\ 0\right)$ | $\{1\}\oplus\{2\}$ or $\{3\}\oplus\{4\}$<br>$\{1\}\oplus\{3\}$ or $\{2\}\oplus\{4\}$<br>$\{1\}\oplus\{4\}$ or $\{2\}\oplus\{3\}$ |
| 193 | LD$(u,\ u,\ 0)$ | $(0,\ 0,\ 1)$, $\left(-\frac{\sqrt{3}}{2},\ \frac{1}{2},\ 0\right)$ | $\{1\}\oplus\{2\}$ or $\{3\}\oplus\{4\}$ |
| 193 | P$\left(\frac{1}{3},\ \frac{1}{3},\ w\right)$ | $\left(-\frac{\sqrt{3}}{2},\ -\frac{1}{2},\ 0\right)$, $(0,\ -1,\ 0)$ | $\{1\}\oplus\{2\}$ |
| 193 | SM$(u,\ 0,\ 0)$ | $\left(\frac{1}{2},\ -\frac{\sqrt{3}}{2},\ 0\right)$, $(0,\ 0,\ 1)$ | $\{1\}\oplus\{2\}$ or $\{3\}\oplus\{4\}$ |
| 193 | U$\left(\frac{1}{2},\ 0,\ w\right)$ | $\left(\frac{1}{2},\ -\frac{\sqrt{3}}{2},\ 0\right)$, $\left(-\frac{\sqrt{3}}{2},\ -\frac{1}{2},\ 0\right)$ | $\{1\}\oplus\{2\}$ or $\{3\}\oplus\{4\}$ |
| 194 | DT$(0,\ 0,\ w)$ | $(1,\ 0,\ 0)$, $\left(\frac{1}{2},\ \frac{\sqrt{3}}{2},\ 0\right)$, $\left(\frac{1}{2},\ -\frac{\sqrt{3}}{2},\ 0\right)$, $\left(-\frac{\sqrt{3}}{2},\ -\frac{1}{2},\ 0\right)$, $(0,\ -1,\ 0)$, $\left(-\frac{\sqrt{3}}{2},\ \frac{1}{2},\ 0\right)$<br>$\left(-\frac{\sqrt{3}}{2},\ -\frac{1}{2},\ 0\right)$, $(0,\ -1,\ 0)$, $\left(-\frac{\sqrt{3}}{2},\ \frac{1}{2},\ 0\right)$<br>$(1,\ 0,\ 0)$, $\left(\frac{1}{2},\ \frac{\sqrt{3}}{2},\ 0\right)$, $\left(\frac{1}{2},\ -\frac{\sqrt{3}}{2},\ 0\right)$ | $\{1\}\oplus\{2\}$ or $\{3\}\oplus\{4\}$<br>$\{1\}\oplus\{3\}$ or $\{2\}\oplus\{4\}$<br>$\{1\}\oplus\{4\}$ or $\{2\}\oplus\{3\}$ |
| 194 | LD$(u,\ u,\ 0)$ | $(0,\ 0,\ 1)$, $\left(-\frac{\sqrt{3}}{2},\ \frac{1}{2},\ 0\right)$ | $\{1\}\oplus\{2\}$ or $\{3\}\oplus\{4\}$ |
| 194 | P$\left(\frac{1}{3},\ \frac{1}{3},\ w\right)$ | $\left(-\frac{\sqrt{3}}{2},\ -\frac{1}{2},\ 0\right)$, $(0,\ -1,\ 0)$ | $\{1\}\oplus\{2\}$ |
| 194 | SM$(u,\ 0,\ 0)$ | $\left(\frac{1}{2},\ -\frac{\sqrt{3}}{2},\ 0\right)$, $(0,\ 0,\ 1)$ | $\{1\}\oplus\{2\}$ or $\{3\}\oplus\{4\}$ |
| 194 | U$\left(\frac{1}{2},\ 0,\ w\right)$ | $\left(\frac{1}{2},\ -\frac{\sqrt{3}}{2},\ 0\right)$, $\left(-\frac{\sqrt{3}}{2},\ -\frac{1}{2},\ 0\right)$ | $\{1\}\oplus\{2\}$ or $\{3\}\oplus\{4\}$ |
| 200 | DT$(0,\ v,\ 0)$ | $(0,\ 0,\ 1)$, $(1,\ 0,\ 0)$ | $\{1\}\oplus\{2\}$ or $\{3\}\oplus\{4\}$ |
| 200 | T$\left(\frac{1}{2},\ \frac{1}{2},\ w\right)$ | $(0,\ -1,\ 0)$, $(-1,\ 0,\ 0)$ | $\{1\}\oplus\{2\}$ or $\{3\}\oplus\{4\}$ |
| 200 | ZA$\left(\frac{1}{2},\ u,\ 0\right)$ | $(0,\ 0,\ 1)$, $(-1,\ 0,\ 0)$ | $\{1\}\oplus\{2\}$ or $\{3\}\oplus\{4\}$ |
| 200 | Z$\left(u,\ \frac{1}{2},\ 0\right)$ | $(0,\ 0,\ 1)$, $(0,\ -1,\ 0)$ | $\{1\}\oplus\{2\}$ or $\{3\}\oplus\{4\}$ |
| 201 | DT$(0,\ v,\ 0)$ | $(0,\ 0,\ 1)$, $(1,\ 0,\ 0)$ | $\{1\}\oplus\{2\}$ or $\{3\}\oplus\{4\}$ |
| 201 | T$\left(\frac{1}{2},\ \frac{1}{2},\ w\right)$ | $(0,\ -1,\ 0)$, $(-1,\ 0,\ 0)$ | $\{1\}\oplus\{2\}$ or $\{3\}\oplus\{4\}$ |
| 202 | DT$(0,\ v,\ 0)$ | $(0,\ 0,\ -1)$, $(-1,\ 0,\ 0)$ | $\{1\}\oplus\{2\}$ or $\{3\}\oplus\{4\}$ |
| 202 | V$(u,\ 1,\ 0)$ | $(0,\ 0,\ -1)$, $(0,\ -1,\ 0)$ | $\{1\}\oplus\{2\}$ or $\{3\}\oplus\{4\}$ |
| 203 | DT$(0,\ v,\ 0)$ | $(0,\ 0,\ -1)$, $(-1,\ 0,\ 0)$ | $\{1\}\oplus\{2\}$ or $\{3\}\oplus\{4\}$ |
| 204 | DT$(0,\ v,\ 0)$ | $(0,\ 0,\ -1)$, $(-1,\ 0,\ 0)$ | $\{1\}\oplus\{2\}$ or $\{3\}\oplus\{4\}$ |
| 205 | DT$(0,\ v,\ 0)$ | $(0,\ 0,\ 1)$, $(1,\ 0,\ 0)$ | $\{1\}\oplus\{2\}$ or $\{3\}\oplus\{4\}$ |
| 206 | DT$(0,\ v,\ 0)$ | $(0,\ 0,\ -1)$, $(-1,\ 0,\ 0)$ | $\{1\}\oplus\{2\}$ or $\{3\}\oplus\{4\}$ |
| 215 | DT$(0,\ v,\ 0)$ | $\left(-\frac{\sqrt{2}}{2},\ 0,\ \frac{\sqrt{2}}{2}\right)$, $\left(-\frac{\sqrt{2}}{2},\ 0,\ -\frac{\sqrt{2}}{2}\right)$ | $\{1\}\oplus\{2\}$ |
| 215 | LD$(u,\ u,\ u)$ | $\left(\frac{\sqrt{2}}{2},\ -\frac{\sqrt{2}}{2},\ 0\right)$, $\left(0,\ \frac{\sqrt{2}}{2},\ -\frac{\sqrt{2}}{2}\right)$ | $1\oplus2$ |
| 215 | T$\left(\frac{1}{2},\ \frac{1}{2},\ w\right)$ | $\left(\frac{\sqrt{2}}{2},\ -\frac{\sqrt{2}}{2},\ 0\right)$, $\left(\frac{\sqrt{2}}{2},\ \frac{\sqrt{2}}{2},\ 0\right)$ | $\{1\}\oplus\{2\}$ |
| 216 | DT$(0,\ v,\ 0)$ | $\left(\frac{\sqrt{2}}{2},\ 0,\ -\frac{\sqrt{2}}{2}\right)$, $\left(\frac{\sqrt{2}}{2},\ 0,\ \frac{\sqrt{2}}{2}\right)$ | $\{1\}\oplus\{2\}$ |
| 216 | LD$(u,\ u,\ u)$ | $\left(-\frac{\sqrt{2}}{2},\ \frac{\sqrt{2}}{2},\ 0\right)$, $\left(0,\ -\frac{\sqrt{2}}{2},\ \frac{\sqrt{2}}{2}\right)$ | $1\oplus2$ |
| 217 | D$\left(\frac{1}{2},\ \frac{1}{2},\ w\right)$ | $\left(-\frac{\sqrt{2}}{2},\ \frac{\sqrt{2}}{2},\ 0\right)$, $\left(-\frac{\sqrt{2}}{2},\ -\frac{\sqrt{2}}{2},\ 0\right)$ | $1\oplus2$ or $3\oplus4$ |
| 217 | DT$(0,\ v,\ 0)$ | $\left(\frac{\sqrt{2}}{2},\ 0,\ -\frac{\sqrt{2}}{2}\right)$, $\left(\frac{\sqrt{2}}{2},\ 0,\ \frac{\sqrt{2}}{2}\right)$ | $\{1\}\oplus\{2\}$ |
| 217 | LD$(u,\ u,\ u)$ | $\left(-\frac{\sqrt{2}}{2},\ \frac{\sqrt{2}}{2},\ 0\right)$, $\left(0,\ -\frac{\sqrt{2}}{2},\ \frac{\sqrt{2}}{2}\right)$ | $1\oplus2$ |
| 218 | DT$(0,\ v,\ 0)$ | $\left(-\frac{\sqrt{2}}{2},\ 0,\ \frac{\sqrt{2}}{2}\right)$, $\left(-\frac{\sqrt{2}}{2},\ 0,\ -\frac{\sqrt{2}}{2}\right)$ | $\{1\}\oplus\{2\}$ |
| 218 | LD$(u,\ u,\ u)$ | $\left(\frac{\sqrt{2}}{2},\ -\frac{\sqrt{2}}{2},\ 0\right)$, $\left(0,\ \frac{\sqrt{2}}{2},\ -\frac{\sqrt{2}}{2}\right)$ | $1\oplus2$ |
| 218 | T$\left(\frac{1}{2},\ \frac{1}{2},\ w\right)$ | $\left(\frac{\sqrt{2}}{2},\ -\frac{\sqrt{2}}{2},\ 0\right)$, $\left(\frac{\sqrt{2}}{2},\ \frac{\sqrt{2}}{2},\ 0\right)$ | $\{3\}\oplus\{4\}$ |
| 219 | DT$(0,\ v,\ 0)$ | $\left(\frac{\sqrt{2}}{2},\ 0,\ -\frac{\sqrt{2}}{2}\right)$, $\left(\frac{\sqrt{2}}{2},\ 0,\ \frac{\sqrt{2}}{2}\right)$ | $\{1\}\oplus\{2\}$ |
| 219 | LD$(u,\ u,\ u)$ | $\left(-\frac{\sqrt{2}}{2},\ \frac{\sqrt{2}}{2},\ 0\right)$, $\left(0,\ -\frac{\sqrt{2}}{2},\ \frac{\sqrt{2}}{2}\right)$ | $1\oplus2$ |

| SG | HSL | Location of nodal chain | Irreps of BC |
|---|---|---|---|
| 220 | DT$(0,\ v,\ 0)$ | $\left(\frac{\sqrt{2}}{2},\ 0,\ -\frac{\sqrt{2}}{2}\right),\ \left(\frac{\sqrt{2}}{2},\ 0,\ \frac{\sqrt{2}}{2}\right)$ | $\{1\}\oplus\{2\}$ |
| 220 | LD$(u,\ u,\ u)$ | $\left(-\frac{\sqrt{2}}{2},\ \frac{\sqrt{2}}{2},\ 0\right),\ \left(0,\ -\frac{\sqrt{2}}{2},\ \frac{\sqrt{2}}{2}\right)$ | $1\oplus2$ |
| 221 | DT$(0,\ v,\ 0)$ | $\left(-\frac{\sqrt{2}}{2},\ 0,\ \frac{\sqrt{2}}{2}\right),\ \left(-\frac{\sqrt{2}}{2},\ 0,\ -\frac{\sqrt{2}}{2}\right),\ (0,\ 0,\ 1),\ (1,\ 0,\ 0)$<br>$\left(-\frac{\sqrt{2}}{2},\ 0,\ \frac{\sqrt{2}}{2}\right),\ \left(-\frac{\sqrt{2}}{2},\ 0,\ -\frac{\sqrt{2}}{2}\right)$<br>$(0,\ 0,\ 1),\ (1,\ 0,\ 0)$ | $\{1\}\oplus\{2\}$ or $\{3\}\oplus\{4\}$<br>$\{1\}\oplus\{3\}$ or $\{2\}\oplus\{4\}$<br>$\{1\}\oplus\{4\}$ or $\{2\}\oplus\{3\}$ |
| 221 | LD$(u,\ u,\ u)$ | $\left(\frac{\sqrt{2}}{2},\ -\frac{\sqrt{2}}{2},\ 0\right),\ \left(0,\ \frac{\sqrt{2}}{2},\ -\frac{\sqrt{2}}{2}\right)$ | $\{1\}\oplus\{2\}$ |
| 221 | S$\left(u,\ \frac{1}{2},\ u\right)$ | $\left(-\frac{\sqrt{2}}{2},\ 0,\ \frac{\sqrt{2}}{2}\right),\ (0,\ -1,\ 0)$ | $\{1\}\oplus\{2\}$ or $\{3\}\oplus\{4\}$ |
| 221 | SM$(u,\ u,\ 0)$ | $\left(\frac{\sqrt{2}}{2},\ -\frac{\sqrt{2}}{2},\ 0\right),\ (0,\ 0,\ 1)$ | $\{1\}\oplus\{2\}$ or $\{3\}\oplus\{4\}$ |
| 221 | T$\left(\frac{1}{2},\ \frac{1}{2},\ w\right)$ | $\left(\frac{\sqrt{2}}{2},\ -\frac{\sqrt{2}}{2},\ 0\right),\ \left(\frac{\sqrt{2}}{2},\ \frac{\sqrt{2}}{2},\ 0\right),\ (0,\ -1,\ 0),\ (-1,\ 0,\ 0)$<br>$\left(\frac{\sqrt{2}}{2},\ -\frac{\sqrt{2}}{2},\ 0\right),\ \left(\frac{\sqrt{2}}{2},\ \frac{\sqrt{2}}{2},\ 0\right)$<br>$(0,\ -1,\ 0),\ (-1,\ 0,\ 0)$ | $\{1\}\oplus\{2\}$ or $\{3\}\oplus\{4\}$<br>$\{1\}\oplus\{3\}$ or $\{2\}\oplus\{4\}$<br>$\{1\}\oplus\{4\}$ or $\{2\}\oplus\{3\}$ |
| 221 | Z$\left(u,\ \frac{1}{2},\ 0\right)$ | $(0,\ 0,\ 1),\ (0,\ -1,\ 0)$ | $\{1\}\oplus\{2\}$ or $\{3\}\oplus\{4\}$ |
| 222 | DT$(0,\ v,\ 0)$ | $\left(-\frac{\sqrt{2}}{2},\ 0,\ \frac{\sqrt{2}}{2}\right),\ \left(-\frac{\sqrt{2}}{2},\ 0,\ -\frac{\sqrt{2}}{2}\right),\ (0,\ 0,\ 1),\ (1,\ 0,\ 0)$<br>$\left(-\frac{\sqrt{2}}{2},\ 0,\ \frac{\sqrt{2}}{2}\right),\ \left(-\frac{\sqrt{2}}{2},\ 0,\ -\frac{\sqrt{2}}{2}\right)$<br>$(0,\ 0,\ 1),\ (1,\ 0,\ 0)$ | $\{1\}\oplus\{2\}$ or $\{3\}\oplus\{4\}$<br>$\{1\}\oplus\{3\}$ or $\{2\}\oplus\{4\}$<br>$\{1\}\oplus\{4\}$ or $\{2\}\oplus\{3\}$ |
| 222 | LD$(u,\ u,\ u)$ | $\left(\frac{\sqrt{2}}{2},\ -\frac{\sqrt{2}}{2},\ 0\right),\ \left(0,\ \frac{\sqrt{2}}{2},\ -\frac{\sqrt{2}}{2}\right)$ | $\{1\}\oplus\{2\}$ |
| 222 | SM$(u,\ u,\ 0)$ | $\left(\frac{\sqrt{2}}{2},\ -\frac{\sqrt{2}}{2},\ 0\right),\ (0,\ 0,\ 1)$ | $\{1\}\oplus\{2\}$ or $\{3\}\oplus\{4\}$ |
| 222 | T$\left(\frac{1}{2},\ \frac{1}{2},\ w\right)$ | $(0,\ -1,\ 0),\ (-1,\ 0,\ 0)$<br>$\left(\frac{\sqrt{2}}{2},\ -\frac{\sqrt{2}}{2},\ 0\right),\ \left(\frac{\sqrt{2}}{2},\ \frac{\sqrt{2}}{2},\ 0\right)$<br>$\left(\frac{\sqrt{2}}{2},\ -\frac{\sqrt{2}}{2},\ 0\right),\ \left(\frac{\sqrt{2}}{2},\ \frac{\sqrt{2}}{2},\ 0\right),\ (0,\ -1,\ 0),\ (-1,\ 0,\ 0)$ | $\{1\}\oplus\{2\}$ or $\{3\}\oplus\{4\}$<br>$\{1\}\oplus\{3\}$ or $\{2\}\oplus\{4\}$<br>$\{1\}\oplus\{4\}$ or $\{2\}\oplus\{3\}$ |
| 223 | DT$(0,\ v,\ 0)$ | $\left(-\frac{\sqrt{2}}{2},\ 0,\ \frac{\sqrt{2}}{2}\right),\ \left(-\frac{\sqrt{2}}{2},\ 0,\ -\frac{\sqrt{2}}{2}\right),\ (0,\ 0,\ 1),\ (1,\ 0,\ 0)$<br>$\left(-\frac{\sqrt{2}}{2},\ 0,\ \frac{\sqrt{2}}{2}\right),\ \left(-\frac{\sqrt{2}}{2},\ 0,\ -\frac{\sqrt{2}}{2}\right)$<br>$(0,\ 0,\ 1),\ (1,\ 0,\ 0)$ | $\{1\}\oplus\{2\}$ or $\{3\}\oplus\{4\}$<br>$\{1\}\oplus\{3\}$ or $\{2\}\oplus\{4\}$<br>$\{1\}\oplus\{4\}$ or $\{2\}\oplus\{3\}$ |
| 223 | LD$(u,\ u,\ u)$ | $\left(\frac{\sqrt{2}}{2},\ -\frac{\sqrt{2}}{2},\ 0\right),\ \left(0,\ \frac{\sqrt{2}}{2},\ -\frac{\sqrt{2}}{2}\right)$ | $\{1\}\oplus\{2\}$ |
| 223 | SM$(u,\ u,\ 0)$ | $\left(\frac{\sqrt{2}}{2},\ -\frac{\sqrt{2}}{2},\ 0\right),\ (0,\ 0,\ 1)$ | $\{1\}\oplus\{2\}$ or $\{3\}\oplus\{4\}$ |
| 223 | T$\left(\frac{1}{2},\ \frac{1}{2},\ w\right)$ | $\left(\frac{\sqrt{2}}{2},\ -\frac{\sqrt{2}}{2},\ 0\right),\ \left(\frac{\sqrt{2}}{2},\ \frac{\sqrt{2}}{2},\ 0\right),\ (0,\ -1,\ 0),\ (-1,\ 0,\ 0)$<br>$\left(\frac{\sqrt{2}}{2},\ -\frac{\sqrt{2}}{2},\ 0\right),\ \left(\frac{\sqrt{2}}{2},\ \frac{\sqrt{2}}{2},\ 0\right)$<br>$(0,\ -1,\ 0),\ (-1,\ 0,\ 0)$ | $\{1\}\oplus\{2\}$ or $\{3\}\oplus\{4\}$<br>$\{1\}\oplus\{3\}$ or $\{2\}\oplus\{4\}$<br>$\{1\}\oplus\{4\}$ or $\{2\}\oplus\{3\}$ |
| 223 | Z$\left(u,\ \frac{1}{2},\ 0\right)$ | $(0,\ 0,\ 1),\ (0,\ -1,\ 0)$ | $\{1\}\oplus\{2\}$ or $\{3\}\oplus\{4\}$ |
| 224 | DT$(0,\ v,\ 0)$ | $\left(-\frac{\sqrt{2}}{2},\ 0,\ \frac{\sqrt{2}}{2}\right),\ \left(-\frac{\sqrt{2}}{2},\ 0,\ -\frac{\sqrt{2}}{2}\right),\ (0,\ 0,\ 1),\ (1,\ 0,\ 0)$<br>$\left(-\frac{\sqrt{2}}{2},\ 0,\ \frac{\sqrt{2}}{2}\right),\ \left(-\frac{\sqrt{2}}{2},\ 0,\ -\frac{\sqrt{2}}{2}\right)$<br>$(0,\ 0,\ 1),\ (1,\ 0,\ 0)$ | $\{1\}\oplus\{2\}$ or $\{3\}\oplus\{4\}$<br>$\{1\}\oplus\{3\}$ or $\{2\}\oplus\{4\}$<br>$\{1\}\oplus\{4\}$ or $\{2\}\oplus\{3\}$ |
| 224 | LD$(u,\ u,\ u)$ | $\left(\frac{\sqrt{2}}{2},\ -\frac{\sqrt{2}}{2},\ 0\right),\ \left(0,\ \frac{\sqrt{2}}{2},\ -\frac{\sqrt{2}}{2}\right)$ | $\{1\}\oplus\{2\}$ |
| 224 | S$\left(u,\ \frac{1}{2},\ u\right)$ | $\left(-\frac{\sqrt{2}}{2},\ 0,\ \frac{\sqrt{2}}{2}\right),\ (0,\ -1,\ 0)$ | $\{1\}\oplus\{3\}$ or $\{2\}\oplus\{4\}$ |
| 224 | SM$(u,\ u,\ 0)$ | $\left(\frac{\sqrt{2}}{2},\ -\frac{\sqrt{2}}{2},\ 0\right),\ (0,\ 0,\ 1)$ | $\{1\}\oplus\{2\}$ or $\{3\}\oplus\{4\}$ |
| 224 | T$\left(\frac{1}{2},\ \frac{1}{2},\ w\right)$ | $(0,\ -1,\ 0),\ (-1,\ 0,\ 0)$<br>$\left(\frac{\sqrt{2}}{2},\ -\frac{\sqrt{2}}{2},\ 0\right),\ \left(\frac{\sqrt{2}}{2},\ \frac{\sqrt{2}}{2},\ 0\right),\ (0,\ -1,\ 0),\ (-1,\ 0,\ 0)$<br>$\left(\frac{\sqrt{2}}{2},\ -\frac{\sqrt{2}}{2},\ 0\right),\ \left(\frac{\sqrt{2}}{2},\ \frac{\sqrt{2}}{2},\ 0\right)$ | $\{1\}\oplus\{2\}$ or $\{3\}\oplus\{4\}$<br>$\{1\}\oplus\{3\}$ or $\{2\}\oplus\{4\}$<br>$\{1\}\oplus\{4\}$ or $\{2\}\oplus\{3\}$ |
| 225 | DT$(0,\ v,\ 0)$ | $(0,\ 0,\ -1),\ (-1,\ 0,\ 0),\ \left(\frac{\sqrt{2}}{2},\ 0,\ -\frac{\sqrt{2}}{2}\right),\ \left(\frac{\sqrt{2}}{2},\ 0,\ \frac{\sqrt{2}}{2}\right)$<br>$\left(\frac{\sqrt{2}}{2},\ 0,\ -\frac{\sqrt{2}}{2}\right),\ \left(\frac{\sqrt{2}}{2},\ 0,\ \frac{\sqrt{2}}{2}\right)$<br>$(0,\ 0,\ -1),\ (-1,\ 0,\ 0)$ | $\{1\}\oplus\{2\}$ or $\{3\}\oplus\{4\}$<br>$\{1\}\oplus\{3\}$ or $\{2\}\oplus\{4\}$<br>$\{1\}\oplus\{4\}$ or $\{2\}\oplus\{3\}$ |

| SG | HSL | Location of nodal chain | Irreps of BC |
|---|---|---|---|
| 225 | LD$(u,\ u,\ u)$ | $\left(-\frac{\sqrt{2}}{2},\ \frac{\sqrt{2}}{2},\ 0\right),\ \left(0,\ -\frac{\sqrt{2}}{2},\ \frac{\sqrt{2}}{2}\right)$ | $\{1\}\oplus\{2\}$ |
| 225 | SM$(u,\ u,\ 0)$ | $(0,\ 0,\ -1),\ \left(-\frac{\sqrt{2}}{2},\ \frac{\sqrt{2}}{2},\ 0\right)$ | $\{1\}\oplus\{2\}$ or $\{3\}\oplus\{4\}$ |
| 225 | V$(u,\ 1,\ 0)$ | $(0,\ 0,\ -1),\ (0,\ -1,\ 0)$ | $\{1\}\oplus\{2\}$ or $\{3\}\oplus\{4\}$ |
| 226 | DT$(0,\ v,\ 0)$ | $(0,\ 0,\ -1),\ (-1,\ 0,\ 0),\ \left(\frac{\sqrt{2}}{2},\ 0,\ -\frac{\sqrt{2}}{2}\right),\ \left(\frac{\sqrt{2}}{2},\ 0,\ \frac{\sqrt{2}}{2}\right)$<br>$\left(\frac{\sqrt{2}}{2},\ 0,\ -\frac{\sqrt{2}}{2}\right),\ \left(\frac{\sqrt{2}}{2},\ 0,\ \frac{\sqrt{2}}{2}\right)$<br>$(0,\ 0,\ -1),\ (-1,\ 0,\ 0)$ | $\{1\}\oplus\{2\}$ or $\{3\}\oplus\{4\}$<br>$\{1\}\oplus\{3\}$ or $\{2\}\oplus\{4\}$<br>$\{1\}\oplus\{4\}$ or $\{2\}\oplus\{3\}$ |
| 226 | LD$(u,\ u,\ u)$ | $\left(-\frac{\sqrt{2}}{2},\ \frac{\sqrt{2}}{2},\ 0\right),\ \left(0,\ -\frac{\sqrt{2}}{2},\ \frac{\sqrt{2}}{2}\right)$ | $\{1\}\oplus\{2\}$ |
| 226 | SM$(u,\ u,\ 0)$ | $(0,\ 0,\ -1),\ \left(-\frac{\sqrt{2}}{2},\ \frac{\sqrt{2}}{2},\ 0\right)$ | $\{1\}\oplus\{2\}$ or $\{3\}\oplus\{4\}$ |
| 226 | V$(u,\ 1,\ 0)$ | $(0,\ 0,\ -1),\ (0,\ -1,\ 0)$ | $\{1\}\oplus\{2\}$ or $\{3\}\oplus\{4\}$ |
| 227 | DT$(0,\ v,\ 0)$ | $(0,\ 0,\ -1),\ (-1,\ 0,\ 0),\ \left(\frac{\sqrt{2}}{2},\ 0,\ -\frac{\sqrt{2}}{2}\right),\ \left(\frac{\sqrt{2}}{2},\ 0,\ \frac{\sqrt{2}}{2}\right)$<br>$\left(\frac{\sqrt{2}}{2},\ 0,\ -\frac{\sqrt{2}}{2}\right),\ \left(\frac{\sqrt{2}}{2},\ 0,\ \frac{\sqrt{2}}{2}\right)$<br>$(0,\ 0,\ -1),\ (-1,\ 0,\ 0)$ | $\{1\}\oplus\{2\}$ or $\{3\}\oplus\{4\}$<br>$\{1\}\oplus\{3\}$ or $\{2\}\oplus\{4\}$<br>$\{1\}\oplus\{4\}$ or $\{2\}\oplus\{3\}$ |
| 227 | LD$(u,\ u,\ u)$ | $\left(-\frac{\sqrt{2}}{2},\ \frac{\sqrt{2}}{2},\ 0\right),\ \left(0,\ -\frac{\sqrt{2}}{2},\ \frac{\sqrt{2}}{2}\right)$ | $\{1\}\oplus\{2\}$ |
| 227 | SM$(u,\ u,\ 0)$ | $(0,\ 0,\ -1),\ \left(-\frac{\sqrt{2}}{2},\ \frac{\sqrt{2}}{2},\ 0\right)$ | $\{1\}\oplus\{2\}$ or $\{3\}\oplus\{4\}$ |
| 228 | DT$(0,\ v,\ 0)$ | $(0,\ 0,\ -1),\ (-1,\ 0,\ 0),\ \left(\frac{\sqrt{2}}{2},\ 0,\ -\frac{\sqrt{2}}{2}\right),\ \left(\frac{\sqrt{2}}{2},\ 0,\ \frac{\sqrt{2}}{2}\right)$<br>$\left(\frac{\sqrt{2}}{2},\ 0,\ -\frac{\sqrt{2}}{2}\right),\ \left(\frac{\sqrt{2}}{2},\ 0,\ \frac{\sqrt{2}}{2}\right)$<br>$(0,\ 0,\ -1),\ (-1,\ 0,\ 0)$ | $\{1\}\oplus\{2\}$ or $\{3\}\oplus\{4\}$<br>$\{1\}\oplus\{3\}$ or $\{2\}\oplus\{4\}$<br>$\{1\}\oplus\{4\}$ or $\{2\}\oplus\{3\}$ |
| 228 | LD$(u,\ u,\ u)$ | $\left(-\frac{\sqrt{2}}{2},\ \frac{\sqrt{2}}{2},\ 0\right),\ \left(0,\ -\frac{\sqrt{2}}{2},\ \frac{\sqrt{2}}{2}\right)$ | $\{1\}\oplus\{2\}$ |
| 228 | SM$(u,\ u,\ 0)$ | $(0,\ 0,\ -1),\ \left(-\frac{\sqrt{2}}{2},\ \frac{\sqrt{2}}{2},\ 0\right)$ | $\{1\}\oplus\{2\}$ or $\{3\}\oplus\{4\}$ |
| 229 | D$\left(\frac{1}{2},\ \frac{1}{2},\ w\right)$ | $\left(-\frac{\sqrt{2}}{2},\ \frac{\sqrt{2}}{2},\ 0\right),\ \left(-\frac{\sqrt{2}}{2},\ -\frac{\sqrt{2}}{2},\ 0\right)$ | $\{1\}\oplus\{2\}$ or $\{3\}\oplus\{4\}$ |
| 229 | DT$(0,\ v,\ 0)$ | $\left(\frac{\sqrt{2}}{2},\ 0,\ -\frac{\sqrt{2}}{2}\right),\ \left(\frac{\sqrt{2}}{2},\ 0,\ \frac{\sqrt{2}}{2}\right),\ (0,\ 0,\ -1),\ (-1,\ 0,\ 0)$<br>$\left(\frac{\sqrt{2}}{2},\ 0,\ -\frac{\sqrt{2}}{2}\right),\ \left(\frac{\sqrt{2}}{2},\ 0,\ \frac{\sqrt{2}}{2}\right)$<br>$(0,\ 0,\ -1),\ (-1,\ 0,\ 0)$ | $\{1\}\oplus\{2\}$ or $\{3\}\oplus\{4\}$<br>$\{1\}\oplus\{3\}$ or $\{2\}\oplus\{4\}$<br>$\{1\}\oplus\{4\}$ or $\{2\}\oplus\{3\}$ |
| 229 | G$(u+1,\ 1-u,\ 1)$ | $\left(-\frac{\sqrt{2}}{2},\ -\frac{\sqrt{2}}{2},\ 0\right),\ (0,\ 0,\ -1)$ | $\{1\}\oplus\{2\}$ or $\{3\}\oplus\{4\}$ |
| 229 | LD$(u,\ u,\ u)$ | $\left(-\frac{\sqrt{2}}{2},\ \frac{\sqrt{2}}{2},\ 0\right),\ \left(0,\ -\frac{\sqrt{2}}{2},\ \frac{\sqrt{2}}{2}\right)$ | $\{1\}\oplus\{2\}$ |
| 229 | SM$(u,\ u,\ 0)$ | $\left(-\frac{\sqrt{2}}{2},\ \frac{\sqrt{2}}{2},\ 0\right),\ (0,\ 0,\ -1)$ | $\{1\}\oplus\{2\}$ or $\{3\}\oplus\{4\}$ |
| 230 | DT$(0,\ v,\ 0)$ | $\left(\frac{\sqrt{2}}{2},\ 0,\ -\frac{\sqrt{2}}{2}\right),\ \left(\frac{\sqrt{2}}{2},\ 0,\ \frac{\sqrt{2}}{2}\right),\ (0,\ 0,\ -1),\ (-1,\ 0,\ 0)$<br>$\left(\frac{\sqrt{2}}{2},\ 0,\ -\frac{\sqrt{2}}{2}\right),\ \left(\frac{\sqrt{2}}{2},\ 0,\ \frac{\sqrt{2}}{2}\right)$<br>$(0,\ 0,\ -1),\ (-1,\ 0,\ 0)$ | $\{1\}\oplus\{2\}$ or $\{3\}\oplus\{4\}$<br>$\{1\}\oplus\{3\}$ or $\{2\}\oplus\{4\}$<br>$\{1\}\oplus\{4\}$ or $\{2\}\oplus\{3\}$ |
| 230 | LD$(u,\ u,\ u)$ | $\left(-\frac{\sqrt{2}}{2},\ \frac{\sqrt{2}}{2},\ 0\right),\ \left(0,\ -\frac{\sqrt{2}}{2},\ \frac{\sqrt{2}}{2}\right)$ | $\{1\}\oplus\{2\}$ |
| 230 | SM$(u,\ u,\ 0)$ | $\left(-\frac{\sqrt{2}}{2},\ \frac{\sqrt{2}}{2},\ 0\right),\ (0,\ 0,\ -1)$ | $\{1\}\oplus\{2\}$ or $\{3\}\oplus\{4\}$ |

Table S16: Intra-chain structure

| SG | HSL | Location of nodal chain | Irreps of BC |
|---|---|---|---|
| 25 | G$\left(\frac{1}{2},\ 0,\ w\right)$ | $(0,\ -1,\ 0), (-1,\ 0,\ 0)$ | $1\oplus2$ or $3\oplus4$ |
| 25 | H$\left(0,\ \frac{1}{2},\ w\right)$ | $(-1,\ 0,\ 0), (0,\ -1,\ 0)$ | $1\oplus2$ or $3\oplus4$ |
| 25 | LD$(0,\ 0,\ w)$ | $(-1,\ 0,\ 0), (0,\ -1,\ 0)$ | $1\oplus2$ or $3\oplus4$ |
| 25 | Q$\left(\frac{1}{2},\ \frac{1}{2},\ w\right)$ | $(-1,\ 0,\ 0), (0,\ -1,\ 0)$ | $1\oplus2$ or $3\oplus4$ |
| 26 | G$\left(\frac{1}{2},\ 0,\ w\right)$ | $(0,\ -1,\ 0), (-1,\ 0,\ 0)$ | $1\oplus2$ or $3\oplus4$ |
| 26 | H$\left(0,\ \frac{1}{2},\ w\right)$ | $(-1,\ 0,\ 0), (0,\ -1,\ 0)$ | $1\oplus2$ or $3\oplus4$ |
| 26 | LD$(0,\ 0,\ w)$ | $(-1,\ 0,\ 0), (0,\ -1,\ 0)$ | $1\oplus2$ or $3\oplus4$ |
| 26 | Q$\left(\frac{1}{2},\ \frac{1}{2},\ w\right)$ | $(-1,\ 0,\ 0), (0,\ -1,\ 0)$ | $1\oplus2$ or $3\oplus4$ |
| 27 | G$\left(\frac{1}{2},\ 0,\ w\right)$ | $(0,\ -1,\ 0), (-1,\ 0,\ 0)$ | $1\oplus2$ or $3\oplus4$ |
| 27 | H$\left(0,\ \frac{1}{2},\ w\right)$ | $(-1,\ 0,\ 0), (0,\ -1,\ 0)$ | $1\oplus2$ or $3\oplus4$ |
| 27 | LD$(0,\ 0,\ w)$ | $(-1,\ 0,\ 0), (0,\ -1,\ 0)$ | $1\oplus2$ or $3\oplus4$ |
| 27 | Q$\left(\frac{1}{2},\ \frac{1}{2},\ w\right)$ | $(-1,\ 0,\ 0), (0,\ -1,\ 0)$ | $1\oplus2$ or $3\oplus4$ |
| 28 | H$\left(0,\ \frac{1}{2},\ w\right)$ | $(-1,\ 0,\ 0), (0,\ 1,\ 0)$ | $1\oplus2$ or $3\oplus4$ |
| 28 | LD$(0,\ 0,\ w)$ | $(0,\ 1,\ 0), (-1,\ 0,\ 0)$ | $1\oplus2$ or $3\oplus4$ |
| 29 | H$\left(0,\ \frac{1}{2},\ w\right)$ | $(-1,\ 0,\ 0), (0,\ 1,\ 0)$ | $1\oplus2$ or $3\oplus4$ |
| 29 | LD$(0,\ 0,\ w)$ | $(0,\ 1,\ 0), (-1,\ 0,\ 0)$ | $1\oplus2$ or $3\oplus4$ |
| 30 | G$\left(\frac{1}{2},\ 0,\ w\right)$ | $(0,\ -1,\ 0), (-1,\ 0,\ 0)$ | $1\oplus2$ or $3\oplus4$ |
| 30 | LD$(0,\ 0,\ w)$ | $(-1,\ 0,\ 0), (0,\ -1,\ 0)$ | $1\oplus2$ or $3\oplus4$ |
| 31 | H$\left(0,\ \frac{1}{2},\ w\right)$ | $(-1,\ 0,\ 0), (0,\ 1,\ 0)$ | $1\oplus2$ or $3\oplus4$ |
| 31 | LD$(0,\ 0,\ w)$ | $(0,\ 1,\ 0), (-1,\ 0,\ 0)$ | $1\oplus2$ or $3\oplus4$ |
| 32 | LD$(0,\ 0,\ w)$ | $(-1,\ 0,\ 0), (0,\ -1,\ 0)$ | $1\oplus2$ or $3\oplus4$ |
| 32 | Q$\left(\frac{1}{2},\ \frac{1}{2},\ w\right)$ | $(-1,\ 0,\ 0), (0,\ -1,\ 0)$ | $1\oplus3$ or $2\oplus4$ |
| 33 | LD$(0,\ 0,\ w)$ | $(0,\ 1,\ 0), (-1,\ 0,\ 0)$ | $1\oplus2$ or $3\oplus4$ |
| 33 | Q$\left(\frac{1}{2},\ \frac{1}{2},\ w\right)$ | $(0,\ 1,\ 0), (-1,\ 0,\ 0)$ | $1\oplus3$ or $2\oplus4$ |
| 34 | LD$(0,\ 0,\ w)$ | $(-1,\ 0,\ 0), (0,\ -1,\ 0)$ | $1\oplus2$ or $3\oplus4$ |
| 34 | Q$\left(\frac{1}{2},\ \frac{1}{2},\ w\right)$ | $(-1,\ 0,\ 0), (0,\ -1,\ 0)$ | $1\oplus3$ or $2\oplus4$ |
| 35 | H$(1,\ 0,\ w)$ | $(0,\ -1,\ 0), (-1,\ 0,\ 0)$ | $1\oplus2$ or $3\oplus4$ |
| 35 | LD$(0,\ 0,\ w)$ | $(0,\ -1,\ 0), (-1,\ 0,\ 0)$ | $1\oplus2$ or $3\oplus4$ |
| 36 | H$(1,\ 0,\ w)$ | $(-1,\ 0,\ 0), (0,\ 1,\ 0)$ | $1\oplus2$ or $3\oplus4$ |
| 36 | LD$(0,\ 0,\ w)$ | $(-1,\ 0,\ 0), (0,\ 1,\ 0)$ | $1\oplus2$ or $3\oplus4$ |
| 37 | H$(1,\ 0,\ w)$ | $(0,\ -1,\ 0), (-1,\ 0,\ 0)$ | $1\oplus2$ or $3\oplus4$ |
| 37 | LD$(0,\ 0,\ w)$ | $(0,\ -1,\ 0), (-1,\ 0,\ 0)$ | $1\oplus2$ or $3\oplus4$ |
| 38 | A$\left(\frac{1}{2},\ 0,\ w\right)$ | $(0,\ -1,\ 0), (1,\ 0,\ 0)$ | $1\oplus2$ or $3\oplus4$ |
| 38 | SM$(0,\ 0,\ w)$ | $(0,\ -1,\ 0), (1,\ 0,\ 0)$ | $1\oplus2$ or $3\oplus4$ |
| 39 | A$\left(\frac{1}{2},\ 0,\ w\right)$ | $(0,\ -1,\ 0), (1,\ 0,\ 0)$ | $1\oplus2$ or $3\oplus4$ |
| 39 | SM$(0,\ 0,\ w)$ | $(0,\ -1,\ 0), (1,\ 0,\ 0)$ | $1\oplus2$ or $3\oplus4$ |
| 40 | SM$(0,\ 0,\ w)$ | $(0,\ -1,\ 0), (1,\ 0,\ 0)$ | $1\oplus2$ or $3\oplus4$ |
| 41 | SM$(0,\ 0,\ w)$ | $(0,\ -1,\ 0), (1,\ 0,\ 0)$ | $1\oplus2$ or $3\oplus4$ |
| 42 | H$(0,\ 1,\ w)$ | $(0,\ 1,\ 0), (1,\ 0,\ 0)$ | $1\oplus2$ or $3\oplus4$ |
| 42 | LD$(0,\ 0,\ w)$ | $(0,\ 1,\ 0), (1,\ 0,\ 0)$ | $1\oplus2$ or $3\oplus4$ |
| 43 | LD$(0,\ 0,\ w)$ | $(0,\ 1,\ 0), (1,\ 0,\ 0)$ | $1\oplus2$ or $3\oplus4$ |

| SG | HSL | Location of nodal chain | Irreps of BC |
|---|---|---|---|
| 44 | LD$(0,\ 0,\ w)$ | $(0,\ -1,\ 0)$, $(1,\ 0,\ 0)$ | $1{\oplus}2$ or $3{\oplus}4$ |
| 45 | LD$(0,\ 0,\ w)$ | $(0,\ -1,\ 0)$, $(1,\ 0,\ 0)$ | $1{\oplus}2$ or $3{\oplus}4$ |
| 46 | LD$(0,\ 0,\ w)$ | $(-1,\ 0,\ 0)$, $(0,\ -1,\ 0)$ | $1{\oplus}2$ or $3{\oplus}4$ |
| 47 | A$\left(u,\ 0,\ \frac{1}{2}\right)$ | $(0,\ -1,\ 0)$, $(0,\ 0,\ 1)$ | $\{1\}{\oplus}\{2\}$ or $\{3\}{\oplus}\{4\}$ |
| 47 | B$\left(0,\ v,\ \frac{1}{2}\right)$ | $(-1,\ 0,\ 0)$, $(0,\ 0,\ 1)$ | $\{1\}{\oplus}\{2\}$ or $\{3\}{\oplus}\{4\}$ |
| 47 | C$\left(u,\ \frac{1}{2},\ 0\right)$ | $(0,\ 0,\ 1)$, $(0,\ -1,\ 0)$ | $\{1\}{\oplus}\{2\}$ or $\{3\}{\oplus}\{4\}$ |
| 47 | D$\left(\frac{1}{2},\ v,\ 0\right)$ | $(0,\ 0,\ 1)$, $(-1,\ 0,\ 0)$ | $\{1\}{\oplus}\{2\}$ or $\{3\}{\oplus}\{4\}$ |
| 47 | DT$(0,\ v,\ 0)$ | $(0,\ 0,\ 1)$, $(-1,\ 0,\ 0)$ | $\{1\}{\oplus}\{2\}$ or $\{3\}{\oplus}\{4\}$ |
| 47 | E$\left(u,\ \frac{1}{2},\ \frac{1}{2}\right)$ | $(0,\ 0,\ 1)$, $(0,\ -1,\ 0)$ | $\{1\}{\oplus}\{2\}$ or $\{3\}{\oplus}\{4\}$ |
| 47 | G$\left(\frac{1}{2},\ 0,\ w\right)$ | $(0,\ -1,\ 0)$, $(-1,\ 0,\ 0)$ | $\{1\}{\oplus}\{2\}$ or $\{3\}{\oplus}\{4\}$ |
| 47 | H$\left(0,\ \frac{1}{2},\ w\right)$ | $(-1,\ 0,\ 0)$, $(0,\ -1,\ 0)$ | $\{1\}{\oplus}\{2\}$ or $\{3\}{\oplus}\{4\}$ |
| 47 | LD$(0,\ 0,\ w)$ | $(-1,\ 0,\ 0)$, $(0,\ -1,\ 0)$ | $\{1\}{\oplus}\{2\}$ or $\{3\}{\oplus}\{4\}$ |
| 47 | P$\left(\frac{1}{2},\ v,\ \frac{1}{2}\right)$ | $(0,\ 0,\ 1)$, $(-1,\ 0,\ 0)$ | $\{1\}{\oplus}\{2\}$ or $\{3\}{\oplus}\{4\}$ |
| 47 | Q$\left(\frac{1}{2},\ \frac{1}{2},\ w\right)$ | $(-1,\ 0,\ 0)$, $(0,\ -1,\ 0)$ | $\{1\}{\oplus}\{2\}$ or $\{3\}{\oplus}\{4\}$ |
| 47 | SM$(u,\ 0,\ 0)$ | $(0,\ 0,\ 1)$, $(0,\ -1,\ 0)$ | $\{1\}{\oplus}\{2\}$ or $\{3\}{\oplus}\{4\}$ |
| 48 | DT$(0,\ v,\ 0)$ | $(0,\ 0,\ 1)$, $(-1,\ 0,\ 0)$ | $\{1\}{\oplus}\{2\}$ or $\{3\}{\oplus}\{4\}$ |
| 48 | E$\left(u,\ \frac{1}{2},\ \frac{1}{2}\right)$ | $(0,\ 0,\ 1)$, $(0,\ -1,\ 0)$ | $\{1\}{\oplus}\{2\}$ or $\{3\}{\oplus}\{4\}$ |
| 48 | LD$(0,\ 0,\ w)$ | $(-1,\ 0,\ 0)$, $(0,\ -1,\ 0)$ | $\{1\}{\oplus}\{2\}$ or $\{3\}{\oplus}\{4\}$ |
| 48 | P$\left(\frac{1}{2},\ v,\ \frac{1}{2}\right)$ | $(0,\ 0,\ 1)$, $(-1,\ 0,\ 0)$ | $\{1\}{\oplus}\{2\}$ or $\{3\}{\oplus}\{4\}$ |
| 48 | Q$\left(\frac{1}{2},\ \frac{1}{2},\ w\right)$ | $(-1,\ 0,\ 0)$, $(0,\ -1,\ 0)$ | $\{1\}{\oplus}\{2\}$ or $\{3\}{\oplus}\{4\}$ |
| 48 | SM$(u,\ 0,\ 0)$ | $(0,\ 0,\ 1)$, $(0,\ -1,\ 0)$ | $\{1\}{\oplus}\{2\}$ or $\{3\}{\oplus}\{4\}$ |
| 49 | C$\left(u,\ \frac{1}{2},\ 0\right)$ | $(0,\ 0,\ 1)$, $(0,\ -1,\ 0)$ | $\{1\}{\oplus}\{2\}$ or $\{3\}{\oplus}\{4\}$ |
| 49 | D$\left(\frac{1}{2},\ v,\ 0\right)$ | $(0,\ 0,\ 1)$, $(-1,\ 0,\ 0)$ | $\{1\}{\oplus}\{2\}$ or $\{3\}{\oplus}\{4\}$ |
| 49 | DT$(0,\ v,\ 0)$ | $(0,\ 0,\ 1)$, $(-1,\ 0,\ 0)$ | $\{1\}{\oplus}\{2\}$ or $\{3\}{\oplus}\{4\}$ |
| 49 | G$\left(\frac{1}{2},\ 0,\ w\right)$ | $(0,\ -1,\ 0)$, $(-1,\ 0,\ 0)$ | $\{1\}{\oplus}\{2\}$ or $\{3\}{\oplus}\{4\}$ |
| 49 | H$\left(0,\ \frac{1}{2},\ w\right)$ | $(-1,\ 0,\ 0)$, $(0,\ -1,\ 0)$ | $\{1\}{\oplus}\{2\}$ or $\{3\}{\oplus}\{4\}$ |
| 49 | LD$(0,\ 0,\ w)$ | $(-1,\ 0,\ 0)$, $(0,\ -1,\ 0)$ | $\{1\}{\oplus}\{2\}$ or $\{3\}{\oplus}\{4\}$ |
| 49 | Q$\left(\frac{1}{2},\ \frac{1}{2},\ w\right)$ | $(-1,\ 0,\ 0)$, $(0,\ -1,\ 0)$ | $\{1\}{\oplus}\{2\}$ or $\{3\}{\oplus}\{4\}$ |
| 49 | SM$(u,\ 0,\ 0)$ | $(0,\ 0,\ 1)$, $(0,\ -1,\ 0)$ | $\{1\}{\oplus}\{2\}$ or $\{3\}{\oplus}\{4\}$ |
| 50 | A$\left(u,\ 0,\ \frac{1}{2}\right)$ | $(0,\ -1,\ 0)$, $(0,\ 0,\ 1)$ | $\{1\}{\oplus}\{2\}$ or $\{3\}{\oplus}\{4\}$ |
| 50 | B$\left(0,\ v,\ \frac{1}{2}\right)$ | $(-1,\ 0,\ 0)$, $(0,\ 0,\ 1)$ | $\{1\}{\oplus}\{2\}$ or $\{3\}{\oplus}\{4\}$ |
| 50 | DT$(0,\ v,\ 0)$ | $(0,\ 0,\ 1)$, $(-1,\ 0,\ 0)$ | $\{1\}{\oplus}\{2\}$ or $\{3\}{\oplus}\{4\}$ |
| 50 | LD$(0,\ 0,\ w)$ | $(-1,\ 0,\ 0)$, $(0,\ -1,\ 0)$ | $\{1\}{\oplus}\{2\}$ or $\{3\}{\oplus}\{4\}$ |
| 50 | Q$\left(\frac{1}{2},\ \frac{1}{2},\ w\right)$ | $(-1,\ 0,\ 0)$, $(0,\ -1,\ 0)$ | $\{1\}{\oplus}\{2\}$ or $\{3\}{\oplus}\{4\}$ |
| 50 | SM$(u,\ 0,\ 0)$ | $(0,\ 0,\ 1)$, $(0,\ -1,\ 0)$ | $\{1\}{\oplus}\{2\}$ or $\{3\}{\oplus}\{4\}$ |
| 51 | A$\left(u,\ 0,\ \frac{1}{2}\right)$ | $(0,\ -1,\ 0)$, $(0,\ 0,\ -1)$ | $\{1\}{\oplus}\{2\}$ or $\{3\}{\oplus}\{4\}$ |
| 51 | B$\left(0,\ v,\ \frac{1}{2}\right)$ | $(-1,\ 0,\ 0)$, $(0,\ 0,\ -1)$ | $\{1\}{\oplus}\{2\}$ or $\{3\}{\oplus}\{4\}$ |
| 51 | C$\left(u,\ \frac{1}{2},\ 0\right)$ | $(0,\ 0,\ -1)$, $(0,\ -1,\ 0)$ | $\{1\}{\oplus}\{2\}$ or $\{3\}{\oplus}\{4\}$ |
| 51 | DT$(0,\ v,\ 0)$ | $(-1,\ 0,\ 0)$, $(0,\ 0,\ -1)$ | $\{1\}{\oplus}\{2\}$ or $\{3\}{\oplus}\{4\}$ |
| 51 | E$\left(u,\ \frac{1}{2},\ \frac{1}{2}\right)$ | $(0,\ 0,\ -1)$, $(0,\ -1,\ 0)$ | $\{1\}{\oplus}\{2\}$ or $\{3\}{\oplus}\{4\}$ |
| 51 | H$\left(0,\ \frac{1}{2},\ w\right)$ | $(-1,\ 0,\ 0)$, $(0,\ -1,\ 0)$ | $\{1\}{\oplus}\{2\}$ or $\{3\}{\oplus}\{4\}$ |

| SG | HSL | Location of nodal chain | Irreps of BC |
|---|---|---|---|
| 51 | LD$(0,\ 0,\ w)$ | $(-1,\ 0,\ 0)$, $(0,\ -1,\ 0)$ | $\{1\}\oplus\{2\}$ or $\{3\}\oplus\{4\}$ |
| 51 | SM$(u,\ 0,\ 0)$ | $(0,\ 0,\ -1)$, $(0,\ -1,\ 0)$ | $\{1\}\oplus\{2\}$ or $\{3\}\oplus\{4\}$ |
| 52 | DT$(0,\ v,\ 0)$ | $(-1,\ 0,\ 0)$, $(0,\ 0,\ 1)$ | $\{1\}\oplus\{2\}$ or $\{3\}\oplus\{4\}$ |
| 52 | LD$(0,\ 0,\ w)$ | $(0,\ 1,\ 0)$, $(-1,\ 0,\ 0)$ | $\{1\}\oplus\{2\}$ or $\{3\}\oplus\{4\}$ |
| 52 | P$\left(\frac{1}{2},\ v,\ \frac{1}{2}\right)$ | $(-1,\ 0,\ 0)$, $(0,\ 0,\ 1)$ | $\{1\}\oplus\{2\}$ or $\{3\}\oplus\{4\}$ |
| 52 | SM$(u,\ 0,\ 0)$ | $(0,\ 1,\ 0)$, $(0,\ 0,\ 1)$ | $\{1\}\oplus\{2\}$ or $\{3\}\oplus\{4\}$ |
| 53 | C$\left(u,\ \frac{1}{2},\ 0\right)$ | $(0,\ 0,\ 1)$, $(0,\ 1,\ 0)$ | $\{1\}\oplus\{2\}$ or $\{3\}\oplus\{4\}$ |
| 53 | DT$(0,\ v,\ 0)$ | $(0,\ 0,\ 1)$, $(-1,\ 0,\ 0)$ | $\{1\}\oplus\{2\}$ or $\{3\}\oplus\{4\}$ |
| 53 | H$\left(0,\ \frac{1}{2},\ w\right)$ | $(-1,\ 0,\ 0)$, $(0,\ 1,\ 0)$ | $\{1\}\oplus\{2\}$ or $\{3\}\oplus\{4\}$ |
| 53 | LD$(0,\ 0,\ w)$ | $(0,\ 1,\ 0)$, $(-1,\ 0,\ 0)$ | $\{1\}\oplus\{2\}$ or $\{3\}\oplus\{4\}$ |
| 53 | SM$(u,\ 0,\ 0)$ | $(0,\ 0,\ 1)$, $(0,\ 1,\ 0)$ | $\{1\}\oplus\{2\}$ or $\{3\}\oplus\{4\}$ |
| 54 | C$\left(u,\ \frac{1}{2},\ 0\right)$ | $(0,\ 0,\ -1)$, $(0,\ -1,\ 0)$ | $\{1\}\oplus\{2\}$ or $\{3\}\oplus\{4\}$ |
| 54 | DT$(0,\ v,\ 0)$ | $(-1,\ 0,\ 0)$, $(0,\ 0,\ -1)$ | $\{1\}\oplus\{2\}$ or $\{3\}\oplus\{4\}$ |
| 54 | H$\left(0,\ \frac{1}{2},\ w\right)$ | $(-1,\ 0,\ 0)$, $(0,\ -1,\ 0)$ | $\{1\}\oplus\{2\}$ or $\{3\}\oplus\{4\}$ |
| 54 | LD$(0,\ 0,\ w)$ | $(-1,\ 0,\ 0)$, $(0,\ -1,\ 0)$ | $\{1\}\oplus\{2\}$ or $\{3\}\oplus\{4\}$ |
| 54 | SM$(u,\ 0,\ 0)$ | $(0,\ 0,\ -1)$, $(0,\ -1,\ 0)$ | $\{1\}\oplus\{2\}$ or $\{3\}\oplus\{4\}$ |
| 55 | A$\left(u,\ 0,\ \frac{1}{2}\right)$ | $(0,\ -1,\ 0)$, $(0,\ 0,\ 1)$ | $\{1\}\oplus\{2\}$ or $\{3\}\oplus\{4\}$ |
| 55 | B$\left(0,\ v,\ \frac{1}{2}\right)$ | $(-1,\ 0,\ 0)$, $(0,\ 0,\ 1)$ | $\{1\}\oplus\{2\}$ or $\{3\}\oplus\{4\}$ |
| 55 | DT$(0,\ v,\ 0)$ | $(0,\ 0,\ 1)$, $(-1,\ 0,\ 0)$ | $\{1\}\oplus\{2\}$ or $\{3\}\oplus\{4\}$ |
| 55 | LD$(0,\ 0,\ w)$ | $(-1,\ 0,\ 0)$, $(0,\ -1,\ 0)$ | $\{1\}\oplus\{2\}$ or $\{3\}\oplus\{4\}$ |
| 55 | SM$(u,\ 0,\ 0)$ | $(0,\ 0,\ 1)$, $(0,\ -1,\ 0)$ | $\{1\}\oplus\{2\}$ or $\{3\}\oplus\{4\}$ |
| 56 | DT$(0,\ v,\ 0)$ | $(0,\ 0,\ 1)$, $(-1,\ 0,\ 0)$ | $\{1\}\oplus\{2\}$ or $\{3\}\oplus\{4\}$ |
| 56 | LD$(0,\ 0,\ w)$ | $(-1,\ 0,\ 0)$, $(0,\ -1,\ 0)$ | $\{1\}\oplus\{2\}$ or $\{3\}\oplus\{4\}$ |
| 56 | SM$(u,\ 0,\ 0)$ | $(0,\ 0,\ 1)$, $(0,\ -1,\ 0)$ | $\{1\}\oplus\{2\}$ or $\{3\}\oplus\{4\}$ |
| 57 | D$\left(\frac{1}{2},\ v,\ 0\right)$ | $(0,\ 0,\ -1)$, $(1,\ 0,\ 0)$ | $\{1\}\oplus\{2\}$ or $\{3\}\oplus\{4\}$ |
| 57 | DT$(0,\ v,\ 0)$ | $(1,\ 0,\ 0)$, $(0,\ 0,\ -1)$ | $\{1\}\oplus\{2\}$ or $\{3\}\oplus\{4\}$ |
| 57 | G$\left(\frac{1}{2},\ 0,\ w\right)$ | $(0,\ -1,\ 0)$, $(1,\ 0,\ 0)$ | $\{1\}\oplus\{2\}$ or $\{3\}\oplus\{4\}$ |
| 57 | LD$(0,\ 0,\ w)$ | $(1,\ 0,\ 0)$, $(0,\ -1,\ 0)$ | $\{1\}\oplus\{2\}$ or $\{3\}\oplus\{4\}$ |
| 57 | SM$(u,\ 0,\ 0)$ | $(0,\ -1,\ 0)$, $(0,\ 0,\ -1)$ | $\{1\}\oplus\{2\}$ or $\{3\}\oplus\{4\}$ |
| 58 | DT$(0,\ v,\ 0)$ | $(0,\ 0,\ 1)$, $(-1,\ 0,\ 0)$ | $\{1\}\oplus\{2\}$ or $\{3\}\oplus\{4\}$ |
| 58 | LD$(0,\ 0,\ w)$ | $(-1,\ 0,\ 0)$, $(0,\ -1,\ 0)$ | $\{1\}\oplus\{2\}$ or $\{3\}\oplus\{4\}$ |
| 58 | SM$(u,\ 0,\ 0)$ | $(0,\ 0,\ 1)$, $(0,\ -1,\ 0)$ | $\{1\}\oplus\{2\}$ or $\{3\}\oplus\{4\}$ |
| 59 | A$\left(u,\ 0,\ \frac{1}{2}\right)$ | $(0,\ -1,\ 0)$, $(0,\ 0,\ 1)$ | $\{1\}\oplus\{2\}$ or $\{3\}\oplus\{4\}$ |
| 59 | B$\left(0,\ v,\ \frac{1}{2}\right)$ | $(-1,\ 0,\ 0)$, $(0,\ 0,\ 1)$ | $\{1\}\oplus\{2\}$ or $\{3\}\oplus\{4\}$ |
| 59 | DT$(0,\ v,\ 0)$ | $(0,\ 0,\ 1)$, $(-1,\ 0,\ 0)$ | $\{1\}\oplus\{2\}$ or $\{3\}\oplus\{4\}$ |
| 59 | LD$(0,\ 0,\ w)$ | $(-1,\ 0,\ 0)$, $(0,\ -1,\ 0)$ | $\{1\}\oplus\{2\}$ or $\{3\}\oplus\{4\}$ |
| 59 | SM$(u,\ 0,\ 0)$ | $(0,\ 0,\ 1)$, $(0,\ -1,\ 0)$ | $\{1\}\oplus\{2\}$ or $\{3\}\oplus\{4\}$ |
| 60 | DT$(0,\ v,\ 0)$ | $(-1,\ 0,\ 0)$, $(0,\ 0,\ 1)$ | $\{1\}\oplus\{2\}$ or $\{3\}\oplus\{4\}$ |
| 60 | LD$(0,\ 0,\ w)$ | $(0,\ 1,\ 0)$, $(-1,\ 0,\ 0)$ | $\{1\}\oplus\{2\}$ or $\{3\}\oplus\{4\}$ |
| 60 | SM$(u,\ 0,\ 0)$ | $(0,\ 1,\ 0)$, $(0,\ 0,\ 1)$ | $\{1\}\oplus\{2\}$ or $\{3\}\oplus\{4\}$ |
| 61 | DT$(0,\ v,\ 0)$ | $(-1,\ 0,\ 0)$, $(0,\ 0,\ 1)$ | $\{1\}\oplus\{2\}$ or $\{3\}\oplus\{4\}$ |

| SG | HSL | Location of nodal chain | Irreps of BC |
|---|---|---|---|
| 61 | LD$(0,\ 0,\ w)$ | $(0,\ 1,\ 0)$, $(-1,\ 0,\ 0)$ | $\{1\}\oplus\{2\}$ or $\{3\}\oplus\{4\}$ |
| 61 | SM$(u,\ 0,\ 0)$ | $(0,\ 1,\ 0)$, $(0,\ 0,\ 1)$ | $\{1\}\oplus\{2\}$ or $\{3\}\oplus\{4\}$ |
| 62 | DT$(0,\ v,\ 0)$ | $(0,\ 0,\ 1)$, $(-1,\ 0,\ 0)$ | $\{1\}\oplus\{2\}$ or $\{3\}\oplus\{4\}$ |
| 62 | LD$(0,\ 0,\ w)$ | $(-1,\ 0,\ 0)$, $(0,\ -1,\ 0)$ | $\{1\}\oplus\{2\}$ or $\{3\}\oplus\{4\}$ |
| 62 | SM$(u,\ 0,\ 0)$ | $(0,\ 0,\ 1)$, $(0,\ -1,\ 0)$ | $\{1\}\oplus\{2\}$ or $\{3\}\oplus\{4\}$ |
| 63 | DT$(0,\ v,\ 0)$ | $(-1,\ 0,\ 0)$, $(0,\ 0,\ 1)$ | $\{1\}\oplus\{2\}$ or $\{3\}\oplus\{4\}$ |
| 63 | H$(1,\ 0,\ w)$ | $(0,\ -1,\ 0)$, $(-1,\ 0,\ 0)$ | $\{1\}\oplus\{2\}$ or $\{3\}\oplus\{4\}$ |
| 63 | LD$(0,\ 0,\ w)$ | $(0,\ -1,\ 0)$, $(-1,\ 0,\ 0)$ | $\{1\}\oplus\{2\}$ or $\{3\}\oplus\{4\}$ |
| 63 | SM$(u,\ 0,\ 0)$ | $(0,\ -1,\ 0)$, $(0,\ 0,\ 1)$ | $\{1\}\oplus\{2\}$ or $\{3\}\oplus\{4\}$ |
| 64 | DT$(0,\ v,\ 0)$ | $(-1,\ 0,\ 0)$, $(0,\ 0,\ 1)$ | $\{1\}\oplus\{2\}$ or $\{3\}\oplus\{4\}$ |
| 64 | H$(1,\ 0,\ w)$ | $(0,\ -1,\ 0)$, $(-1,\ 0,\ 0)$ | $\{1\}\oplus\{2\}$ or $\{3\}\oplus\{4\}$ |
| 64 | LD$(0,\ 0,\ w)$ | $(0,\ -1,\ 0)$, $(-1,\ 0,\ 0)$ | $\{1\}\oplus\{2\}$ or $\{3\}\oplus\{4\}$ |
| 64 | SM$(u,\ 0,\ 0)$ | $(0,\ -1,\ 0)$, $(0,\ 0,\ 1)$ | $\{1\}\oplus\{2\}$ or $\{3\}\oplus\{4\}$ |
| 65 | A$\left(u,\ 0,\ \frac{1}{2}\right)$ | $(0,\ -1,\ 0)$, $(0,\ 0,\ 1)$ | $\{1\}\oplus\{2\}$ or $\{3\}\oplus\{4\}$ |
| 65 | B$\left(0,\ v,\ \frac{1}{2}\right)$ | $(-1,\ 0,\ 0)$, $(0,\ 0,\ 1)$ | $\{1\}\oplus\{2\}$ or $\{3\}\oplus\{4\}$ |
| 65 | DT$(0,\ v,\ 0)$ | $(-1,\ 0,\ 0)$, $(0,\ 0,\ 1)$ | $\{1\}\oplus\{2\}$ or $\{3\}\oplus\{4\}$ |
| 65 | H$(1,\ 0,\ w)$ | $(0,\ -1,\ 0)$, $(-1,\ 0,\ 0)$ | $\{1\}\oplus\{2\}$ or $\{3\}\oplus\{4\}$ |
| 65 | LD$(0,\ 0,\ w)$ | $(0,\ -1,\ 0)$, $(-1,\ 0,\ 0)$ | $\{1\}\oplus\{2\}$ or $\{3\}\oplus\{4\}$ |
| 65 | SM$(u,\ 0,\ 0)$ | $(0,\ -1,\ 0)$, $(0,\ 0,\ 1)$ | $\{1\}\oplus\{2\}$ or $\{3\}\oplus\{4\}$ |
| 66 | DT$(0,\ v,\ 0)$ | $(-1,\ 0,\ 0)$, $(0,\ 0,\ 1)$ | $\{1\}\oplus\{2\}$ or $\{3\}\oplus\{4\}$ |
| 66 | H$(1,\ 0,\ w)$ | $(0,\ -1,\ 0)$, $(-1,\ 0,\ 0)$ | $\{1\}\oplus\{2\}$ or $\{3\}\oplus\{4\}$ |
| 66 | LD$(0,\ 0,\ w)$ | $(0,\ -1,\ 0)$, $(-1,\ 0,\ 0)$ | $\{1\}\oplus\{2\}$ or $\{3\}\oplus\{4\}$ |
| 66 | SM$(u,\ 0,\ 0)$ | $(0,\ -1,\ 0)$, $(0,\ 0,\ 1)$ | $\{1\}\oplus\{2\}$ or $\{3\}\oplus\{4\}$ |
| 67 | A$\left(u,\ 0,\ \frac{1}{2}\right)$ | $(0,\ -1,\ 0)$, $(0,\ 0,\ 1)$ | $\{1\}\oplus\{2\}$ or $\{3\}\oplus\{4\}$ |
| 67 | B$\left(0,\ v,\ \frac{1}{2}\right)$ | $(-1,\ 0,\ 0)$, $(0,\ 0,\ 1)$ | $\{1\}\oplus\{2\}$ or $\{3\}\oplus\{4\}$ |
| 67 | DT$(0,\ v,\ 0)$ | $(-1,\ 0,\ 0)$, $(0,\ 0,\ 1)$ | $\{1\}\oplus\{2\}$ or $\{3\}\oplus\{4\}$ |
| 67 | H$(1,\ 0,\ w)$ | $(0,\ -1,\ 0)$, $(-1,\ 0,\ 0)$ | $\{1\}\oplus\{2\}$ or $\{3\}\oplus\{4\}$ |
| 67 | LD$(0,\ 0,\ w)$ | $(0,\ -1,\ 0)$, $(-1,\ 0,\ 0)$ | $\{1\}\oplus\{2\}$ or $\{3\}\oplus\{4\}$ |
| 67 | SM$(u,\ 0,\ 0)$ | $(0,\ -1,\ 0)$, $(0,\ 0,\ 1)$ | $\{1\}\oplus\{2\}$ or $\{3\}\oplus\{4\}$ |
| 68 | DT$(0,\ v,\ 0)$ | $(-1,\ 0,\ 0)$, $(0,\ 0,\ 1)$ | $\{1\}\oplus\{2\}$ or $\{3\}\oplus\{4\}$ |
| 68 | H$(1,\ 0,\ w)$ | $(0,\ -1,\ 0)$, $(-1,\ 0,\ 0)$ | $\{1\}\oplus\{2\}$ or $\{3\}\oplus\{4\}$ |
| 68 | LD$(0,\ 0,\ w)$ | $(0,\ -1,\ 0)$, $(-1,\ 0,\ 0)$ | $\{1\}\oplus\{2\}$ or $\{3\}\oplus\{4\}$ |
| 68 | SM$(u,\ 0,\ 0)$ | $(0,\ -1,\ 0)$, $(0,\ 0,\ 1)$ | $\{1\}\oplus\{2\}$ or $\{3\}\oplus\{4\}$ |
| 69 | A$(u,\ 0,\ 1)$ | $(0,\ 0,\ -1)$, $(0,\ 1,\ 0)$ | $\{1\}\oplus\{2\}$ or $\{3\}\oplus\{4\}$ |
| 69 | B$(0,\ v,\ 1)$ | $(0,\ 0,\ -1)$, $(1,\ 0,\ 0)$ | $\{1\}\oplus\{2\}$ or $\{3\}\oplus\{4\}$ |
| 69 | DT$(0,\ v,\ 0)$ | $(0,\ 0,\ -1)$, $(1,\ 0,\ 0)$ | $\{1\}\oplus\{2\}$ or $\{3\}\oplus\{4\}$ |
| 69 | H$(0,\ 1,\ w)$ | $(0,\ 1,\ 0)$, $(1,\ 0,\ 0)$ | $\{1\}\oplus\{2\}$ or $\{3\}\oplus\{4\}$ |
| 69 | LD$(0,\ 0,\ w)$ | $(0,\ 1,\ 0)$, $(1,\ 0,\ 0)$ | $\{1\}\oplus\{2\}$ or $\{3\}\oplus\{4\}$ |
| 69 | SM$(u,\ 0,\ 0)$ | $(0,\ 0,\ -1)$, $(0,\ 1,\ 0)$ | $\{1\}\oplus\{2\}$ or $\{3\}\oplus\{4\}$ |
| 70 | DT$(0,\ v,\ 0)$ | $(0,\ 0,\ -1)$, $(1,\ 0,\ 0)$ | $\{1\}\oplus\{2\}$ or $\{3\}\oplus\{4\}$ |
| 70 | LD$(0,\ 0,\ w)$ | $(0,\ -1,\ 0)$, $(1,\ 0,\ 0)$ | $\{1\}\oplus\{2\}$ or $\{3\}\oplus\{4\}$ |

| SG | HSL | Location of nodal chain | Irreps of BC |
|---|---|---|---|
| 70 | SM$(u,\ 0,\ 0)$ | $(0,\ -1,\ 0)$, $(0,\ 0,\ -1)$ | $\{1\}\oplus\{2\}$ or $\{3\}\oplus\{4\}$ |
| 71 | DT$(0,\ v,\ 0)$ | $(0,\ 0,\ -1)$, $(1,\ 0,\ 0)$ | $\{1\}\oplus\{2\}$ or $\{3\}\oplus\{4\}$ |
| 71 | LD$(0,\ 0,\ w)$ | $(0,\ -1,\ 0)$, $(1,\ 0,\ 0)$ | $\{1\}\oplus\{2\}$ or $\{3\}\oplus\{4\}$ |
| 71 | SM$(u,\ 0,\ 0)$ | $(0,\ 0,\ -1)$, $(0,\ -1,\ 0)$ | $\{1\}\oplus\{2\}$ or $\{3\}\oplus\{4\}$ |
| 72 | DT$(0,\ v,\ 0)$ | $(0,\ 0,\ -1)$, $(1,\ 0,\ 0)$ | $\{1\}\oplus\{2\}$ or $\{3\}\oplus\{4\}$ |
| 72 | LD$(0,\ 0,\ w)$ | $(0,\ -1,\ 0)$, $(1,\ 0,\ 0)$ | $\{1\}\oplus\{2\}$ or $\{3\}\oplus\{4\}$ |
| 72 | SM$(u,\ 0,\ 0)$ | $(0,\ 0,\ -1)$, $(0,\ -1,\ 0)$ | $\{1\}\oplus\{2\}$ or $\{3\}\oplus\{4\}$ |
| 73 | DT$(0,\ v,\ 0)$ | $(0,\ 0,\ -1)$, $(1,\ 0,\ 0)$ | $\{1\}\oplus\{2\}$ or $\{3\}\oplus\{4\}$ |
| 73 | LD$(0,\ 0,\ w)$ | $(0,\ -1,\ 0)$, $(1,\ 0,\ 0)$ | $\{1\}\oplus\{2\}$ or $\{3\}\oplus\{4\}$ |
| 73 | SM$(u,\ 0,\ 0)$ | $(0,\ 0,\ -1)$, $(0,\ -1,\ 0)$ | $\{1\}\oplus\{2\}$ or $\{3\}\oplus\{4\}$ |
| 74 | DT$(0,\ v,\ 0)$ | $(0,\ 0,\ -1)$, $(1,\ 0,\ 0)$ | $\{1\}\oplus\{2\}$ or $\{3\}\oplus\{4\}$ |
| 74 | LD$(0,\ 0,\ w)$ | $(0,\ -1,\ 0)$, $(1,\ 0,\ 0)$ | $\{1\}\oplus\{2\}$ or $\{3\}\oplus\{4\}$ |
| 74 | SM$(u,\ 0,\ 0)$ | $(0,\ 0,\ -1)$, $(0,\ -1,\ 0)$ | $\{1\}\oplus\{2\}$ or $\{3\}\oplus\{4\}$ |
| 99 | W$\left(0,\ \frac{1}{2},\ w\right)$ | $(1,\ 0,\ 0)$, $(0,\ -1,\ 0)$ | $1\oplus2$ or $3\oplus4$ |
| 101 | W$\left(0,\ \frac{1}{2},\ w\right)$ | $(1,\ 0,\ 0)$, $(0,\ -1,\ 0)$ | $1\oplus2$ or $3\oplus4$ |
| 103 | W$\left(0,\ \frac{1}{2},\ w\right)$ | $(1,\ 0,\ 0)$, $(0,\ -1,\ 0)$ | $1\oplus2$ or $3\oplus4$ |
| 105 | W$\left(0,\ \frac{1}{2},\ w\right)$ | $(1,\ 0,\ 0)$, $(0,\ -1,\ 0)$ | $1\oplus2$ or $3\oplus4$ |
| 107 | W$\left(\frac{1}{2},\ \frac{1}{2},\ w\right)$ | $\left(-\frac{\sqrt{2}}{2},\ -\frac{\sqrt{2}}{2},\ 0\right)$, $\left(\frac{\sqrt{2}}{2},\ -\frac{\sqrt{2}}{2},\ 0\right)$ | $1\oplus2$ or $3\oplus4$ |
| 108 | W$\left(\frac{1}{2},\ \frac{1}{2},\ w\right)$ | $\left(-\frac{\sqrt{2}}{2},\ -\frac{\sqrt{2}}{2},\ 0\right)$, $\left(\frac{\sqrt{2}}{2},\ -\frac{\sqrt{2}}{2},\ 0\right)$ | $1\oplus2$ or $3\oplus4$ |
| 115 | W$\left(0,\ \frac{1}{2},\ w\right)$ | $(1,\ 0,\ 0)$, $(0,\ -1,\ 0)$ | $1\oplus2$ or $3\oplus4$ |
| 116 | W$\left(0,\ \frac{1}{2},\ w\right)$ | $(1,\ 0,\ 0)$, $(0,\ -1,\ 0)$ | $1\oplus2$ or $3\oplus4$ |
| 121 | W$\left(\frac{1}{2},\ \frac{1}{2},\ w\right)$ | $\left(-\frac{\sqrt{2}}{2},\ -\frac{\sqrt{2}}{2},\ 0\right)$, $\left(-\frac{\sqrt{2}}{2},\ \frac{\sqrt{2}}{2},\ 0\right)$ | $1\oplus2$ or $3\oplus4$ |
| 123 | DT$(0,\ v,\ 0)$ | $(0,\ 0,\ 1)$, $(1,\ 0,\ 0)$ | $\{1\}\oplus\{2\}$ or $\{3\}\oplus\{4\}$ |
| 123 | S$\left(u,\ u,\ \frac{1}{2}\right)$ | $(0,\ 0,\ 1)$, $\left(\frac{\sqrt{2}}{2},\ -\frac{\sqrt{2}}{2},\ 0\right)$ | $\{1\}\oplus\{2\}$ or $\{3\}\oplus\{4\}$ |
| 123 | SM$(u,\ u,\ 0)$ | $(0,\ 0,\ 1)$, $\left(\frac{\sqrt{2}}{2},\ -\frac{\sqrt{2}}{2},\ 0\right)$ | $\{1\}\oplus\{2\}$ or $\{3\}\oplus\{4\}$ |
| 123 | T$\left(u,\ \frac{1}{2},\ \frac{1}{2}\right)$ | $(0,\ 0,\ 1)$, $(0,\ -1,\ 0)$ | $\{1\}\oplus\{2\}$ or $\{3\}\oplus\{4\}$ |
| 123 | U$\left(0,\ v,\ \frac{1}{2}\right)$ | $(0,\ 0,\ 1)$, $(1,\ 0,\ 0)$ | $\{1\}\oplus\{2\}$ or $\{3\}\oplus\{4\}$ |
| 123 | W$\left(0,\ \frac{1}{2},\ w\right)$ | $(1,\ 0,\ 0)$, $(0,\ -1,\ 0)$ | $\{1\}\oplus\{2\}$ or $\{3\}\oplus\{4\}$ |
| 123 | Y$\left(u,\ \frac{1}{2},\ 0\right)$ | $(0,\ 0,\ 1)$, $(0,\ -1,\ 0)$ | $\{1\}\oplus\{2\}$ or $\{3\}\oplus\{4\}$ |
| 124 | DT$(0,\ v,\ 0)$ | $(0,\ 0,\ 1)$, $(1,\ 0,\ 0)$ | $\{1\}\oplus\{2\}$ or $\{3\}\oplus\{4\}$ |
| 124 | SM$(u,\ u,\ 0)$ | $(0,\ 0,\ 1)$, $\left(\frac{\sqrt{2}}{2},\ -\frac{\sqrt{2}}{2},\ 0\right)$ | $\{1\}\oplus\{2\}$ or $\{3\}\oplus\{4\}$ |
| 124 | W$\left(0,\ \frac{1}{2},\ w\right)$ | $(1,\ 0,\ 0)$, $(0,\ -1,\ 0)$ | $\{1\}\oplus\{2\}$ or $\{3\}\oplus\{4\}$ |
| 124 | Y$\left(u,\ \frac{1}{2},\ 0\right)$ | $(0,\ 0,\ 1)$, $(0,\ -1,\ 0)$ | $\{1\}\oplus\{2\}$ or $\{3\}\oplus\{4\}$ |
| 125 | DT$(0,\ v,\ 0)$ | $(0,\ 0,\ 1)$, $(1,\ 0,\ 0)$ | $\{1\}\oplus\{2\}$ or $\{3\}\oplus\{4\}$ |
| 125 | S$\left(u,\ u,\ \frac{1}{2}\right)$ | $(0,\ 0,\ 1)$, $\left(\frac{\sqrt{2}}{2},\ -\frac{\sqrt{2}}{2},\ 0\right)$ | $\{1\}\oplus\{2\}$ or $\{3\}\oplus\{4\}$ |
| 125 | SM$(u,\ u,\ 0)$ | $(0,\ 0,\ 1)$, $\left(\frac{\sqrt{2}}{2},\ -\frac{\sqrt{2}}{2},\ 0\right)$ | $\{1\}\oplus\{2\}$ or $\{3\}\oplus\{4\}$ |
| 125 | U$\left(0,\ v,\ \frac{1}{2}\right)$ | $(0,\ 0,\ 1)$, $(1,\ 0,\ 0)$ | $\{1\}\oplus\{2\}$ or $\{3\}\oplus\{4\}$ |
| 126 | DT$(0,\ v,\ 0)$ | $(0,\ 0,\ 1)$, $(1,\ 0,\ 0)$ | $\{1\}\oplus\{2\}$ or $\{3\}\oplus\{4\}$ |
| 126 | SM$(u,\ u,\ 0)$ | $(0,\ 0,\ 1)$, $\left(\frac{\sqrt{2}}{2},\ -\frac{\sqrt{2}}{2},\ 0\right)$ | $\{1\}\oplus\{2\}$ or $\{3\}\oplus\{4\}$ |
| 126 | T$\left(u,\ \frac{1}{2},\ \frac{1}{2}\right)$ | $(0,\ 0,\ 1)$, $(0,\ -1,\ 0)$ | $\{1\}\oplus\{2\}$ or $\{3\}\oplus\{4\}$ |

| SG | HSL | Location of nodal chain | Irreps of BC |
| --- | --- | --- | --- |
| 127 | DT$(0,\ v,\ 0)$ | $(0,\ 0,\ 1)$, $(1,\ 0,\ 0)$ | {1}⊕{2} or {3}⊕{4} |
| 127 | S$\left(u,\ u,\ \frac{1}{2}\right)$ | $(0,\ 0,\ 1)$, $\left(\frac{\sqrt{2}}{2},\ -\frac{\sqrt{2}}{2},\ 0\right)$ | {1}⊕{2} or {3}⊕{4} |
| 127 | SM$(u,\ u,\ 0)$ | $(0,\ 0,\ 1)$, $\left(\frac{\sqrt{2}}{2},\ -\frac{\sqrt{2}}{2},\ 0\right)$ | {1}⊕{2} or {3}⊕{4} |
| 127 | U$\left(0,\ v,\ \frac{1}{2}\right)$ | $(0,\ 0,\ 1)$, $(1,\ 0,\ 0)$ | {1}⊕{2} or {3}⊕{4} |
| 128 | DT$(0,\ v,\ 0)$ | $(0,\ 0,\ 1)$, $(1,\ 0,\ 0)$ | {1}⊕{2} or {3}⊕{4} |
| 128 | SM$(u,\ u,\ 0)$ | $(0,\ 0,\ 1)$, $\left(\frac{\sqrt{2}}{2},\ -\frac{\sqrt{2}}{2},\ 0\right)$ | {1}⊕{2} or {3}⊕{4} |
| 129 | DT$(0,\ v,\ 0)$ | $(0,\ 0,\ 1)$, $(1,\ 0,\ 0)$ | {1}⊕{2} or {3}⊕{4} |
| 129 | S$\left(u,\ u,\ \frac{1}{2}\right)$ | $(0,\ 0,\ 1)$, $\left(\frac{\sqrt{2}}{2},\ -\frac{\sqrt{2}}{2},\ 0\right)$ | {1}⊕{2} or {3}⊕{4} |
| 129 | SM$(u,\ u,\ 0)$ | $(0,\ 0,\ 1)$, $\left(\frac{\sqrt{2}}{2},\ -\frac{\sqrt{2}}{2},\ 0\right)$ | {1}⊕{2} or {3}⊕{4} |
| 129 | U$\left(0,\ v,\ \frac{1}{2}\right)$ | $(0,\ 0,\ 1)$, $(1,\ 0,\ 0)$ | {1}⊕{2} or {3}⊕{4} |
| 130 | DT$(0,\ v,\ 0)$ | $(0,\ 0,\ 1)$, $(1,\ 0,\ 0)$ | {1}⊕{2} or {3}⊕{4} |
| 130 | SM$(u,\ u,\ 0)$ | $(0,\ 0,\ 1)$, $\left(\frac{\sqrt{2}}{2},\ -\frac{\sqrt{2}}{2},\ 0\right)$ | {1}⊕{2} or {3}⊕{4} |
| 131 | DT$(0,\ v,\ 0)$ | $(0,\ 0,\ 1)$, $(1,\ 0,\ 0)$ | {1}⊕{2} or {3}⊕{4} |
| 131 | SM$(u,\ u,\ 0)$ | $(0,\ 0,\ 1)$, $\left(\frac{\sqrt{2}}{2},\ -\frac{\sqrt{2}}{2},\ 0\right)$ | {1}⊕{2} or {3}⊕{4} |
| 131 | T$\left(u,\ \frac{1}{2},\ \frac{1}{2}\right)$ | $(0,\ 0,\ 1)$, $(0,\ -1,\ 0)$ | {1}⊕{2} or {3}⊕{4} |
| 131 | U$\left(0,\ v,\ \frac{1}{2}\right)$ | $(0,\ 0,\ 1)$, $(1,\ 0,\ 0)$ | {1}⊕{2} or {3}⊕{4} |
| 131 | W$\left(0,\ \frac{1}{2},\ w\right)$ | $(1,\ 0,\ 0)$, $(0,\ -1,\ 0)$ | {1}⊕{2} or {3}⊕{4} |
| 131 | Y$\left(u,\ \frac{1}{2},\ 0\right)$ | $(0,\ 0,\ 1)$, $(0,\ -1,\ 0)$ | {1}⊕{2} or {3}⊕{4} |
| 132 | DT$(0,\ v,\ 0)$ | $(0,\ 0,\ 1)$, $(1,\ 0,\ 0)$ | {1}⊕{2} or {3}⊕{4} |
| 132 | S$\left(u,\ u,\ \frac{1}{2}\right)$ | $(0,\ 0,\ 1)$, $\left(\frac{\sqrt{2}}{2},\ -\frac{\sqrt{2}}{2},\ 0\right)$ | {1}⊕{3} or {2}⊕{4} |
| 132 | SM$(u,\ u,\ 0)$ | $(0,\ 0,\ 1)$, $\left(\frac{\sqrt{2}}{2},\ -\frac{\sqrt{2}}{2},\ 0\right)$ | {1}⊕{2} or {3}⊕{4} |
| 132 | W$\left(0,\ \frac{1}{2},\ w\right)$ | $(1,\ 0,\ 0)$, $(0,\ -1,\ 0)$ | {1}⊕{2} or {3}⊕{4} |
| 132 | Y$\left(u,\ \frac{1}{2},\ 0\right)$ | $(0,\ 0,\ 1)$, $(0,\ -1,\ 0)$ | {1}⊕{2} or {3}⊕{4} |
| 133 | DT$(0,\ v,\ 0)$ | $(0,\ 0,\ 1)$, $(1,\ 0,\ 0)$ | {1}⊕{2} or {3}⊕{4} |
| 133 | SM$(u,\ u,\ 0)$ | $(0,\ 0,\ 1)$, $\left(\frac{\sqrt{2}}{2},\ -\frac{\sqrt{2}}{2},\ 0\right)$ | {1}⊕{2} or {3}⊕{4} |
| 133 | U$\left(0,\ v,\ \frac{1}{2}\right)$ | $(0,\ 0,\ 1)$, $(1,\ 0,\ 0)$ | {1}⊕{2} or {3}⊕{4} |
| 134 | DT$(0,\ v,\ 0)$ | $(0,\ 0,\ 1)$, $(1,\ 0,\ 0)$ | {1}⊕{2} or {3}⊕{4} |
| 134 | S$\left(u,\ u,\ \frac{1}{2}\right)$ | $(0,\ 0,\ 1)$, $\left(\frac{\sqrt{2}}{2},\ -\frac{\sqrt{2}}{2},\ 0\right)$ | {1}⊕{3} or {2}⊕{4} |
| 134 | SM$(u,\ u,\ 0)$ | $(0,\ 0,\ 1)$, $\left(\frac{\sqrt{2}}{2},\ -\frac{\sqrt{2}}{2},\ 0\right)$ | {1}⊕{2} or {3}⊕{4} |
| 134 | T$\left(u,\ \frac{1}{2},\ \frac{1}{2}\right)$ | $(0,\ 0,\ 1)$, $(0,\ -1,\ 0)$ | {1}⊕{2} or {3}⊕{4} |
| 135 | DT$(0,\ v,\ 0)$ | $(0,\ 0,\ 1)$, $(1,\ 0,\ 0)$ | {1}⊕{2} or {3}⊕{4} |
| 135 | SM$(u,\ u,\ 0)$ | $(0,\ 0,\ 1)$, $\left(\frac{\sqrt{2}}{2},\ -\frac{\sqrt{2}}{2},\ 0\right)$ | {1}⊕{2} or {3}⊕{4} |
| 135 | U$\left(0,\ v,\ \frac{1}{2}\right)$ | $(0,\ 0,\ 1)$, $(1,\ 0,\ 0)$ | {1}⊕{2} or {3}⊕{4} |
| 136 | DT$(0,\ v,\ 0)$ | $(0,\ 0,\ 1)$, $(1,\ 0,\ 0)$ | {1}⊕{2} or {3}⊕{4} |
| 136 | S$\left(u,\ u,\ \frac{1}{2}\right)$ | $(0,\ 0,\ 1)$, $\left(\frac{\sqrt{2}}{2},\ -\frac{\sqrt{2}}{2},\ 0\right)$ | {1}⊕{3} or {2}⊕{4} |
| 136 | SM$(u,\ u,\ 0)$ | $(0,\ 0,\ 1)$, $\left(\frac{\sqrt{2}}{2},\ -\frac{\sqrt{2}}{2},\ 0\right)$ | {1}⊕{2} or {3}⊕{4} |
| 137 | DT$(0,\ v,\ 0)$ | $(0,\ 0,\ 1)$, $(1,\ 0,\ 0)$ | {1}⊕{2} or {3}⊕{4} |
| 137 | SM$(u,\ u,\ 0)$ | $(0,\ 0,\ 1)$, $\left(\frac{\sqrt{2}}{2},\ -\frac{\sqrt{2}}{2},\ 0\right)$ | {1}⊕{2} or {3}⊕{4} |
| 137 | U$\left(0,\ v,\ \frac{1}{2}\right)$ | $(0,\ 0,\ 1)$, $(1,\ 0,\ 0)$ | {1}⊕{2} or {3}⊕{4} |

| SG | HSL | Location of nodal chain | Irreps of BC |
|---|---|---|---|
| 138 | DT$(0,\ v,\ 0)$ | $(0,\ 0,\ 1)$, $(1,\ 0,\ 0)$ | $\{1\}\oplus\{2\}$ or $\{3\}\oplus\{4\}$ |
| 138 | S$\left(u,\ u,\ \frac{1}{2}\right)$ | $(0,\ 0,\ 1)$, $\left(\frac{\sqrt{2}}{2},\ -\frac{\sqrt{2}}{2},\ 0\right)$ | $\{1\}\oplus\{3\}$ or $\{2\}\oplus\{4\}$ |
| 138 | SM$(u,\ u,\ 0)$ | $(0,\ 0,\ 1)$, $\left(\frac{\sqrt{2}}{2},\ -\frac{\sqrt{2}}{2},\ 0\right)$ | $\{1\}\oplus\{2\}$ or $\{3\}\oplus\{4\}$ |
| 139 | DT$(u,\ u,\ 0)$ | $\left(\frac{\sqrt{2}}{2},\ -\frac{\sqrt{2}}{2},\ 0\right)$, $(0,\ 0,\ -1)$ | $\{1\}\oplus\{2\}$ or $\{3\}\oplus\{4\}$ |
| 139 | SM$(u,\ 0,\ 0)$ | $(0,\ 1,\ 0)$, $(0,\ 0,\ -1)$ | $\{1\}\oplus\{2\}$ or $\{3\}\oplus\{4\}$ |
| 139 | W$\left(\frac{1}{2},\ \frac{1}{2},\ w\right)$ | $\left(-\frac{\sqrt{2}}{2},\ -\frac{\sqrt{2}}{2},\ 0\right)$, $\left(\frac{\sqrt{2}}{2},\ -\frac{\sqrt{2}}{2},\ 0\right)$ | $\{1\}\oplus\{2\}$ or $\{3\}\oplus\{4\}$ |
| 139 | Y$(u,\ 1-u,\ 0)$ | $\left(-\frac{\sqrt{2}}{2},\ -\frac{\sqrt{2}}{2},\ 0\right)$, $(0,\ 0,\ -1)$ | $\{1\}\oplus\{2\}$ or $\{3\}\oplus\{4\}$ |
| 140 | DT$(u,\ u,\ 0)$ | $\left(\frac{\sqrt{2}}{2},\ -\frac{\sqrt{2}}{2},\ 0\right)$, $(0,\ 0,\ -1)$ | $\{1\}\oplus\{2\}$ or $\{3\}\oplus\{4\}$ |
| 140 | SM$(u,\ 0,\ 0)$ | $(0,\ 1,\ 0)$, $(0,\ 0,\ -1)$ | $\{1\}\oplus\{2\}$ or $\{3\}\oplus\{4\}$ |
| 140 | W$\left(\frac{1}{2},\ \frac{1}{2},\ w\right)$ | $\left(-\frac{\sqrt{2}}{2},\ -\frac{\sqrt{2}}{2},\ 0\right)$, $\left(\frac{\sqrt{2}}{2},\ -\frac{\sqrt{2}}{2},\ 0\right)$ | $\{1\}\oplus\{2\}$ or $\{3\}\oplus\{4\}$ |
| 140 | Y$(u,\ 1-u,\ 0)$ | $\left(-\frac{\sqrt{2}}{2},\ -\frac{\sqrt{2}}{2},\ 0\right)$, $(0,\ 0,\ -1)$ | $\{1\}\oplus\{2\}$ or $\{3\}\oplus\{4\}$ |
| 141 | DT$(u,\ u,\ 0)$ | $\left(\frac{\sqrt{2}}{2},\ -\frac{\sqrt{2}}{2},\ 0\right)$, $(0,\ 0,\ -1)$ | $\{1\}\oplus\{2\}$ or $\{3\}\oplus\{4\}$ |
| 141 | SM$(u,\ 0,\ 0)$ | $(0,\ 1,\ 0)$, $(0,\ 0,\ -1)$ | $\{1\}\oplus\{2\}$ or $\{3\}\oplus\{4\}$ |
| 142 | DT$(u,\ u,\ 0)$ | $\left(-\frac{\sqrt{2}}{2},\ \frac{\sqrt{2}}{2},\ 0\right)$, $(0,\ 0,\ -1)$ | $\{1\}\oplus\{2\}$ or $\{3\}\oplus\{4\}$ |
| 142 | SM$(u,\ 0,\ 0)$ | $(0,\ -1,\ 0)$, $(0,\ 0,\ -1)$ | $\{1\}\oplus\{2\}$ or $\{3\}\oplus\{4\}$ |
| 183 | U$\left(\frac{1}{2},\ 0,\ w\right)$ | $\left(\frac{1}{2},\ -\frac{\sqrt{3}}{2},\ 0\right)$, $\left(-\frac{\sqrt{3}}{2},\ -\frac{1}{2},\ 0\right)$ | $1\oplus2$ or $3\oplus4$ |
| 184 | U$\left(\frac{1}{2},\ 0,\ w\right)$ | $\left(\frac{1}{2},\ -\frac{\sqrt{3}}{2},\ 0\right)$, $\left(-\frac{\sqrt{3}}{2},\ -\frac{1}{2},\ 0\right)$ | $1\oplus2$ or $3\oplus4$ |
| 185 | U$\left(\frac{1}{2},\ 0,\ w\right)$ | $\left(\frac{1}{2},\ -\frac{\sqrt{3}}{2},\ 0\right)$, $\left(-\frac{\sqrt{3}}{2},\ -\frac{1}{2},\ 0\right)$ | $1\oplus2$ or $3\oplus4$ |
| 186 | U$\left(\frac{1}{2},\ 0,\ w\right)$ | $\left(\frac{1}{2},\ -\frac{\sqrt{3}}{2},\ 0\right)$, $\left(-\frac{\sqrt{3}}{2},\ -\frac{1}{2},\ 0\right)$ | $1\oplus2$ or $3\oplus4$ |
| 187 | R$\left(u,\ 0,\ \frac{1}{2}\right)$ | $\left(-\frac{1}{2},\ \frac{\sqrt{3}}{2},\ 0\right)$, $(0,\ 0,\ 1)$ | $1\oplus2$ or $3\oplus4$ |
| 187 | SM$(u,\ 0,\ 0)$ | $\left(-\frac{1}{2},\ \frac{\sqrt{3}}{2},\ 0\right)$, $(0,\ 0,\ 1)$ | $1\oplus2$ or $3\oplus4$ |
| 188 | SM$(u,\ 0,\ 0)$ | $\left(-\frac{1}{2},\ \frac{\sqrt{3}}{2},\ 0\right)$, $(0,\ 0,\ 1)$ | $1\oplus2$ or $3\oplus4$ |
| 189 | LD$(u,\ u,\ 0)$ | $(0,\ 0,\ 1)$, $\left(\frac{\sqrt{3}}{2},\ -\frac{1}{2},\ 0\right)$ | $1\oplus2$ or $3\oplus4$ |
| 189 | Q$\left(u,\ u,\ \frac{1}{2}\right)$ | $\left(\frac{\sqrt{3}}{2},\ -\frac{1}{2},\ 0\right)$, $(0,\ 0,\ 1)$ | $1\oplus2$ or $3\oplus4$ |
| 190 | LD$(u,\ u,\ 0)$ | $(0,\ 0,\ 1)$, $\left(\frac{\sqrt{3}}{2},\ -\frac{1}{2},\ 0\right)$ | $1\oplus2$ or $3\oplus4$ |
| 191 | LD$(u,\ u,\ 0)$ | $(0,\ 0,\ 1)$, $\left(-\frac{\sqrt{3}}{2},\ \frac{1}{2},\ 0\right)$ | $\{1\}\oplus\{2\}$ or $\{3\}\oplus\{4\}$ |
| 191 | Q$\left(u,\ u,\ \frac{1}{2}\right)$ | $\left(-\frac{\sqrt{3}}{2},\ \frac{1}{2},\ 0\right)$, $(0,\ 0,\ 1)$ | $\{1\}\oplus\{2\}$ or $\{3\}\oplus\{4\}$ |
| 191 | R$\left(u,\ 0,\ \frac{1}{2}\right)$ | $\left(\frac{1}{2},\ -\frac{\sqrt{3}}{2},\ 0\right)$, $(0,\ 0,\ 1)$ | $\{1\}\oplus\{2\}$ or $\{3\}\oplus\{4\}$ |
| 191 | SM$(u,\ 0,\ 0)$ | $\left(\frac{1}{2},\ -\frac{\sqrt{3}}{2},\ 0\right)$, $(0,\ 0,\ 1)$ | $\{1\}\oplus\{2\}$ or $\{3\}\oplus\{4\}$ |
| 191 | U$\left(\frac{1}{2},\ 0,\ w\right)$ | $\left(\frac{1}{2},\ -\frac{\sqrt{3}}{2},\ 0\right)$, $\left(-\frac{\sqrt{3}}{2},\ -\frac{1}{2},\ 0\right)$ | $\{1\}\oplus\{2\}$ or $\{3\}\oplus\{4\}$ |
| 192 | LD$(u,\ u,\ 0)$ | $(0,\ 0,\ 1)$, $\left(-\frac{\sqrt{3}}{2},\ \frac{1}{2},\ 0\right)$ | $\{1\}\oplus\{2\}$ or $\{3\}\oplus\{4\}$ |
| 192 | SM$(u,\ 0,\ 0)$ | $\left(\frac{1}{2},\ -\frac{\sqrt{3}}{2},\ 0\right)$, $(0,\ 0,\ 1)$ | $\{1\}\oplus\{2\}$ or $\{3\}\oplus\{4\}$ |
| 192 | U$\left(\frac{1}{2},\ 0,\ w\right)$ | $\left(\frac{1}{2},\ -\frac{\sqrt{3}}{2},\ 0\right)$, $\left(-\frac{\sqrt{3}}{2},\ -\frac{1}{2},\ 0\right)$ | $\{1\}\oplus\{2\}$ or $\{3\}\oplus\{4\}$ |
| 193 | LD$(u,\ u,\ 0)$ | $(0,\ 0,\ 1)$, $\left(-\frac{\sqrt{3}}{2},\ \frac{1}{2},\ 0\right)$ | $\{1\}\oplus\{2\}$ or $\{3\}\oplus\{4\}$ |
| 193 | SM$(u,\ 0,\ 0)$ | $\left(\frac{1}{2},\ -\frac{\sqrt{3}}{2},\ 0\right)$, $(0,\ 0,\ 1)$ | $\{1\}\oplus\{2\}$ or $\{3\}\oplus\{4\}$ |
| 193 | U$\left(\frac{1}{2},\ 0,\ w\right)$ | $\left(\frac{1}{2},\ -\frac{\sqrt{3}}{2},\ 0\right)$, $\left(-\frac{\sqrt{3}}{2},\ -\frac{1}{2},\ 0\right)$ | $\{1\}\oplus\{2\}$ or $\{3\}\oplus\{4\}$ |
| 194 | LD$(u,\ u,\ 0)$ | $(0,\ 0,\ 1)$, $\left(-\frac{\sqrt{3}}{2},\ \frac{1}{2},\ 0\right)$ | $\{1\}\oplus\{2\}$ or $\{3\}\oplus\{4\}$ |

| SG | HSL | Location of nodal chain | Irreps of BC |
|---|---|---|---|
| 194 | SM$(u,\ 0,\ 0)$ | $\left(\frac{1}{2},\ -\frac{\sqrt{3}}{2},\ 0\right)$, $(0,\ 0,\ 1)$ | $\{1\}\oplus\{2\}$ or $\{3\}\oplus\{4\}$ |
| 194 | U$\left(\frac{1}{2},\ 0,\ w\right)$ | $\left(\frac{1}{2},\ -\frac{\sqrt{3}}{2},\ 0\right)$, $\left(-\frac{\sqrt{3}}{2},\ -\frac{1}{2},\ 0\right)$ | $\{1\}\oplus\{2\}$ or $\{3\}\oplus\{4\}$ |
| 200 | DT$(0,\ v,\ 0)$ | $(0,\ 0,\ 1)$, $(1,\ 0,\ 0)$ | $\{1\}\oplus\{2\}$ or $\{3\}\oplus\{4\}$ |
| 200 | T$\left(\frac{1}{2},\ \frac{1}{2},\ w\right)$ | $(0,\ -1,\ 0)$, $(-1,\ 0,\ 0)$ | $\{1\}\oplus\{2\}$ or $\{3\}\oplus\{4\}$ |
| 200 | ZA$\left(\frac{1}{2},\ u,\ 0\right)$ | $(0,\ 0,\ 1)$, $(-1,\ 0,\ 0)$ | $\{1\}\oplus\{2\}$ or $\{3\}\oplus\{4\}$ |
| 200 | Z$\left(u,\ \frac{1}{2},\ 0\right)$ | $(0,\ 0,\ 1)$, $(0,\ -1,\ 0)$ | $\{1\}\oplus\{2\}$ or $\{3\}\oplus\{4\}$ |
| 201 | DT$(0,\ v,\ 0)$ | $(0,\ 0,\ 1)$, $(1,\ 0,\ 0)$ | $\{1\}\oplus\{2\}$ or $\{3\}\oplus\{4\}$ |
| 201 | T$\left(\frac{1}{2},\ \frac{1}{2},\ w\right)$ | $(0,\ -1,\ 0)$, $(-1,\ 0,\ 0)$ | $\{1\}\oplus\{2\}$ or $\{3\}\oplus\{4\}$ |
| 202 | DT$(0,\ v,\ 0)$ | $(0,\ 0,\ -1)$, $(-1,\ 0,\ 0)$ | $\{1\}\oplus\{2\}$ or $\{3\}\oplus\{4\}$ |
| 202 | V$(u,\ 1,\ 0)$ | $(0,\ 0,\ -1)$, $(0,\ -1,\ 0)$ | $\{1\}\oplus\{2\}$ or $\{3\}\oplus\{4\}$ |
| 203 | DT$(0,\ v,\ 0)$ | $(0,\ 0,\ -1)$, $(-1,\ 0,\ 0)$ | $\{1\}\oplus\{2\}$ or $\{3\}\oplus\{4\}$ |
| 204 | DT$(0,\ v,\ 0)$ | $(0,\ 0,\ -1)$, $(-1,\ 0,\ 0)$ | $\{1\}\oplus\{2\}$ or $\{3\}\oplus\{4\}$ |
| 205 | DT$(0,\ v,\ 0)$ | $(0,\ 0,\ 1)$, $(1,\ 0,\ 0)$ | $\{1\}\oplus\{2\}$ or $\{3\}\oplus\{4\}$ |
| 206 | DT$(0,\ v,\ 0)$ | $(0,\ 0,\ -1)$, $(-1,\ 0,\ 0)$ | $\{1\}\oplus\{2\}$ or $\{3\}\oplus\{4\}$ |
| 217 | D$\left(\frac{1}{2},\ \frac{1}{2},\ w\right)$ | $\left(-\frac{\sqrt{2}}{2},\ \frac{\sqrt{2}}{2},\ 0\right)$, $\left(-\frac{\sqrt{2}}{2},\ -\frac{\sqrt{2}}{2},\ 0\right)$ | $1\oplus2$ or $3\oplus4$ |
| 221 | S$\left(u,\ \frac{1}{2},\ u\right)$ | $\left(-\frac{\sqrt{2}}{2},\ 0,\ \frac{\sqrt{2}}{2}\right)$, $(0,\ -1,\ 0)$ | $\{1\}\oplus\{2\}$ or $\{3\}\oplus\{4\}$ |
| 221 | SM$(u,\ u,\ 0)$ | $\left(\frac{\sqrt{2}}{2},\ -\frac{\sqrt{2}}{2},\ 0\right)$, $(0,\ 0,\ 1)$ | $\{1\}\oplus\{2\}$ or $\{3\}\oplus\{4\}$ |
| 221 | Z$\left(u,\ \frac{1}{2},\ 0\right)$ | $(0,\ 0,\ 1)$, $(0,\ -1,\ 0)$ | $\{1\}\oplus\{2\}$ or $\{3\}\oplus\{4\}$ |
| 222 | SM$(u,\ u,\ 0)$ | $\left(\frac{\sqrt{2}}{2},\ -\frac{\sqrt{2}}{2},\ 0\right)$, $(0,\ 0,\ 1)$ | $\{1\}\oplus\{2\}$ or $\{3\}\oplus\{4\}$ |
| 223 | SM$(u,\ u,\ 0)$ | $\left(\frac{\sqrt{2}}{2},\ -\frac{\sqrt{2}}{2},\ 0\right)$, $(0,\ 0,\ 1)$ | $\{1\}\oplus\{2\}$ or $\{3\}\oplus\{4\}$ |
| 223 | Z$\left(u,\ \frac{1}{2},\ 0\right)$ | $(0,\ 0,\ 1)$, $(0,\ -1,\ 0)$ | $\{1\}\oplus\{2\}$ or $\{3\}\oplus\{4\}$ |
| 224 | S$\left(u,\ \frac{1}{2},\ u\right)$ | $\left(-\frac{\sqrt{2}}{2},\ 0,\ \frac{\sqrt{2}}{2}\right)$, $(0,\ -1,\ 0)$ | $\{1\}\oplus\{3\}$ or $\{2\}\oplus\{4\}$ |
| 224 | SM$(u,\ u,\ 0)$ | $\left(\frac{\sqrt{2}}{2},\ -\frac{\sqrt{2}}{2},\ 0\right)$, $(0,\ 0,\ 1)$ | $\{1\}\oplus\{2\}$ or $\{3\}\oplus\{4\}$ |
| 225 | SM$(u,\ u,\ 0)$ | $(0,\ 0,\ -1)$, $\left(-\frac{\sqrt{2}}{2},\ \frac{\sqrt{2}}{2},\ 0\right)$ | $\{1\}\oplus\{2\}$ or $\{3\}\oplus\{4\}$ |
| 225 | V$(u,\ 1,\ 0)$ | $(0,\ 0,\ -1)$, $(0,\ -1,\ 0)$ | $\{1\}\oplus\{2\}$ or $\{3\}\oplus\{4\}$ |
| 226 | SM$(u,\ u,\ 0)$ | $(0,\ 0,\ -1)$, $\left(-\frac{\sqrt{2}}{2},\ \frac{\sqrt{2}}{2},\ 0\right)$ | $\{1\}\oplus\{2\}$ or $\{3\}\oplus\{4\}$ |
| 226 | V$(u,\ 1,\ 0)$ | $(0,\ 0,\ -1)$, $(0,\ -1,\ 0)$ | $\{1\}\oplus\{2\}$ or $\{3\}\oplus\{4\}$ |
| 227 | SM$(u,\ u,\ 0)$ | $(0,\ 0,\ -1)$, $\left(-\frac{\sqrt{2}}{2},\ \frac{\sqrt{2}}{2},\ 0\right)$ | $\{1\}\oplus\{2\}$ or $\{3\}\oplus\{4\}$ |
| 228 | SM$(u,\ u,\ 0)$ | $(0,\ 0,\ -1)$, $\left(-\frac{\sqrt{2}}{2},\ \frac{\sqrt{2}}{2},\ 0\right)$ | $\{1\}\oplus\{2\}$ or $\{3\}\oplus\{4\}$ |
| 229 | D$\left(\frac{1}{2},\ \frac{1}{2},\ w\right)$ | $\left(-\frac{\sqrt{2}}{2},\ \frac{\sqrt{2}}{2},\ 0\right)$, $\left(-\frac{\sqrt{2}}{2},\ -\frac{\sqrt{2}}{2},\ 0\right)$ | $\{1\}\oplus\{2\}$ or $\{3\}\oplus\{4\}$ |
| 229 | G$(u+1,\ 1-u,\ 1)$ | $\left(-\frac{\sqrt{2}}{2},\ -\frac{\sqrt{2}}{2},\ 0\right)$, $(0,\ 0,\ -1)$ | $\{1\}\oplus\{2\}$ or $\{3\}\oplus\{4\}$ |
| 229 | SM$(u,\ u,\ 0)$ | $\left(-\frac{\sqrt{2}}{2},\ \frac{\sqrt{2}}{2},\ 0\right)$, $(0,\ 0,\ -1)$ | $\{1\}\oplus\{2\}$ or $\{3\}\oplus\{4\}$ |
| 230 | SM$(u,\ u,\ 0)$ | $\left(-\frac{\sqrt{2}}{2},\ \frac{\sqrt{2}}{2},\ 0\right)$, $(0,\ 0,\ -1)$ | $\{1\}\oplus\{2\}$ or $\{3\}\oplus\{4\}$ |

# References


[1] https://github.com/atztogo/phonondb.

[2] Kresse, G.; Furthmüller, J. Efficient iterative schemes for ab initio total-energy calculations using a plane-wave basis set. *Phys. Rev. B* **1996**, *54*, 11169.

[3] Kresse, G.; Furthmuller, J. Efficiency of ab-initio total energy calculations for metals and semiconductors using a plane-wave basis set. *Comput. Mater. Sci.* **1996**, *6*, 15.

[4] Togo, A.; Tanaka, I. First principles phonon calculations in materials science. *Scr. Mater.* **2015**, *108*, 1.

[5] https://github.com/quanshengwu/wannier_tools/tree/master/utility/phonopyTB.

[6] Wu, Q.; Zhang, S.; Song, H.-F.; Troyer, M.; Soluyanov, A. A. WannierTools: An open-source software package for novel topological materials. *Comput. Phys. Commun.* **2018**, *224*, 405.

[7] Sancho, M. P. L.; Sancho, J. M. L.; Rubio, J. Highly convergent schemes for the calculation of bulk and surface Green functions. *J. Phys. F: Met. Phys.* **1985**, *15*, 851.

[8] http://www.cryst.ehu.es.

[9] Leal-Gonzalez, J.; Melibary, S. A.; Smith, A. J. Structure of lithium gallium sulfide, $LiGaS_2$. *Acta Cryst. C* **1990**, *46*, 2017.

[10] Isaenko, L.; Vasilyeva, I.; Merkulov, A.; Yelisseyev, A.; Lobanov, S. Growth of new nonlinear crystals $LiMX_2$ (M = Al, In, Ga; X = S, Se, Te) for the mid-IR optics. *J. Cryst. Growth* **2005**, *275*, 217.

[11] Isaenko, L. I.; Vasilyeva, I. G. Nonlinear $LiB^{III}C_2^{VI}$ crystals for mid-IR and far-IR:: Novel aspects in crystal growth. *J. Cryst. Growth* **2008**, *310*, 1954.

[12] Ibanez, R.; gravereau, P.; Garcia, A.; Fouassier, C. Structural study of $NaNdGa_4S_8$, a luminescent material with low-concentration quenching. *J. Sol. St. Chem.* **1988**, *73*, 252.

[13] Junggeburth, S. C.; Oeckler, O.; Johrendt, D.; Schnick, W. Nitridogermanate Nitrides $Sr_7[GeN_4]N_2$ and $Ca_7[GeN_4]N_2$: Synthesis Employing Sodium Melts, Crystal Structure, and Density-Functional Theory Calculations. *Inorg. Chem.* **2008**, *47*, 12018.

[14] https://next-gen.materialsproject.org/.
